# Supplementary material for: Provenance-based Data Skipping (TechReport)
Source: arXiv:2104.12815 source file (2021-05-27)
Supplement: Supplementary file 1 [file capture_appendix.tex]

%%%%%%%%%%%%%%%%%%%%%%%%%%%%%%%%%%%%%%%%%%%%%%%%%%%%%%%%%%%%%%%%%%%%%%%%%%%%%%%%
\section{Provenance Sketch Capture}
\label{sec:ps-capture}
In this section, we introduce how do we compute each kind of provenance sketches in detail, e.g., range-based and hash-based. Recall the definition of provenance sketch is that a table is divided into a number of fragments, then we figure out a set of fragments, each fragment in the set includes the provenance of a query and all of them together are sufficient for answering the query. Thus instead of computing the provenance, we compute the set of fragments. The state-of-the-art provenance capture technique~\cite{KG12,GA12} is to model provenance as annotations on data and  capture provenance by propagating annotations. For example, let us recall the example shown in Sec.~\ref{sec:introduction}.  Each tuple in student table is annotated with a variable $a_i$ where $a_i \in \{1,2,...,8\}$ (see Fig.~\ref{stud}) and then annotations are propagated with the running of Q2, at last we get one result tuple with annotation $a_1 + a_2$ (see Fig.~\ref{tab:r2}).  Here the annotation $a_1 + a_2$ indicates the provenance of Q2 that only tuples (Peter, 1) and (Seokki, 2) are needed to compute the result tuple (2,CS). Thus, to compute the provenance sketch, what we can do is that instead of annotating each tuple, we annotate each fragment and then propagate them with the running of the query. Thus assumes the student table is divided into three fragments annotated by $f_1$, $f_2$ and $f_3$ (see Fig.~\ref{stud}), after the running of Q2, only $f_1$  is propagated to the end (see Fig.~\ref{tab:r2}). Thus the provenance sketch for Q2 is $f_1$ in this case. Assuming $f_1$ includes a large number of tuples, instead of materializing these tuples, we only need to materialize this variable $f_1$ for Q2. In this example, we only compute provenance sketch on student table for Q2, we can also compute the provenance sketch on major table or more advanced we can compute several provenance sketches for one table for different partitions, e.g., partitioning on different column, then there might be a set of provenance sketches for one query. 

Thus we divide our computations to two steps. The first one is \textbf{annotating} each fragment which needs the partition informantion that is how do we partition the table such as a hash-partition or a range-partition on different column. The second one is \textbf{propagating} the annotations through each operator of the query. 
%Thus in the following parts of the section, we discuss how do we annotating the fragments under different partition methods which are range-based, hash-based and hash-page-based partitions and then introduce a set of generic instrumentation rules we designed to propagate such kinds of annotations through each operator in the query. 

Before moving to the following parts, it is worth to mention that instead of using a set of fragments number, we use a bit vector to represent each provenance sketch which we called the \emph{bitvector encoding},  i.e., each fragment is represented by one bit where `1' means current partition contains provenance and `0' means without provenance. Thus the three fregments $f_1$, $f_2$ and $f_3$ shown in Fig.~\ref{stud} would be represented as  '100', '010' and '001'. This kind bitvector encoding only needs less than 100 bytes for storage even for large number of fragments and is easy to propagate through some bitwise operations.

\subsection{Annotation Initialization (Init)}
\label{tab:annotate}
In this section, we discuss how to annotate each fragment for each table accessed by a query under different partition methods. Assumes a  table R is partitioned to a set of fragments already, we annotate each tuple with the fragment it belongs to as an additional column in R such that the value in this column could be propagated through each operation of the query. Here we name the column as a word $ps$ plus the table name, e.g., $ps_R$ to represent the annotations in table R. To achieve this goal, we rewrite the R in the query by adding an projection on top through a \emph{case when} clause to check which fragment the tuple belongs to and then store the fragment in the new column $ps_R$ as the annotation of the tuple. Thus for different partition methods, the condition used in the \emph{case when} clause would be different. In the following, we discuss each method individually. 

\parttitle{Range-based Provenance Sketch}
Recall the Def.~\ref{def:hash} that %given a set of ranges on a column A which covers all values in this column, 
the table is partitioned by a set of ranges over one column and the tuples in the same range belong to the same fragment. Thus the condition used in \emph{case when} clause should be a range comparison condition, that is if the tuple in this range, then it belongs to this fragment. For example, given a table $R$ with schema $\{A,B\}$ is partitioned into four fragments by using ranges [1,10), [10,16), [16,30), [30,37) on column A, then $R$ will be rewrited to the SQL shown below that we check the value of A under which range and store the fragment in column PS.  
\lstset{tabsize=4,style=psqlcolor,basicstyle=\scriptsize\upshape\ttfamily}
\begin{lstlisting}
    SELECT  A, B, 
    				 CASE WHEN  A >= 1  AND A < 10 THEN '1000'
    				 		  WHEN  A >= 10 AND A < 16 THEN '0100'
    				 		  WHEN  A >= 16 AND A < 30 THEN '0010'
    				 		  WHEN  A >= 30 AND A < 37 THEN '0001' 
    				 END AS $ps_R$
    FROM  R 
\end{lstlisting}

\parttitle{Hash-based Provenance Sketch}
Recall the Def.~\ref{def:range} we hash on one column and tuples with the same hash result belong to the same fragment. Thus similar with range-based method, instead of checking in which range the value of this column, this method checks which value the hash function returns. For example, assuems we hash the values in column A to four numbers 1, 2, 3 and 4, then the  \emph{case when}  condition would be \lstset{tabsize=4,style=psqlcolor,basicstyle=\scriptsize\upshape\ttfamily}
\begin{lstlisting}
			 CASE WHEN  hash(A,4) = 1 THEN '1000' ... 
\end{lstlisting}

%$R$ will be rewrited to under SQL. 
%\lstset{tabsize=4,style=psqlcolor,basicstyle=\scriptsize\upshape\ttfamily}
%\begin{lstlisting}
%    SELECT  A, B, 
%    				 CASE WHEN  hash(A,4) = 1 THEN '1000'
%    				 		  WHEN  hash(A,4) = 2 THEN '0100'
%    				 		  WHEN  hash(A,4) = 3 THEN '0010'
%    				 		  WHEN  hash(A,4) = 4 THEN '0001' 
%    				 END AS PS
%    FROM  R 
%\end{lstlisting}

\parttitle{Hash-page-based Provenance Sketch}
Recall the Def.~\ref{def:page}, similar with hash-based method, instead of hashing on a column, this method hashs on page number which could be extracted from the row numeber. For example, in postgresql, we can use the command (ctid::text::point)[0] which casts the ctid to an array and get the first element which stores the page number. Thus the pages with the same hash result belong to the same fragment. For example, assuems we hash the page number to four numbers 1, 2, 3 and 4, then the \emph{case when}  condition would be  
\begin{lstlisting}
CASE WHEN hash((ctid::text::point)[0],4) = 1 THEN '1000' ...
\end{lstlisting}

%then $R$ will be rewrited to under SQL. 
%\lstset{tabsize=4,style=psqlcolor,basicstyle=\scriptsize\upshape\ttfamily}
%\begin{lstlisting}
%    SELECT  A, B, 
%    				 CASE WHEN  hash((ctid::text::point)[0],4) = 1 THEN '1000'
%    				 		  WHEN  hash((ctid::text::point)[0],4) = 2 THEN '0100'
%    				 		  WHEN  hash((ctid::text::point)[0],4) = 3 THEN '0010'
%    				 		  WHEN  hash((ctid::text::point)[0],4) = 4 THEN '0001' 
%    				 END AS PS
%    FROM  R 
%\end{lstlisting}

\subsection{Annotation Propagation (Prop)}
\label{tab:propagate}
In this section, we introduce a set of generic instrumentation rules we designed to propagate the initialized annotations through each operator in the query. Recal we stored the annotations in $ps$ column, thus now we only need to propagate the values in this column. We defined the generic rules for each operator of the query, then when a query comes each operator is rewrited based on its matched rule. The rules are shown in Fig.~\ref{fig:cap-rules}. 
%introduce a set of generic instrumentation rules we designed to propagate such kinds of annotations through each operator in the query
%We design and implement a set of instrumentation rules to capture the provenance sketch by annotating each tuple as its partition (each is represented as a bit vector) and propagating them. We defined the generic rules for each operator of the query such that when a query comes each operator is rewrited based on its matched rule to achieve the goal of annotating and propagating. The rules are shown in Fig.~\ref{fig:cap-rules}. 

\begin{figure}[H]
%\begin{table}%[h!]
\centering
 \begin{adjustbox}{max width=1\linewidth}
 \begin{tabular}{|c|c|c|} 
 \hline
 \rowcolor{lightgray}
 Rule & Op & Propagation rules \\ [0.5ex] 
 \hline \hline
 %$r_1$ & $R$ & $ R \rightarrow \projection_{\schema{R}, case \cdots when \cdots \rightarrow prov } (R) $ \\
 $r_0$ & $R$ & $\propagate{R} = \initialize{R}$  \\ 
 $r_1$ & $\projection_{A}(Q)$& $\propagate{\projection_{A}(Q)} = \projection_{A, ps}(\propagate{Q}) $ \\  [0.3ex]
  $r_2$ & $\selection(Q)$& $\propagate{\selection(Q)} = \selection(\propagate{Q}) $ \\
 %$r_2$ & $\selection(Q)$& $\propagate{\selection(Q)} = \selection(\propagate{Q})[\schema{\selection(Q)},ps] $ \\
 $r_3$ & $_{G} \aggregation _{F(a)}(Q) $ &$ \propagate{_{G} \aggregation _{F(a)}(Q)} = _{G} \aggregation _{F(a),bit\_or(ps)}(\propagate{Q})$  \\ [0.3ex]
 $r_4$ & $Q_1 \crossprod Q_2$ & $ \propagate{Q_1 \crossprod Q_2} = \propagate{Q_1} \crossprod \propagate{Q_2}$ \\
 $r_5$ & \propagate{$\rootOp(Q)}$ & $\propagate{\rootOp(Q)} \rightarrow  \aggregation _{bit\_or(ps) \rightarrow ps}  (\propagate{\rootOp(Q)})$\\[1ex] 
 \hline
 \end{tabular}
  \end{adjustbox}
    \caption{Instrumentation rules}
   \label{fig:cap-rules}
% \end{table}
 \end{figure}

%
%When a query comes, we apply each rule for this query through a bottom-up traversal of the relational algebra tree of this query. $r_1$ in Fig.~\ref{fig:cap-rules} is used to annotate each tuple with its partition, i.e., once a table access operator comes, we add a projection on top and use \emph{case ... when} clause to annotate each tuple with a bit vector which represents this tuple is in which partition. For example, given a table $R$ with schema $\{A,B\}$, we divide $R$ into four partitions on the values of column A and the partitions are [1,10), [10,16), [16,30), [30,37), then $R$ will be rewrited to: 
%
%\lstset{tabsize=4,style=psqlcolor,basicstyle=\scriptsize\upshape\ttfamily}
%\begin{lstlisting}
%    SELECT  A, B, 
%    				 CASE WHEN  A >= 1  AND A < 10 THEN '1000'
%    				 		  WHEN  A >= 10 AND A < 16 THEN '0100'
%    				 		  WHEN  A >= 16 AND A < 30 THEN '0010'
%    				 		  WHEN  A >= 30 AND A < 37 THEN '0001' 
%    				 END AS PROV
%    FROM  R 
%\end{lstlisting}

We apply the rules through a bottom-up traversal of relational algebra tree of the query. $R_0$ is the base rule to initialize the table R by adding additional column to store the annotations which is introduced in Sec.~\ref{tab:annotate}. For projection we only need to add the ps column into the schema propagated through its child operator ($r_1$). Similar with projection, we only need to adapt the schema of the selection to its child operator ($r_2$). Aggregation operator aggregates the  tuples in the same group such that the annotations in the same group should also be combined together, i.e.,`1000' and `0010' should be combined to `1010', since we need to know the fragments used per group. This is implemented by using a bitwise or operation on fragments and then adding this operation into the schema of the aggregation as an additional aggregation function ($r_3$). For join we need to adapt its schema to its two children ($r_4$). Finally, we combine the values in each $ps$ column to construct the provenance sketch by adding an additional $bit\_or$ operation on top of the root opeartor (noted as $\rootOp$) since the result of the query might be not just one row and we want to use only one bit vector to represent the provenance sketch per table ($r_5$).

In next section we use one end-to-end example to show how does our provenacne sketch capture works. 
%During the process of capturing provenance sketch, we should follow some rules. Generally, here are three rules we can apply: \textbf{table access}, \textbf{aggregation}, and \textbf{others}. Below table \ref{tab:PS_Cap_Rule} shows the rules with their definitions.
%Before talking about the rules, first comes the inputs for each ps capture. Recall that the provenance sketch is the information about fragments that contains results to answer a query. For a query, we should know which attributes from which tables can build the result set based on what kind of partition. So, it is obvious that the input for capturing the provenance sketch is: \textbf{tables}, \textbf{attributes} of table(s) and the \textbf{partitions}.
%Rule 1 shows how to apply to get provenance sketch for table access operator. 
%Rule 2 is applied when there come aggregation operators.
%Rule 3 is for all other operators like \textbf{join, selection, $\cdots$} except table access and aggregation.

\subsection{Provenance Sketch Capture Example}
\label{tab:example_capture}
Now let us see one example of how do we capture provenance sketch of the query. Given a salary table which records teacher id (\emph{tid}), teacher's salary (\emph{salary}) and his/her department number (\emph{depid}) (The table is shown in Fig.~\ref{tab:cp-eg-input}), now we want to know the average salary per department and list the top 2 by using the query Q which is shown in Fig.~\ref{fig:eg-q}. Afterwards, we do annotation initialization and propagation for this query and generates the new query $Q^{capture}$ shown in Fig.~\ref{fig:eg-q-capture}. Assume we %want to partition the table to four fragments on depid column, we first ask the database statistics to generate the histogram, here from the histogram we get the four partitions [1,2), [2,4), [4,5) and [5,6), each contains two tuples (See Fig.~\ref{fig:eg-capture}, the partitions 
use range partition to divide the salaries table to four fragments $f_1$, $f_2$, $f_3$ and $f_4$ and then do a bottom-up traversal of the relational algebra tree of the query.  We first find the salaries table and initialize it by addting the $case ... when$ clause to create the new column $ps_{salaries}$ to store the annotation for each tuple. Since we use range partition, then the process is shown in \fignumref{4} of Fig.~\ref{fig:eg-q-capture} and the generated annotations are shown under the $ps_{salaries}$ column of Fig.~\ref{tab:cp-eg-input}.  Next, we reach the aggregation operator, to propagate the values in $ps_{salaries}$ column over aggregation operator, we apply propagation rule $r_3$ which adds the $bit\_or$ function in the schema to do bitwise or operation for the values under  $ps_{salaries}$ column per group. See \fignumref{3} in Fig.~\ref{fig:eg-q-capture} for this process and the propagated annotations are shown in Fig.~\ref{tab:cp-eg-result1}. Next is selection operator  with order by and rule $r_2$ is applied for it by adding the additional column $ps_{salaries}$ in the schema. See \fignumref{2} in Fig.~\ref{fig:eg-q-capture} for this process and the result is shown in Fig.~\ref{tab:cp-eg-result2}. Finally, we reach the top of the query and add the final $bit\_or$ function on top to do bitwise or over the $ps_{salaries}$ column which is shown in \fignumref{1} in Fig.~\ref{fig:eg-q-capture}  and the provenance sketch we get at last is shown in Fig.~\ref{tab:cp-eg-result} which indicates which fragments of table salaries are used to answer this query Q.

\begin{figure}[t]
%\captionsetup[subfigure]{justification=centering,singlelinecheck=off}
\begin{minipage}{0.45\linewidth}
\begin{minipage}{1\linewidth}
   \begin{subfigure}{1\linewidth}
   \resizebox{0.95\textwidth}{!}{
\begin{tabular}{c|c|c|c|c} \hhline{~|-|-|-|}
 & \cthead tid & \cthead salary & \cthead depid & \color{dgrey}{$ps_{salaries}$} \\  
\color{LGreen}{$f_1$}  & 1 & 4800 & \gcell{1}  &\color{dgrey}{1000} \\  
& 2	& 5000 &  \gcell{1} &  \color{dgrey}{1000}\\   \hhline{~|-|-|-|}
\color{selectiveyellow}{$f_2$} & 3	&  6800 & \ycell{2} &\color{dgrey}{0100}\\ 
& 4 &  7200 & \ycell{2} &\color{dgrey}{0100} \\  \hhline{~|-|-|-|}
\color{LRed}{$f_3$} & 5 &   5400 & \rcell{4} &  \color{dgrey}{0010}\\
& 6 & 7000 & \rcell{4} &\color{dgrey}{0010}\\ \hhline{~|-|-|-|}
\color{LightBlue}{$f_4$} & 7 & 6800 & \bcell{5} &\color{dgrey}{0001}\\
& 8 & 6600 & \bcell{5} &\color{dgrey}{0001}\\
\hhline{~|-|-|-|}
\end{tabular} }
   	\caption{salaries + \fignumref{4} result}
     \label{tab:cp-eg-input}
   \end{subfigure}
\end{minipage} 
%%%%%%%%%%%%%%%%%%%
\begin{minipage}{1\linewidth}
   \begin{subfigure}{1\linewidth}
   \centering
         \resizebox{0.5\textwidth}{!}{
\begin{tabular}{|c|c|}  \hline
\cthead $ps_{salaries}$ &  0101 \\ 
 \hline
\end{tabular} }
     \caption{\fignumref{1} result}
     \label{tab:cp-eg-result}
   \end{subfigure}
\end{minipage}
\end{minipage}
%%%%%%%%%%%%%%%%%%%%1
\begin{minipage}{0.45\linewidth}
\begin{minipage}{1\linewidth}
   \begin{subfigure}{1\linewidth}
   \centering
      \resizebox{0.7\textwidth}{!}{
\begin{tabular}{|c|c|c|}  \hline
\cthead salary & \cthead depid & \cthead $ps_{salaries}$ \\  
  4900 & 1 & 1000 \\
  7000 & 2 & 0100 \\
  6200 & 4 & 0010 \\
  6700 & 5 & 0001 \\ \hline
\end{tabular} }
     \caption{\fignumref{3} result}
     \label{tab:cp-eg-result1}
   \end{subfigure}
\end{minipage}
%%%%%%%%%%%%%%%%%%%
\begin{minipage}{1\linewidth}
   \begin{subfigure}{1\linewidth}
   \centering
         \resizebox{0.7\textwidth}{!}{
\begin{tabular}{|c|c|c|}  \hline
\cthead salary & \cthead depid & \cthead $ps_{salaries}$ \\  
  7000 & 2 & 0100 \\
  6700 & 5 & 0001 \\ \hline
\end{tabular} }
     \caption{\fignumref{2} result}
     \label{tab:cp-eg-result2}
   \end{subfigure}
\end{minipage}
%%%%%%%%%%%%%%%%
\end{minipage}
\caption{Example Inputs and Outputs}
\label{fig:eg-capture}
\end{figure}

\begin{figure}[t]
\begin{tabular}{c}
\lstset{tabsize=4,style=psqlcolor,basicstyle=\scriptsize\upshape\ttfamily}
\begin{lstlisting}
SELECT avg(salary) AS avg_salary, depid 
FROM salaries 
GROUP BY depid
ORDER BY avg_salary desc
LIMIT 2;
\end{lstlisting}
\end{tabular}
\caption{Example Query Q}
\label{fig:eg-q}
\end{figure}
%
%\lstset{tabsize=4,style=psqlcolor,basicstyle=\scriptsize\upshape\ttfamily}
%\begin{lstlisting}
%SELECT bit_or(prov) AS prov 
%FROM (
%	SELECT avg(salary) AS avg_salary, 
%				 bit_or(prov) AS prov, 
%				 depid 
%	FROM (
%		SELECT tid, salary, depid, 
%					 CASE  WHEN  depid >= 1 AND depid < 2 THEN '1000'
%					 			 WHEN  depid >= 2 AND depid < 4 THEN '0100'
%					 			 WHEN  depid >= 4 AND depid < 5 THEN '0010'
%					 			 WHEN  depid >= 5 AND depid < 6 THEN '0001'  
%					 			 AS prov
%    		FROM salaries) p1
%	GROUP BY depid
%	ORDER BY avg_salary
%	LIMIT 2) p2;
%\end{lstlisting}

\begin{figure}[t]
\begin{adjustbox}{max width=1\linewidth}
\begin{tabular}{clc}   
\cellcolor{white} \fignumref{1} &
\begin{lstlisting}
SELECT bit_or($ps_{salaries}$) AS $ps_{salaries}$               
FROM (
\end{lstlisting} 
%%%%%%%%%%%%%%%%%%%
& \cellcolor{white} \large \textbf{Prop $r_5$} \\  
\cellcolor{lllgrey} \fignumref{3} &
\cellcolor{lllgrey}
\begin{lstlisting}
	SELECT avg(salary) AS avg_salary, 
				 bit_or($ps_{salaries}$) AS $ps_{salaries}$, 
				 depid 
	FROM (
\end{lstlisting}
&  \cellcolor{lllgrey}  \large \textbf{Prop $r_3$} \\  
%%%%%%%%%%%%%%%%%%%%%%%%%%%%%
\cellcolor{llgrey} \fignumref{4} & \cellcolor{llgrey}
\begin{lstlisting}
		SELECT tid, salary, depid, 
					 CASE  WHEN  depid >= 1 AND depid < 2 THEN '1000'
					 			 WHEN  depid >= 2 AND depid < 4 THEN '0100'
					 			 WHEN  depid >= 4 AND depid < 5 THEN '0010'
					 			 WHEN  depid >= 5 AND depid < 6 THEN '0001'  
					 			 AS $ps_{salaries}$
    		FROM salaries
\end{lstlisting}
&  \cellcolor{llgrey}  \large \textbf{Init} \\   
%%%%%%%%%%%%%%%%%%%%%%%%%%%%%
\cellcolor{lllgrey} \fignumref{3} &
\cellcolor{lllgrey}
\begin{lstlisting}
    		) p1
	GROUP BY depid
\end{lstlisting}
&   \cellcolor{lllgrey}  \large \textbf{Prop $r_3$} \\   
%%%%%%%%%%%%%%%%%%%%%%%%%%%%%
\cellcolor{white} \fignumref{2} &
\begin{lstlisting}
	ORDER BY avg_salary desc
	LIMIT 2
\end{lstlisting}
&  \cellcolor{white}  \large \textbf{Prop $r_2$} \\ 
%%%%%%%%%%%%%%%%%%%%%%%%%%%%%
\cellcolor{white} \fignumref{1} &
\begin{lstlisting}
	) p2;
\end{lstlisting}
&  \cellcolor{white}  \large \textbf{Prop $r_5$} \\ 
\end{tabular} 
\end{adjustbox}
\caption{Instrumented Query $Q^{capture}$}
\label{fig:eg-q-capture}
\end{figure}

\subsection{Optimization}
\label{tab:opt_capture}
We do some optimization to reduce the overhead of our apporach. Compared with orignal query, overhead can only be added when we do annotation initialization and propagation through aggregation operator. For the first one, since it might result to a large number of cases in \emph{case when}  clause when we partition the table to a large number of fragments.  The linear scan of the large emph{case when} clause for each tuple would increase the overhead especially for the huge table, the cost would be highly increased. To optimize it, we implement binary search for it through the user defined c function. For the second one, we optimized the existing $bit\_or$ function by removing some unnecessary copys by directly doing bitwise or for destination object. At the same time, we reduce the cost of for loop by doing bitwise or per word one time instead of per bit one time. By applying our optimization, the overhead is highly reduced escepially when partition the table to large number of fragments. 

%
%\begin{minipage}{0.9\linewidth}
%\captionsetup{singlelinecheck = false, justification=justified}
%\lstset{upquote=true,frame=single, title = \bf{Q-4}}
%\begin{lstlisting}
%SELECT *
%FROM r
%WHERE B > 10
%\end{lstlisting}
%\end{minipage}
%
%
%Example 2 (Q-5):  return all tuples with attribute B greater than 20 based on relation r in Figure \ref{fig:relation_cap}. This time, the result only contains two tuples: $t_5, t_6$, which locate in $f_3$. The bit representation is $001$.
%
%\begin{minipage}{0.9\linewidth}
%\captionsetup{singlelinecheck = false, justification=justified}
%\lstset{upquote=true,frame=single, title = \bf{Q-5}}
%\begin{lstlisting}
%SELECT *
%FROM r
%WHERE B > 20
%\end{lstlisting}
%\end{minipage}
%
%
%
%\begin{figure}[h]
%\centering
%\begin{minipage}{0.45\linewidth}  
%\centering
%\begin{tabular}{c|c|c|c} \hhline{~|-|-|}
% & \cthead A & \cthead B  \\  
%\color{LGreen}{$f_1$}  & \gcell{1} & \gcell{1} &\color{black}{$t_1$} \\
%& \gcell{2}	& \gcell{17} &\color{black}{$t_2$}\\  
%\color{LRed}{$f_2$} & \rcell{7}	&  \rcell{0} &\color{black}{$t_3$}\\ 
%& \rcell{8}	&  \rcell{2} &\color{black}{$t_4$} \\ 
%$f_3$ & 4 & 13 &\color{black}{$t_5$}\\
%&5 & 26 &\color{black}{$t_6$}\\
%\hhline{~|-|-|}
%\end{tabular}
%\end{minipage}
%\caption{Dataset r with 3 fragments}
%\label{fig:relation_cap}
%\end{figure}
