# Supplementary material for: Provenance-based Data Skipping (TechReport)
Source: arXiv:2104.12815 source file (2021-05-27)
Supplement: Supplementary file 2 [file experiments_appendix.tex]

%%%%%%%%%%%%%%%%%%%%%%%%%%%%%%%%%%%%%%%%%%%%%%%%%%%%%%%%%%%%%%%%%%%%%%%%%%%%%%%%%%%
\clearpage
%%%%%%%%%%%%%%%%%%%%%%%%%%%%%%%%%%%%%%%%%%%%%%%%%%%%%%%%%%%%%%%%%%%%%%%%%%%%%%%%

\section{Experiments Appendix}
\label{sec:exp-appendix}

%old to appendix
%%%%%%%%%%%%%%%%%%%%%%%%%%%%%%%%%%%%%%%%%%
%
%
% tables for 1 gb (binary search or) and 10 gb(binary search)
%
%
%%%%%%%%%%%%%%%%%%%%%%%%%%%%%%%%%%%%%%%%%%%

%%1 gb binary search
\begin{table}[]
\begin{adjustbox}{max width=1\linewidth}
\begin{tabular}{|l|l|l|l|l|l|l|}
\hline

\rowcolor[HTML]{9B9B9B} 
{\color[HTML]{000000} } & {\color[HTML]{000000} PS32} & {\color[HTML]{000000} PS64} & {\color[HTML]{000000} PS400} & {\color[HTML]{000000} PS40000} & {\color[HTML]{000000} PS10000} & {\color[HTML]{000000} PS100000} \\ \hline
Q2  &      &      &       & 29      & 10      & 19       \\ \hline
Q3  & 2    & 2    & 2     & 2       & 2       & 3        \\ \hline
Q5  &      &      &       & 9       & 3       & 3        \\ \hline
Q7  &      &      &       & 4       & 2       & 2        \\ \hline
Q8  &      &      &       & 6       & 4       & 4        \\ \hline
Q10 & 5    & 3    & 2     & 2       & 2       & 8        \\ \hline
Q17 &      &      &       & 2       & 2       & 11       \\ \hline
Q18 & 6    & 5    & 2     & 2       & 2       & 10       \\ \hline
Q19 & 9    & 5    & 3     & 3       & 3       & 8        \\ \hline
Q20 &      &      &       & 3       & 4       & 13       \\ \hline
Q21 &      &      &       & 15      & 15      & 28      \\\hline
\end{tabular}
\end{adjustbox}
  \caption{binary search: Running times for Query with ps can beat normal 1GB}
	\label{tab:tpch-1g-binarysearch-times}
\end{table}

\begin{table}[]
\begin{adjustbox}{max width=1\linewidth}
\begin{tabular}{|l|l|l|l|l|l|l|l|}
\hline
\rowcolor[HTML]{9B9B9B}
{\color[HTML]{000000} } & {\color[HTML]{000000} Nor} & {\color[HTML]{000000} PS32} & {\color[HTML]{000000} PS64} & {\color[HTML]{000000} PS400} & {\color[HTML]{000000} PS40000} & {\color[HTML]{000000} PS10000} & {\color[HTML]{000000} PS100000} \\ \hline
Q2 & {[}1,10)  & &                             &                              &                                & {[}10,73)                      & {[}73, $\infty$)                     \\ \hline
Q3                      & {[}1,2)                    &                             &                             &                              & {[}2, $\infty$)                     &       -                         &            -                     \\ \hline
Q5                      & {[}1, 3)                   &                             &                             &                              &                                &                                & {[}3, $\infty$)                      \\ \hline
Q7                      & {[}1,2)                    &                             &                             &                              &                                &                                & {[}2, $\infty$)                      \\ \hline
Q8                      & {[}1, 4)                   &                             &                             &                              &                                & {[}4, 5)                       & {[}5, $\infty$)                      \\ \hline
Q10                     & {[}1,2)                    &                             &                             &                              & {[}2,46)                       & {[}46, 667)                    & {[}667, $\infty$)                    \\ \hline
Q17                     & {[}1, 2)                   &                             &                             &                              &                                & {[}2, 799)                     & {[}799, $\infty$)                    \\ \hline
Q18                     & {[}1, 2)                   &                             &                             &                              & {[}2, 3)                       & {[}3, 1968)                    & {[}1968, $\infty$)                   \\ \hline
Q19                     & {[}1, 3)                   &                             &                             &                              &                                & {[}3, 195)                     & {[}195, $\infty$)                    \\ \hline
Q20                     & {[}1, 3)                   &                             &                             &                              & {[}3, 11)                      & {[}11, 387)                    & {[}387, $\infty$)                    \\ \hline
Q21                     & {[}1, 15)                  &                             &                             &                              &                                & {[}15, 507)                    & {[}507, $\infty$)                    \\ \hline
\end{tabular}
\end{adjustbox}
\caption{Option for query with ps under different run times 1GB}
\label{tab:tpch_1gb_binarysearch_option}

\end{table}

%%1 gb or
\begin{table}[]
\begin{adjustbox}{max width=1\linewidth}
\begin{tabular}{|l|l|l|l|l|l|l|}
\hline
\rowcolor[HTML]{9B9B9B} 
{\color[HTML]{000000} } & {\color[HTML]{000000} PS32} & {\color[HTML]{000000} PS64} & {\color[HTML]{000000} PS400} & {\color[HTML]{000000} PS40000} & {\color[HTML]{000000} PS10000} & {\color[HTML]{000000} PS100000} \\ \hline
Q2  &      &      &2       & 2      & 2      & 4       \\ \hline
Q3  & 2    & 2    & 2     & 2       & 2       & 3        \\ \hline
Q10 & 4    & 3    & 2     & 2       & 2       & 7        \\ \hline
Q15 & 118     & 48     &2       & 2       & 2       & 2       \\ \hline
Q18 & 2    & 2    & 2     & 2       & 2       & 9       \\ \hline
Q19 &     & 3    & 2     & 2       & 2       & 5        \\ \hline
\end{tabular}
\end{adjustbox}
\caption{OR: Running times for Query with ps can beat normal 1GB}
\label{tab:tpch_1g_OR_times}

\end{table}

\begin{table}[]
\begin{adjustbox}{max width=1\linewidth}
\begin{tabular}{|l|l|l|l|l|l|l|l|}
\hline
\rowcolor[HTML]{9B9B9B}
{\color[HTML]{000000} } & {\color[HTML]{000000} Nor} & {\color[HTML]{000000} PS32} & {\color[HTML]{000000} PS64} & {\color[HTML]{000000} PS400} & {\color[HTML]{000000} PS40000} & {\color[HTML]{000000} PS10000} & {\color[HTML]{000000} PS100000} \\ \hline
Q2 & {[}1,2)  & &  &  &{[}2,4) & {[}5,941)  & {[}942, $\infty$) \\ \hline
Q3   & {[}1,2)   &  & & {[}2,3)  & {[3},272) & {[}273, 1364) &{[}1364, $\infty$) \\ \hline

Q10 & {[}1,2)  & & &{[}2, 5)  & {[}5,9) & {[}9, 166) & {[}167, $\infty$)  \\ \hline
Q15  & {[}1, 2)  &  &  & & {[}2, 355)&  - & {[}355, $\infty$)    \\ \hline
Q18   & {[}1, 2) &    &   &   & {[}2, 5) & {[}5, 10111) & {[}10111, $\infty$)    \\ \hline
Q19   & {[}1, 3)  & &  &   & & {[}2, 122) & {[}122, $\infty$) \\ \hline

\end{tabular}
\end{adjustbox}
\caption{Option for query with ps under different run times:OR}
\label{tab:tpch_1gb_OR_option}

\end{table}

%10gb

\begin{table}[]
\begin{adjustbox}{max width=1\linewidth}
\begin{tabular}{|l|l|l|l|l|l|l|}
\hline
\rowcolor[HTML]{9B9B9B} 
{\color[HTML]{000000} } & {\color[HTML]{000000} PS32} & {\color[HTML]{000000} PS64} & {\color[HTML]{000000} PS400} & {\color[HTML]{000000} PS40000} & {\color[HTML]{000000} PS10000} & {\color[HTML]{000000} PS100000} \\ \hline
Q2         &3 &3 &3  &3 &3  &10 \\ \hline
Q3         &2        & 2         &2        & 2        & 2        & 4 \\ \hline
Q10        &44         &5       &  2         &2        & 2        & 8\\ \hline
Q18       &-       &-       &-        &2       &  2     &  -\\ \hline
Q19      &-      & -     &  -         &7       &  7        & 7\\ \hline
Q20      & -      & -     & -        & 5        & 5      & 131\\ \hline
Q21       &-      & -     & -      &  6         &6      & -\\ \hline
\end{tabular}
\end{adjustbox}
\caption{Binary search: Running times for Query with ps can beat normal 10GB}
\label{tab:tpch_10g_binarysearch_times(cishu)}

\end{table}

\begin{table}[]
\begin{adjustbox}{max width=1\linewidth}
\begin{tabular}{|l|l|l|l|l|l|l|l|}
\hline
\rowcolor[HTML]{9B9B9B}
{\color[HTML]{000000} } & {\color[HTML]{000000} Nor} & {\color[HTML]{000000} PS32} & {\color[HTML]{000000} PS64} & {\color[HTML]{000000} PS400} & {\color[HTML]{000000} PS40000} & {\color[HTML]{000000} PS10000} & {\color[HTML]{000000} PS100000} \\ \hline
Q2 & {[}1,3)  & &  &  &{[}3,6) & {[}6,215)  & {[}215, $\infty$) \\ \hline
Q3   & {[}1,2)   &  & && {[}2,17)  & {[}17,1629)  &{[}1629, $\infty$) \\ \hline

Q10 & {[}1,2)  & & & &{[}2, 3)  & {[}3,462) & {[}462, $\infty$)  \\ \hline

Q18   & {[}1, 2) &    &   &  & & {[}2, $\infty$) &  - \\ \hline
Q19   & {[}1, 7)  & &  &   & & {[}7, 8) & {[}8, $\infty$) \\ \hline
Q20  & {[}1, 5)  &  &  & & {[}5, 8) & {[}8, 540) & {[}540, $\infty$) \\ \hline
Q21 & {[}1, 6)  &  &  & & {[}6, 26)& {[}26, $\infty$) & -    \\ \hline

\end{tabular}
\end{adjustbox}
\caption{Option for query with ps under different run times:OR 10GB}
\label{tab:tpch_10gb_binary_search_option}
\end{table}

\begin{figure}
\centering
 \begin{adjustbox}{max width=1\linewidth}
\begin{tabular}{|c|c|r|r|r|r|r|r|} \hline
\cthead Query  & \cthead Table   &  \cthead PS32   & \cthead PS64  &  \cthead PS400   &  \cthead PS4000 &  \cthead PS10000    &  \cthead PS100000  \\ \hline
   \multirow{3}{*}{Q2}  &  partsupp  & 96.88\%  & 81.25\% & 22.75\% & 2.48\% & 0.95\%& 0.10\%    \\ 
       & part  & 93.75\%  & 81.25\%  & 22.75\%   &  2.48\% & 0.99\%& 0.10\%\\ 
       & supplier & 93.75\% & 73.44\% & 19.75\%   &   2.23\% & 0.89\%& 0.09\% \\ \hline   \yellowrow  
      & customer  & 25.00\%  & 14.06\% & 2.50\% & 0.25\% & 0.10\%& 0.01\%    \\   \yellowrow  
  & orders   & 28.13\%  & 15.63\% & 2.50\% & 0.25\% & 0.10\%& 0.01\%\\ 
        \yellowrow      
 \multirow{-3}{*}{Q3}      & lineitem  & 28.13\%  & 15.63\% & 2.50\% & 0.25\% & 0.10\%& 0.01\%\\ \hline
 \multirow{2}{*}{Q5} & orders  & 100.00\%  & 100.00\% & 100.00\% & 81.55\% & 48.90\%& 6.46\%    \\ 
   & customer  & 100.00\%  & 100.00\% & 100.00\% & 76.50\% & 43.40\%& 5.40\%\\ \hline     \yellowrow   
 & orders  & 100.00\%  & 100.00\% & 100.00\% & 74.70\% & 42.42\%& 5.34\%    \\ 
    \yellowrow     
 \multirow{-2}{*}{Q7}  & customer  & 100.00\%  & 100.00\% & 100.00\% & 64.55\% & 33.06\%& 3.80\%\\ \hline    
 \multirow{1}{*}{Q8} & lineitem  & 100.00\%  & 100.00\% & 100.00\% & 47.20\% & 22.62\%& 2.53\%    \\ \hline  \yellowrow   
  &  lineitem  & 87.50\%  & 57.81\% & 16.75\% & 1.75\% & 0.71\%& 0.07\%    \\   \yellowrow   
       & orders & 87.50\%  & 57.81\% & 17.00\% & 1.78\% & 0.71\%& 0.07\%\\ 
     \yellowrow   
  \multirow{-3}{*}{Q10}   & customer & 46.88\% & 28.13\% & 5.00\% & 0.50\% & 0.20\%& 0.02\% \\ \hline
  \multirow{2}{*}{Q15} & lineitem  & 3.13\%  & 1.56\% & 0.25\% & 0.03\% & 0.01\%&0.01\%\\ 
   & supplier   & 3.13\%  & 1.56\% & 0.25\% & 0.03\% & 0.01\%& 0.01\% \\ \hline  \yellowrow   
 & lineitem  & 100.00\%  & 93.75\% & 38.75\% & 4.80\% & 1.95\%& 0.20\%    \\ 
  \yellowrow    
   \multirow{-2}{*}{Q17} & part  & 100.00\%  & 93.75\% & 39.00\% & 4.85\% & 1.97\%& 0.20\% \\ \hline
  \multirow{3}{*}{Q18} & lineitem  & 21.88\%  & 14.06\% & 2.50\% & 0.25\% & 0.10\%& 0.01\%    \\ 
   & orders  & 21.88\%  & 14.06\% & 2.50\% & 0.25\% & 0.10\%& 0.01\% \\ 
   & customer & 21.88\%  & 14.06\% & 2.50\% & 0.25\% & 0.10\%& 0.01\% \\ \hline \yellowrow  
& lineitem  & 96.88\%  & 84.38\% & 24.25\% & 3.00\% & 1.20\%& 0.12\%    \\ 
 \yellowrow    
   \multirow{-2}{*}{Q19}    & part  & 100.00\%  & 76.56\% & 22.25\% & 2.55\% & 1.02\%& 0.10\% \\ \hline
   \multirow{4}{*}{Q20} & lineitem  & 100.00\%  & 100.00\% & 100.00\% & 9.95\% & 4.10\%& 0.41\%    \\ 
   & part  & 100.00\%  & 100.00\% & 100.00\% & 6.03\% & 2.44\%& 0.25\% \\ 
    &  partsupp  & 100.00\%  & 100.00\% & 100.00\% & 5.93\% & 2.44\%& 0.23\% \\ 
     & supplier   & 100.00\%  & 100.00\% & 100.00\% & 4.88\% & 1.97\%&0.20\% \\ \hline   \yellowrow 
& lineitem  & 100.00\%  & 100.00\% & 100.00\% & 28.98\% & 12.90\%& 1.37\%    \\ 
  \yellowrow   \multirow{-2}{*}{Q21}   & supplier  & 100.00\%  & 100.00\% & 100.00\% & 2.50\% & 1.00\%& 0.10\% \\ \hline
\end{tabular}
\end{adjustbox}
  \caption{Selectivity-TPC-H-1GB}
  \label{fig:Selectivity-TPC-H-1GB}
\end{figure}
%%%%%%%%%%%%%%%%%%%%%%%%%%%%%%%%%%%%%%%%

%%%%%%%%%%%%%%%%%%%%%%%%%%%%%%%%%%%%%%%%
\begin{figure}[h]
\centering
\begin{tabular}{|c|c|c|c|c|} \cline{2-4}
\multicolumn{1}{c|}{} & \multicolumn{3}{c|}{\cthead Runtime (sec)} &        \multicolumn{1}{c}{}                           \\ \cline{1-1}
\cthead selectivity   & \cthead w/o \pbds                           & \cthead \pbds & \cthead acc. capture & \cthead \#reuse \\
60                    & 2850.45                                    & 231.97       & 230.27               & 981             \\
600                   & 2880.85                                    & 282.17       & 280.00               & 977             \\
10000                 & 2882.15                                    & 307.70       & 267.55               & 978             \\
1327622               & 2883.06                                    & 2884.23      & 274.09               & 979             \\ \hline
\end{tabular}
\caption{End-to-end results for a workloads of 1000 instances of query template $Q^{st}$. We vary the threshold for the upper range of the query's selection parameter with and w/o \pbds.}
\label{fig:self-tuning-result}
\end{figure}
%%%%%%%%%%%%%%%%%%%%%%%%%%%%%%%%%%%%%%%%

%%%%%%%%%%%%%%%%%%%%%%%%%%%%%%%%%%%%%%%%
\begin{figure}[h]
\centering
\begin{tabular}{|c|c|c|c|c|} \cline{2-4}
\multicolumn{1}{c|}{} & \multicolumn{3}{c|}{\cthead Runtime (sec)} &        \multicolumn{1}{c}{}                           \\ \cline{1-1}
\cthead selectivity   & \cthead w/o \pbds                           & \cthead \pbds & \cthead acc. capture & \cthead \#reuse \\
5\%                    & 2855.17                                    & 608.61       & 224.76              & 981             \\
10\%                    & 2849.51                                   & 867.81       & 257.17               & 978             \\
20\%                  & 2851.63                                    & 1121.98      & 189.22               & 984             \\
100\%                 & 2862.13                                    & 2764.02      & 189.39              & 984             \\ \hline
\end{tabular}
\caption{End-to-end results for a workloads of 1000 instances of query template $Q^{st}$. We vary the threshold for the upper range of the query's selection parameter with and w/o \pbds.}
\label{fig:self-tuning-result1}
\end{figure}
%%%%%%%%%%%%%%%%%%%%%%%%%%%%%%%%%%%%%%%%

%%%%%%%%%%%%% crimes ps size
\begin{figure}
\centering
   \begin{subfigure}{1\linewidth}
    \centering
 \begin{adjustbox}{max width=1\linewidth}
\begin{tabular}{|c|c|c|c|c|} \hline
\cthead Attribute & \cthead ND & \cthead NDP & \gycell PS & \cthead PR \\ \hline
 district         & 24         & 4           & 4          & 0.007\%    \\ \hline
community\_area   & 78         & 4           & 4          & 0.007\%    \\ \hline
ward              & 50         & 3           & 3          & 0.007\%    \\ \hline
beat              & 303        & 5           & 5          & 0.007\%    \\ \hline
\end{tabular}
\end{adjustbox}
   	\caption{C-Q1}
     \label{tab:cq1}
   \end{subfigure}
      \begin{subfigure}{1\linewidth}
    \centering
 \begin{adjustbox}{max width=1\linewidth}
\begin{tabular}{|c|c|c|c|c|} \hline
\cthead Attribute & \cthead ND & \cthead NDP & \gycell PS & \cthead PR \\ \hline
 district         & 24         & 2           & 2          & 0.01\%     \\ \hline
 community\_area  & 78         & 2           & 2          & 0.01\%     \\ \hline
 ward             & 50         & 2           & 2          & 0.01\%     \\ \hline
 beat             & 303        & 3           & 3          & 0.01\%     \\ \hline
\end{tabular}
\end{adjustbox}
   	\caption{C-Q2}
     \label{tab:cq2}
   \end{subfigure}
  \caption{Provenance and provenance sketch sizes (Crimes dataset)}
  \label{fig:crimes-size-post}
\end{figure}
%%%%%%%%%%%%%%%%%%%%%%%%%%%%%%%%%%%%%%%%%%%%%%%%%%%%%%%%%%%%%%%%

%%%%%%%%%%%%% movies ps size
\begin{figure}[t]
\centering
   \begin{subfigure}{1\linewidth}
    \centering
 \begin{adjustbox}{max width=1\linewidth}
\begin{tabular}{|c|c|c|c|c|c|c|c|} \hline
\cthead Table & \cthead Attribute & \cthead ND & \cthead NDP & \gycell PS32 & \gycell PS64 & \gycell PS400 & \cthead PR \\ \hline
 movies       & movieid           & 27.3k      & 10          & 2p           & 3p           & 8p            & 0.0004\%   \\ \hline
 ratings      & movieid           & 26.7k      & 10          & 6p           & 7p           & 9p            & 0.03\%     \\ \hline
\end{tabular}
\end{adjustbox}
   	\caption{M-Q1}
     \label{tab:mq1}
   \end{subfigure}
 %%%%%%%%%%%%%%%%%%%%%%%%%%%%%%%%%%%%%%%%%
  \begin{subfigure}{1\linewidth}
    \centering
 \begin{adjustbox}{max width=1\linewidth}
\begin{tabular}{|c|c|c|c|c|c|c|c|} \hline
\cthead Table & \cthead Attribute & \cthead ND & \cthead NDP & \gycell PS32 & \gycell PS64 & \gycell PS400 & \cthead PR \\ \hline
 movies       & movieid           & 27.3k      & 3           & 1p           & 1p           & 2p            & 0.0001\%   \\ \hline
 ratings      & movieid           & 26.7k      & 3           & 2p           & 2p           & 3p            & 0.01\%     \\ \hline
\end{tabular}
\end{adjustbox}
   	\caption{M-Q2}
     \label{tab:mq2}
   \end{subfigure}
   %%%%%%%%%%%%%%%%%%%%%%%%%%%%%%%%%%%%%%%%
    \begin{subfigure}{1\linewidth}
    \centering
 \begin{adjustbox}{max width=1\linewidth}
\begin{tabular}{|c|c|c|c|c|c|c|c|} \hline
\cthead Table & \cthead Attribute & \cthead ND & \cthead NDP & \gycell PS32 & \gycell PS64 & \gycell PS400 & \cthead PR \\ \hline
 movies       & movieid           & 27.3k      & 10          & 2p           & 3p           & 8p            & 0.0004\%   \\ \hline
 ratings      & movieid           & 26.7k      & 10          & 6p           & 7p           & 9p            & 0.03\%     \\ \hline
 tags         & movieid           & 19.5k      & 10          & 3p           & 4p           & 9p            & 0.02\%     \\ \hline
\end{tabular}
\end{adjustbox}
   	\caption{M-Q3}
     \label{tab:mq3}
   \end{subfigure}
  \caption{Provenance and provenance sketch sizes (Movies dataset)}
  \label{fig:movies-size-post}
\end{figure}
%%%%%%%%%%%%%%%%%%%%%%%%%%%%%%%%%%%%%%%%%%%%%%%%%%%%%%%%%%%%%%%%

%%%%%%%%%%%%%%%%%%%%%%%%%%%%%%%%%%%%%%%%
\begin{figure*}[t]
  \centering
  %%%%%%%%%%%%%%%%%%%% USAGE
  \begin{minipage}{1.0\linewidth}
    \centering
    \begin{subfigure}{0.78\linewidth}
      \includegraphics[width=1\linewidth,trim=0pt 0pt 0 0pt, clip]{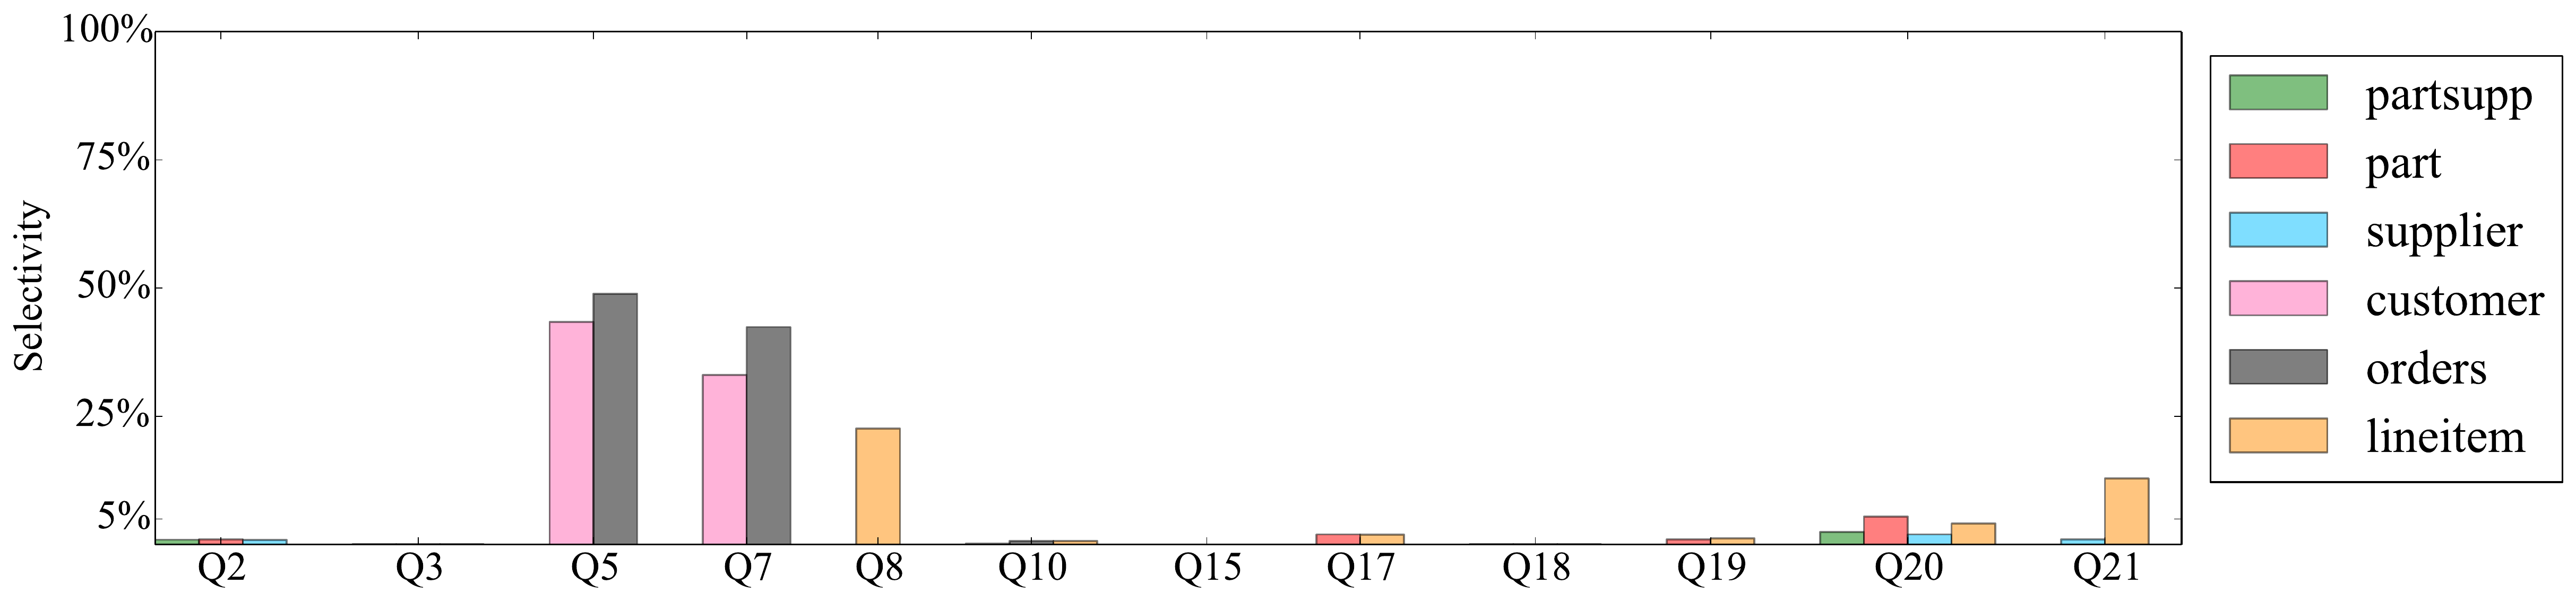}
      \caption{Selectivity - TPC-H - 1GB - PS10000}
      \label{fig:selectivity-tpch-post-1gb-ps10000}
    \end{subfigure}
    \begin{subfigure}{0.78\linewidth}
      \includegraphics[width=1\linewidth,trim=0pt 0pt 0 0pt, clip]{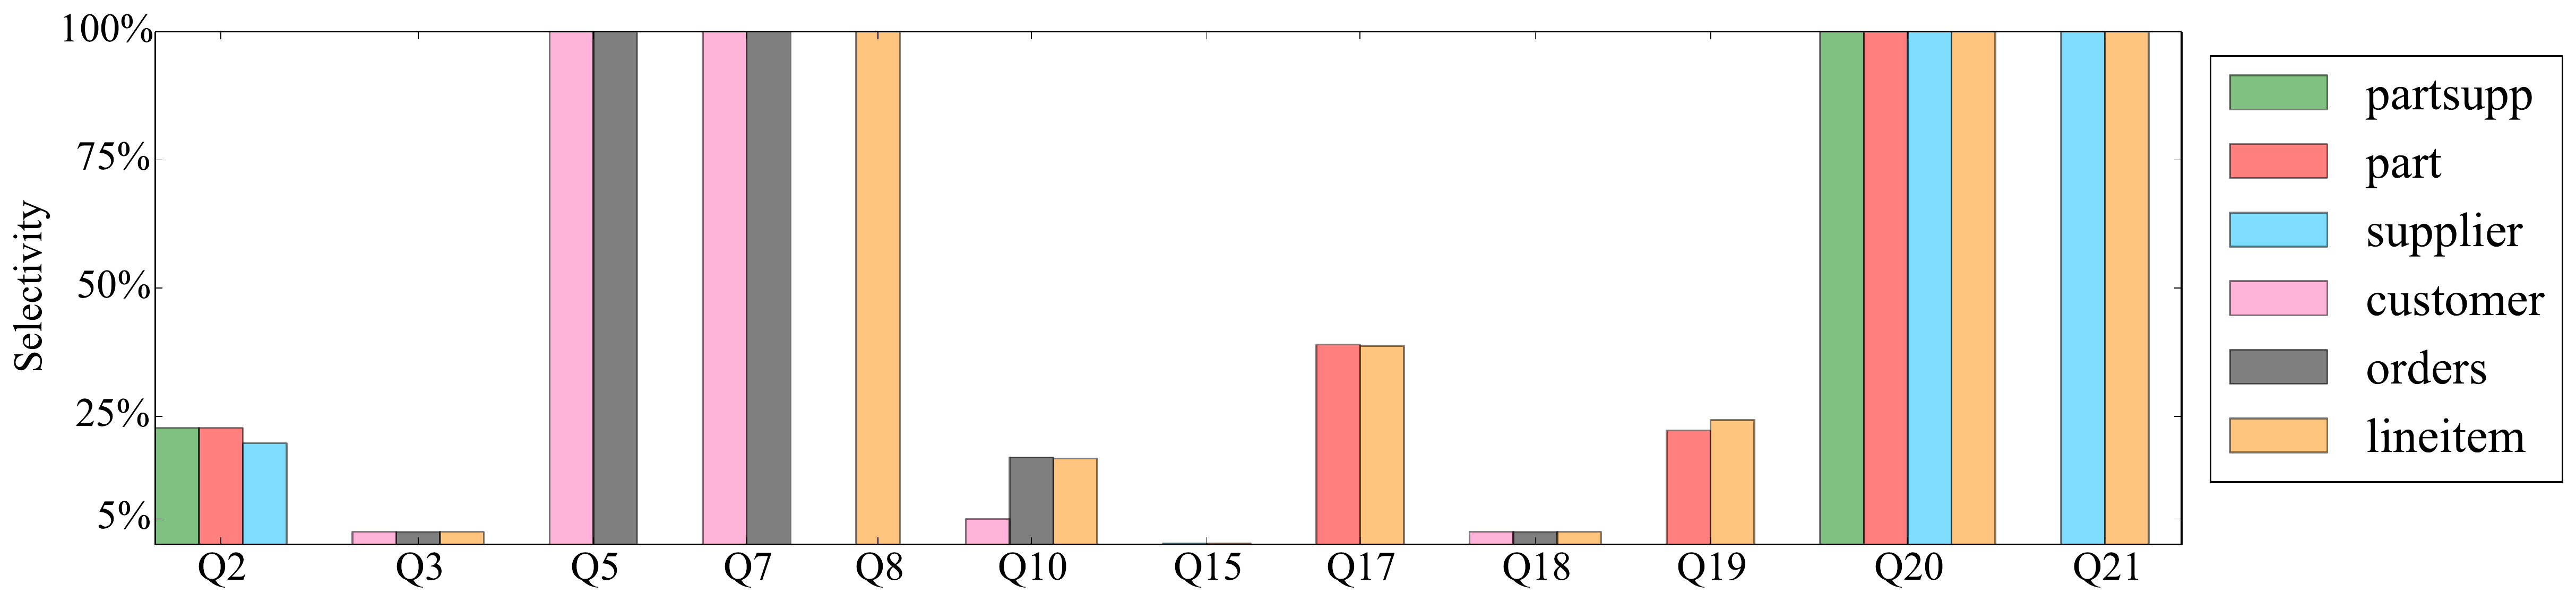}
      \caption{Selectivity - TPC-H - 1GB - PS400}
      \label{fig:selectivity-tpch-post-1gb-ps400}
    \end{subfigure}
    \begin{subfigure}{0.78\linewidth}
      \includegraphics[width=1\linewidth,trim=0pt 0pt 0 0pt, clip]{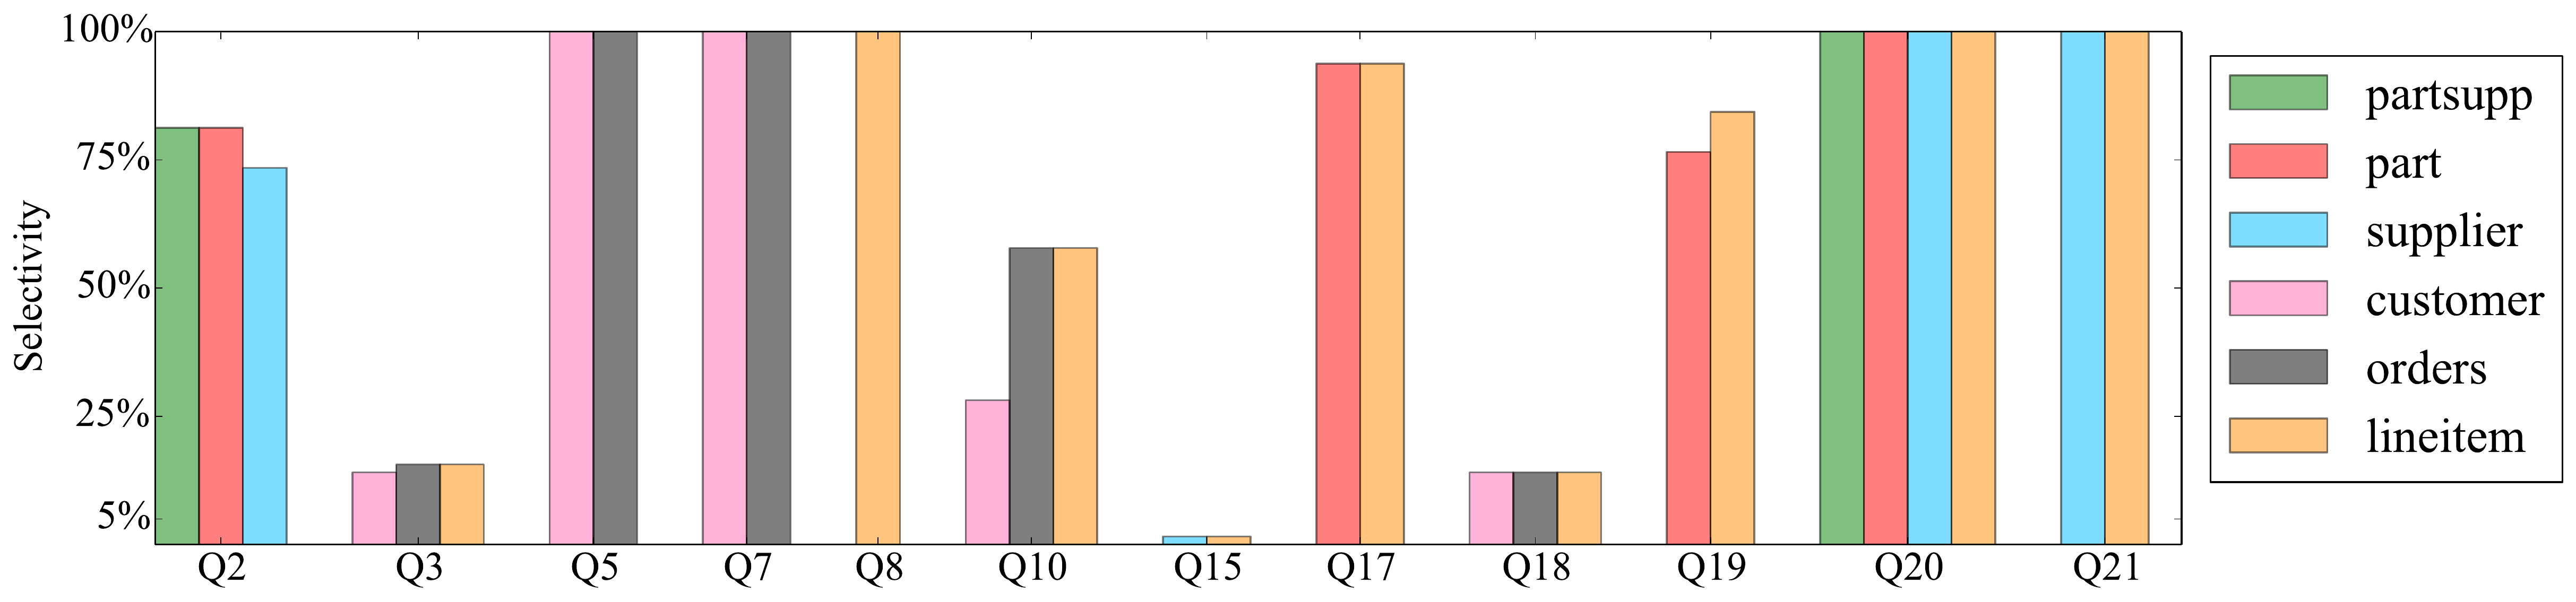}
      \caption{Selectivity - TPC-H - 1GB - PS64}
      \label{fig:selectivity-tpch-post-1gb-ps64}
    \end{subfigure}
       \begin{subfigure}{0.78\linewidth}
      \includegraphics[width=1\linewidth,trim=0pt 0pt 0 0pt, clip]{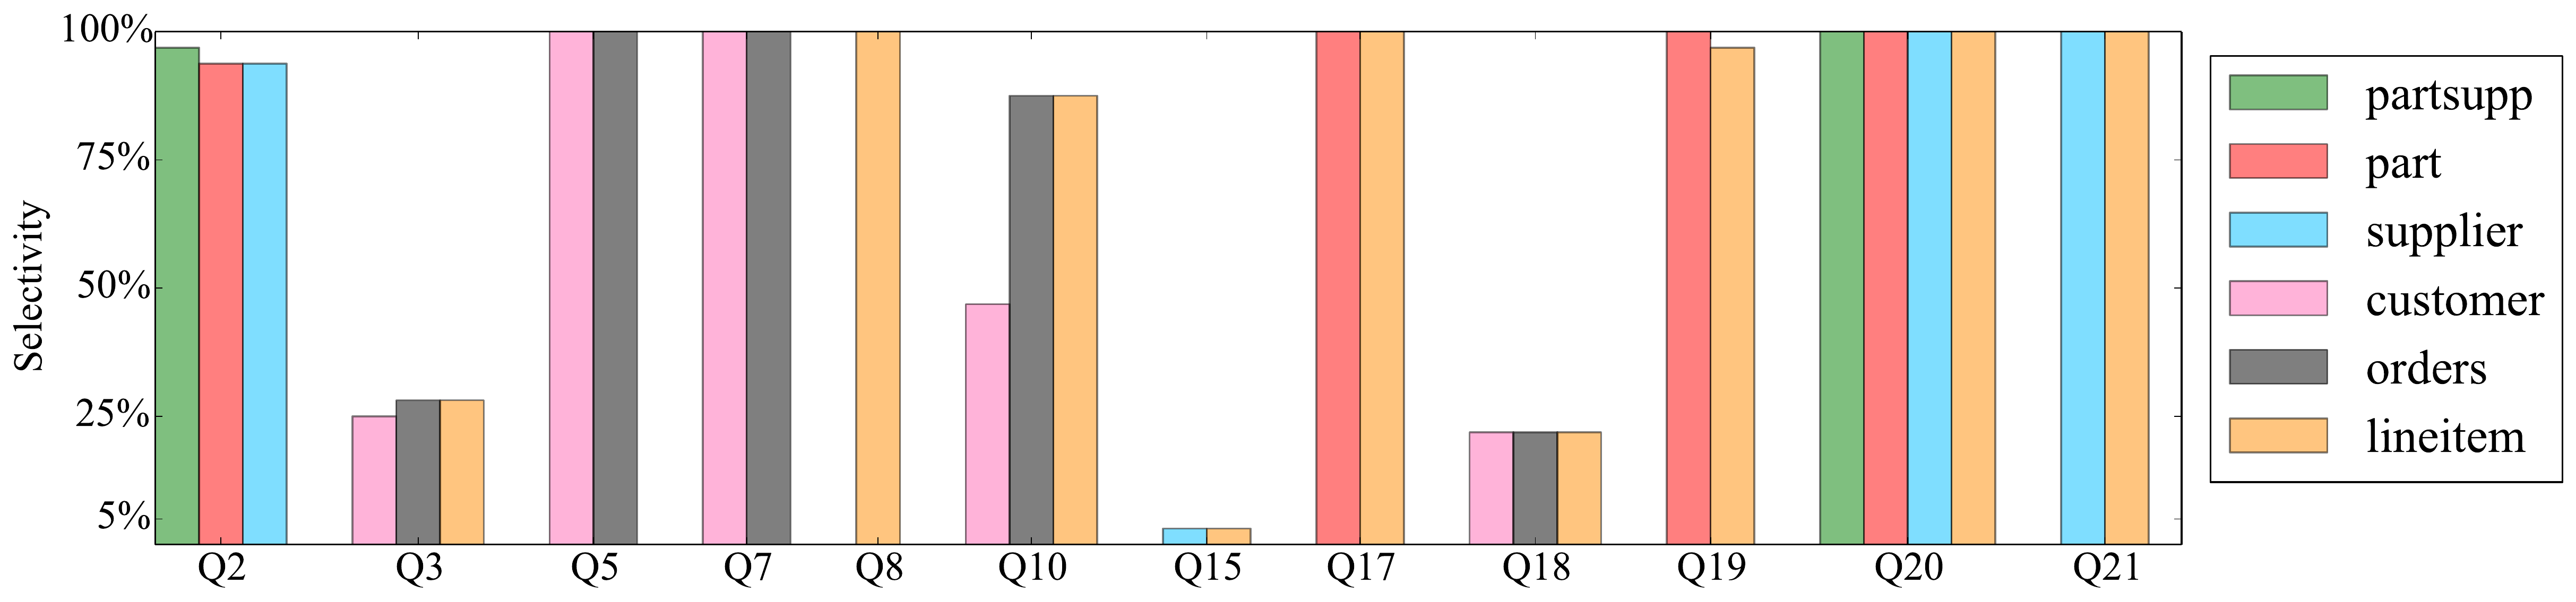}
      \caption{Selectivity - TPC-H - 1GB - PS32}
      \label{fig:selectivity-tpch-post-1gb-ps32}
    \end{subfigure}
    \caption{Selectivity - TPC-H  - 1GB}
    \label{fig:tpch-1gb-Selectivity}
  \end{minipage}
\end{figure*}
%%%%%%%%%%%%%%%%%%%%%%%%%%%%%%%%%%%%%%%%

%%%%%%%%%%%%%%%%%%%%%%%%%%%%%%%%%%%%%%%%
\begin{figure*}[t]
  \centering
  %%%%%%%%%%%%%%%%%%%% USAGE
  \begin{minipage}{1.0\linewidth}
    \centering
    \begin{subfigure}{0.78\linewidth}
      \includegraphics[width=1\linewidth,trim=0pt 0pt 0 0pt, clip]{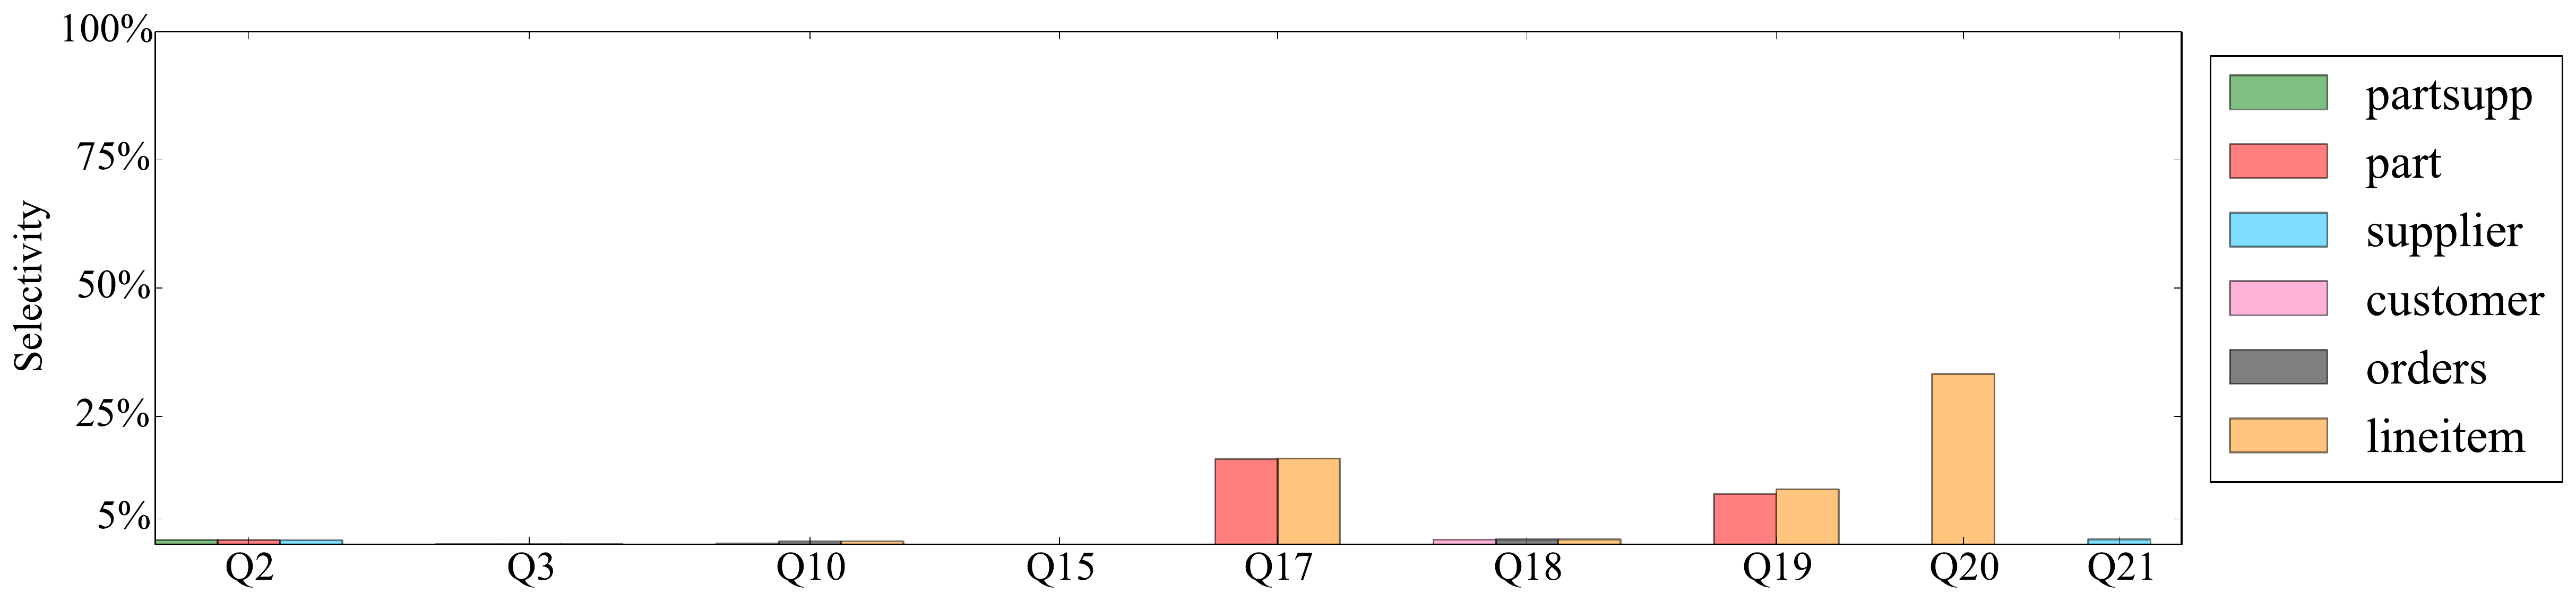}
      \caption{Selectivity - TPC-H - 10GB - PS10000}
      \label{fig:selectivity-tpch-post-1gb-ps10000}
    \end{subfigure}
    \begin{subfigure}{0.78\linewidth}
      \includegraphics[width=1\linewidth,trim=0pt 0pt 0 0pt, clip]{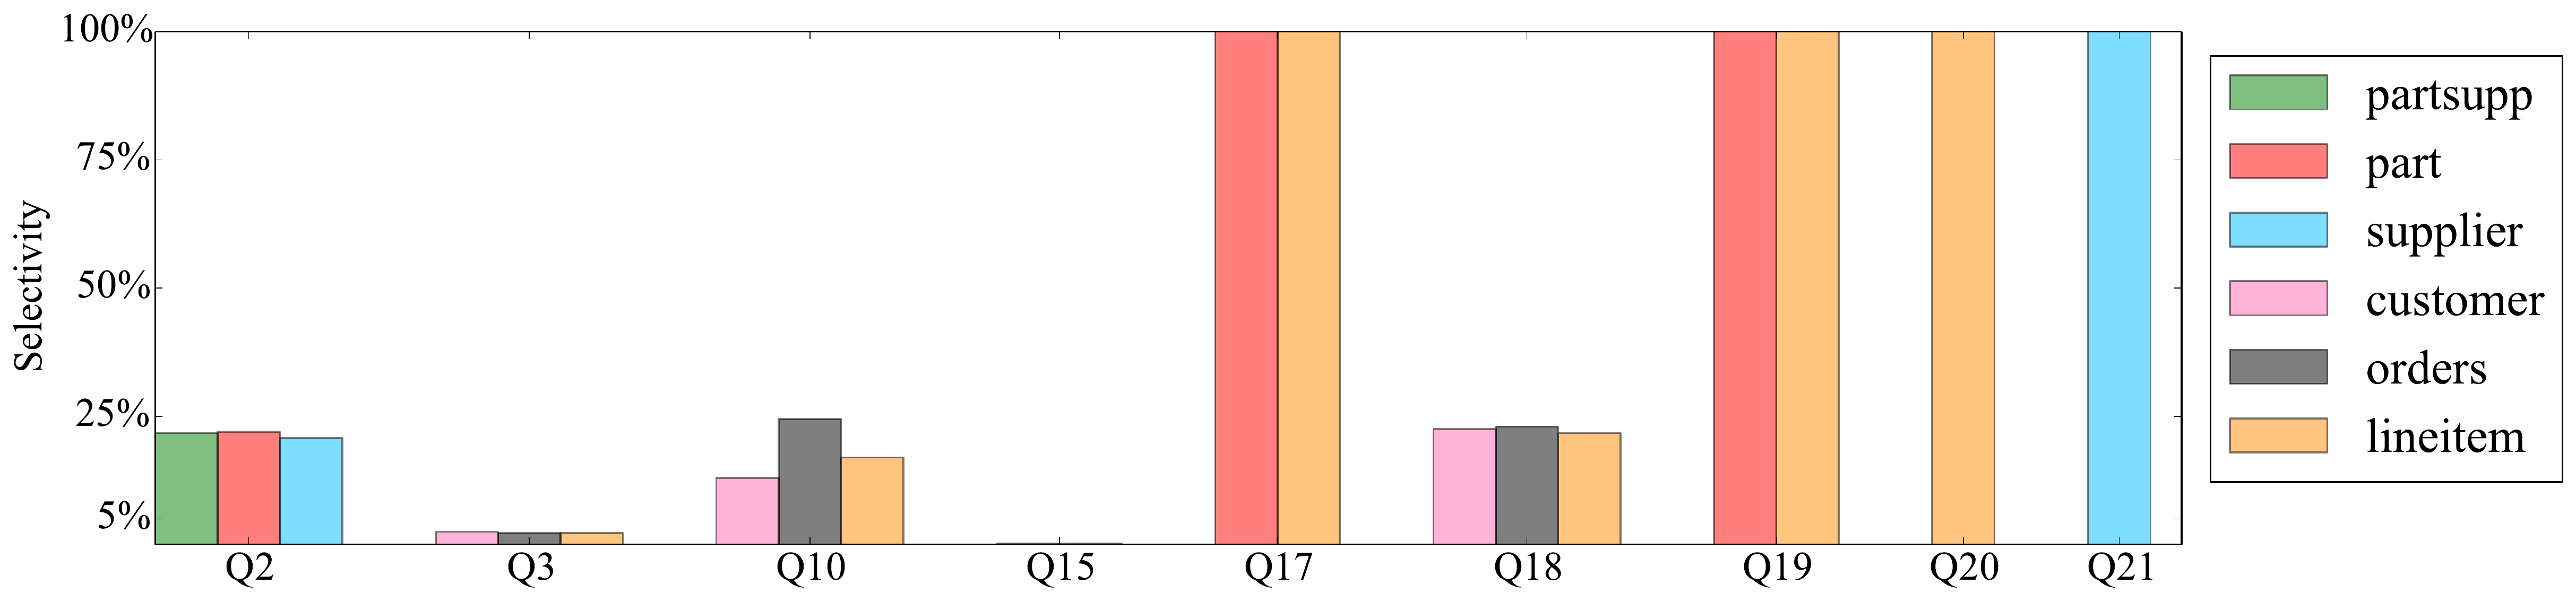}
      \caption{Selectivity - TPC-H - 10GB - PS400}
      \label{fig:selectivity-tpch-post-1gb-ps400}
    \end{subfigure}
    \begin{subfigure}{0.78\linewidth}
      \includegraphics[width=1\linewidth,trim=0pt 0pt 0 0pt, clip]{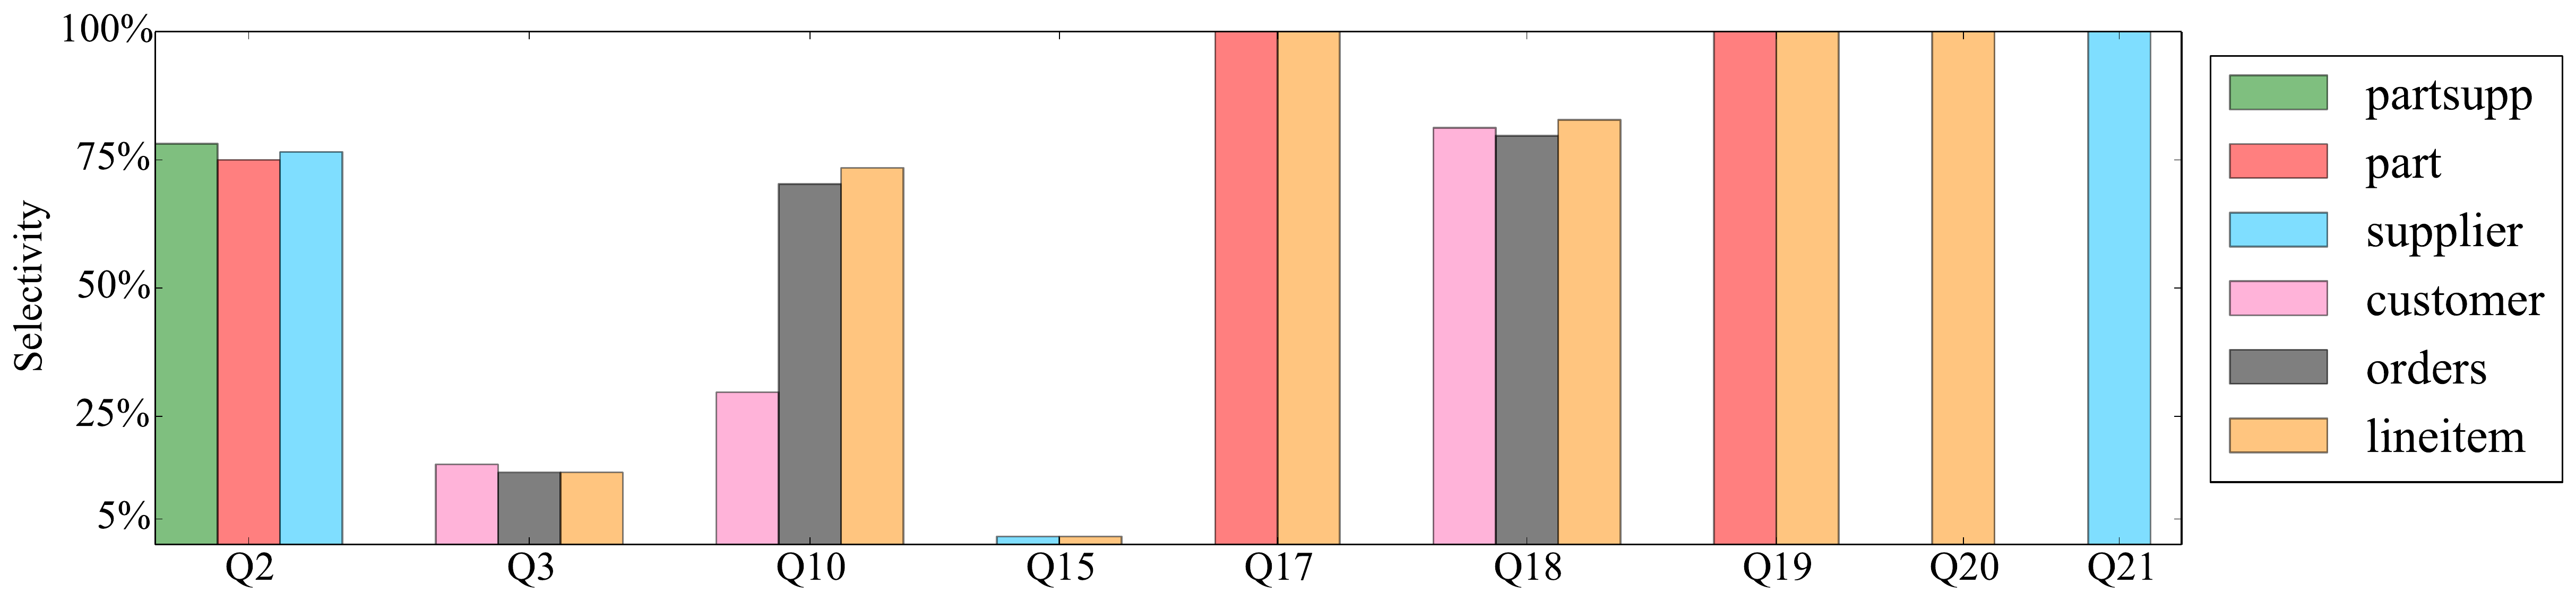}
      \caption{Selectivity - TPC-H - 10GB - PS64}
      \label{fig:selectivity-tpch-post-1gb-ps64}
    \end{subfigure}
       \begin{subfigure}{0.78\linewidth}
      \includegraphics[width=1\linewidth,trim=0pt 0pt 0 0pt, clip]{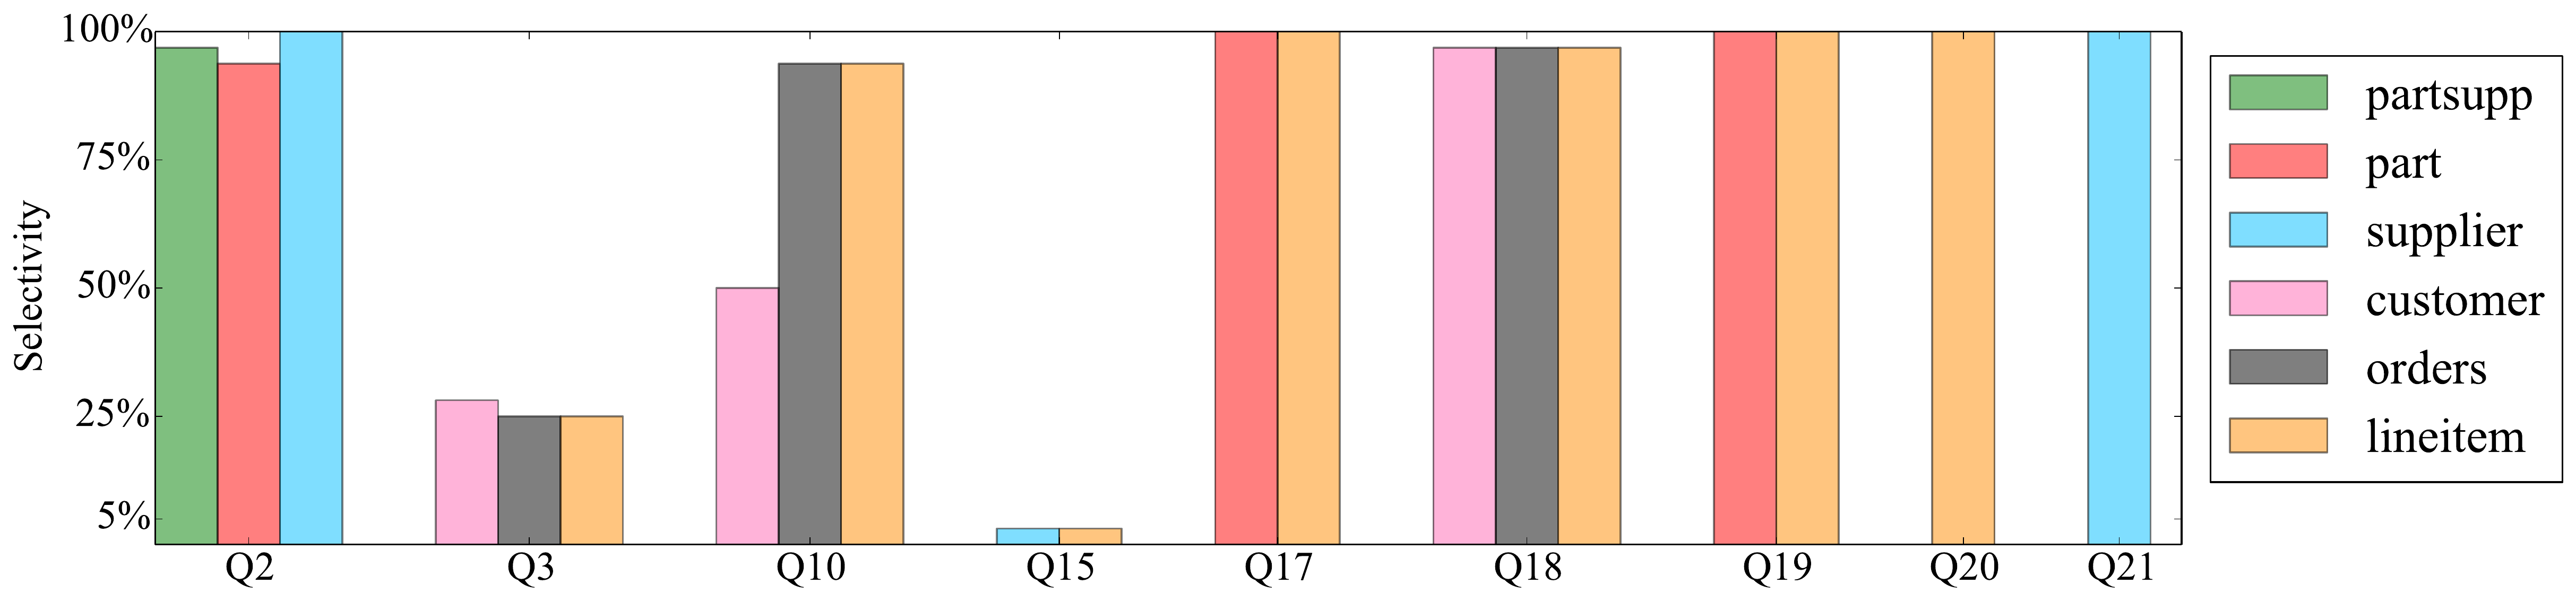}
      \caption{Selectivity - TPC-H - 10GB - PS32}
      \label{fig:selectivity-tpch-post-1gb-ps32}
    \end{subfigure}
    \caption{Selectivity - TPC-H  - 10GB}
    \label{fig:tpch-10gb-Selectivity}
  \end{minipage}
\end{figure*}

%%%%%%%%%%%%%%%%
\subsection{Performance}
\label{sec:ep-performance}
\BG{move to discussion of sketch effectiveness in one of the earlier sections.}
Before go through the experimental results, let us discuss when does the query could get benefit from the provenance sketch. Let us define following variables needed to evaluate the effectiveness of the provenance sketch.  \emph{numPart} : the number of partitions used for the provenance sketch, \emph{provRate} : the percentage of the provenance among the entire table, %\emph{numRes} : the number of tuples in the query result,
\emph{numDist(A)} : the number of distinct values of attribute A , \emph{numDistProv(A)} : the number of distinct values of attribute A in the provenance and  \emph{distRate(A)} : the ratio of the number of distinct values of attribute A in the provenance to the total number of distinct values. Assume A is the attribute in the schema of the table.

%tabsize=4, , xleftmargin=.15\textwidth
%\begin{lstlisting}[style=pseudocode, basicstyle=\scriptsize\upshape\ttfamily,xleftmargin=.02\textwidth ]
%if (provRate $\approx$ 1)							       	(case 1)
%	No
%else
%	if (numRes < numPart)
%		if (exists A and distRate(A) < 1)      (case 2)
%			Yes
%		else												(case 3)
%			No
%	else
%		if (exists A and numDist(A) < numPart) (case 4)
%			Yes
%		else 				      					   (case 5)
%			No
%\end{lstlisting}
%%%%%%%%%%%%%%%%%%%%%%%
%provRate $\approx$ 1 represents provenance accounts for almost the whole input table, e.g, $provRate = 98\%$, provenance sketch is no help since almost no inputs can be skipped (case 1). Else, the provenance is part of the input table which gives the chance to skip the unnecessary inputs, then we have two cases: 1) the number of result tuples smaller than the partition size or 2) not. For 1) if we can find an attribute from the table schema such that the provenance contains part of its distinct values not all of them, which makes chance for some partitions to do not contain provenance and can be filtered out (case 2).  For example, let us consider the top-k query where $k = 10$ and $numPart = 400$. It is obviously to see, even for the worst case, 10 distinct values and each one in one partition, still 390 partitions will be filtered out. Otherwise, provenance contains all the distinct values ($distRate(A) = 1)$), such that every partition contains the provenance (case 3). For 2)  the number of result tuples larger than or equal to the partition size, it is possible the provenance is distributed in every partition especially for the table in which the data is evenly distributed. And with the

\begin{figure}[H]
\begin{lstlisting}[style=pseudocode, basicstyle=\scriptsize\upshape\ttfamily,xleftmargin=.02\textwidth ]
if (provRate $\approx$ 1)							       	(case 1)
	No
else
	if (exists A  and numDistProv(A)  < numPart)
		if (distRate(A) < 1)      				   (case 2)
			Yes
		else												(case 3)
			No
	else													(case 4)
			Yes or No
\end{lstlisting}
  \caption{PS Effectiveness Evaluation}
  \label{fig:ps-effect-evaluate}
\end{figure}
%%%%%%%%%%%%%%%%%%%%%%
provRate $\approx$ 1 represents provenance accounts for almost the whole input table ( e.g, $provRate = 98\%$), provenance sketch is no help since almost no inputs can be skipped (case 1). Else, the provenance is part of the input table which gives the chance to skip the unnecessary inputs. Then we have two cases: 1) if we can find an attribute (say A) from the table schema such that the number of distinct value of A in the provenance is smaller than the number of partitions which makes chance for some partitions to do not contain provenance and can be filtered out if we partition on this attribute A. In addition, we need to keep the provenance do not contain all distinct values of A (case 2). For example,  assume given a query Q and exists an attribute A such that $numDistProv(A) = 100$ , if we generate 400 partitions based on attribute A,  it is obvious to see that even for the worst case the 100 distinct values are evenly distributed in 100 partitions (one distinct value takes one partition), still 300 partitions can be filtered out. However, if the number of distinct values of A is 100 in total, then we can only make 100 partitions at most, so provenance includes all partitions (case 3).  2) if  $numDistProv(A)  >= numPart$, we might get partitions without any provenance or not which is based on the data distribution. It is possible the distinct values of the attribute in the provenance are distributed in a few partitions (Yes) or they are evenly distributed in all the partitions, i.e., every partition contains some of these distinct values (No) (case 4).  And with the increase of the numDistProv(A), the rate that more partitions contain the provenance also tends to increase.

%%%%%%%%%%%%% tpch ps size
\begin{figure}
\centering
   \begin{subfigure}{1\linewidth}
 \begin{adjustbox}{max width=1\linewidth}
\begin{tabular}{|c|c|c|c|c|c|c|c|} \hline
\cthead Table & \cthead Attribute  & \cthead ND & \cthead NDP & \gycell PS32 & \gycell PS64 & \gycell PS400 & \cthead PR  \\ \hline
 customer & c\_custkey  & 150k & 10& 8 & 9 & 10 & 0.007\%\\ \hline
 lineitem &  l\_orderkey  & 1500k  &  10 & 6 & 8 & 9 & 0.001\% \\ \hline
 orders &  o\_orderkey  &  1500k &  10 & 6 & 8 & 9 & 0.0007 \%\\ \hline
\end{tabular}
\end{adjustbox}
   	\caption{Q3}
     \label{tab:q3}
   \end{subfigure}
   %%%%%%%%%%%%%%%%%%%%%%%%%%%%%%%%%%%%%%%%%%%%%%%%%%%%%%%%%%%%%%%%
      \begin{subfigure}{1\linewidth}
\begin{adjustbox}{max width=1\linewidth}
\begin{tabular}{|c|c|c|c|c|c|c|c|} \hline
\cthead Table & \cthead Attribute  & \cthead ND & \cthead NDP & \gycell PS32 & \gycell PS64 & \gycell PS400 & \cthead PR \\ \hline
 customer & c\_custkey  & 150k & 20 & 15 & 19 & 20 & 0.013\%\\ \hline
 lineitem &  l\_orderkey  & 1500k  &  71 & 25 & 38 & 67 & 0.004\%\\ \hline
 orders &  o\_orderkey  &  1500k &  71 & 25 & 37 & 68 & 0.005\%\\ \hline
 nation &  n\_nationkey  &  25 &  15 & 15 & 15 & 15 &60\% \\ \hline
\end{tabular}
\end{adjustbox}
       \caption{Q10}
     \label{tab:q10}
   \end{subfigure}
   %%%%%%%%%%%%%%%%%%%%%%%%%%%%%%%%%%%%%%%%%%%%%%%%%%%%%%%%%%%%%%%%
   \begin{subfigure}{1\linewidth}
\begin{adjustbox}{max width=1\linewidth}
\begin{tabular}{|c|c|c|c|c|c|c|c|} \hline
\cthead Table & \cthead Attribute  & \cthead ND & \cthead NDP & \gycell PS32 & \gycell PS64 & \gycell PS400 & \cthead PR \\ \hline
 supplier & s\_suppkey  & 10k &  1 & 1 & 1 & 1 & 0.01\%\\ \hline
 lineitem &  l\_suppkey  & 10k  &  1 & 1 & 1 & 1 & 0.01\%\\ \hline
\end{tabular}
\end{adjustbox}
      \caption{Q15}
     \label{tab:q15}
   \end{subfigure}
   %%%%%%%%%%%%%%%%%%%%%%%%%%%%%%%%%%%%%%%%%%%%%%%%%%%%%%%%%%%%%%%%
    \begin{subfigure}{1\linewidth}
\begin{adjustbox}{max width=1\linewidth}
\begin{tabular}{|c|c|c|c|c|c|c|c|} \hline
\cthead Table & \cthead Attribute  & \cthead ND & \cthead NDP & \gycell PS32 & \gycell PS64 & \gycell PS400 & \cthead PR\\ \hline
 part & p\_partkey  & 200k &  197 & 32 & 60 & 155 & 0.01\% \\ \hline
 lineitem &  l\_orderkey  & 1500k  &  591 & 32 & 64 & 310 & 0.01\% \\ \hline
 lineitem &  l\_partkey  &  200k &  197  & 32 & 60 & 155 & 0.01\%  \\ \hline
\end{tabular}
\end{adjustbox}
      \caption{Q17}
     \label{tab:q17}
   \end{subfigure}
   %%%%%%%%%%%%%%%%%%%%%%%%%%%%%%%%%%%%%%%%%%%%%%%%%%%%%%%%%%%%%%%%
    \begin{subfigure}{1\linewidth}
\begin{adjustbox}{max width=1\linewidth}
\begin{tabular}{|c|c|c|c|c|c|c|c|} \hline
\cthead Table & \cthead Attribute  & \cthead ND & \cthead NDP & \gycell PS32 & \gycell PS64 & \gycell PS400 & \cthead PR \\ \hline
 customer & c\_custkey  & 150k & 10 & 7 & 9 & 10 & 0.007\%\\ \hline
 lineitem &  l\_orderkey  & 1500k  &  70 & 7 & 9 & 10 & 0.001\% \\ \hline
 orders &  o\_orderkey  &  1500k &  70 & 7 & 9 & 10 & 0.005\% \\ \hline
\end{tabular}
\end{adjustbox}
      \caption{Q18}
     \label{tab:q18}
   \end{subfigure}
   %%%%%%%%%%%%%%%%%%%%%%%%%%%%%%%%%%%%%%%%%%%%%%%%%%%%%%%%%%%%%%%%
       \begin{subfigure}{1\linewidth}
\begin{adjustbox}{max width=1\linewidth}
\begin{tabular}{|c|c|c|c|c|c|c|c|} \hline
\cthead Table & \cthead Attribute  & \cthead ND & \cthead NDP & \gycell PS32 & \gycell PS64 & \gycell PS400 & \cthead PR\\ \hline
 part & p\_partkey  & 200k &  103& 32  & 49 & 89 & 0.05\% \\ \hline
 lineitem &  l\_orderkey  & 1500k  &  121 & 31 & 54 & 97 &0.002\% \\ \hline
\end{tabular}
\end{adjustbox}
     \caption{Q19}
     \label{tab:q19}
   \end{subfigure}
   %%%%%%%%%%%%%%%%%%%%%%%%%%%%%%%%%%%%%%%%%%%%%%%%%%%%%%%%%%%%%%%%
          \begin{subfigure}{1\linewidth}
\begin{adjustbox}{max width=1\linewidth}
\begin{tabular}{|c|c|c|c|c|c|c|c|} \hline
\cthead Table & \cthead Attribute  & \cthead ND & \cthead NDP & \gycell PS32 & \gycell PS64 & \gycell PS400& \cthead PR \\ \hline
 supplier & s\_suppkey  & 10k &  197 & 32  & 59 & 157 & 1.97\%\\ \hline
 part &  p\_partkey  & 200k  & 247  & 32 &63  & 186 & 0.1\%\\ \hline
 lineitem &  l\_orderkey  &  1500k & 2052  & 32 & 64 & 246 & 0.03\%\\ \hline
 \gcell partsupp &  ps\_partkey  & 200k  & 247  & 32 & 63 & 186 & 0.03\% \\ \hline
 \gcell partsupp &  ps\_suppkey  & 10k  & 197  & 32 & 59 & 157 & 0.03\% \\ \hline
 nation &  n\_nationkey  &  25 &  1 & 1 & 1 & 1 & 4\%\\ \hline
\end{tabular}
\end{adjustbox}
     \caption{Q20}
     \label{tab:q20}
   \end{subfigure}
  \caption{Provenance and Provenance Sketch Sizes - TPC-H 1GB: NDP}
  \label{fig:tpch-size-post}
\end{figure}
%%%%%%%%%%%%%%%%%%%%%%%%%%%%%%%%%%%%%%%%%%%%%%%%%%%%%%%%%%%%%%%%

\begin{figure}[H]
\centering
 \begin{adjustbox}{max width=1\linewidth}
\begin{tabular}{|c|c|c|c|c|c|c|c|c|c|c|c|c|} \hline  \rowcolor{red!30}
 	& Q1  & Q3 & Q5 & Q6 & Q7 & Q8 & Q9 & Q10 & Q12 & Q13 & Q14 & Q19  \\ \hline
Provenance size  &98.6\%  &  0.00011\% & 0.28\% &  0.63\%& 0.21\% & 0.136\% &  8.55\%& 0.00048\% & 0.8\%& 99\%& 8.18\%&  0.0036\% \\ \hline
%PS25   & - & - & 98.3\% & - & 98.1\% & & & - & & & &    \\ \hline
PS32 & 100\%  &  28.1\%  & 98.3\% & 100\%& 98\%& 98.5\% & 100\%&   77.5\%  & 100\%& 100\%& 100\%& 97\%  \\ \hline
PS64 & 100\% & 15.6\%&  98.3\% & 100\% & 98\% & 98.5\% &100\% &  57.2\%& 100\%&  100\%& 100\%&  84.1\% \\ \hline
PS400 & 100\% & 2.5\% & 98.3\% & 100\% & 98\% & 98\% &100\% & 16.6\% & 100\%& 100\%& 100\%&  24.2\% \\ \hline
\end{tabular}
\end{adjustbox}
  \caption{Provenance size of TPC-H queries - 1GB}
  \label{fig:prov-size-tpch-1gb}
\end{figure}

%%%%%%%%%%%%%%%%
\subsection{Queries}
\label{sec:queries}
%%%%%%%%%%%%%%%%
%,basicstyle=\small \scriptsize\upshape\ttfamily
\parttitle{Q-1}
Return the.
%\lstset{style=psqlcolor,basicstyle=\small}
\lstset{tabsize=4,style=psqlcolor,basicstyle=\scriptsize\upshape\ttfamily}
\begin{lstlisting}
SELECT * 
FROM (
    SELECT  sum(l_extendedprice*(1-l_discount)) AS revenue, 
    				l_orderkey
    FROM  lineitem 
    GROUP BY  l_orderkey 
    ORDER BY  revenue DESC
    ) 
WHERE rownum <= 10;
\end{lstlisting}

%%%%%%%%%%%%%%%%%%%%%%%%%%%%%%%%%%%%%%%%
\parttitle{Q-2}
Return the.
%\begin{lstlisting}[title = \bf{Query: Q2}, captionpos=b]
\lstset{tabsize=4, style=psqlcolor,basicstyle=\scriptsize\upshape\ttfamily}
\begin{lstlisting}
SELECT * 
FROM (
    SELECT  c_custkey, c_name, c_acctbal, n_name, c_address,
            sum(l_extendedprice * (1 - l_discount)) AS revenue,
            c_acctbal, n_name, c_address, c_phone, c_comment 
    FROM    customer, orders, lineitem, nation 
    WHERE   c_custkey = o_custkey
            AND l_orderkey = o_orderkey
            AND c_nationkey = n_nationkey 
    GROUP BY  c_custkey, c_name, c_acctbal, c_phone,
              n_name, c_address, c_comment 
    ORDER BY  revenue DESC
    ) 
WHERE   rownum <= 10;
\end{lstlisting}

%%%%%%%%%%%%%%%%

%%%%%%%%%%%%%%%%%%%%%%%%%%%%%%%%%%%%%%%%
\parttitle{Q-3}
Return the.
%\begin{lstlisting}[title = \bf{Query: Q2}, captionpos=b]
\lstset{tabsize=4, style=psqlcolor,basicstyle=\scriptsize\upshape\ttfamily}
\begin{lstlisting}
SELECT * FROM (
SELECT p_brand, count(*) AS cnt FROM (
SELECT * FROM 
customer,
orders, 
lineitem, 
partsupp,
part
WHERE c_custkey = o_custkey AND 
      l_orderkey = o_orderkey AND 
      l_partkey = ps_partkey AND
      l_suppkey = ps_suppkey AND
      ps_partkey = p_partkey AND 
      c_custkey in (
SELECT c_custkey 
FROM (
    SELECT 	c_custkey, 
    	   	c_name, 
    	   	sum(l_extendedprice * (1 - l_discount)) AS revenue, 
    	   	c_acctbal,
    	   	n_name,
    	   	c_address,
    	   	c_phone,
    	   	c_comment 
    FROM 	customer, 
    	 	orders, 
    	 	lineitem, 
    	 	nation 
    WHERE 	c_custkey = o_custkey AND 
    		l_orderkey = o_orderkey AND 
    		c_nationkey = n_nationkey 
    GROUP BY 	c_custkey, 
    		 	c_name, 
    			c_acctbal, 
    			c_phone, 
    			n_name, 
    			c_address, 
    			c_comment 
    ORDER BY revenue DESC) 
WHERE rownum <= 1000
))
GROUP BY p_brand
ORDER BY cnt DESC
)
WHERE rownum <= 20;
\end{lstlisting}

%%%%%%%%%%%%%%%%%%%%%%%%%%%%%%%%%%%%%%%%%
%\parttitle{Q-3}
%%
%Return the.
%%\begin{lstlisting}[title = \bf{Query: Q2}, captionpos=b]
%\lstset{tabsize=4, style=psqlcolor,basicstyle=\scriptsize\upshape\ttfamily}
%\begin{lstlisting}
%SELECT * FROM (
%	SELECT	sum(ps_supplycost) AS c, 
%					ps_suppkey 
%	FROM	partsupp
%	WHERE		ps_suppkey IN (
%		SELECT 	l_suppkey 
%		FROM (
%			SELECT 	l_suppkey, 
%							sum(l_extendedprice * (1 - l_discount)) AS revenue
%			FROM 	lineitem 
%			GROUP  BY 	l_suppkey
%			ORDER BY 	sum(l_extendedprice * (1 - l_discount)) desc 
%			)
%		WHERE 	revenue > 23000000)
%	GROUP  BY 	ps_suppkey
%	ORDER BY 	count(*) desc)
%WHERE rownum <= 5;
%\end{lstlisting}
%
%
%
%
%%%%%%%%%%%%%%%%%%%%%%%%%%%%%%%%%%%%%%%%%
%\parttitle{Q-4}
%%
%Return the.
%%\begin{lstlisting}[title = \bf{Query: Q2}, captionpos=b]
%\lstset{tabsize=4, style=psqlcolor,basicstyle=\scriptsize\upshape\ttfamily}
%\begin{lstlisting}
%SELECT * FROM (
%	SELECT	sum(ps_supplycost) AS c, 
%					ps_suppkey 
%	FROM	partsupp
%	WHERE		ps_suppkey IN (
%		SELECT 	l_suppkey 
%		FROM (
%			SELECT 	l_suppkey, 
%							sum(l_extendedprice * (1 - l_discount)) AS revenue
%			FROM 	lineitem 
%			GROUP  BY 	l_suppkey
%			ORDER BY 	sum(l_extendedprice * (1 - l_discount)) desc 
%			)
%		WHERE 	rownum < 1000)
%	GROUP  BY 	ps_suppkey
%	ORDER BY 	count(*) desc)
%WHERE rownum <= 5;
%\end{lstlisting}
%
%%%%%%%%%%%%%%%%%

%%%%%%%%%%%%%%%%
%,basicstyle=\small \scriptsize\upshape\ttfamily
\parttitle{Crimes Q-1}
Return the.
%\lstset{style=psqlcolor,basicstyle=\small}
\lstset{tabsize=4,style=psqlcolor,basicstyle=\scriptsize\upshape\ttfamily}
\begin{lstlisting}
SELECT * FROM (
		SELECT count(*) AS cnt, 
					 district, 
					 ward, 
					 block, 
					 community_area, 
					 beat 
		FROM crimes 
		GROUP BY district, 
						 ward, 
						 block, 
						 community_area, 
						 beat
		) f 
ORDER BY cnt DESC 
LIMIT 5;
\end{lstlisting}
%%%%%%%%%%%%%%%%%%%%%%
%%%%%%%%%%%%%%%%
%,basicstyle=\small \scriptsize\upshape\ttfamily
\parttitle{Crimes Q-2}
Return the.
%\lstset{style=psqlcolor,basicstyle=\small}
\lstset{tabsize=4,style=psqlcolor,basicstyle=\scriptsize\upshape\ttfamily}
\begin{lstlisting}
SELECT count(*) 
FROM (
	SELECT count(*) AS cnt, block 
	FROM crimes 
	GROUP BY block 
	HAVING count(*) > 10000) c
\end{lstlisting}
%%%%%%%%%%%%%%%%%%%%%%

%%%%%%%%%%%%%%%%
%,basicstyle=\small \scriptsize\upshape\ttfamily
\parttitle{Movies Q-1}
Compute the number of ratings per movies and return the top 10.
%\lstset{style=psqlcolor,basicstyle=\small}
\lstset{tabsize=4,style=psqlcolor,basicstyle=\scriptsize\upshape\ttfamily}
\begin{lstlisting}
SELECT title, m.movieid , count(rating) as num_ratings
FROM movies m, ratings r 
WHERE m.movieid=r.movieid 
GROUP BY m.movieid, title
ORDER BY count(rating) DESC 
LIMIT 10;
\end{lstlisting}

%\parttitle{Movies Q-2}
%%
%Compute the number of ratings per comedy movies after 2010  and return the top 10.
%%\lstset{style=psqlcolor,basicstyle=\small}
%\lstset{tabsize=4,style=psqlcolor,basicstyle=\scriptsize\upshape\ttfamily}
%\begin{lstlisting}
%SELECT title, m.movieid , count(rating) as num_ratings
%FROM movies m, ratings r 
%WHERE m.movieid=r.movieid AND
%			genres LIKE '%Comedy%' AND
%			ryear >= 2010
%GROUP BY m.movieid, title
%ORDER BY count(rating) DESC 
%LIMIT 10
%\end{lstlisting}

\parttitle{Movies  Q-2}
Compute the 
%\lstset{style=psqlcolor,basicstyle=\small}
\lstset{tabsize=4,style=psqlcolor,basicstyle=\scriptsize\upshape\ttfamily}
\begin{lstlisting}
SELECT COUNT(*) AS cnt FROM (
SELECT title, m.movieid , count(rating) as num_ratings
FROM movies m, ratings r 
WHERE m.movieid=r.movieid 
GROUP BY m.movieid, title 
HAVING count(rating) >= 63300) c;
\end{lstlisting}

%\parttitle{Movies Q-3}
%
%Return from 2010, the number of the rated comedy movies each year.
%%\lstset{style=psqlcolor,basicstyle=\small}
%\lstset{tabsize=4,style=psqlcolor,basicstyle=\scriptsize\upshape\ttfamily}
%\begin{lstlisting}
%SELECT count(*) as cnt, ryear
%FROM movies m, ratings r 
%WHERE m.movieid=r.movieid AND
%			genres LIKE '%Comedy%' AND
%			ryear >= 2010
%GROUP BY ryear
%\end{lstlisting}

\parttitle{Movies Q-3}
Return the top 10 popular movies (the movies with  top 10 number of  tags + ratings, count(ratings)/count(tags) = 43).
%\lstset{style=psqlcolor,basicstyle=\small}
\lstset{tabsize=4,style=psqlcolor,basicstyle=\scriptsize\upshape\ttfamily}
\begin{lstlisting}
SELECT title, m.movieid, total_cnt
FROM (
	SELECT total_cnt, movieid
	FROM ( 
		SELECT cnt1/43 + cnt2 AS total_cnt, t1.movieid
		FROM
			(SELECT count(*) AS cnt1, movieid
			FROM ratings
			GROUP BY movieid) r1,
			(SELECT count(*) AS cnt2, movieid
			FROM tags
			GROUP BY movieid) t1
		WHERE r1.movieid = t1.movieid) tc1
	ORDER BY total_cnt DESC
	LIMIT 10) tc2,
	movies m
WHERE tc2.movieid = m.movieid			
\end{lstlisting}
%
%\parttitle{Movies Q-4}
%%
%Return the.
%%\lstset{style=psqlcolor,basicstyle=\small}
%\lstset{tabsize=4,style=psqlcolor,basicstyle=\scriptsize\upshape\ttfamily}
%\begin{lstlisting}
%SELECT title , m.movieid , cnt 
%FROM (
%	SELECT cnt , movieid 
%	FROM (
%		SELECT count(distinct tag)+count(distinct rating) AS cnt,
%		r.movieId
%		FROM ratings r, tags t 
%		WHERE r.movieid = t.movieId 
%		GROUP BY r.movieid) c
%	ORDER BY cnt DESC 
%	LIMIT 10) tc, 
%	movies m
%WHERE tc.movieid =m.movieid
%\end{lstlisting}
%
%
%\parttitle{Movies Q-5}
%%
%Return the.
%%\lstset{style=psqlcolor,basicstyle=\small}
%\lstset{tabsize=4,style=psqlcolor,basicstyle=\scriptsize\upshape\ttfamily}
%\begin{lstlisting}
%SELECT * FROM (
%	SELECT max(total_rating) AS max_total_rating, ryear
%	FROM (
%		SELECT ryear, movieid, sum(rating) AS total_rating
%		FROM ratings
%		GROUP BY ryear, movieid) t
%	GROUP BY ryear) mt,
%	(SELECT ryear , movieid , sum(rating) AS total_rating
%	FROM ratings
%	GROUP BY ryear, movieid) t1,
%	movies m
%WHERE max_total_rating=total_rating AND 
%			mt.ryear = t1.ryear AND
%			t1.movieid=m.movieid 
%ORDER BY max_total_rating DESC 
%LIMIT 3;
%\end{lstlisting}

%%%%%%%%%%%%%%%%%%%%%%%%%%%%%%%%%%%%%%%%

\parttitle{Virtual sketches + Primary/Foreign Key index} \\

\parttitle{Postgres + Movies} \\
%%%%%%%%%%%%%%%%%%%%%%%%%%%%%%%%%%%%%%%%%%%%%%%%%%%%%%%%%%%%%%%%
%% CQ1
%%%%%%%%%%%%% CQ1
\begin{figure}[H]
\centering
\begin{tabular}{|c|c|c|c|} \hline  \rowcolor{red!30}
 Movies Q1  &  PS32 & PS64 & PS400 \\ \hline
Capture cost  &  56.82 & 57.32 & 65.58  \\ \hline
 Normal cost  &  12.29 & 12.29 & 12.29 \\ \hline
 PS cost  & 3.82 & 2.85 &  2.17\\ \hline
\end{tabular}
  \caption{Movies Q1 Cost - Postgresql}
  \label{fig:movies-q1-cost-post}
\end{figure}
%%%%%%%%%%%%% CQ1 ps size
\begin{figure}[H]
\centering
 \begin{adjustbox}{max width=1\linewidth}
\begin{tabular}{|c|c|c|} \hline  \rowcolor{red!30}
Movies Q1 & Movies  & Ratings   \\ \hline
PS attributes & movieid & movieid\\ \hline
Total size &   27278 &   20000263 \\ \hline
 Provenance size &  10  &  581765\\ \hline
 PS size (PS32)  &  1705  &  4427150  \\ \hline
 PS size (PS64)  &   1278 &   3197823 \\ \hline
 PS size (PS400)  &  546  &   1622633 \\ \hline
\end{tabular}
\end{adjustbox}
  \caption{Movies Q1 Size - Postgresql}
  \label{fig:movies-q1-size-post}
\end{figure}
%%%%%%%%%%%%%%%%%%%%%%%%%%%%%%%%%%%%%%%%%%%%%%%%%%%%%%%%%%%%%%%%

%
%%%%%%%%%%%%%%%%%%%%%%%%%%%%%%%%%%%%%%%%%%%%%%%%%%%%%%%%%%%%%%%%%
%%% Movie Q2
%%%%%%%%%%%%%% MQ2
%\begin{figure}[H]
%\centering
%\begin{tabular}{|c|c|c|c|} \hline  \rowcolor{red!30}
% Movies Q2  &  PS32 & PS64 & PS400 \\ \hline
%Capture cost  &  6.63 & 6.81 & 7.27 \\ \hline
% Normal cost  &  4.07 &4.07 & 4.07 \\ \hline
% PS cost  &   2.85 &  2.03 &  1.07 \\ \hline
%\end{tabular}
%  \caption{Movies Q2 Cost - Postgresql}
%  \label{fig:movies-q2-cost-post}
%\end{figure}
%%%%%%%%%%%%%% CQ1 ps size
%\begin{figure}[H]
%\centering
% \begin{adjustbox}{max width=1\linewidth}
%\begin{tabular}{|c|c|c|} \hline  \rowcolor{red!30}
%Movies Q2 & Movies  & Ratings   \\ \hline
%PS attributes & movieid & movieid\\ \hline
%Total size &   27278 &   20000263 \\ \hline
% Provenance size &  10 & 407761 \\ \hline
% PS size (PS32)  &   5114 &  5949919  \\ \hline
% PS size (PS64)  &   2984 &    3696253 \\ \hline
% PS size (PS400)  &   681 &  1219933  \\ \hline
%\end{tabular}
%\end{adjustbox}
%  \caption{Movies Q2 Size - Postgresql}
%  \label{fig:movies-q2-size-post}
%\end{figure}
%%%%%%%%%%%%%%%%%%%%%%%%%%%%%%%%%%%%%%%%%%%%%%%%%%%%%%%%%%%%%%%%%

%%%%%%%%%%%%%%%%%%%%%%%%%%%%%%%%%%%%%%%%%%%%%%%%%%%%%%%%%%%%%%%%
%% CQ1
%%%%%%%%%%%%% CQ1
\begin{figure}[H]
\centering
\begin{tabular}{|c|c|c|c|} \hline  \rowcolor{red!30}
 Movies Q2   &  PS32 & PS64 & PS400 \\ \hline
Capture cost  & 56.48  & 58.04 & 64.54 \\ \hline
 Normal cost  &   11.76& 11.76 & 11.76 \\ \hline
 PS cost  &   1.33 & 1.95  & 0.86  \\ \hline
\end{tabular}
  \caption{Movies Q2 Cost - Postgresql}
  \label{fig:movies-q2-cost-post}
\end{figure}
%%%%%%%%%%%%% CQ1 ps size
\begin{figure}[H]
\centering
 \begin{adjustbox}{max width=1\linewidth}
\begin{tabular}{|c|c|c|} \hline  \rowcolor{red!30}
Movies Q2  & Movies  & Ratings   \\ \hline
PS attributes & movieid & movieid \\ \hline
Total size &   27278 &  20000263   \\ \hline
 Provenance size &  3 & 196848 \\ \hline
 PS size (PS32)  &  852  & 1510063  \\ \hline
 PS size (PS64)  &   426 &  978988  \\ \hline
 PS size (PS400)  &   137 &  591595 \\ \hline
\end{tabular}
\end{adjustbox}
  \caption{Movies Q2 Size - Postgresql}
  \label{fig:movies-q2-size-post}
\end{figure}
%%%%%%%%%%%%%%%%%%%%%%%%%%%%%%%%%%%%%%%%%%%%%%%%%%%%%%%%%%%%%%%%

\xn{32p uses hash join, 64p uses nested loop}

%%%%%%%%%%%%%%%%%%%%%%%%%%%%%%%%%%%%%%%%%%%%%%%%%%%%%%%%%%%%%%%%
%% mQ3
%%%%%%%%%%%%% mQ3
\begin{figure}[H]
\centering
\begin{tabular}{|c|c|c|c|} \hline  \rowcolor{red!30}
 Movies Q3  &  PS32 & PS64 & PS400 \\ \hline
Capture cost  &  28.76 & 29.67 & 33.26 \\ \hline
 Normal cost  &  6.59 & 6.59 & 6.59 \\ \hline
 PS cost  &  2.53  &  2.0 &  1.23 \\ \hline
\end{tabular}
  \caption{Movies Q3 Cost - Postgresql}
  \label{fig:movies-q3-cost-post}
\end{figure}
%%%%%%%%%%%%% CQ1 ps size
\begin{figure}[H]
\centering
 \begin{adjustbox}{max width=1\linewidth}
\begin{tabular}{|c|c|c|c|} \hline  \rowcolor{red!30}
Movies Q3 & Movies  & Ratings & tags  \\ \hline
PS attributes & movieid & movieid & movieid\\ \hline
Total size &   27278 &  20000263  & 465564 \\ \hline
 Provenance size &  10 & 581765 &  9858\\ \hline
 PS size (PS32)  &   1705 &  4427150 & 51375\\ \hline
 PS size (PS64)  &  1278  & 3197823  & 46056 \\ \hline
 PS size (PS400)  &   546 &  1622633 &  20020\\ \hline
\end{tabular}
\end{adjustbox}
  \caption{Movies Q3 Size - Postgresql}
  \label{fig:movies-q3-size-post}
\end{figure}
%%%%%%%%%%%%%%%%%%%%%%%%%%%%%%%%%%%%%%%%%%%%%%%%%%%%%%%%%%%%%%%%

\parttitle{Postgres + Crimes} \\
%%%%%%%%%%%%%%%%%%%%%%%%%%%%%%%%%%%%%%%%%%%%%%%%%%%%%%%%%%%%%%%%
%% CQ1
%%%%%%%%%%%%% CQ1
\begin{figure}[H]
\centering
\begin{tabular}{|c|c|} \hline  \rowcolor{red!30}
 Crimes Q1  &   \\ \hline
Capture cost  & 35.27   \\ \hline
 Normal cost  &  6.17  \\ \hline
 PS cost  & 3.16   \\ \hline
\end{tabular}
  \caption{Crimes CQ1 Cost - Postgresql}
  \label{fig:crimes-cq1-cost-post}
\end{figure}
%%%%%%%%%%%%% CQ1 ps size
\begin{figure}[H]
\centering
 \begin{adjustbox}{max width=1\linewidth}
\begin{tabular}{|c|c|c|c|c|c|} \hline  \rowcolor{red!30}
Crimes Q1 & Crimes  & Crimes & Crimes  & Crimes & Crimes  \\ \hline
PS attributes & district & community\_area & ward & beat & \color{red}{combination} \\ \hline
Total size & 6271290  &  6271290 &  6271290 & 6271290 &\color{red}{ 6271290}\\ \hline
 Provenance size & 42360   &  42360 & 42360 &  42360 & \color{red}{42360}\\ \hline
 PS size   &  1162958  &  447675  &  399751 & 133657  & \color{red}{114726}\\ \hline
\end{tabular}
\end{adjustbox}
  \caption{Crimes CQ1 Size - Postgresql}
  \label{fig:crimes-cq1-size-post}
\end{figure}
%%%%%%%%%%%%%%%%%%%%%%%%%%%%%%%%%%%%%%%%%%%%%%%%%%%%%%%%%%%%%%%%

\xn{\\
Order by cnt desc: \\
	1. tried 400 ps on cid, but can not save inputs \\
	2. number of distinct value:  district(24) ,community\_area(78),  ward(50), beat(303)  \\
Order by cnt: \\
	1. result is wrong after apply ps on cid
}

%%%%%%%%%%%%%%%%%%%%%%%%%%%%%%%%%%%%%%%%%%%%%%%%%%%%%%%%%%%%%%%%
%% CQ2
%%%%%%%%%%%%% CQ2
\begin{figure}[H]
\centering
\begin{tabular}{|c|c|} \hline  \rowcolor{red!30}
 Crimes Q2  &   \\ \hline
Capture cost  &  34.1  \\ \hline
 Normal cost  &  3.26  \\ \hline
 PS cost  &  1.93  \\ \hline
\end{tabular}
  \caption{Crimes Q2 Cost - Postgresql}
  \label{fig:crimes-q2-cost-post}
\end{figure}
%%%%%%%%%%%%% CQ1 ps size
\begin{figure}[H]
\centering
 \begin{adjustbox}{max width=1\linewidth}
\begin{tabular}{|c|c|c|c|c|c|} \hline  \rowcolor{red!30}
Crimes Q2 & Crimes  & Crimes & Crimes  & Crimes & Crimes  \\ \hline
PS attributes & district & community\_area & ward & beat & \color{red}{combination} \\ \hline
Total size & 6271290  &  6271290 &  6271290 & 6271290 &\color{red}{ 6271290}\\ \hline
 Provenance size & 60722   &  60722 & 60722 &  60722 & \color{red}{60722}\\ \hline
 PS size   &  458423  &  185069  &  319984 & 74582  & \color{red}{60722}\\ \hline
\end{tabular}
\end{adjustbox}
  \caption{Crimes Q2 Size - Postgresql}
  \label{fig:crimes-q2-size-post}
\end{figure}
%%%%%%%%%%%%%%%%%%%%%%%%%%%%%%%%%%%%%%%%%%%%%%%%%%%%%%%%%%%%%%%%	

\parttitle{Postgres + TPC-H 10GB} \\
%%%%%%%%%%%%%%%%%%%%%%%%%%%%%%%%%%%%%%%%%%%%%%%%%%%%%%%%%%%%%%%%
%% Q3
%%%%%%%%%%%%% Q3 cost
\begin{figure}[H]
\centering
\begin{tabular}{|c|c|c|c|} \hline  \rowcolor{red!30}
 Q3  & 32P & 64P & 400P \\ \hline
 Capture cost  &  53.56 &  53.92 & 53.93 \\ \hline
%Capture cost  &  56.86 &  59.50 & 89.10 \\ \hline
 Normal cost  &  53.23 &  53.23 &   53.23 \\ \hline
 PS cost  & 4.20  &  2.05 &   0.31 \\ \hline
\end{tabular}
  \caption{TPC-H 10GB Q3 Cost - Postgresql}
  \label{fig:tpch-10gb-q3-cost-post}
\end{figure}

%%%%%%%%%%%%% Q3 ps size
\begin{figure}[H]
\centering
\begin{tabular}{|c|c|c|c|} \hline  \rowcolor{red!30}
 Q3 & Customer  & Lineitem & Orders  \\ \hline
PS attributes & c\_custkey  & l\_orderkey & o\_orderkey  \\ \hline
Total size & 1500000  &  59986052 &  15000000  \\ \hline
 Provenance size &  10  & 68  & 10  \\ \hline
 PS size  (32P) & 417673  & 14904439 &  3836659 \\ \hline
  PS size  (64P)&  236321 & 8360710  &  2092083  \\ \hline
  PS size  (400P) &  37733 &   1380787 &   366926  \\ \hline
\end{tabular}
  \caption{TPC-H 10GB Q3 Size - Postgresql}
  \label{fig:tpch-10gb-q3-size-post}
\end{figure}
%%%%%%%%%%%%%%%%%%%%%%%%%%%%%%%%%%%%%%%%%%%%%%%%%%%%%%%%%%%%%%%%

%%%%%%%%%%%%%%%%%%%%%%%%%%%%%%%%%%%%%%%%%%%%%%%%%%%%%%%%%%%%%%%%
%% Q10
%%%%%%%%%%%%% Q10 cost
\begin{figure}[H]
\centering
\begin{tabular}{|c|c|c|c|} \hline  \rowcolor{red!30}
 Q10  & 32P & 64P  & 400P \\ \hline
 Capture cost  &  36.37 &  36.17 & 36.52 \\ \hline
%Capture cost  &  42.87 &  51.27 & 156.23 \\ \hline
 Normal cost & 32.62 &  32.62 & 32.62   \\ \hline
 PS cost  &  14.69 &  7.54  & 1.44 \\ \hline
\end{tabular}
  \caption{TPC-H 10GB Q10 Cost - Postgresql}
  \label{fig:tpch-10gb-q10-cost-post}
\end{figure}

%\xn{hippo size get from plan, might not correct }
%%%%%%%%%%%%% Q10 ps size
\begin{figure}[H]
\centering
 \begin{adjustbox}{max width=1\linewidth}
\begin{tabular}{|c|c|c|c|c|} \hline  \rowcolor{red!30}
 Q10 & Customer  & Lineitem & Orders & Nation \\ \hline
 PS attributes & c\_custkey  & l\_orderkey & o\_orderkey & n\_nationkey\\ \hline
Total size & 1500000  &  59986052 &  15000000  & 25\\ \hline
 Provenance size & 20  & 309  &  85  & 14 \\ \hline
 PS size  (32P) & 705121   & 56113835  &   14024463  & 14\\ \hline
  PS size   (64P)& 435974  & 44233236  &  10599688  & 14\\ \hline
  PS size   (400P)&  75545 &   11557482 &  2885719  & 14 \\ \hline
\end{tabular}
 \end{adjustbox}
  \caption{TPC-H 10GB Q10 Size - Postgresql}
  \label{fig:tpch-10gb-q10-size-post}
\end{figure}
%%%%%%%%%%%%%%%%%%%%%%%%%%%%%%%%%%%%%%%%%%%%%%%%%%%%%%%%%%%%%%%%

%%%%%%%%%%%%%%%%%%%%%%%%%%%%%%%%%%%%%%%%%%%%%%%%%%%%%%%%%%%%%%%%
%% Q19
%%%%%%%%%%%%% Q19 cost
\begin{figure}[H]
\centering
\begin{tabular}{|c|c|c|c|} \hline  \rowcolor{red!30}
 Q19 & 32P & 64P & 400P  \\ \hline
 Capture cost  &  1.249 & 1.251   &  1.3\\ \hline
  Normal cost  &  1.27 & 1.27  &  1.27\\ \hline
  PS cost  & 1.27 &  1.27 & 1.27 \\ \hline
%Capture cost  &  1.50 & 1.58   &  1.58\\ \hline
% Normal cost  &  1.43 & 1.43  &  1.43\\ \hline
% PS cost  & 1.43 &  1.43 & 1.43 \\ \hline
\end{tabular}
  \caption{TPC-H 10GB Q19 Cost - Postgresql}
  \label{fig:tpch-10gb-q19-cost-post}
\end{figure}

%%%%%%%%%%%%% Q19 overhead
\begin{figure}[H]
\centering
 \begin{adjustbox}{max width=1\linewidth}
\begin{tabular}{|c|c|c|} \hline  \rowcolor{red!30}
 Q19  & Part  & Lineitem\\ \hline
PS attributes   &  p\_partkey & l\_orderkey\\ \hline
Total size &  2000000 & 59986052 \\ \hline
 Provenance size &   1032 & 1134  \\ \hline
 PS size  (32P) &  2000000  &  59986052\\ \hline
 PS size  (64P) &  2000000  & 59986052 \\ \hline
  PS size  (400P) &  1846867 & 56335758 \\ \hline
\end{tabular}
 \end{adjustbox}
  \caption{TPC-H 10GB Q19 Size - Postgresql}
  \label{fig:tpch-10gb-q19-size-post}
\end{figure}

\parttitle{Postgres + TPC-H 1GB} \\

\begin{itemize}
  \item Quick Overview 
    		\begin{itemize}
  			\item Q3 : 0.0059x
  			\item Q10: 0.06x
  			\item Q19: 0.47x
  		\end{itemize}
\end{itemize}
  		
 %runtime
 %%%%%%%%%%%%%%%%%%%%%%%%%%%%%%%%%%%%%%%%
 \begin{figure}[H]
   \centering
   \includegraphics[width=1\linewidth,trim=0pt 0pt 0 0pt, clip]{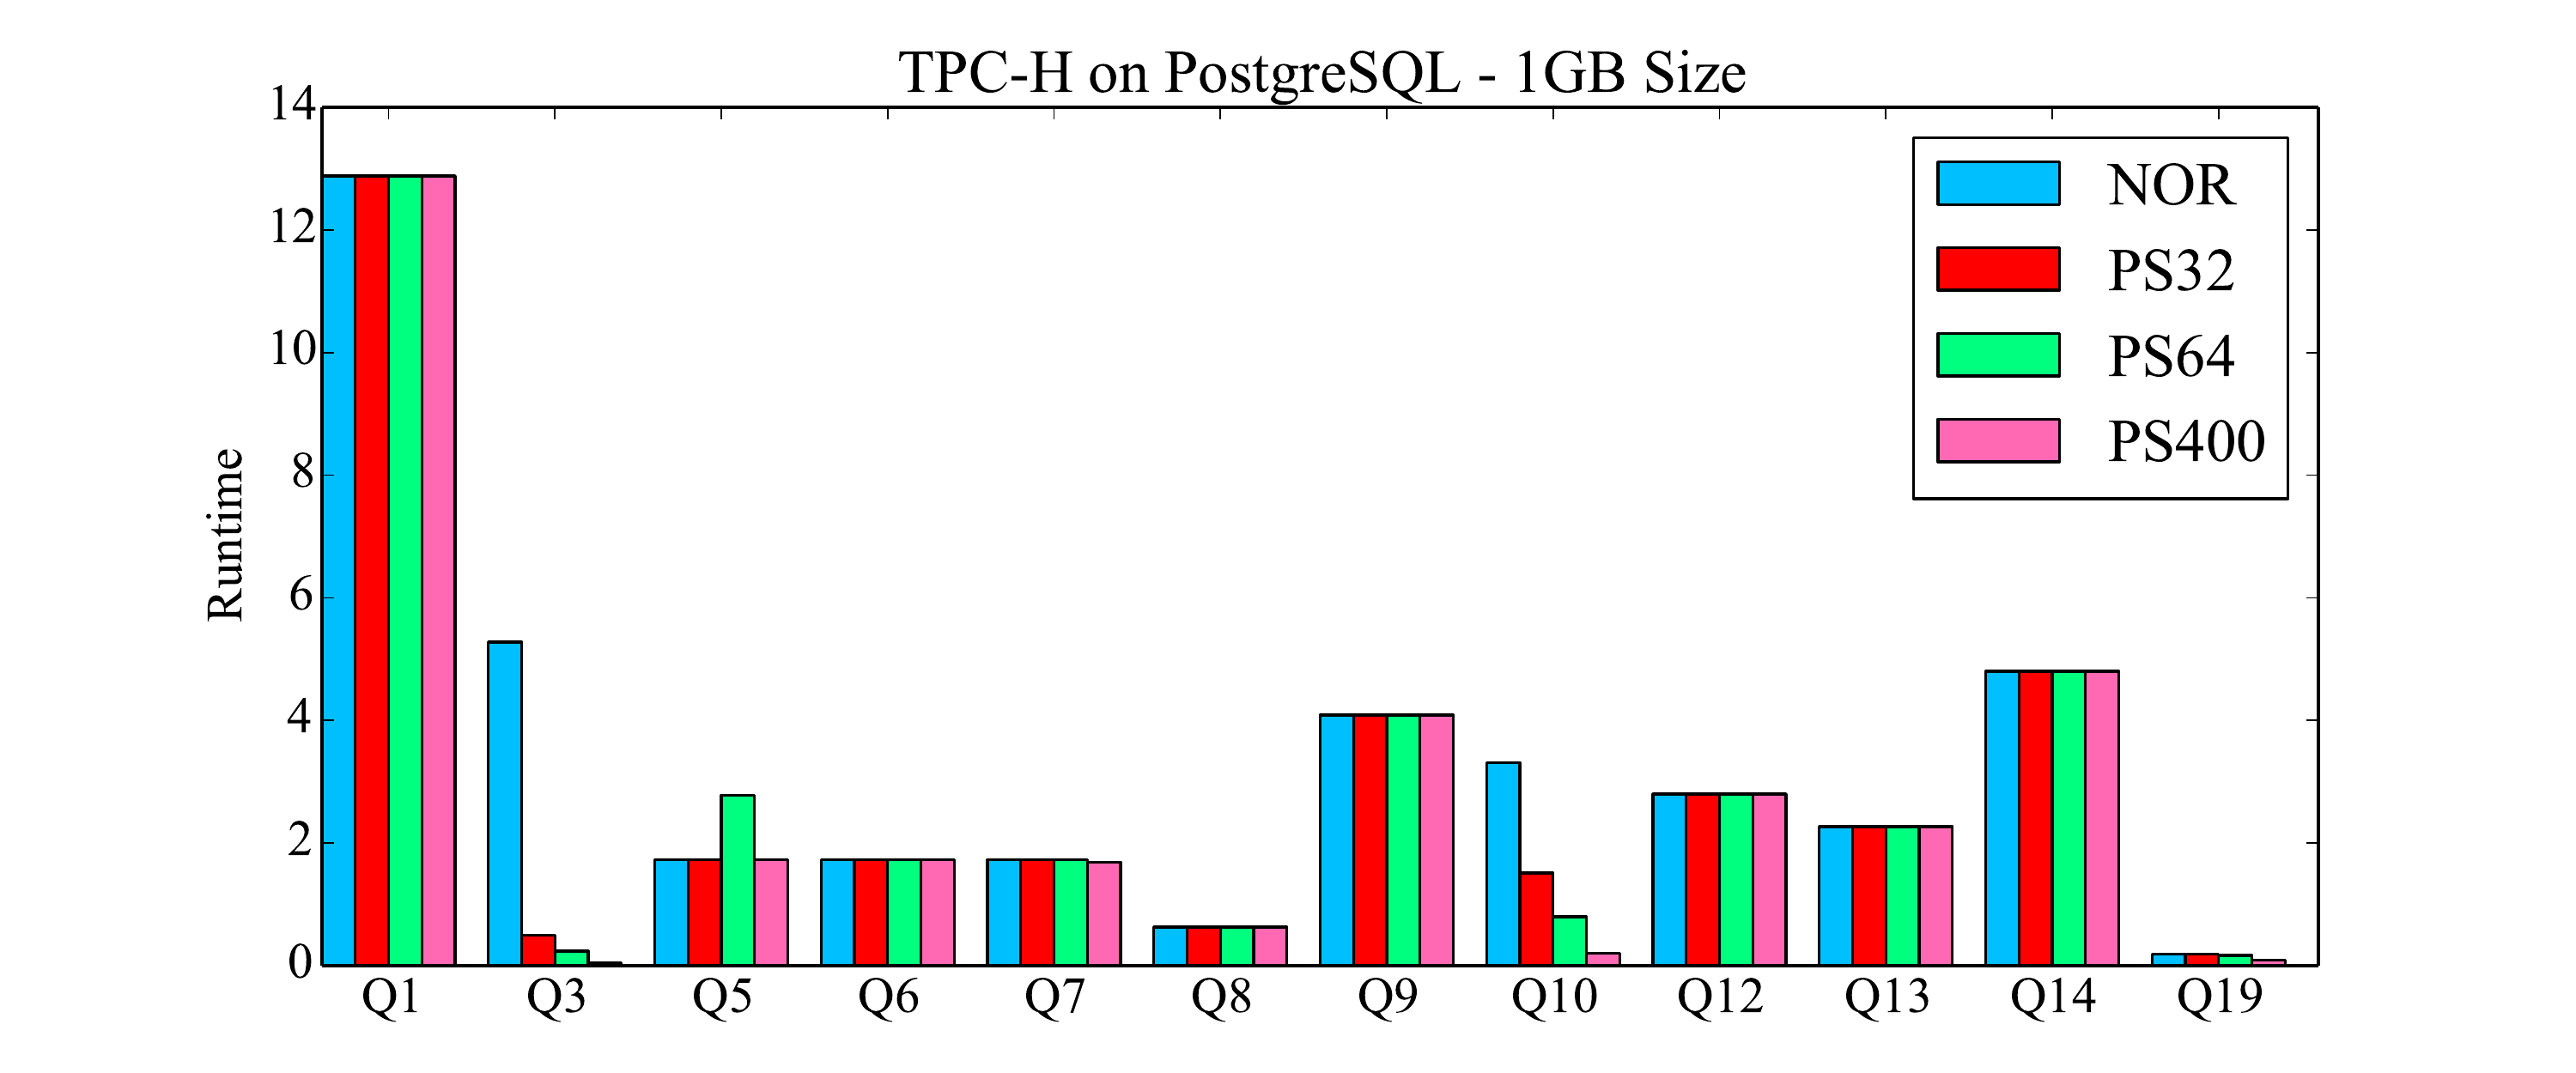}
   \caption{Runtime of TPC-H queries on PostgreSQL - 1GB Size}
   \label{fig:tpch-post-1gb-old}
 \end{figure}
%%%%%%%%%%%%%%%%%%%%%%%%%%%%%%%%%%%%%%%% 		

 %capture
 %%%%%%%%%%%%%%%%%%%%%%%%%%%%%%%%%%%%%%%%
 \begin{figure}[H]
   \centering
   \includegraphics[width=1\linewidth,trim=0pt 0pt 0 0pt, clip]{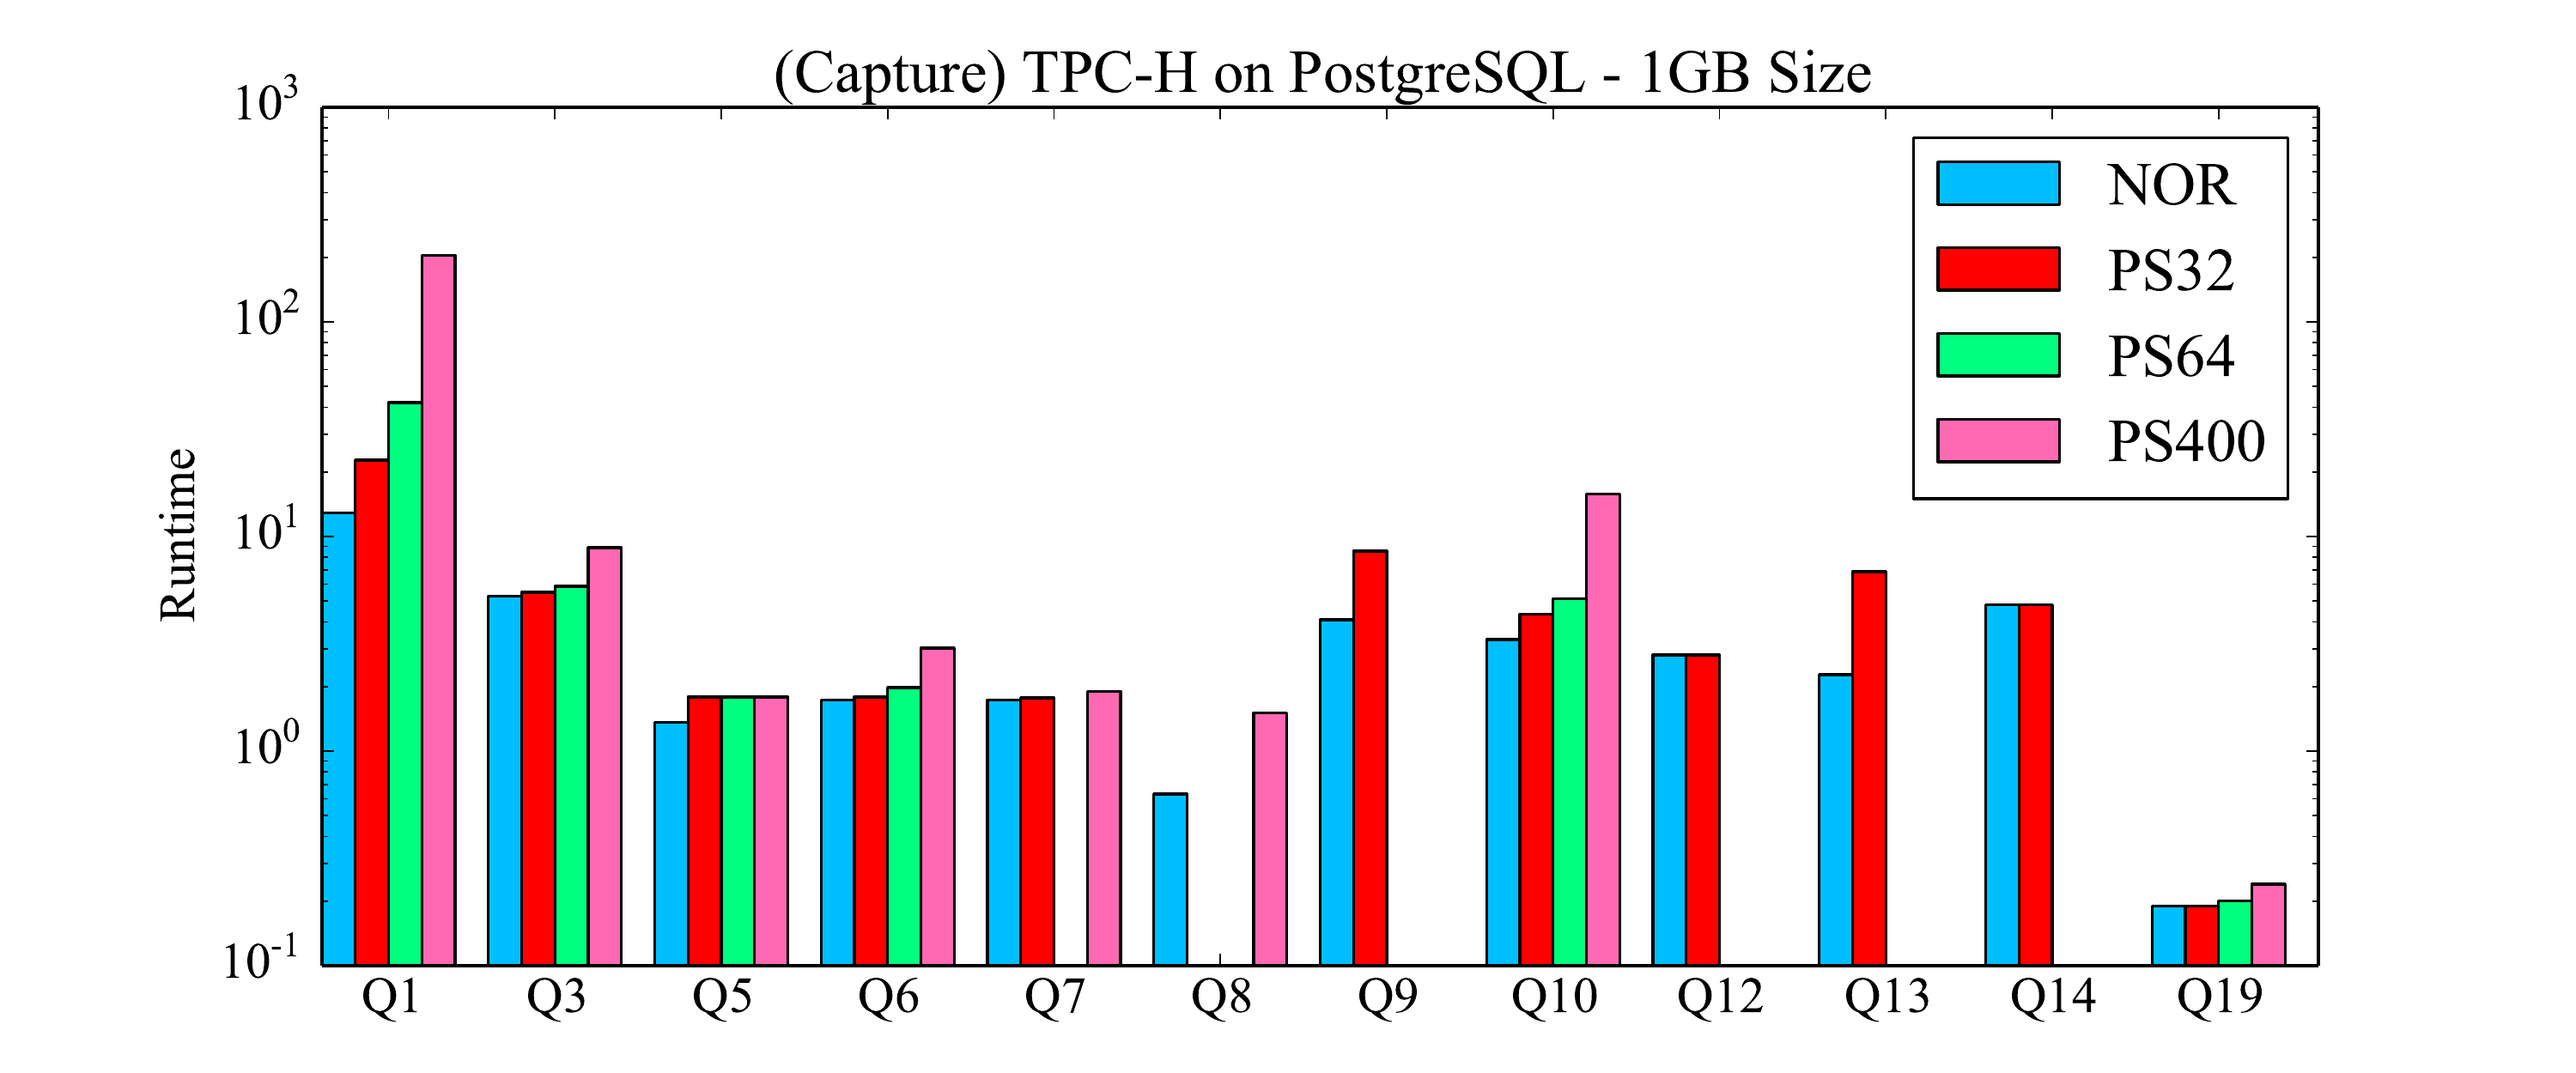}
   \caption{(Capture cost of TPC-H queries on PostgreSQL - 1GB Size}
   \label{fig:cap-tpch-post-1gb-old}
 \end{figure}
%%%%%%%%%%%%%%%%%%%%%%%%%%%%%%%%%%%%%%%% 	

%size
 %%%%%%%%%%%%%%%%%%%%%%%%%%%%%%%%%%%%%%%%
 \begin{figure}[H]
   \centering
   \includegraphics[width=1\linewidth,trim=0pt 0pt 0 0pt, clip]{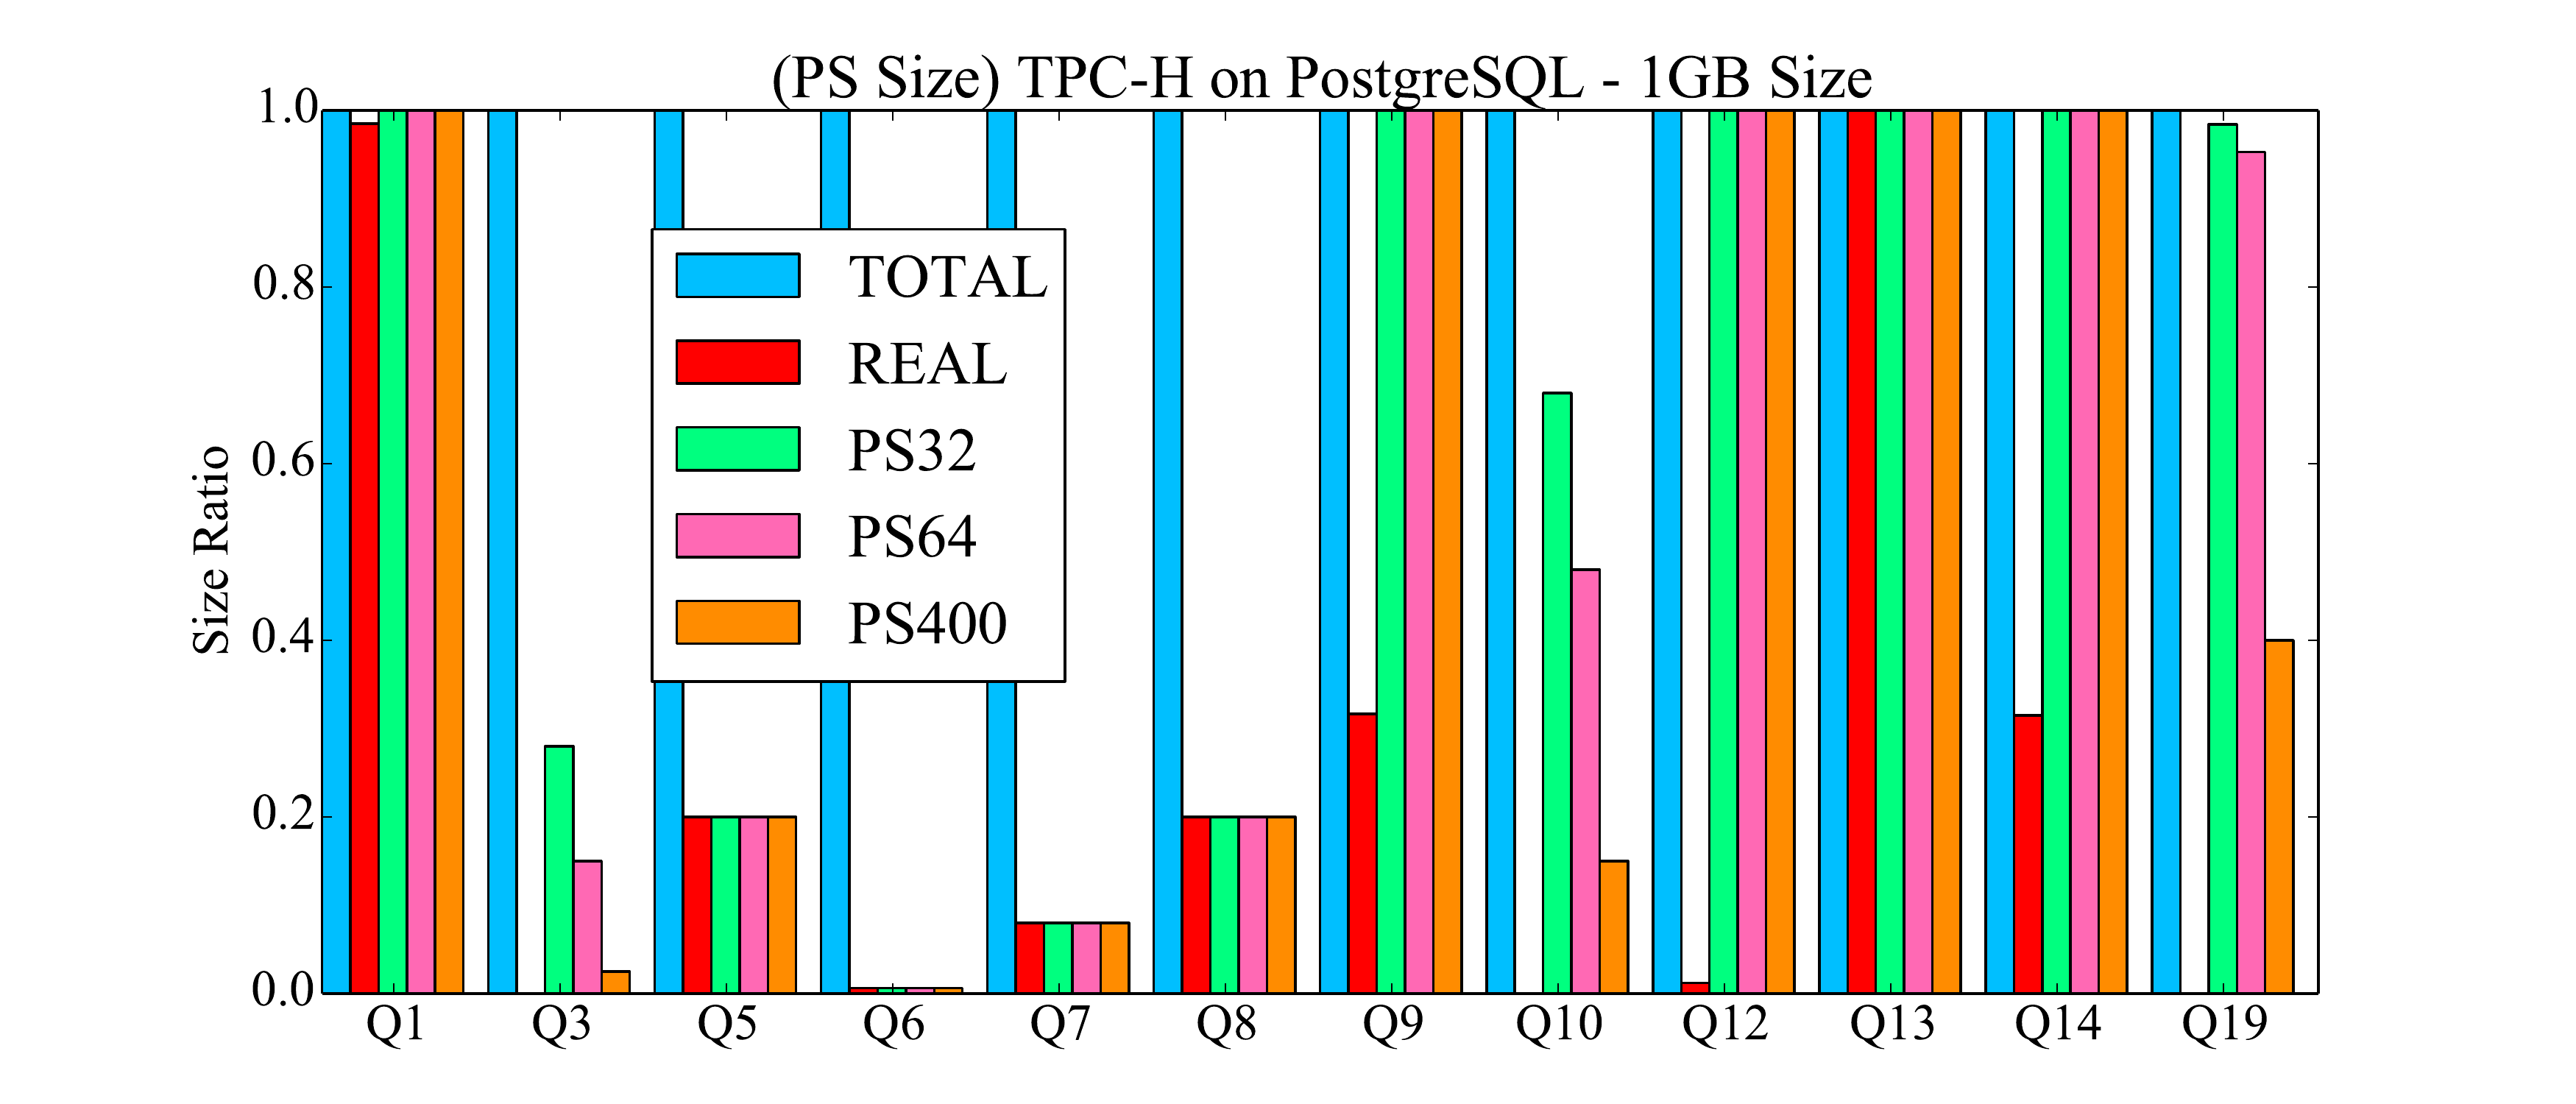}
   \caption{(PS Size of TPC-H queries on PostgreSQL - 1GB Size}
   \label{fig:size-tpch-post-1gb-old}
 \end{figure}
%%%%%%%%%%%%%%%%%%%%%%%%%%%%%%%%%%%%%%%% 	
  		
%%%%%%%%%%%%%%%%%%%%%%%%%%%%%%%%%%%%%%%%%%%%%%%%%%%%%%%%%%%%%%%%
%% Q3
%%%%%%%%%%%%% Q3 cost
\begin{figure}[H]
\centering
\begin{tabular}{|c|c|c|c|} \hline  \rowcolor{red!30}
 Q3  & 32P & 64P & 400P \\ \hline
Capture cost  &  2.34 &  2.34  &  2.38\\ \hline
 Normal cost  &  2.2 &  2.2&  2.2 \\ \hline
 PS cost  & 0.46  &  0.23 &  0.047 \\ \hline
%Capture cost  &  5.50 &  5.86  &  8.88\\ \hline
% Normal cost  &  5.28 &  5.28 &  5.28 \\ \hline
% PS cost  & 0.50  &  0.24 &  0.05 \\ \hline
  %Hippo cost  &  0.77 &  0.48 & -  \\ \hline  
\end{tabular}
  \caption{TPC-H Q3 Cost - Postgresql}
  \label{fig:tpch-q3-cost-post}
\end{figure}

%%%%%%%%%%%%% Q3 ps size
\begin{figure}[H]
\centering
\begin{tabular}{|c|c|c|c|} \hline  \rowcolor{red!30}
 Q3 & Customer  & Lineitem & Orders  \\ \hline
PS attributes & c\_custkey  & l\_orderkey & o\_orderkey  \\ \hline
Total size & 150000  & 6001215  &  1500000  \\ \hline
 Provenance size &  10 &  65 &  10 \\ \hline
 PS size  (32P) & 42188  & 1687846 & 421875  \\ \hline
 %Hippo size (32 ranges)  & 14210  & not use  & 96670  \\ \hline  
  PS size  (64P)& 21094  &  937698 &  234377  \\ \hline
 %Hippo size  (64 ranges) &  8900 & not use  & 68510  \\ \hline  
  PS size  (400P) &  3750 &   150040 &   37500  \\ \hline
\end{tabular}
  \caption{TPC-H Q3 Size - Postgresql}
  \label{fig:tpch-q3-size-post}
\end{figure}
%%%%%%%%%%%%%%%%%%%%%%%%%%%%%%%%%%%%%%%%%%%%%%%%%%%%%%%%%%%%%%%%

%%%%%%%%%%%%%%%%%%%%%%%%%%%%%%%%%%%%%%%%%%%%%%%%%%%%%%%%%%%%%%%%
%% Q10
%%%%%%%%%%%%% Q10 cost
\begin{figure}[H]
\centering
\begin{tabular}{|c|c|c|c|} \hline  \rowcolor{red!30}
 Q10  & 32P & 64P  & 400P\\ \hline
 Capture cost  & 3.3 & 3.25  & 3.28\\ \hline
  Normal cost  & 2.78  &   2.78 &  2.78\\ \hline
   PS cost  & 1.42  &  0.72 & 0.20\\ \hline
%Capture cost  &  4.35 & 5.12  & 15.86\\ \hline
% Normal cost  & 3.31  &   3.31 &  3.31\\ \hline
 %PS cost  & 1.51  &  0.80 & 0.20\\ \hline
  %Hippo cost  & 1.82  &  2.45  &  -\\ \hline  
\end{tabular}
  \caption{TPC-H Q10 Cost - Postgresql}
  \label{fig:tpch-q10-cost-post}
\end{figure}

%\xn{hippo size get from plan, might not correct }
%%%%%%%%%%%%% Q10 ps size
\begin{figure}[H]
\centering
\begin{tabular}{|c|c|c|c|c|} \hline  \rowcolor{red!30}
 Q10 & Customer  & Lineitem & Orders  & Nation\\ \hline
 PS attributes & c\_custkey  & l\_orderkey & o\_orderkey & n\_nationkey  \\ \hline
Total size & 150000  & 6001215  &  1500000  & 25\\ \hline
 Provenance size & 20  &  259 &  71 & 15  \\ \hline
 PS size  (32P) &  70312  &  4688449 &  1171875  & 15 \\ \hline
 %Hippo size  (32 ranges)  &  21810  & not use  & 215140  \\ \hline  
  PS size   (64P)&  42201 &  3468643 & 867185  & 15 \\ \hline
 %Hippo size   (64 ranges) & 15890  & not use  & 182980  \\ \hline  
  PS size   (400P)&  7500 &  1005215  &  255000  & 15 \\ \hline
\end{tabular}
  \caption{TPC-H Q10 Size - Postgresql}
  \label{fig:tpch-q10-size-post}
\end{figure}
%%%%%%%%%%%%%%%%%%%%%%%%%%%%%%%%%%%%%%%%%%%%%%%%%%%%%%%%%%%%%%%%

%
%%%%%%%%%%%%%% Q10 ps size
%\begin{figure}[H]
%\centering
%\begin{tabular}{|c|c|c|c|c|} \hline  \rowcolor{red!30}
% Q10 & Customer  & Lineitem & Orders & Nation \\ \hline
%Total size & 150000  & 6001215  &  1500000 & 25 \\ \hline
% Provenance size & 20  &  1775 &  432 &  15 \\ \hline
% PS size  (32 ranges) &  70312  &  4688449 &  1171875 &  15 \\ \hline
% %Hippo size  (32 ranges)  &  21810  & not use  & 215140 & 15 \\ \hline  
%  PS size   (64 ranges)&  42201 &  3468643 & 867185  &  15 \\ \hline
% %Hippo size   (64 ranges) & 15890  & not use  & 182980 &  15 \\ \hline  
%  PS size   (400 ranges)&  13500 &  424061  &  431250  &  15 \\ \hline
%\end{tabular}
%  \caption{TPC-H Q10 Size - Postgresql}
%  \label{fig:tpch-q10-size-post}
%\end{figure}
%%%%%%%%%%%%%%%%%%%%%%%%%%%%%%%%%%%%%%%%%%%%%%%%%%%%%%%%%%%%%%%%%

%%%%%%%%%%%%%%%%%%%%%%%%%%%%%%%%%%%%%%%%%%%%%%%%%%%%%%%%%%%%%%%%
%% Q1
%%%%%%%%%%%%% Q1 cost
\begin{figure}[H]
\centering
\begin{tabular}{|c|c|c|c|} \hline  \rowcolor{red!30}
 Q1  & 32P& 64P & 400P \\ \hline
Capture cost  & 22.71  & 42.12 &  204.24\\ \hline
 Normal cost  & 12.88 & 12.88 & 12.88   \\ \hline
 PS cost  &  12.88 &  12.88 &  12.88 \\ \hline
\end{tabular}
  \caption{TPC-H Q1 Cost - Postgresql}
  \label{fig:tpch-q1-cost-post}
\end{figure}

%%%%%%%%%%%%% Q1 overhead
\begin{figure}[H]
\centering
\begin{tabular}{|c|c|} \hline  \rowcolor{red!30}
 Q1   & Lineitem   \\ \hline
Total size &  6001215   \\ \hline
 Provenance size &   5914748  \\ \hline
 PS size  (32P) &   6001215    \\ \hline
 PS size   (64P) &    6001215    \\ \hline
 PS size   (400P) &   6001215      \\ \hline
\end{tabular}
  \caption{TPC-H Q1 Size - Postgresql}
  \label{fig:tpch-q1-size-post}
\end{figure}

%%%%%%%%%%%%%%%%%%%%%%%%%%%%%%%%%%%%%%%%%%%%%%%%%%%%%%%%%%%%%%%%

%%%%%%%%%%%%%%%%%%%%%%%%%%%%%%%%%%%%%%%%%%%%%%%%%%%%%%%%%%%%%%%%
%% Q2
%%%%%%%%%%%%% Q2 cost
\begin{figure}[H]
\centering
\begin{tabular}{|c|c|c|c|} \hline  \rowcolor{red!30}
 Q2  & 32P& 64P & 400P \\ \hline
Capture cost  & 0.61 & 0.61 &  0.65\\ \hline
 Normal cost  & 0.4 & 0.4  & 0.4    \\ \hline
 PS cost  &  0.45 &  0.52 &  1.6 \\ \hline
\end{tabular}
  \caption{TPC-H Q2 Cost - Postgresql}
  \label{fig:tpch-q2-cost-post}
\end{figure}

%%%%%%%%%%%%% Q2 size
\begin{figure}[H]
\centering
\begin{tabular}{|c|c|c|c|c|c|} \hline  \rowcolor{red!30}
 Q2   & Part & Supplier & Partsupp & nation & region   \\ \hline
Total size &   200000 & 10000 &  800000 & 25 & 5 \\ \hline
 Provenance size &  100 & 89 & 400 & 5 & 1   \\ \hline
 PS size  (32P) &   193750 & 9375 &  775000 & 5 & 1    \\ \hline
 PS size   (64P) &   162500 & 7344 & 650000 & 5 & 1     \\ \hline
 PS size   (400P) &   45499 & 1976 & 181996 & 5 & 1      \\ \hline
\end{tabular}
  \caption{TPC-H Q2 Size - Postgresql}
  \label{fig:tpch-q2-size-post}
\end{figure}

%%%%%%%%%%%%%%%%%%%%%%%%%%%%%%%%%%%%%%%%%%%%%%%%%%%%%%%%%%%%%%%%

%%%%%%%%%%%%%%%%%%%%%%%%%%%%%%%%%%%%%%%%%%%%%%%%%%%%%%%%%%%%%%%%
%% Q4
%%%%%%%%%%%%% Q4 cost
\begin{figure}[H]
\centering
\begin{tabular}{|c|c|c|c|} \hline  \rowcolor{red!30}
 Q4 & 32P & 64P & 400P  \\ \hline
Capture cost  & &  &   \\ \hline
 Normal cost  &   &    &    \\ \hline
 PS cost  &  &  &   \\ \hline
\end{tabular}
  \caption{TPC-H Q4 Cost - Postgresql}
  \label{fig:tpch-q4-cost-post}
\end{figure}

%%%%%%%%%%%%% Q4 overhead
\begin{figure}[H]
\centering
 \begin{adjustbox}{max width=1\linewidth}
\begin{tabular}{|c|c|c|} \hline  \rowcolor{red!30}
 Q4 & Orders & Lineitem  \\ \hline
PS attributes  & o\_orderkey & l\_orderkey  \\ \hline
Total size &  1500000 &  6001215  \\ \hline
 Provenance size &   53035 &  146450  \\ \hline
 PS size  (32P) &   &       \\ \hline
 PS size  (64P) &  &     \\ \hline
  PS size  (400P) &  &     \\ \hline
\end{tabular}
 \end{adjustbox}
  \caption{TPC-H Q4 Size - Postgresql}
  \label{fig:tpch-q4-size-post}
\end{figure}

%%%%%%%%%%%%%%%%%%%%%%%%%%%%%%%%%%%%%%%%%%%%%%%%%%%%%%%%%%%%%%%%

%%%%%%%%%%%%%%%%%%%%%%%%%%%%%%%%%%%%%%%%%%%%%%%%%%%%%%%%%%%%%%%%
%% Q5
%%%%%%%%%%%%% Q5 cost
\begin{figure}[H]
\centering
\begin{tabular}{|c|c|} \hline  \rowcolor{red!30}
 Q5  & 25P \\ \hline
Capture cost  &  1.48   \\ \hline
 Normal cost  & 1.36   \\ \hline
 PS cost  &   1.36  \\ \hline
\end{tabular}
  \caption{TPC-H Q5 Cost - Postgresql}
  \label{fig:tpch-q5-cost-post}
\end{figure}

%%%%%%%%%%%%% Q5 overhead
\begin{figure}[H]
\centering
 \begin{adjustbox}{max width=1\linewidth}
\begin{tabular}{|c|c|c|c|c|c|c|} \hline  \rowcolor{red!30}
 Q5 & Customer  & Orders & Lineitem & Supplier  & Nation & Region\\ \hline
 PS attributes   &  c\_nationkey  &  &  & s\_nationkey & n\_nationkey  & \\ \hline
Total size &  150000  & 1500000   &  6001215  & 10000 & 25 & 5\\ \hline
 Provenance size &  5561 &  6670 &  7243 & 1945 & 5 & 1   \\ \hline
 PS size  (25P) &  30183 &    &   & 2003  & 5 & 1 \\ \hline
\end{tabular}
 \end{adjustbox}
  \caption{TPC-H Q5 Size - Postgresql}
  \label{fig:tpch-q5-size-post}
\end{figure}
%\begin{figure}[H]
%\centering
%\begin{tabular}{|c|c|c|c|} \hline  \rowcolor{red!30}
% Q5 & Customer  & Supplier  & Nation \\ \hline
% PS attributes   & c\_nationkey  &  s\_nationkey & n\_nationkey \\ \hline
%Total size & 150000  & 10000  &  25 \\ \hline
% Provenance size &  30183 &  2003 &  5  \\ \hline
% PS size  (25P) &  30183 & 2003   &  5  \\ \hline
%\end{tabular}
%  \caption{TPC-H Q5 Size - Postgresql}
%  \label{fig:tpch-q5-size-post}
%\end{figure}

%%%%%%%%%%%%%%%%%%%%%%%%%%%%%%%%%%%%%%%%%%%%%%%%%%%%%%%%%%%%%%%%

\xn{\\
      1. Q5: Tried  400 partitions on c\_custkey in customer, l\_orderkey in lineitem, o\_orderkey in orders and s\_suppkey in supplier, only ps on supplier can save 2 partitions.  \\
      2. Only find ps on nationkey in customer, supplier and nation table can save input tuples.\\
      3. 25 partitions since only 25 nations \\
      4. The ps query cost is same with the normal query cost, I checked the query plan, since the join order and nationkey is the join condition, join was used as the same effect as the ps. }

%%%%%%%%%%%%%%%%%%%%%%%%%%%%%%%%%%%%%%%%%%%%%%%%%%%%%%%%%%%%%%%%
%% Q6
%%%%%%%%%%%%% Q6 cost
\begin{figure}[H]
\centering
\begin{tabular}{|c|c|c|c|} \hline  \rowcolor{red!30}
 Q6  & 32P& 64P & 400P\\ \hline
Capture cost  &  1.79 & 1.98 & 3.02 \\ \hline
 Normal cost  & 1.73 & 1.73 & 1.73 \\ \hline
 PS cost  &  1.73 & 1.73 & 1.73 \\ \hline
\end{tabular}
  \caption{TPC-H Q6 Cost - Postgresql}
  \label{fig:tpch-q6-cost-post}
\end{figure}

%%%%%%%%%%%%% Q6 overhead
\begin{figure}[H]
\centering
\begin{tabular}{|c|c|} \hline  \rowcolor{red!30}
 Q6  & Lineitem  \\ \hline
  PS attributes    & l\_orderkey \\ \hline
Total size  & 6001215  \\ \hline
 Provenance size    &  37898  \\ \hline
 PS size  (32P)    & 6001215  \\ \hline
  PS size   (64P)   &  6001215  \\ \hline
   PS size  (400P)    & 6001215  \\ \hline
\end{tabular}
  \caption{TPC-H Q6 Size - Postgresql}
  \label{fig:tpch-q6-size-post}
\end{figure}

\xn{Q6\\ 
1. $l\_discount > 0.05$ AND $l\_discount < 0.07$ only includes 0.06 (one distinct tuple) \\
2.$ l\_quantity < 24$ (return 1-23, with other conditions together still same with containing this condition only \\
3. 400 partitions can not save inputs)
}

%%%%%%%%%%%%%%%%%%%%%%%%%%%%%%%%%%%%%%%%%%%%%%%%%%%%%%%%%%%%%%%%

%%%%%%%%%%%%%%%%%%%%%%%%%%%%%%%%%%%%%%%%%%%%%%%%%%%%%%%%%%%%%%%%
%% Q7
%%%%%%%%%%%%% Q1 cost
%\begin{figure}[H]
%\centering
%\begin{tabular}{|c|c|} \hline  \rowcolor{red!30}
% Q7  & 25P \\ \hline
%Capture cost  &  3.94   \\ \hline
% Normal cost  & 3.94   \\ \hline
% PS cost  &  3.11   \\ \hline
%\end{tabular}
%  \caption{TPC-H Q7 Cost - Postgresql}
%  \label{fig:tpch-q7-cost-post}
%\end{figure}

%%%%%%%%%%%%%% Q7 overhead
%\begin{figure}[H]
%\centering
%\begin{tabular}{|c|c|c|} \hline  \rowcolor{red!30}
% Q7 & Customer  & Supplier   \\ \hline
% PS attributes   & c\_nationkey  &  s\_nationkey  \\ \hline
%Total size & 150000  & 10000     \\ \hline
% Provenance size &  12008 &  798   \\ \hline
% PS size  (25P) &  12008 & 798     \\ \hline
%\end{tabular}
%  \caption{TPC-H Q7 Size - Postgresql}
%  \label{fig:tpch-q7-size-post}
%\end{figure}

\begin{figure}[H]
\centering
\begin{tabular}{|c|c|c|} \hline  \rowcolor{red!30}
 Q7  & 25P & 400p\\ \hline
Capture cost  &  1.77 &  1.90\\ \hline
 Normal cost  & 1.73  & 1.73 \\ \hline
 PS cost  &  1.73 & 1.69 \\ \hline
\end{tabular}
  \caption{TPC-H Q7 Cost - Postgresql}
  \label{fig:tpch-q7-cost-post}
\end{figure}

%%%%%%%%%%%%% Q7 overhead
\begin{figure}[H]
\centering
 \begin{adjustbox}{max width=1\linewidth}
\begin{tabular}{|c|c|c|c|c|c|c|} \hline  \rowcolor{red!30}
 Q7 & Customer  & Orders & Lineitem &  Supplier & nation1 & nation2  \\ \hline
 PS attributes   & c\_nationkey  &   &  &  s\_nationkey/s\_suppkey &  &   \\ \hline
Total size &  150000 & 1500000  & 6001215 &  10000 & 25 & 25   \\ \hline
 Provenance size & 3882  &  5484 & 5906 & 796 & 2 & 2  \\ \hline
 PS size  (25P) & 12008 & & & 798 &  &      \\ \hline
 PS size  (400p) &  & & & 9051 &  &      \\ \hline
 PS size  (1000p) &  & & & 5791 &  &      \\ \hline
\end{tabular}
 \end{adjustbox}
  \caption{TPC-H Q7 Size - Postgresql}
  \label{fig:tpch-q7-size-post}
\end{figure}

%%%%%%%%%%%%%%%%%%%%%%%%%%%%%%%%%%%%%%%%%%%%%%%%%%%%%%%%%%%%%%%%

\xn{Q7\\ 
      1. Tried  400 partitions on c\_custkey in customer, l\_orderkey in lineitem, o\_orderkey in orders and s\_suppkey in supplier, only s\_suppkey save 949 tuples (9.4\%). try more partitions ? \\
      2.  nationkey saves more }

%%%%%%%%%%%%%%%%%%%%%%%%%%%%%%%%%%%%%%%%%%%%%%%%%%%%%%%%%%%%%%%%
%% Q8
%%%%%%%%%%%%% Q1 cost
\begin{figure}[H]
\centering
\begin{tabular}{|c|c|c|c|} \hline  \rowcolor{red!30}
 Q8 & 32 Ranges& 64 Ranges & 400 Ranges \\ \hline
Capture cost  &   &  &  1.51 \\ \hline
 Normal cost  & 0.63 &  0.63  &   0.63 \\ \hline
 PS cost  &  0.63  &  0.63  & 0.63  \\ \hline
\end{tabular}
  \caption{TPC-H Q8 Cost - Postgresql}
  \label{fig:tpch-q8-cost-post}
\end{figure}

%%%%%%%%%%%%% Q1 overhead
\begin{figure}[H]
\centering
 \begin{adjustbox}{max width=1\linewidth}
\begin{tabular}{|c|c|c|c|c|c|c|c|c|} \hline  \rowcolor{red!30}
 Q8 & Customer  & Orders  & Lineitem & Supplier & Part & Nation1 & Nation2 & regiton\\ \hline
PS attributes   & c\_nationkey/c\_custkey &o\_orderkey & l\_orderkey & s\_suppkey & p\_partkey & n\_nationkey & n\_nationkey & r\_regionkey \\ \hline
Total size & 150000 & 1500000  & 6001215  &  10000 & 200000 & 25 & 25 & 5 \\ \hline
 Provenance size &  2385 &  2567 &  2603 & 1895 & 1221  &  5 & 25 & 1 \\ \hline
% PS size  (32 ranges) & 150000  & 6001215  &  10000 & 200000 & 5 \\ \hline
 %PS size  (64 ranges) & 150000  & 6001215  &  10000 & 200000 & 5 \\ \hline
 PS size  (25p) &  29952 &    &   &   &  & 5 &   & 1\\ \hline
 PS size  (400p) &  150000 &  1496250  & 5986213  &  9900 & 186500 & 5 &  25 & 1 \\ \hline
 PS size  (1000p) &  139200 &  1411516  & 5602456  &  8781 & 138401 & 5 &  25 & 1 \\ \hline
\end{tabular}
 \end{adjustbox}
  \caption{TPC-H Q8 Size - Postgresql}
  \label{fig:tpch-q8-size-post}
\end{figure}

%\begin{figure}[H]
%\centering
%\begin{tabular}{|c|c|c|c|} \hline  \rowcolor{red!30}
% Q8 & 32 Ranges& 64 Ranges & 400 Ranges \\ \hline
%Capture cost  & 0.98  &  &  \\ \hline
% Normal cost  & 0.96 &  0.96  &   0.96 \\ \hline
% PS cost  &  0.96  &  0.96  & 0.96  \\ \hline
%\end{tabular}
%  \caption{TPC-H Q8 Cost - Postgresql}
%  \label{fig:tpch-q8-cost-post}
%\end{figure}
%
%%%%%%%%%%%%%% Q1 overhead
%\begin{figure}[H]
%\centering
% \begin{adjustbox}{max width=1\linewidth}
%\begin{tabular}{|c|c|c|c|c|c|} \hline  \rowcolor{red!30}
% Q8 & Customer  & Lineitem & Supplier & Part &Nation(n1) \\ \hline
%PS attributes   & c\_custkey  & l\_orderkey & s\_suppkey & p\_partkey & n\_nationkey \\ \hline
%Total size & 150000  & 6001215  &  10000 & 200000 & 25 \\ \hline
% Provenance size &  2385 &  5914748 &  1895 & 1221  &  5 \\ \hline
% PS size  (32 ranges) & 150000  & 6001215  &  10000 & 200000 & 5 \\ \hline
% PS size  (64 ranges) & 150000  & 6001215  &  10000 & 200000 & 5 \\ \hline
% PS size  (400 ranges) & 150000  & 6001215   &  10000 &  198500 & 5 \\ \hline
%\end{tabular}
% \end{adjustbox}
%  \caption{TPC-H Q8 Size - Postgresql}
%  \label{fig:tpch-q8-size-post}
%\end{figure}

%%%%%%%%%%%%%%%%%%%%%%%%%%%%%%%%%%%%%%%%%%%%%%%%%%%%%%%%%%%%%%%%

\xn{Q8\\
1. Tried 32p and 64p, only 400p can save some, try more partitions? \\
2.Since s\_nationkey = n2.n\_nationkey where n2 uses all tuples,  c\_nationkey in customer and n\_nationkey in nation n1 is selective, but they were used in the join condition , apply the ps on these two attributes which is no use and hurts the query which results in the query cost 1.84s since the join order was changed. \\
}

%%%%%%%%%%%%%%%%%%%%%%%%%%%%%%%%%%%%%%%%%%%%%%%%%%%%%%%%%%%%%%%%
%% Q9
%%%%%%%%%%%%% Q9 cost
\begin{figure}[H]
\centering
\begin{tabular}{|c|c|c|c|} \hline  \rowcolor{red!30}
 Q9 & 32P &64P & 400P \\ \hline
Capture cost  & 8.56  & &   \\ \hline
 Normal cost  & 4.09 & 4.09 & 4.09   \\ \hline
 PS cost  & 4.09  & 4.09 & 4.09  \\ \hline
\end{tabular}
  \caption{TPC-H Q9 Cost - Postgresql}
  \label{fig:tpch-q9-cost-post}
\end{figure}

%%%%%%%%%%%%% Q9 overhead
\begin{figure}[H]
\centering
 \begin{adjustbox}{max width=1\linewidth}
\begin{tabular}{|c|c|c|c|c|c|c|} \hline  \rowcolor{red!30}
 Q9 & Part & Partsupp & Orders  & Lineitem & Supplier & Nation(n1) \\ \hline
 PS attributes & p\_partkey & ps\_partkey  & o\_orderkey & l\_orderkey  & s\_suppkey & n\_nationkey \\ \hline
Total size & 200000 & 800000 & 1500000  & 6001215  &  10000 & 25 \\ \hline
 Provenance size & 11637 & 46525  & 311172  &  348760 & 9923 & 25 \\ \hline
 PS size  (32P) & 200000& 800000  & 1500000 & 6001215   &  10000 &  25 \\ \hline
 PS size  (64P) & 200000&  800000  & 1500000 & 6001215   &  10000 &  25 \\ \hline
  PS size  (400P) & 200000 & 800000  & 1500000 & 6001215   &  10000 &  25 \\ \hline
\end{tabular}
 \end{adjustbox}
  \caption{TPC-H Q9 Size - Postgresql}
  \label{fig:tpch-q9-size-post}
\end{figure}

%%%%%%%%%%%%%%%%%%%%%%%%%%%%%%%%%%%%%%%%%%%%%%%%%%%%%%%%%%%%%%%%

%%%%%%%%%%%%%%%%%%%%%%%%%%%%%%%%%%%%%%%%%%%%%%%%%%%%%%%%%%%%%%%%
%% Q11
%%%%%%%%%%%%% Q11 cost
\begin{figure}[H]
\centering
\begin{tabular}{|c|c|c|c|} \hline  \rowcolor{red!30}
 Q11 & 32P & 64P & 400P  \\ \hline
Capture cost  & &  &   \\ \hline
 Normal cost  &   &    &    \\ \hline
 PS cost  &  &  &   \\ \hline
\end{tabular}
  \caption{TPC-H Q11 Cost - Postgresql}
  \label{fig:tpch-q11-cost-post}
\end{figure}

%%%%%%%%%%%%% Q11 overhead
\begin{figure}[H]
\centering
 \begin{adjustbox}{max width=1\linewidth}
\begin{tabular}{|c|c|c|c|} \hline  \rowcolor{red!30}
 Q11 & Partsupp & Supplier  & Nation\\ \hline
PS attributes  & ps\_partkey or ps\_suppkey &  s\_suppkey  & n\_nationkey \\ \hline
Total size &  800000 &  10000 &   25\\ \hline
 Provenance size &  1062&  2743  &   1 \\ \hline
 PS size  (32P) &   &   &    \\ \hline
 PS size  (64P) &  &   &   \\ \hline
  PS size  (400P) &  &   &   \\ \hline
\end{tabular}
 \end{adjustbox}
  \caption{TPC-H Q11 Size - Postgresql}
  \label{fig:tpch-q11-size-post}
\end{figure}

%%%%%%%%%%%%%%%%%%%%%%%%%%%%%%%%%%%%%%%%%%%%%%%%%%%%%%%%%%%%%%%%

%%%%%%%%%%%%%%%%%%%%%%%%%%%%%%%%%%%%%%%%%%%%%%%%%%%%%%%%%%%%%%%%
%% Q12
%%%%%%%%%%%%% Q12 cost
\begin{figure}[H]
\centering
\begin{tabular}{|c|c|c|c|} \hline  \rowcolor{red!30}
 Q12 & 32P &64P & 400P \\ \hline
Capture cost  &  2.8  & &  \\ \hline
 Normal cost  & 2.8  & 2.8 & 2.8 \\ \hline
 PS cost  &  2.8  & 2.8 & 2.8 \\ \hline
\end{tabular}
  \caption{TPC-H Q12 Cost - Postgresql}
  \label{fig:tpch-q12-cost-post}
\end{figure}

%%%%%%%%%%%%% Q12 overhead
\begin{figure}[H]
\centering
 \begin{adjustbox}{max width=1\linewidth}
\begin{tabular}{|c|c|c|} \hline  \rowcolor{red!30}
 Q12  & Orders  & Lineitem\\ \hline
PS attributes   &  o\_orderkey  & l\_orderkey\\ \hline
Total size & 1500000  & 6001215\\ \hline
 Provenance size &  29099 & 30988  \\ \hline
 PS size  (32P) &  1500000  & 6001215\\ \hline
 PS size  (64P) &  1500000 & 6001215 \\ \hline
   PS size  (400P) &  1500000 & 6001215 \\ \hline
\end{tabular}
 \end{adjustbox}
  \caption{TPC-H Q12 Size - Postgresql}
  \label{fig:tpch-q12-size-post}
\end{figure}

%%%%%%%%%%%%%%%%%%%%%%%%%%%%%%%%%%%%%%%%%%%%%%%%%%%%%%%%%%%%%%%%

%%%%%%%%%%%%%%%%%%%%%%%%%%%%%%%%%%%%%%%%%%%%%%%%%%%%%%%%%%%%%%%%
%% Q13
%%%%%%%%%%%%% Q13 cost
\begin{figure}[H]
\centering
\begin{tabular}{|c|c|c|c|} \hline  \rowcolor{red!30}
 Q13 & 32P &64P & 400P \\ \hline
Capture cost  &  6.84 & &   \\ \hline
 Normal cost  & 2.27  & 2.27 & 2.27 \\ \hline
 PS cost  & 2.27 & 2.27 & 2.27 \\ \hline
\end{tabular}
  \caption{TPC-H Q13 Cost - Postgresql}
  \label{fig:tpch-q13-cost-post}
\end{figure}

%%%%%%%%%%%%% Q13 overhead
\begin{figure}[H]
\centering
 \begin{adjustbox}{max width=1\linewidth}
\begin{tabular}{|c|c|c|} \hline  \rowcolor{red!30}
 Q13  & Customer & Orders \\ \hline
PS attributes  &  c\_custkey & o\_orders \\ \hline
Total size &  150000 & 1500000 \\ \hline
 Provenance size &  150000  & 1483918 \\ \hline
 PS size  (32P) &  150000 & 1500000\\ \hline
  PS size   (64P)&     150000 & 1500000\\ \hline
    PS size   (400P)&     150000 & 1500000\\ \hline
\end{tabular}
 \end{adjustbox}
  \caption{TPC-H Q13 Size - Postgresql}
  \label{fig:tpch-q13-size-post}
\end{figure}

%%%%%%%%%%%%%%%%%%%%%%%%%%%%%%%%%%%%%%%%%%%%%%%%%%%%%%%%%%%%%%%%

%%%%%%%%%%%%%%%%%%%%%%%%%%%%%%%%%%%%%%%%%%%%%%%%%%%%%%%%%%%%%%%%
%% Q14
%%%%%%%%%%%%% Q14 cost
\begin{figure}[H]
\centering
\begin{tabular}{|c|c|c|c|} \hline  \rowcolor{red!30}
 Q14 & 32P &64P & 400P \\ \hline
Capture cost  &  4.80  & &  \\ \hline
 Normal cost  & 4.80  & 4.80 &  4.80\\ \hline
 PS cost  & 4.80  & 4.80 & 4.80 \\ \hline
\end{tabular}
  \caption{TPC-H Q14 Cost - Postgresql}
  \label{fig:tpch-q14-cost-post}
\end{figure}

%%%%%%%%%%%%% Q14 overhead
\begin{figure}[H]
\centering
 \begin{adjustbox}{max width=1\linewidth}
\begin{tabular}{|c|c|c|} \hline  \rowcolor{red!30}
 Q14  & Part  & Lineitem\\ \hline
PS attributes   &  p\_partkey & l\_orderkey\\ \hline
Total size &  200000 & 1500000\\ \hline
 Provenance size &  63112  &  75983\\ \hline
 PS size  (32P) &  200000 & 1500000\\ \hline
 PS size  (64P) &  200000 & 1500000\\ \hline
  PS size  (400P) &  200000 & 1500000\\ \hline
\end{tabular}
 \end{adjustbox}
  \caption{TPC-H Q14 Size - Postgresql}
  \label{fig:tpch-q14-size-post}
\end{figure}

%%%%%%%%%%%%%%%%%%%%%%%%%%%%%%%%%%%%%%%%%%%%%%%%%%%%%%%%%%%%%%%%

%%%%%%%%%%%%%%%%%%%%%%%%%%%%%%%%%%%%%%%%%%%%%%%%%%%%%%%%%%%%%%%%
%% Q15
%%%%%%%%%%%%% Q15 cost
\begin{figure}[H]
\centering
\begin{tabular}{|c|c|c|c|} \hline  \rowcolor{red!30}
 Q15& 32P & 64P & 400P  \\ \hline
Capture cost  & 4.47 & 4.52  &  4.64 \\ \hline
 Normal cost  & 2.62  &  2.62 & 2.62  \\ \hline
 PS cost  &  0.52 &  0.34 & 0.104  \\ \hline
\end{tabular}
  \caption{TPC-H Q15 Cost - Postgresql}
  \label{fig:tpch-q15-cost-post}
\end{figure}

%%%%%%%%%%%%% Q15 overhead
\begin{figure}[H]
\centering
 \begin{adjustbox}{max width=1\linewidth}
\begin{tabular}{|c|c|c|} \hline  \rowcolor{red!30}
 Q15 & Lineitem & Supplier  \\ \hline
PS attributes  & l\_suppkey &  s\_suppkey  \\ \hline
Total size &   &    \\ \hline
 Provenance size &  &      \\ \hline
 PS size  (32P) &   &     \\ \hline
 PS size  (64P) &  &    \\ \hline
  PS size  (400P) &   &   \\ \hline
\end{tabular}
 \end{adjustbox}
  \caption{TPC-H Q15 Size - Postgresql}
  \label{fig:tpch-q15-size-post}
\end{figure}

%%%%%%%%%%%%%%%%%%%%%%%%%%%%%%%%%%%%%%%%%%%%%%%%%%%%%%%%%%%%%%%%

%%%%%%%%%%%%%%%%%%%%%%%%%%%%%%%%%%%%%%%%%%%%%%%%%%%%%%%%%%%%%%%%
%% Q16
%%%%%%%%%%%%% Q16 cost
\begin{figure}[H]
\centering
\begin{tabular}{|c|c|c|c|} \hline  \rowcolor{red!30}
 Q16 & 32P & 64P & 400P  \\ \hline
Capture cost  & &  &   \\ \hline
 Normal cost  & 0.78   &  0.78  &  0.78  \\ \hline
 PS cost  &  &  &   \\ \hline
\end{tabular}
  \caption{TPC-H Q16 Cost - Postgresql}
  \label{fig:tpch-q16-cost-post}
\end{figure}

%%%%%%%%%%%%% Q16 overhead
\begin{figure}[H]
\centering
 \begin{adjustbox}{max width=1\linewidth}
\begin{tabular}{|c|c|c|c|} \hline  \rowcolor{red!30}
 Q16 & Partsupp & Part  & Supplier\\ \hline
PS attributes  & l\_orderkey &  p\_partkey & l\_partkey \\ \hline
Total size &  800000 &  200000 &   10000\\ \hline
 Provenance size &  119190&  29810  &   9996\\ \hline
 PS size  (32P) &  800000 &  200000 &  10000  \\ \hline
 PS size  (64P) & 800000 &  200000 &  10000 \\ \hline
  PS size  (400P) & 800000 &  200000 &  10000 \\ \hline
\end{tabular}
 \end{adjustbox}
  \caption{TPC-H Q16 Size - Postgresql}
  \label{fig:tpch-q16-size-post}
\end{figure}

%%%%%%%%%%%%%%%%%%%%%%%%%%%%%%%%%%%%%%%%%%%%%%%%%%%%%%%%%%%%%%%%

%%%%%%%%%%%%%%%%%%%%%%%%%%%%%%%%%%%%%%%%%%%%%%%%%%%%%%%%%%%%%%%%
%% Q17
%%%%%%%%%%%%% Q17 cost
\begin{figure}[H]
\centering
\begin{tabular}{|c|c|c|c|} \hline  \rowcolor{red!30}
 Q17 & 32P & 64P & 400P  \\ \hline
Capture cost  & 4.26 & 4.23  &  4.18 \\ \hline
 Normal cost  & 3.96  &  3.96 & 3.96  \\ \hline
 PS cost  &  3.96 &  3.96 & 2.27  \\ \hline
\end{tabular}
  \caption{TPC-H Q17 Cost - Postgresql}
  \label{fig:tpch-q17-cost-post}
\end{figure}

%%%%%%%%%%%%% Q17 overhead
\begin{figure}[H]
\centering
 \begin{adjustbox}{max width=1\linewidth}
\begin{tabular}{|c|c|c|c|} \hline  \rowcolor{red!30}
 Q17 & Lineitem & Part  & Lineitem\\ \hline
PS attributes  & l\_orderkey &  p\_partkey & l\_partkey \\ \hline
Total size & 6001215  &  200000 &  6001215 \\ \hline
 Provenance size & 591 &  197  & 591  \\ \hline
 PS size  (32P) &  6001215 &  200000  & 6001215 \\ \hline
 PS size  (64P) & 6001215 &  187500 & 5626148 \\ \hline
  PS size  (400P) & 4650929 &  77500 & 2340480  \\ \hline
\end{tabular}
 \end{adjustbox}
  \caption{TPC-H Q17 Size - Postgresql}
  \label{fig:tpch-q17-size-post}
\end{figure}

%%%%%%%%%%%%%%%%%%%%%%%%%%%%%%%%%%%%%%%%%%%%%%%%%%%%%%%%%%%%%%%%

%%%%%%%%%%%%%%%%%%%%%%%%%%%%%%%%%%%%%%%%%%%%%%%%%%%%%%%%%%%%%%%%
%% Q18
%%%%%%%%%%%%% Q18 cost
\begin{figure}[H]
\centering
\begin{tabular}{|c|c|c|c|} \hline  \rowcolor{red!30}
 Q18 & 32P & 64P & 400P  \\ \hline
Capture cost  & 10.98 &  11.15 & 11.77  \\ \hline
 Normal cost  &  5.20 &  5.20 & 5.20  \\ \hline
 PS cost  & 1.03 & 0.63 & 0.13  \\ \hline
\end{tabular}
  \caption{TPC-H Q18 Cost - Postgresql}
  \label{fig:tpch-q18-cost-post}
\end{figure}

%%%%%%%%%%%%% Q18 overhead
\begin{figure}[H]
\centering
 \begin{adjustbox}{max width=1\linewidth}
\begin{tabular}{|c|c|c|c|} \hline  \rowcolor{red!30}
 Q18 & Customer & Orders  & Lineitem\\ \hline
PS attributes  & c\_custkey &  o\_orderkey & l\_orderkey\\ \hline
Total size & 150000  &  1500000 &  6001215 \\ \hline
 Provenance size & 10 &  70  & 70  \\ \hline
 PS size  (32P) &  32812& 328125  & 1312770 \\ \hline
 PS size  (64P) & 21091 &  210938 & 843929 \\ \hline
  PS size  (400P) &3750 &  37500& 150022 \\ \hline
\end{tabular}
 \end{adjustbox}
  \caption{TPC-H Q18 Size - Postgresql}
  \label{fig:tpch-q18-size-post}
\end{figure}

%%%%%%%%%%%%%%%%%%%%%%%%%%%%%%%%%%%%%%%%%%%%%%%%%%%%%%%%%%%%%%%%

%%%%%%%%%%%%%%%%%%%%%%%%%%%%%%%%%%%%%%%%%%%%%%%%%%%%%%%%%%%%%%%%
%% Q19
%%%%%%%%%%%%% Q19 cost
\begin{figure}[H]
\centering
\begin{tabular}{|c|c|c|c|} \hline  \rowcolor{red!30}
 Q19 & 32P & 64P & 400P  \\ \hline
 Capture cost  &  0.165 & 0.165  & 0.165 \\ \hline
  Normal cost  & 0.165 &  0.165 & 0.165 \\ \hline
 PS cost  & 0.164 & 0.152 & 0.087 \\ \hline
%Capture cost  &  0.19 & 0.20  & 0.24 \\ \hline
% Normal cost  & 0.19  &  0.19 & 0.19 \\ \hline
% PS cost  & 0.19 & 0.17 & 0.09 \\ \hline
\end{tabular}
  \caption{TPC-H Q19 Cost - Postgresql}
  \label{fig:tpch-q19-cost-post}
\end{figure}

%%%%%%%%%%%%% Q19 overhead
\begin{figure}[H]
\centering
 \begin{adjustbox}{max width=1\linewidth}
\begin{tabular}{|c|c|c|} \hline  \rowcolor{red!30}
 Q19  & Part  & Lineitem\\ \hline
PS attributes   &  p\_partkey & l\_orderkey\\ \hline
Total size &  200000 & 6001215 \\ \hline
 Provenance size &   103 & 121  \\ \hline
 PS size  (32P) &  200000  &  5813679\\ \hline
 PS size  (64P) &  153125  & 5063532 \\ \hline
  PS size  (400P) &  44499 & 1455285 \\ \hline
\end{tabular}
 \end{adjustbox}
  \caption{TPC-H Q19 Size - Postgresql}
  \label{fig:tpch-q19-size-post}
\end{figure}

%%%%%%%%%%%%%%%%%%%%%%%%%%%%%%%%%%%%%%%%%%%%%%%%%%%%%%%%%%%%%%%%

%\xn{\\
%Q19 64 partition $0.33 > 0.25$ Seq Scan on additional condition add the cost}

%%%%%%%%%%%%%%%%%%%%%%%%%%%%%%%%%%%%%%%%%%%%%%%%%%%%%%%%%%%%%%%%
%% Q20
%%%%%%%%%%%%% Q20 cost
\begin{figure}[H]
\centering
\begin{tabular}{|c|c|c|c|} \hline  \rowcolor{red!30}
 Q20 & 32P & 64P & 400P  \\ \hline
 Capture cost  &   &  &  \\ \hline
  Normal cost  & 2.45 & 2.45   & 2.45   \\ \hline
 PS cost & &    &  2.0 \\ \hline
%Capture cost  &  0.19 & 0.20  & 0.24 \\ \hline
% Normal cost  & 0.19  &  0.19 & 0.19 \\ \hline
% PS cost  & 0.19 & 0.17 & 0.09 \\ \hline
\end{tabular}
  \caption{TPC-H Q20 Cost - Postgresql}
  \label{fig:tpch-q20-cost-post}
\end{figure}

%%%%%%%%%%%%% Q19 overhead
\begin{figure}[H]
\centering
 \begin{adjustbox}{max width=1\linewidth}
\begin{tabular}{|c|c|c|c|c|c|} \hline  \rowcolor{red!30}
 Q20  & Supplier & Part  & Lineitem  & Partsupp & nation\\ \hline
PS attributes  & s\_suppkey &  o\_partkey & l\_orderkey &  ps\_partkey, ps\_suppkey, both & n\_nationkey \\ \hline
Total size & 10000 &  200000 & 6001215 & 800000 & 25 \\ \hline
 Provenance size & 197  & 247 & 2052 & 257 & 1 \\ \hline
 PS size  (32P) &  10000  &  200000&   6001215&  800000 & 1\\ \hline
 PS size  (64P) &  9218  & 196875 &  6001215 & 787500, 737440, 725897 & 1\\ \hline
  PS size  (400P) &3924  &  93000 &  3690747 & 372000, 313920, 146937& 1 \\ \hline
\end{tabular}
 \end{adjustbox}
  \caption{TPC-H Q20 Size - Postgresql}
  \label{fig:tpch-q20-size-post}
\end{figure}

%%%%%%%%%%%%%%%%%%%%%%%%%%%%%%%%%%%%%%%%%%%%%%%%%%%%%%%%%%%%%%%%

%%%%%%%%%%%%%%%%%%%%%%%%%%%%%%%%%%%%%%%%%%%%%%%%%%%%%%%%%%%%%%%%
%% Q21
%%%%%%%%%%%%% Q21 cost
\begin{figure}[H]
\centering
\begin{tabular}{|c|c|c|c|} \hline  \rowcolor{red!30}
 Q21 & 32P & 64P & 400P  \\ \hline
 Capture cost  &   &  &  \\ \hline
  Normal cost  & 21.84 &  21.84  & 21.84  \\ \hline
 PS cost & 21.84 &  21.84  & 21.84  \\ \hline
%Capture cost  &  0.19 & 0.20  & 0.24 \\ \hline
% Normal cost  & 0.19  &  0.19 & 0.19 \\ \hline
% PS cost  & 0.19 & 0.17 & 0.09 \\ \hline
\end{tabular}
  \caption{TPC-H Q21 Cost - Postgresql}
  \label{fig:tpch-q21-cost-post}
\end{figure}

%%%%%%%%%%%%% Q19 overhead
\begin{figure}[H]
\centering
 \begin{adjustbox}{max width=1\linewidth}
\begin{tabular}{|c|c|c|c|c|} \hline  \rowcolor{red!30}
 Q21  & Supplier & Orders  & Lineitem  & nation \\ \hline
PS attributes  & s\_suppkey &  o\_orderkey & l\_orderkey & n\_nationkey \\ \hline
Total size & 10000 &  1500000 & 6001215 & 25\\ \hline
 Provenance size &  100 & 1380&  1380& 1 \\ \hline
 PS size  (32P) &   9375 & 1500000 &  6001215 & 1 \\ \hline
 PS size  (64P) &   7809 & 1500000&  6001215& 1\\ \hline
  PS size  (400P) & 2224 & 1458750  & 5851188 & 1\\ \hline
\end{tabular}
 \end{adjustbox}
  \caption{TPC-H Q21 Size - Postgresql}
  \label{fig:tpch-q21-size-post}
\end{figure}

%%%%%%%%%%%%%%%%%%%%%%%%%%%%%%%%%%%%%%%%%%%%%%%%%%%%%%%%%%%%%%%%

%%%%%%%%%%%%% Q22 overhead
\begin{figure}[H]
\centering
 \begin{adjustbox}{max width=1\linewidth}
\begin{tabular}{|c|c|} \hline  \rowcolor{red!30}
 Q22  & Customer \\ \hline
PS attributes  & c\_custkey  \\ \hline
Total size & 150000 \\ \hline
num distinct in prov &  6443  \\ \hline
\end{tabular}
 \end{adjustbox}
  \caption{TPC-H Q22 Size - Postgresql}
  \label{fig:tpch-q22-size-post}
\end{figure}

%%%%%%%%%%%%%%%%%%%%%%%%%%%%%%%%%%%%%%%%%%%%%%%%%%%%%%%%%%%%%%%%

\parttitle{Postgres + Completly synthetic}

%%%q1 range
%%%%%%%%%%%%%%%%%%%%%%%%%%%%%%%%%%%%%%%%
 \begin{figure}[H]
   \centering
   \includegraphics[width=0.8\linewidth,trim=0pt 0pt 0 0pt, clip]{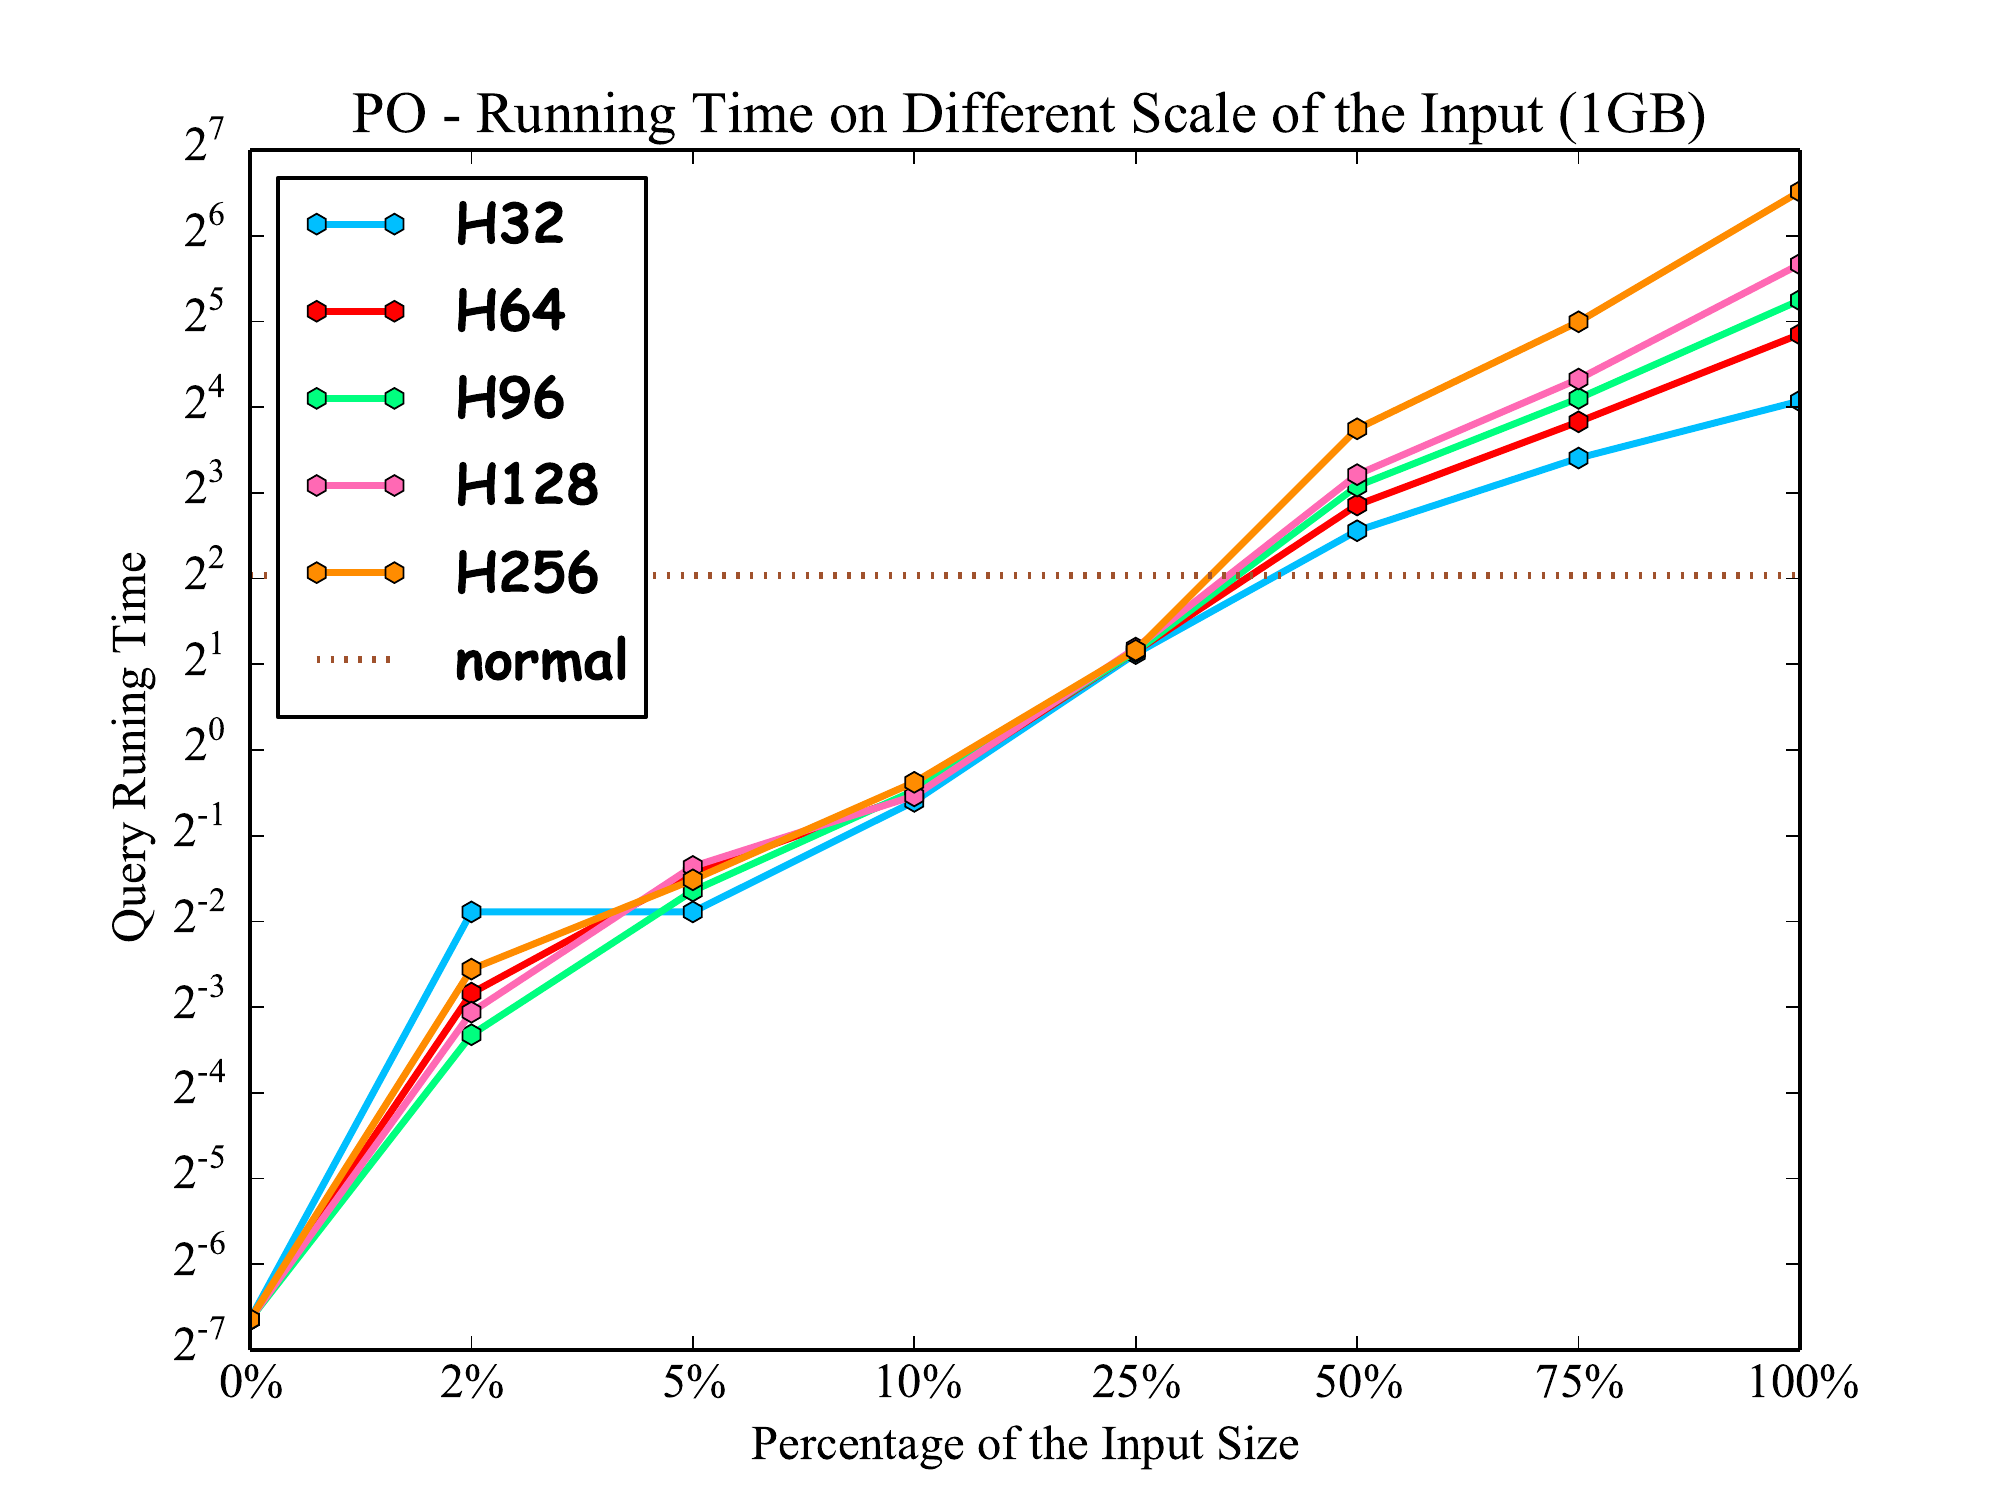}
   \caption{PostgreSQL + Virtual sketches + Index + Range +  Completly synthetic for Q1 on 1GB dataset}
    \label{fig:post-fv-r-cs-q1-1gb}
 \end{figure}
%%%%%%%%%%%%%%%%%%%%%%%%%%%%%%%%%%%%%%%%

%%%q2 range
%%%%%%%%%%%%%%%%%%%%%%%%%%%%%%%%%%%%%%%%
 \begin{figure}[H]
   \centering
   \includegraphics[width=0.8\linewidth,trim=0pt 0pt 0 0pt, clip]{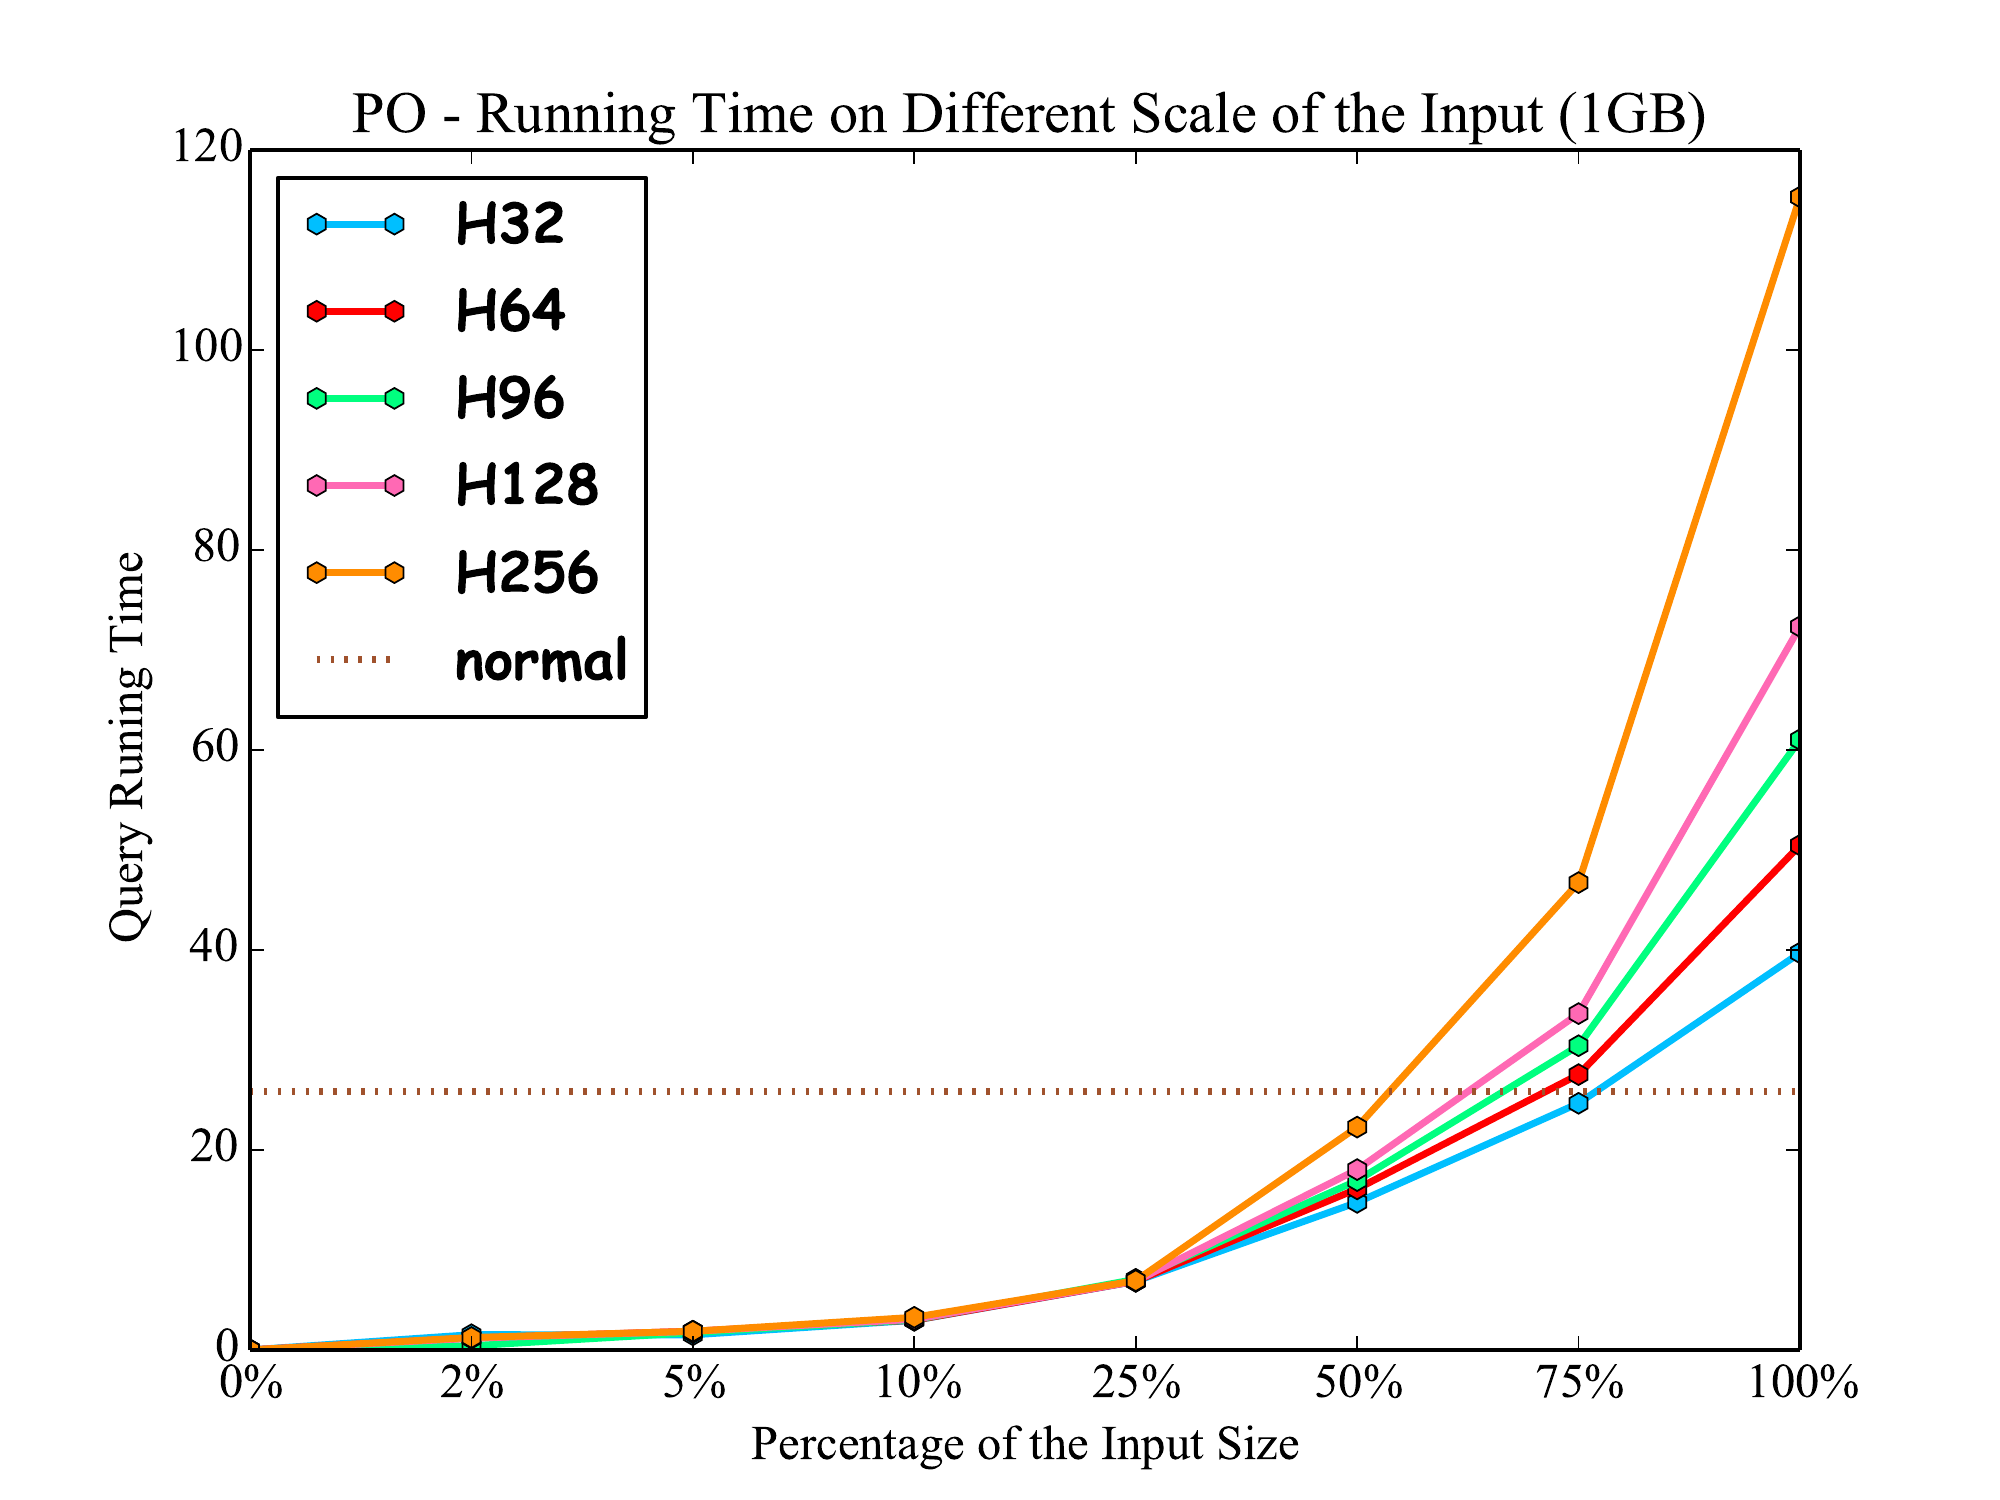}
   \caption{PostgreSQL + Virtual sketches + Index + Range +  Completly synthetic for Q2 on 1GB dataset}
   \label{fig:post-fv-r-cs-q2-1gb}
 \end{figure}
%%%%%%%%%%%%%%%%%%%%%%%%%%%%%%%%%%%%%%%%

%%%q3 range apply ps on both inside and outside
%%%%%%%%%%%%%%%%%%%%%%%%%%%%%%%%%%%%%%%%
 \begin{figure}[H]
   \centering
   \includegraphics[width=0.8\linewidth,trim=0pt 0pt 0 0pt, clip]{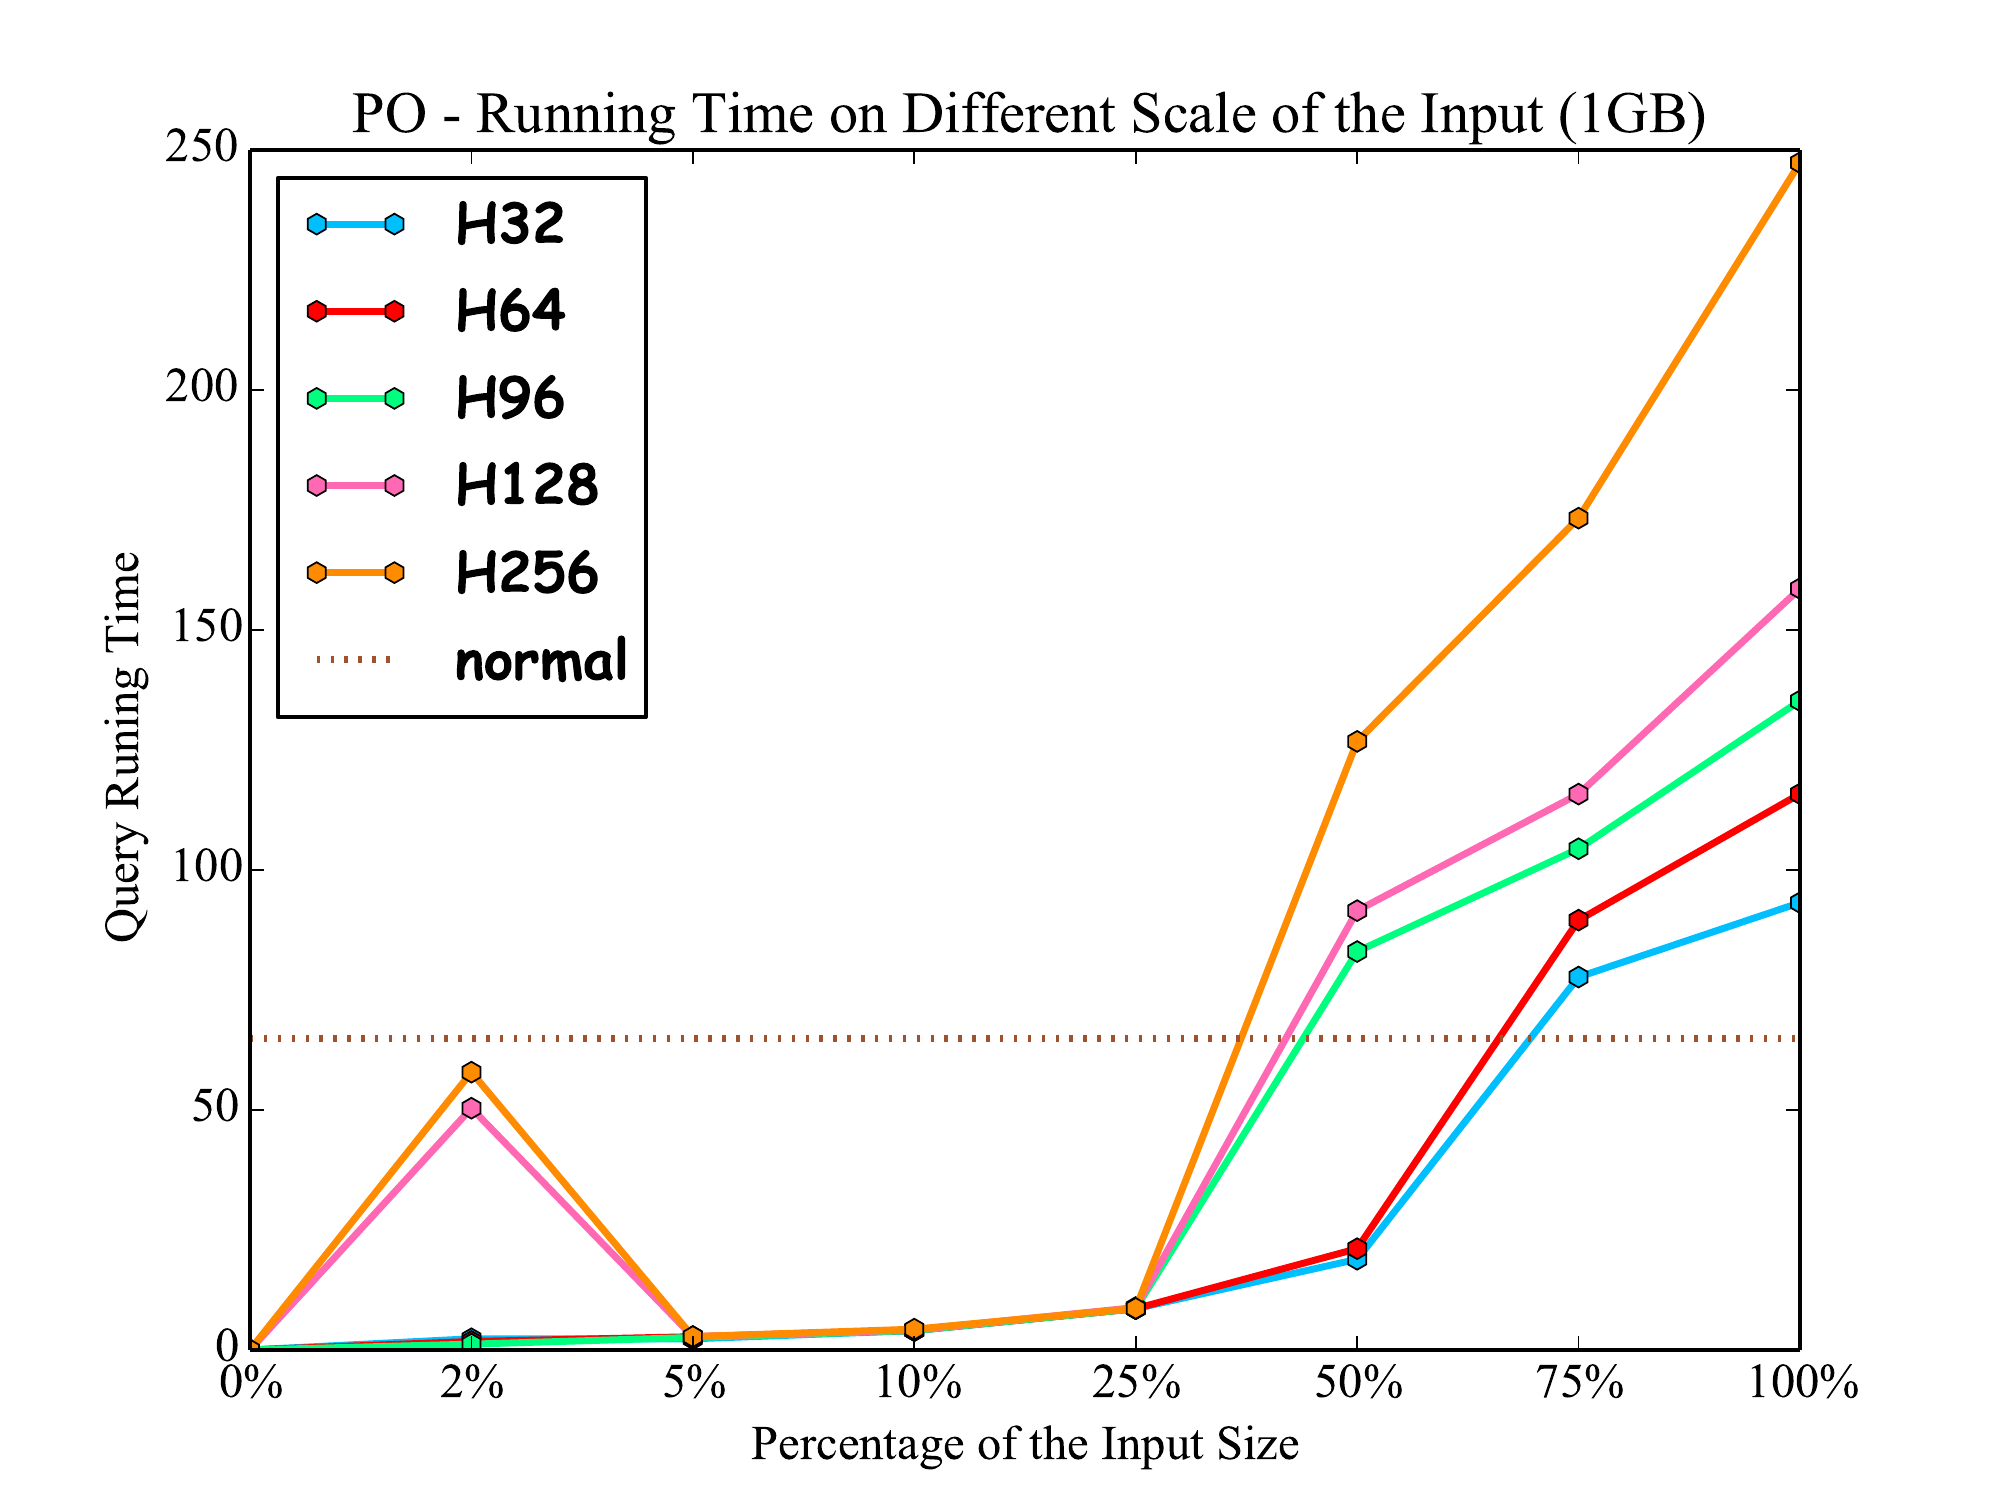}
   \caption{PostgreSQL + Virtual sketches + Index + Range +  Completly synthetic for Q3 (ps on both inside and outside) on 1GB dataset}
   \label{fig:post-fv-r-cs-q3-1gb-both}
 \end{figure}
%%%%%%%%%%%%%%%%%%%%%%%%%%%%%%%%%%%%%%%%

%%%q3 range apply ps on inside 
%%%%%%%%%%%%%%%%%%%%%%%%%%%%%%%%%%%%%%%%
 \begin{figure}[H]
   \centering
   \includegraphics[width=0.8\linewidth,trim=0pt 0pt 0 0pt, clip]{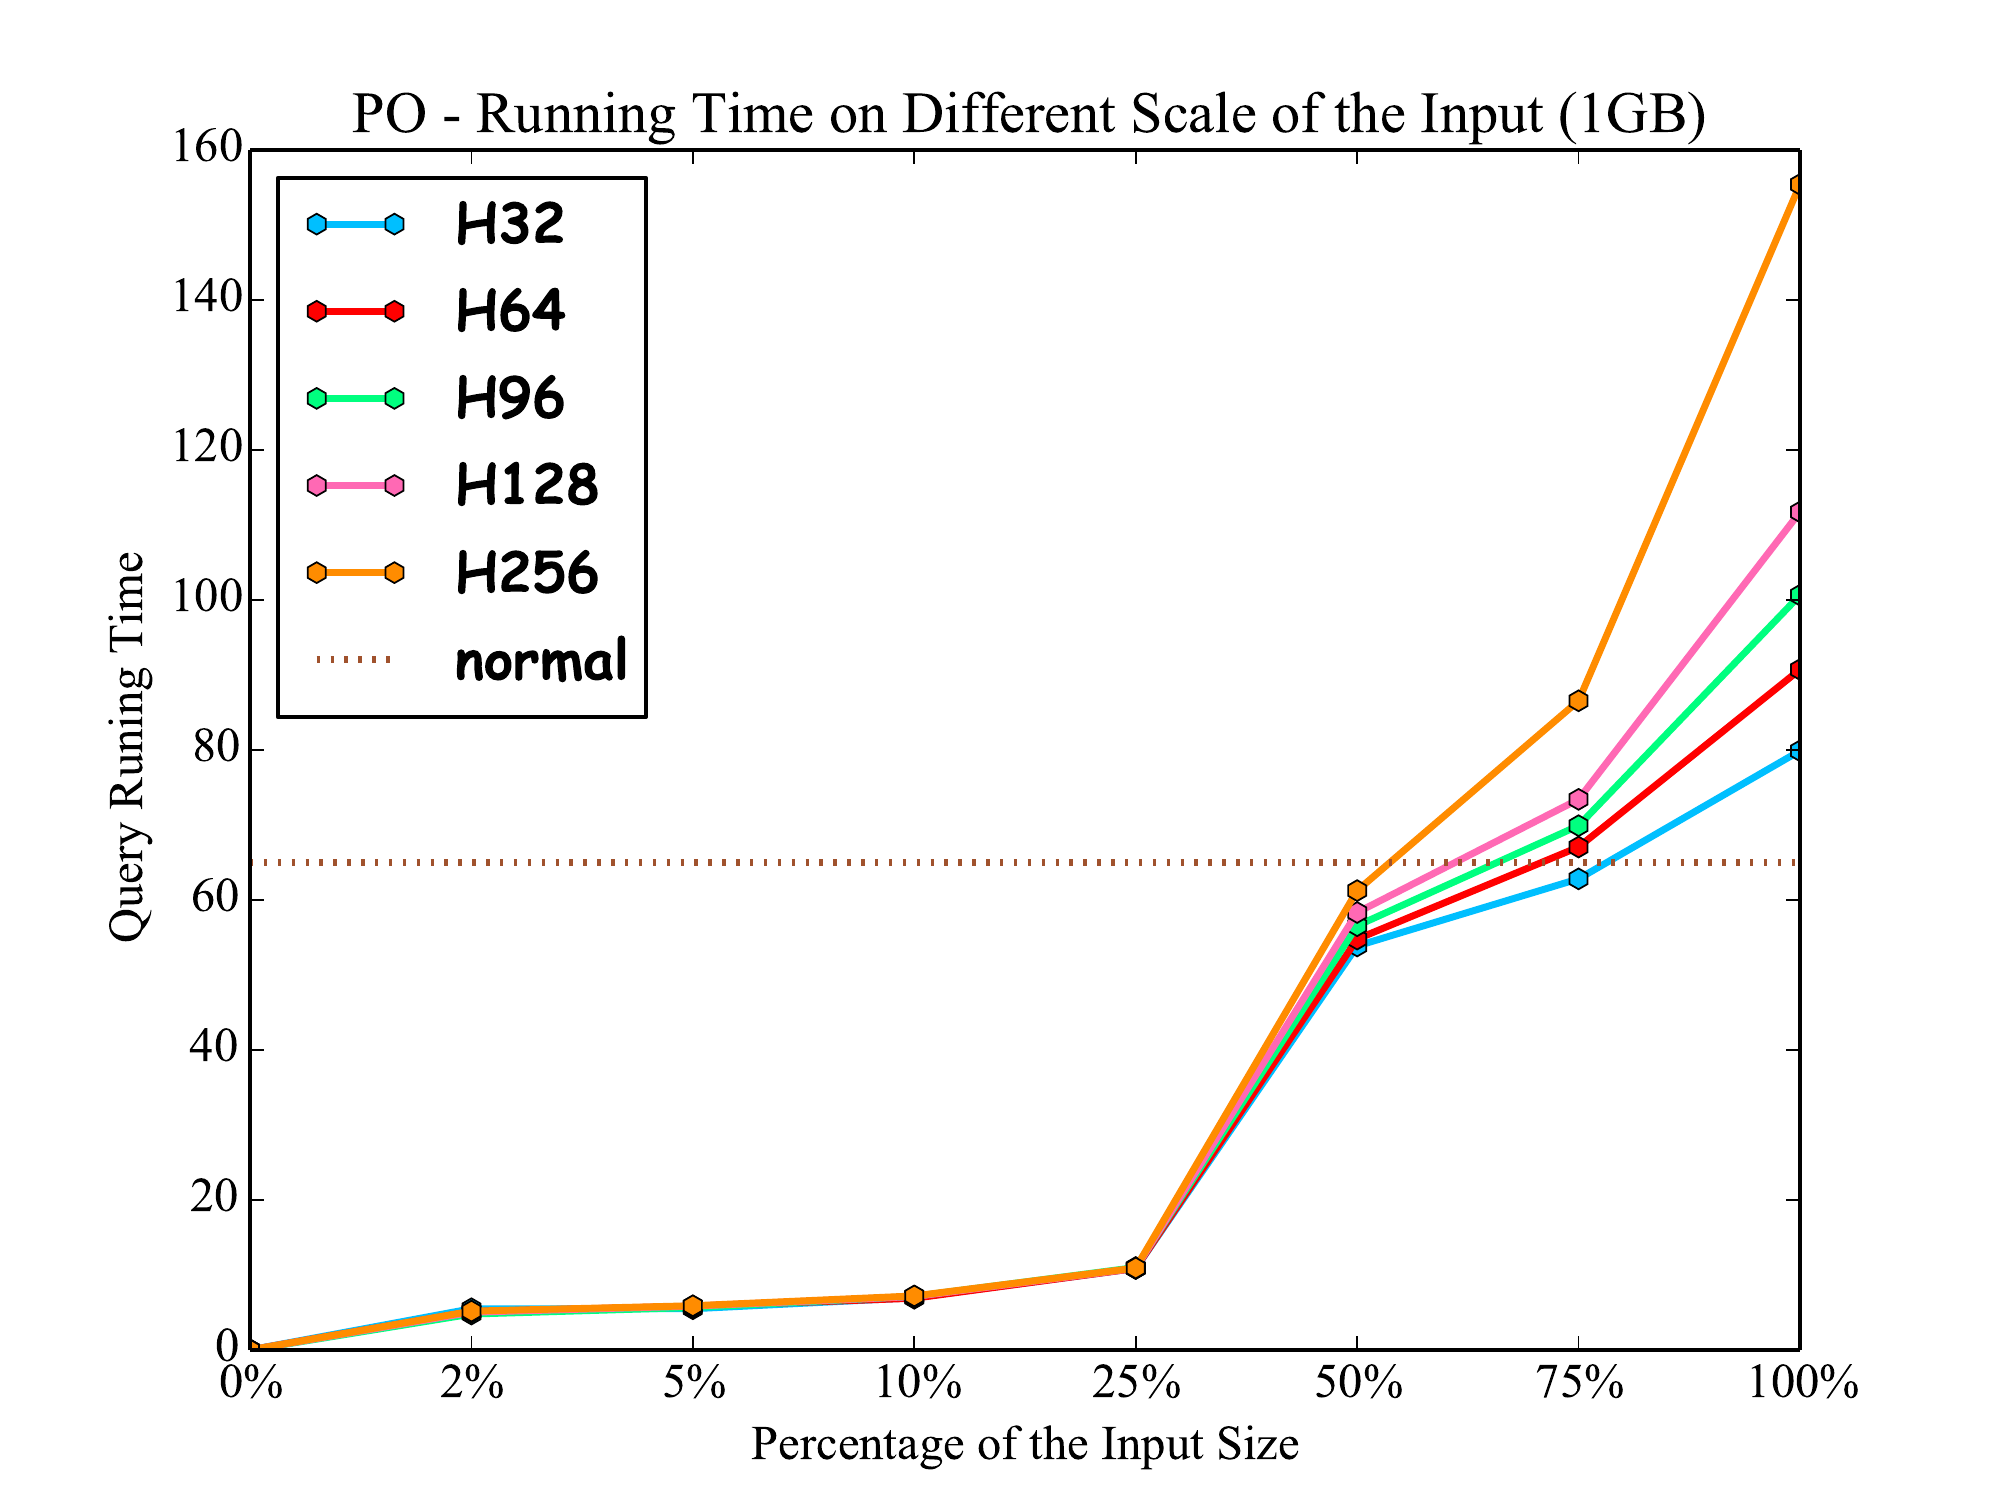}
   \caption{PostgreSQL + Virtual sketches + Index + Range +  Completly synthetic for Q3 (ps only on inside) on 1GB dataset}
   \label{fig:post-fv-r-cs-q3-1gb-in}
 \end{figure}
%%%%%%%%%%%%%%%%%%%%%%%%%%%%%%%%%%%%%%%%

\xn{below is oracle result}

\parttitle{Hash + Completly synthetic} 
Test Q1, Q2 on 1GB and 10GB datasets.

%%%%%%%%%%%%%%%%%%%%%%%%%%%%%%%%%%%%%%%%%%%%%%%%%%%%%%%%%%%%%%%%%%%%%%%%
%%%%%%%%%%%%%%%%%%%%%%%%%%%%%%%%%%%%%%%%%%%%%%%%%%%%%%%%%%%%%%%%%%%%%%%%
%% h->hash, r->range
%% cs->Completly synthetic 
%% fv->Fully virtual sketches
%% ph->physical sketches
%% idx->index
%% pre-h -> pre-hash and store the hashed value in a column, directly use this column
%%%%%%%%%%%%%%%%%%%%%%%%%%%%%%%%%%%%%%%%
%%%%q1
%%%%%%%%%%%%%%%%%%%%%%%%%%%%%%%%%%%%%%%%
%%%%q1 hash
%%%%%%%%%%%%%%%%%%%%%%%%%%%%%%%%%%%%%%%%
 \begin{figure}[H]
   \centering
   \includegraphics[width=0.8\linewidth,trim=0pt 0pt 0 0pt, clip]{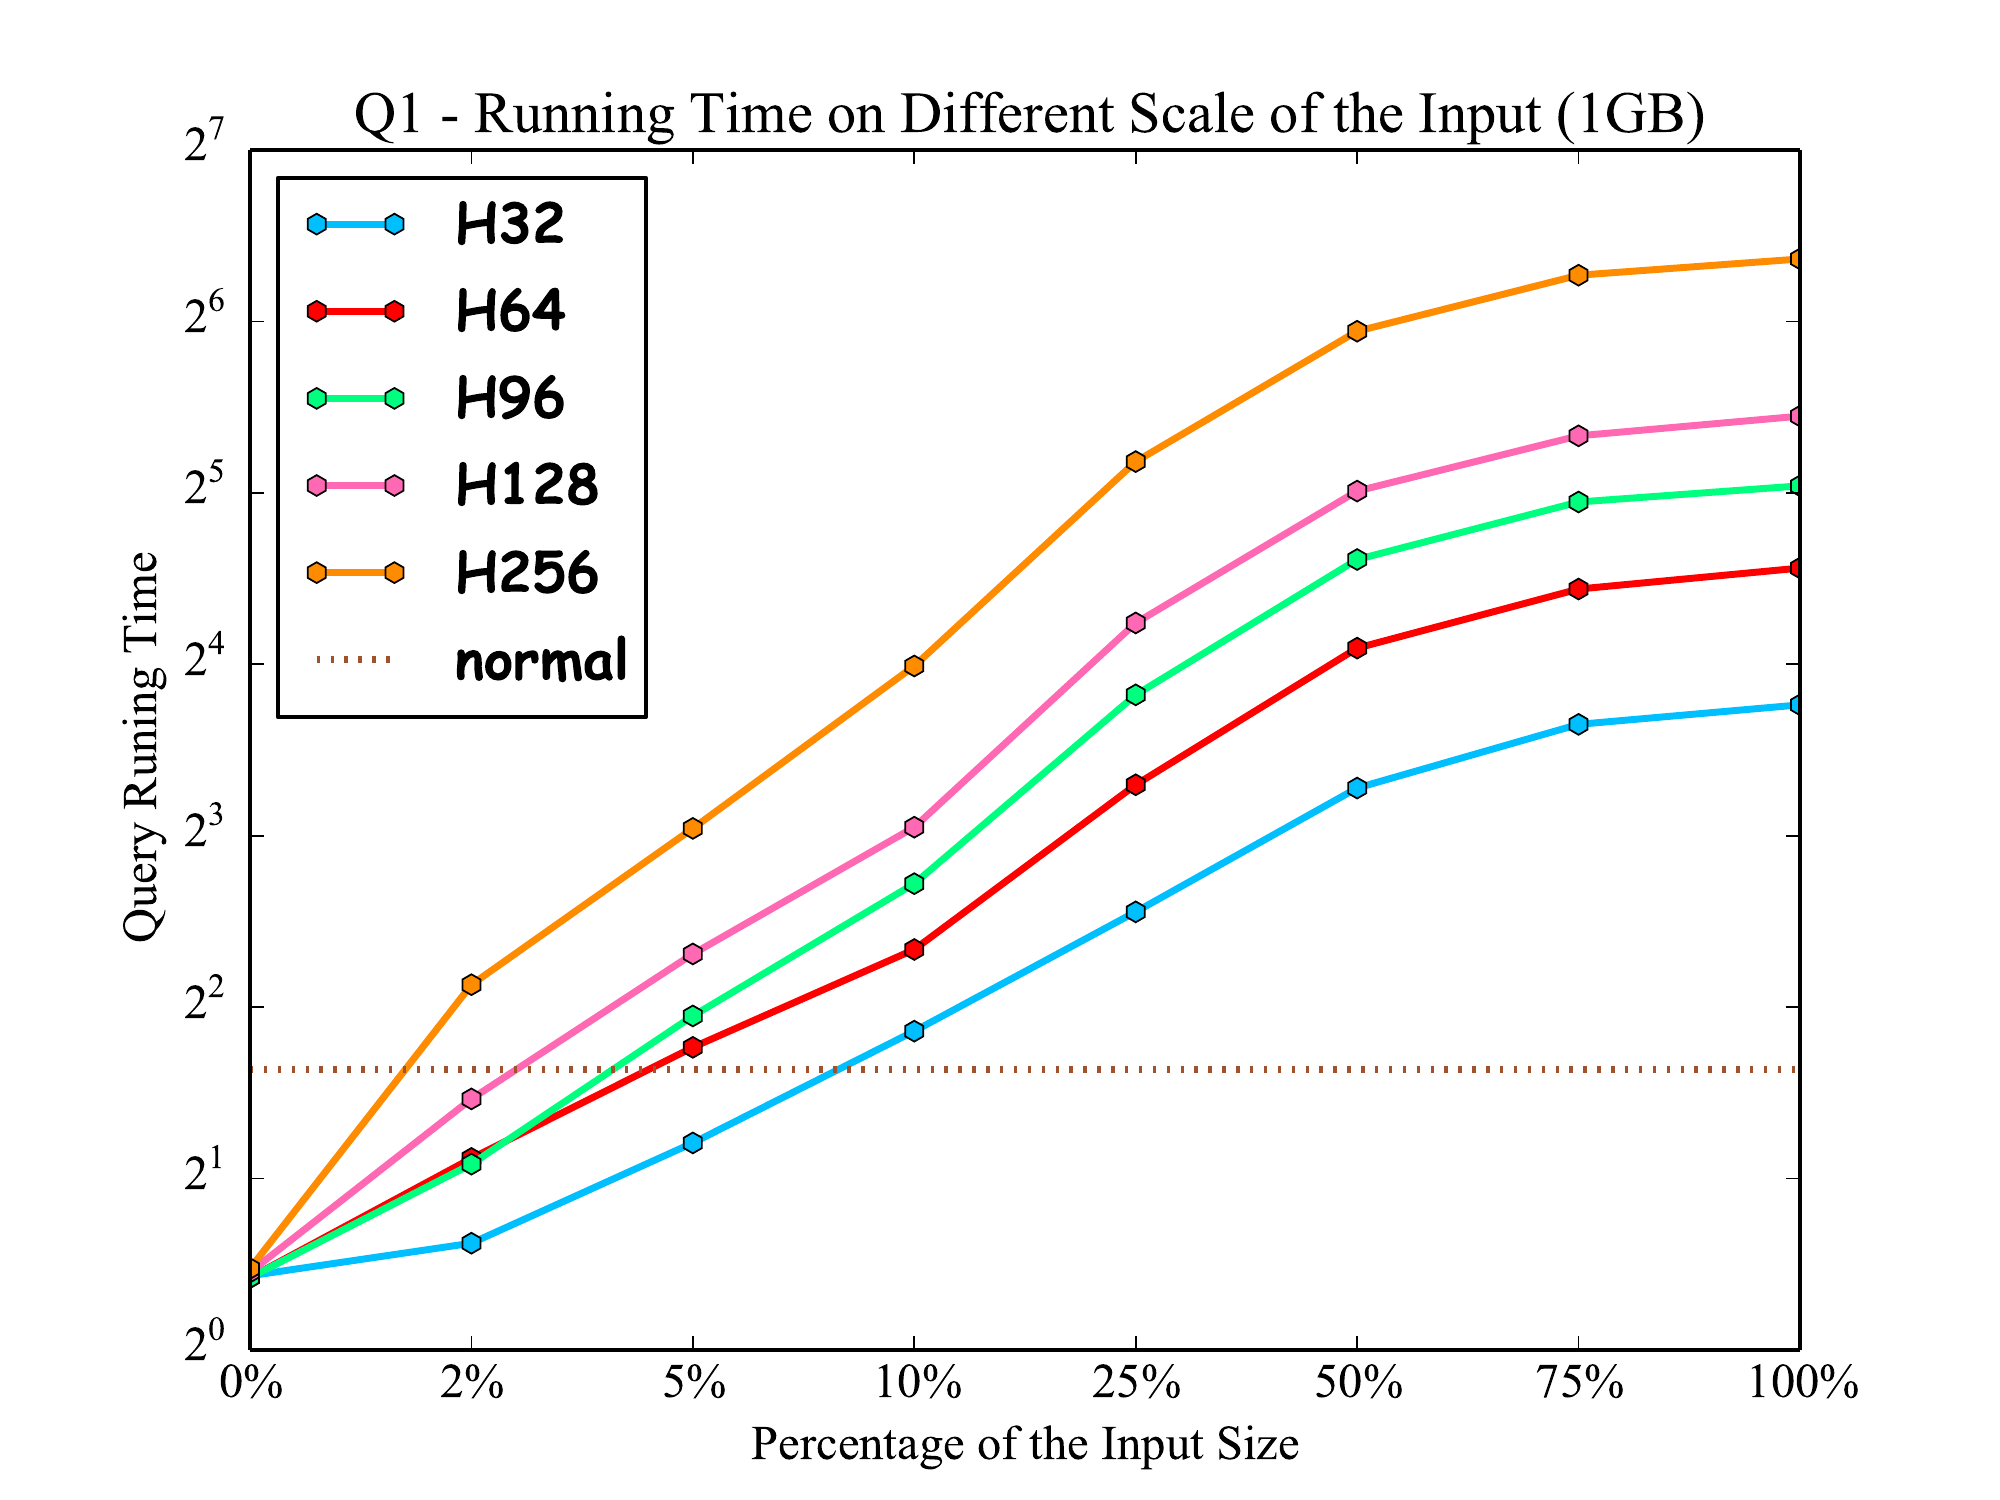}
   \caption{Fully virtual sketches + Hash +  Completly synthetic for Q1 on 1GB dataset}
   \label{fig:fv-h-cs-q1-1gb}
 \end{figure}
%%%%%%%%%%%%%%%%%%%%%%%%%%%%%%%%%%%%%%%%

%%%%%%%%%%%%%%%%%%%%%%%%%%%%%%%%%%%%%%%%%
% \begin{figure}[H]
%   \centering
%   \includegraphics[width=0.8\linewidth,trim=0pt 0pt 0 0pt, clip]{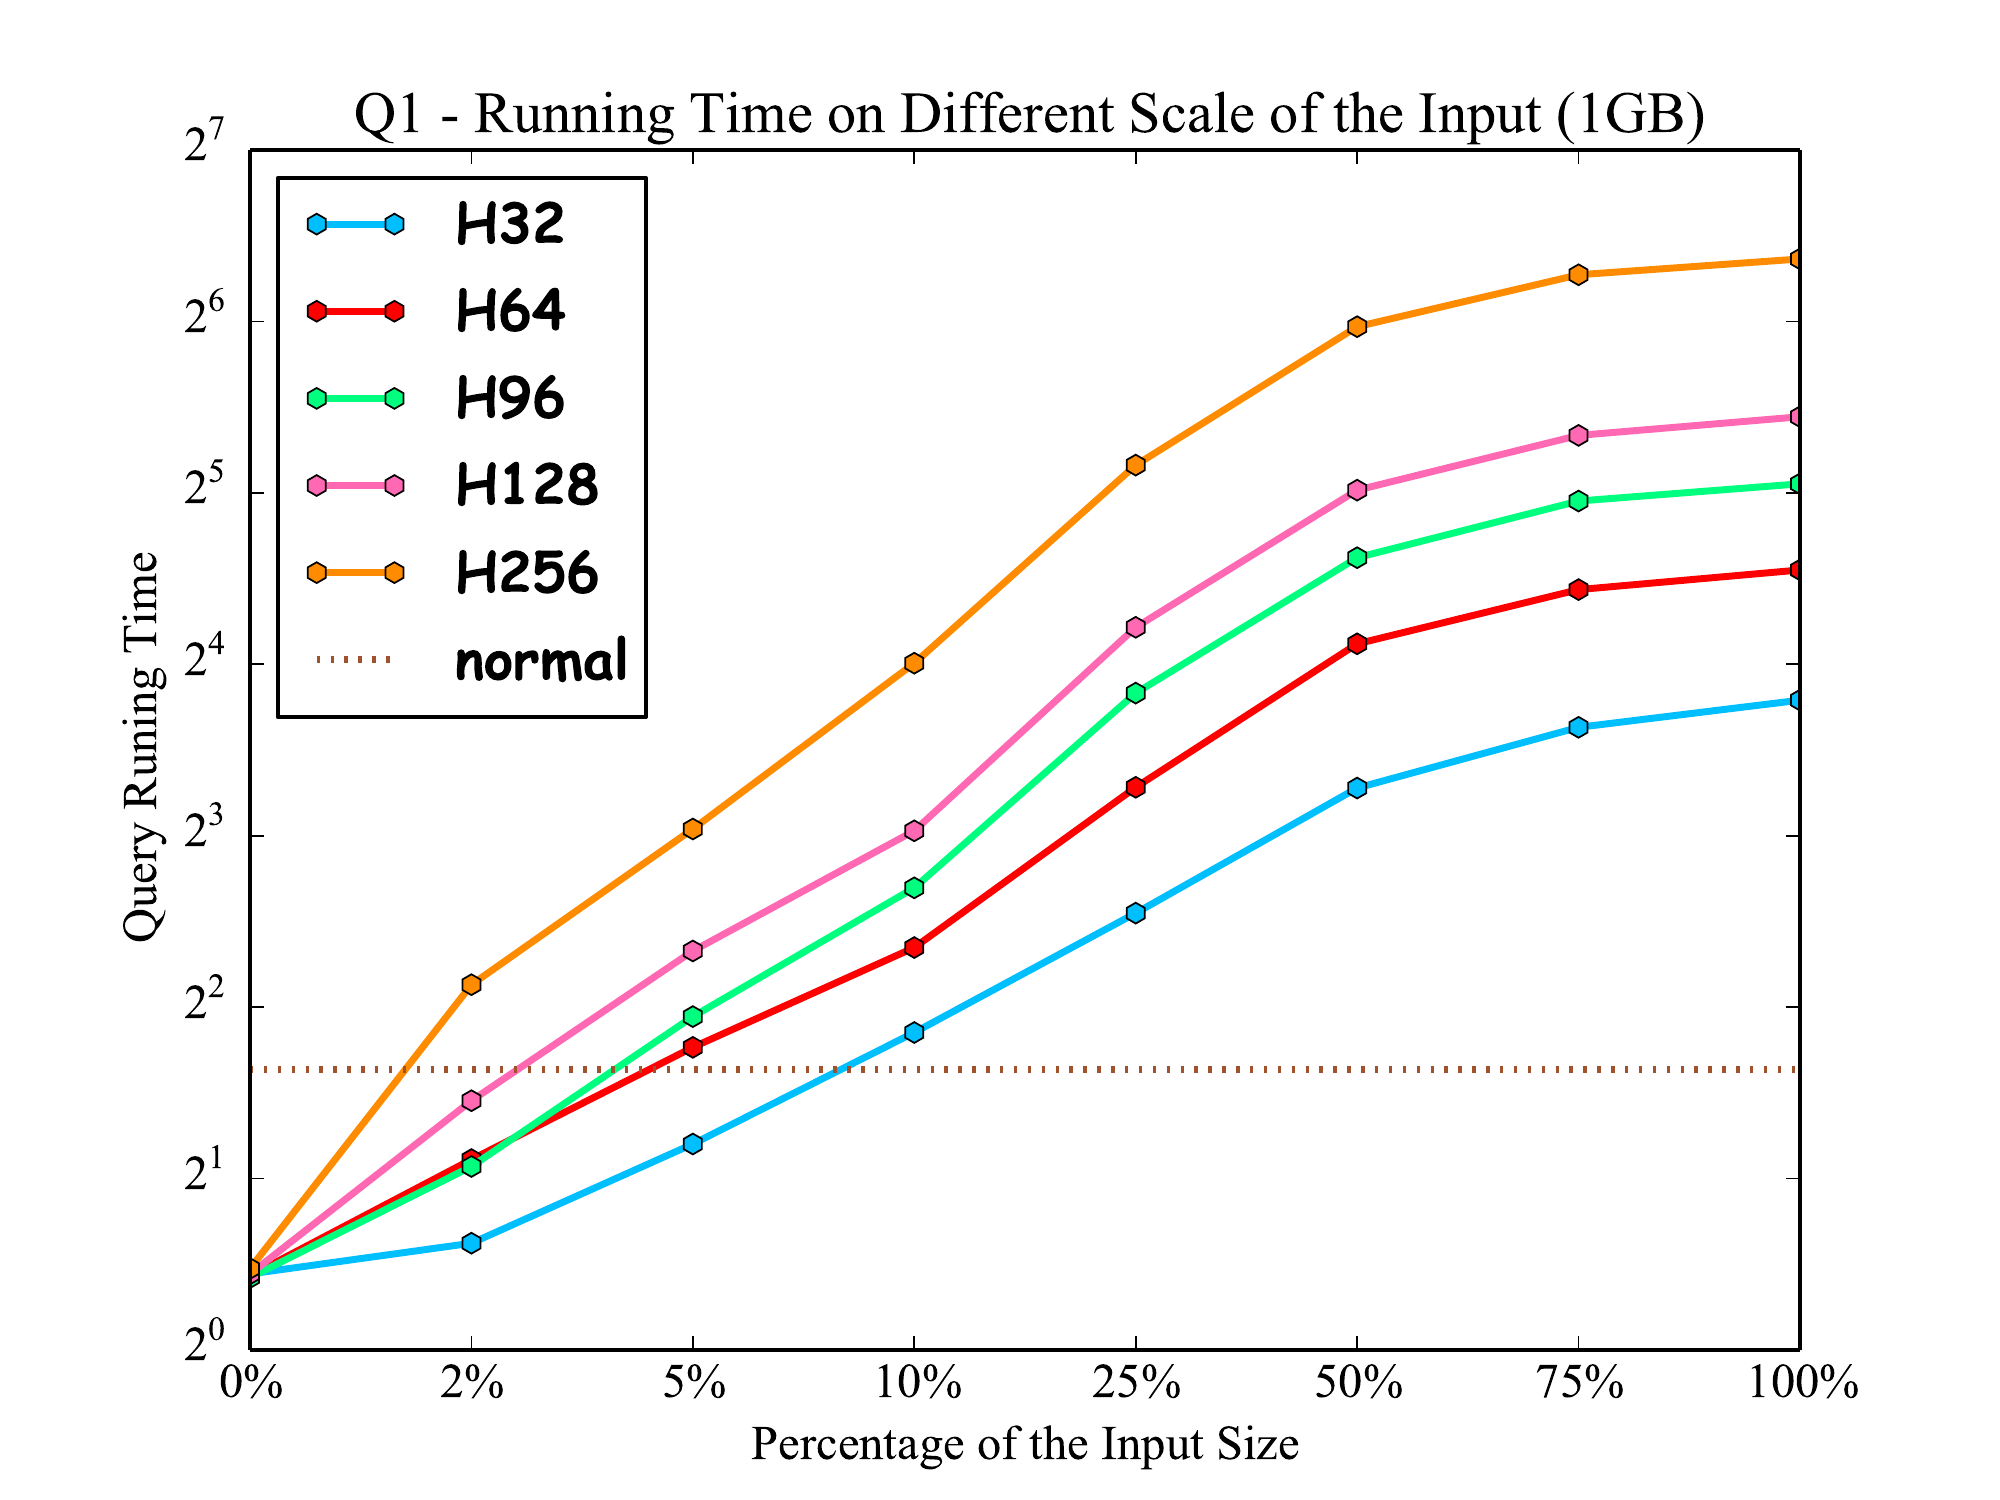}
%   \caption{Fully virtual sketches + Hash + index +  Completly synthetic for Q1 on 1GB dataset}
%   \label{fig:fv-h-idx-cs-q1-1gb}
% \end{figure}
%%%%%%%%%%%%%%%%%%%%%%%%%%%%%%%%%%%%%%%%%

%%%%%%%%%%%%%%%%%%%%%%%%%%%%%%%%%%%%%%%%
 \begin{figure}[H]
   \centering
   \includegraphics[width=0.8\linewidth,trim=0pt 0pt 0 0pt, clip]{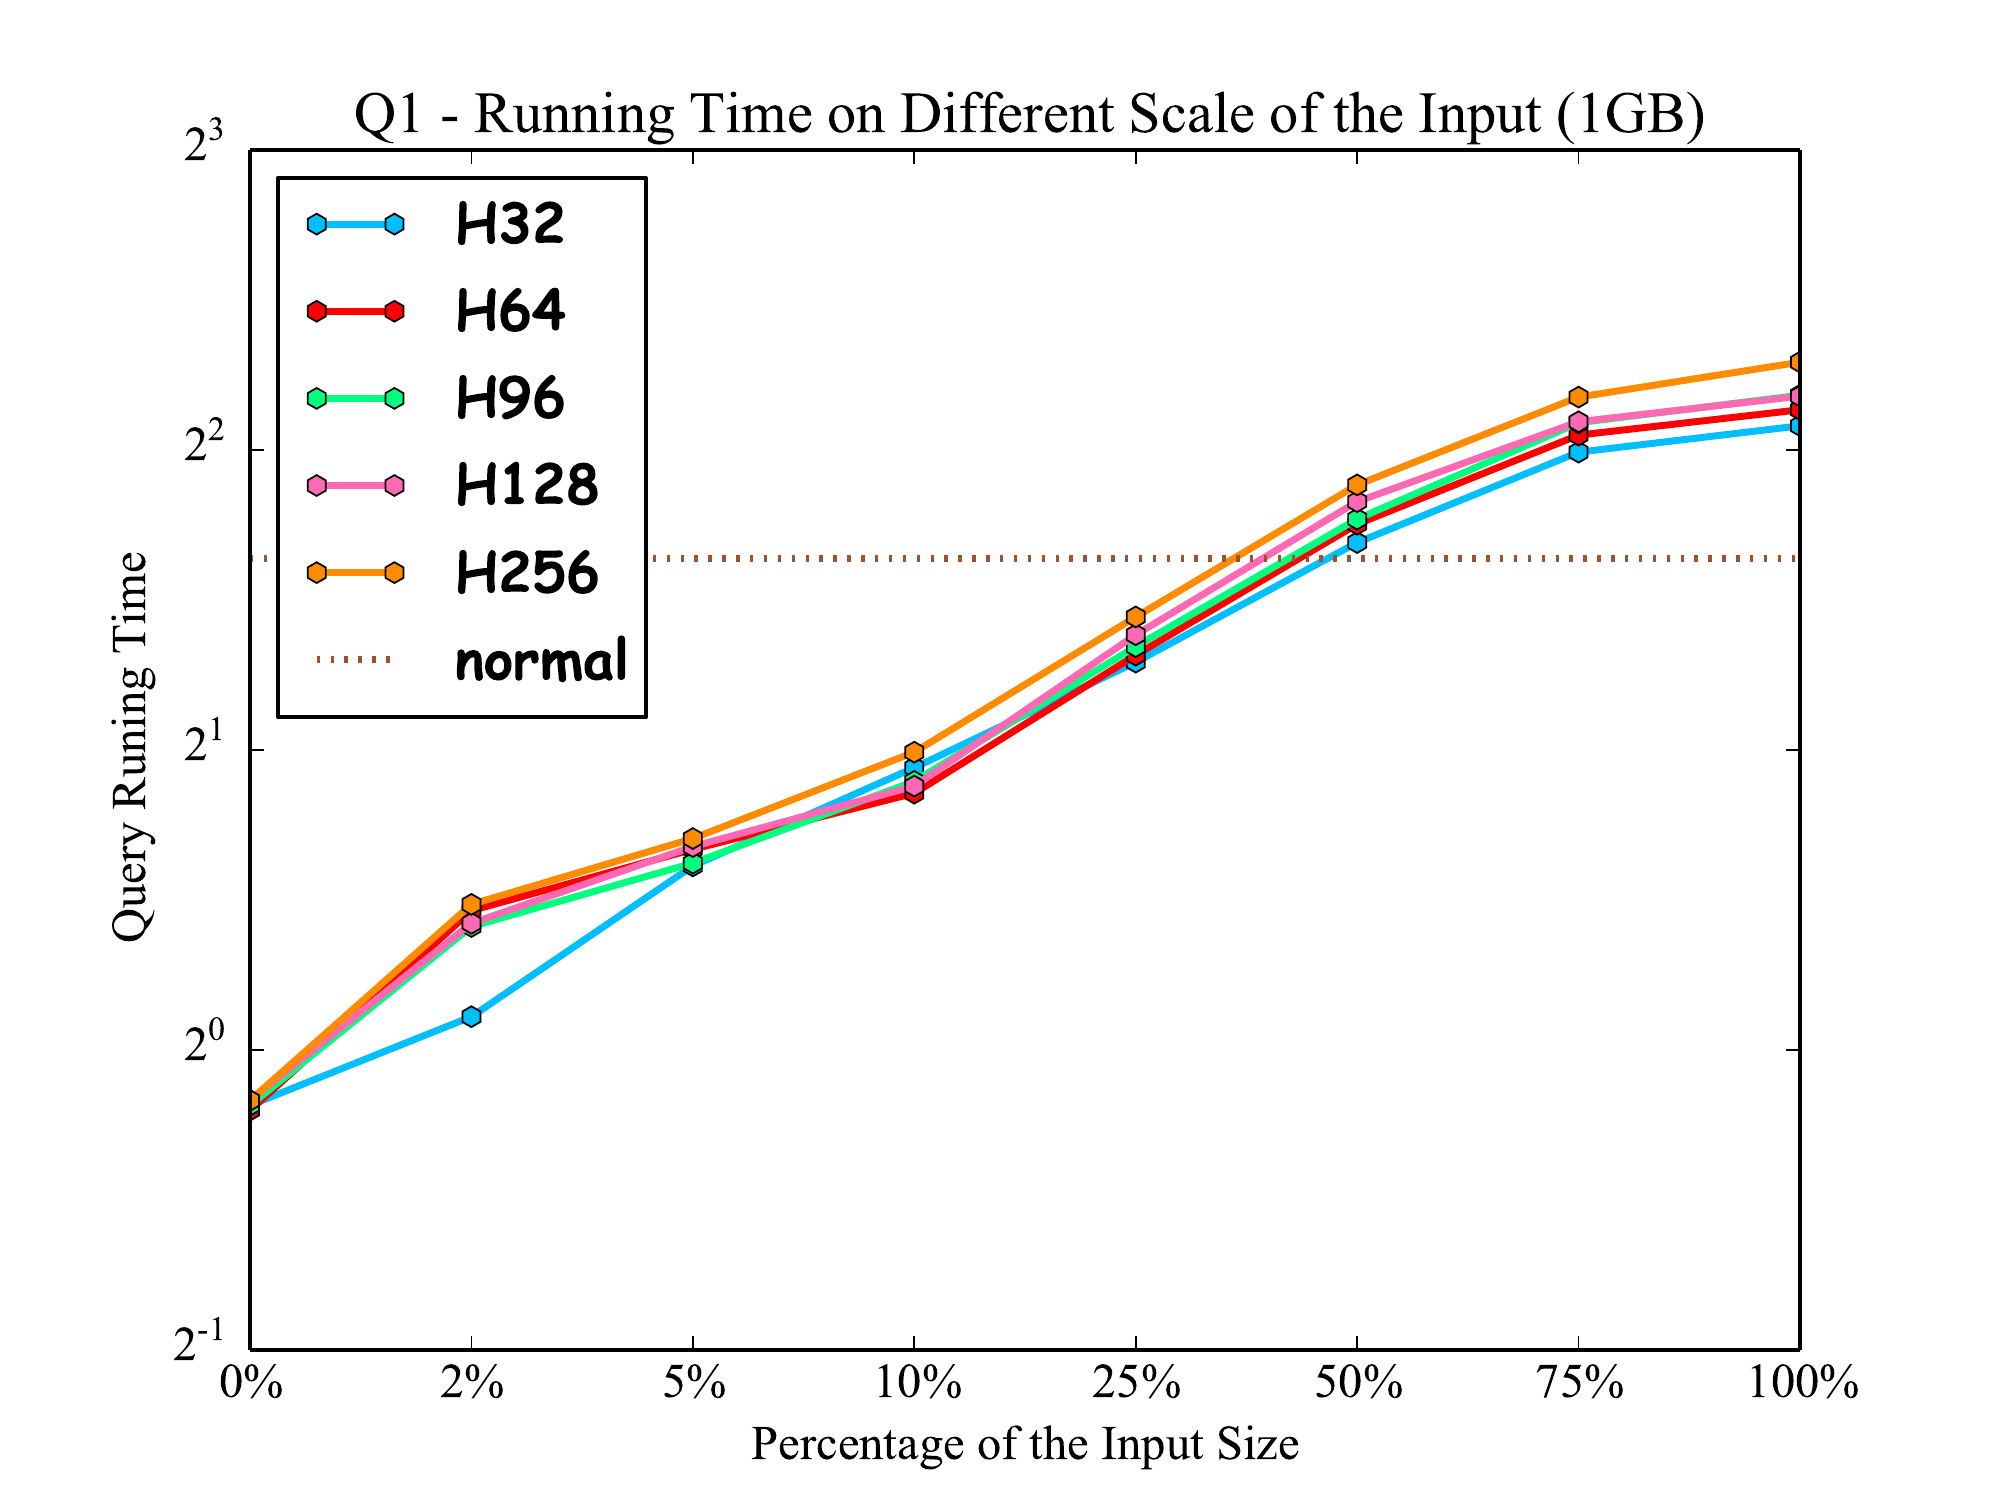}
   \caption{Fully virtual sketches + Pre-Hash +  Completly synthetic for Q1 on 1GB dataset}
   \label{fig:fv-pre-h-cs-q1-1gb}
 \end{figure}
%%%%%%%%%%%%%%%%%%%%%%%%%%%%%%%%%%%%%%%%

%%%%%%%%%%%%%%%%%%%%%%%%%%%%%%%%%%%%%%%%%
% \begin{figure}[H]
%   \centering
%   \includegraphics[width=0.8\linewidth,trim=0pt 0pt 0 0pt, clip]{figs/all/q1_hash_column_index_1gb.pdf}
%   \caption{Fully virtual sketches + Pre-Hash + index +  Completly synthetic for Q1 on 1GB dataset}
%   \label{fig:fv-pre-h-idx-cs-q1-1gb}
% \end{figure}
%%%%%%%%%%%%%%%%%%%%%%%%%%%%%%%%%%%%%%%%%

%%%%%%%%%%%%%%%%%%%%%%%%%%%%%%%%%%%%%%%%
 \begin{figure}[H]
   \centering
   \includegraphics[width=0.8\linewidth,trim=0pt 0pt 0 0pt, clip]{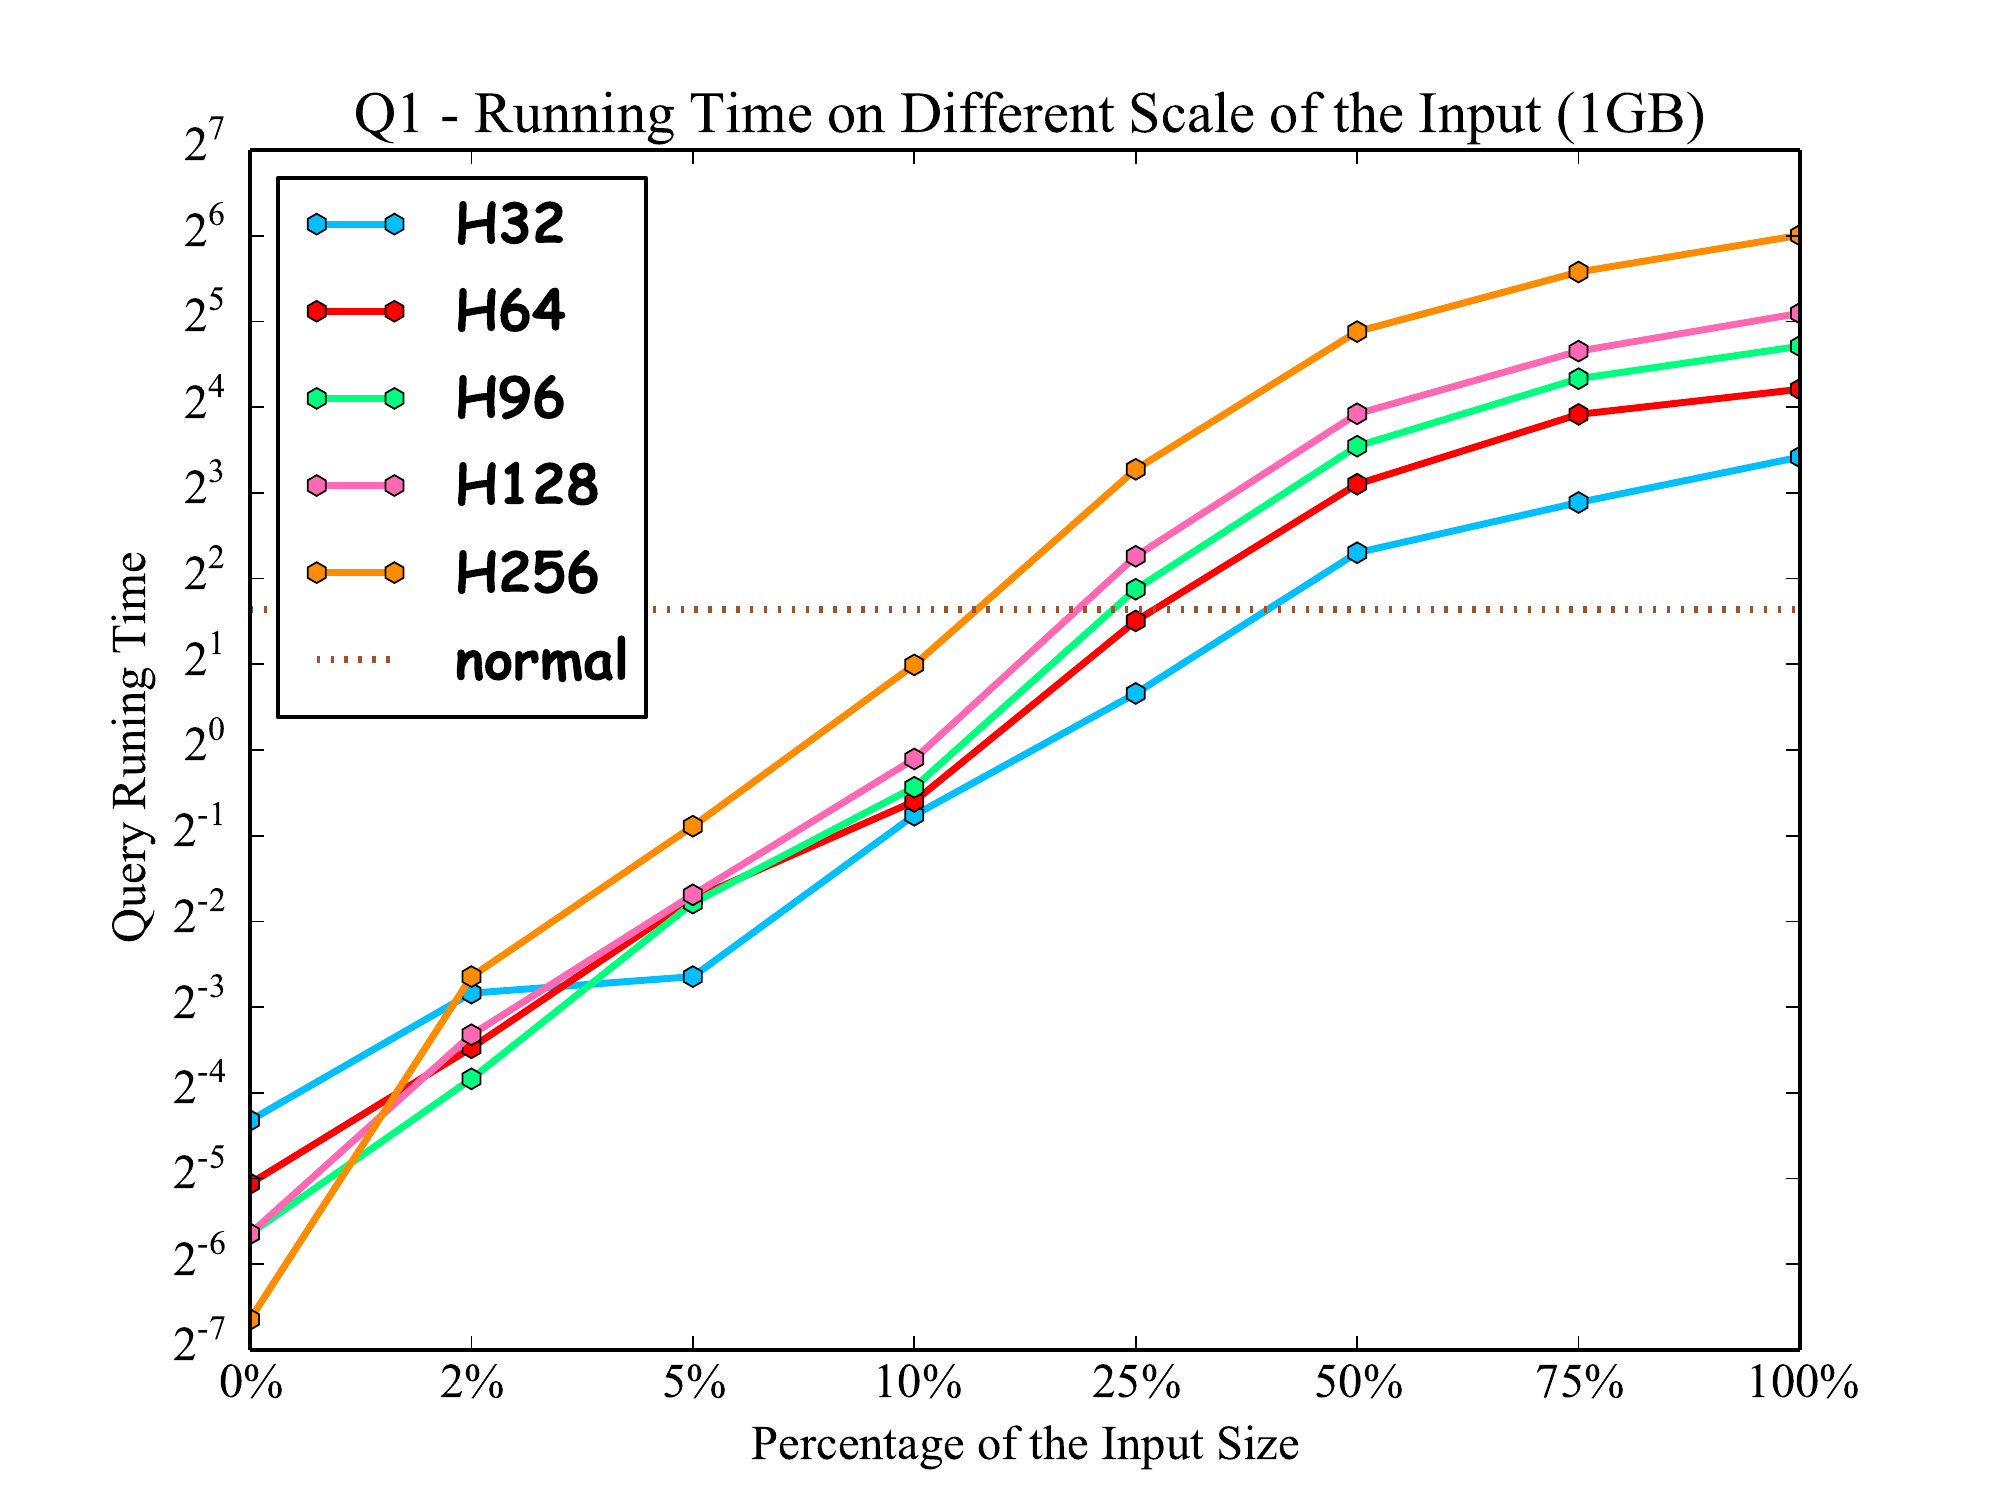}
   \caption{Physical sketches + Pre-Hash +  Completly synthetic for Q1 on 1GB dataset}
   \label{fig:ph-pre-h-cs-q1-1gb}
 \end{figure}
%%%%%%%%%%%%%%%%%%%%%%%%%%%%%%%%%%%%%%%%

%%%%%%%%%%%%%%%%%%%%%%%%%%%%%%%%%%%%%%%%
%%%%q1 range
%%%%%%%%%%%%%%%%%%%%%%%%%%%%%%%%%%%%%%%%
 \begin{figure}[H]
   \centering
   \includegraphics[width=0.8\linewidth,trim=0pt 0pt 0 0pt, clip]{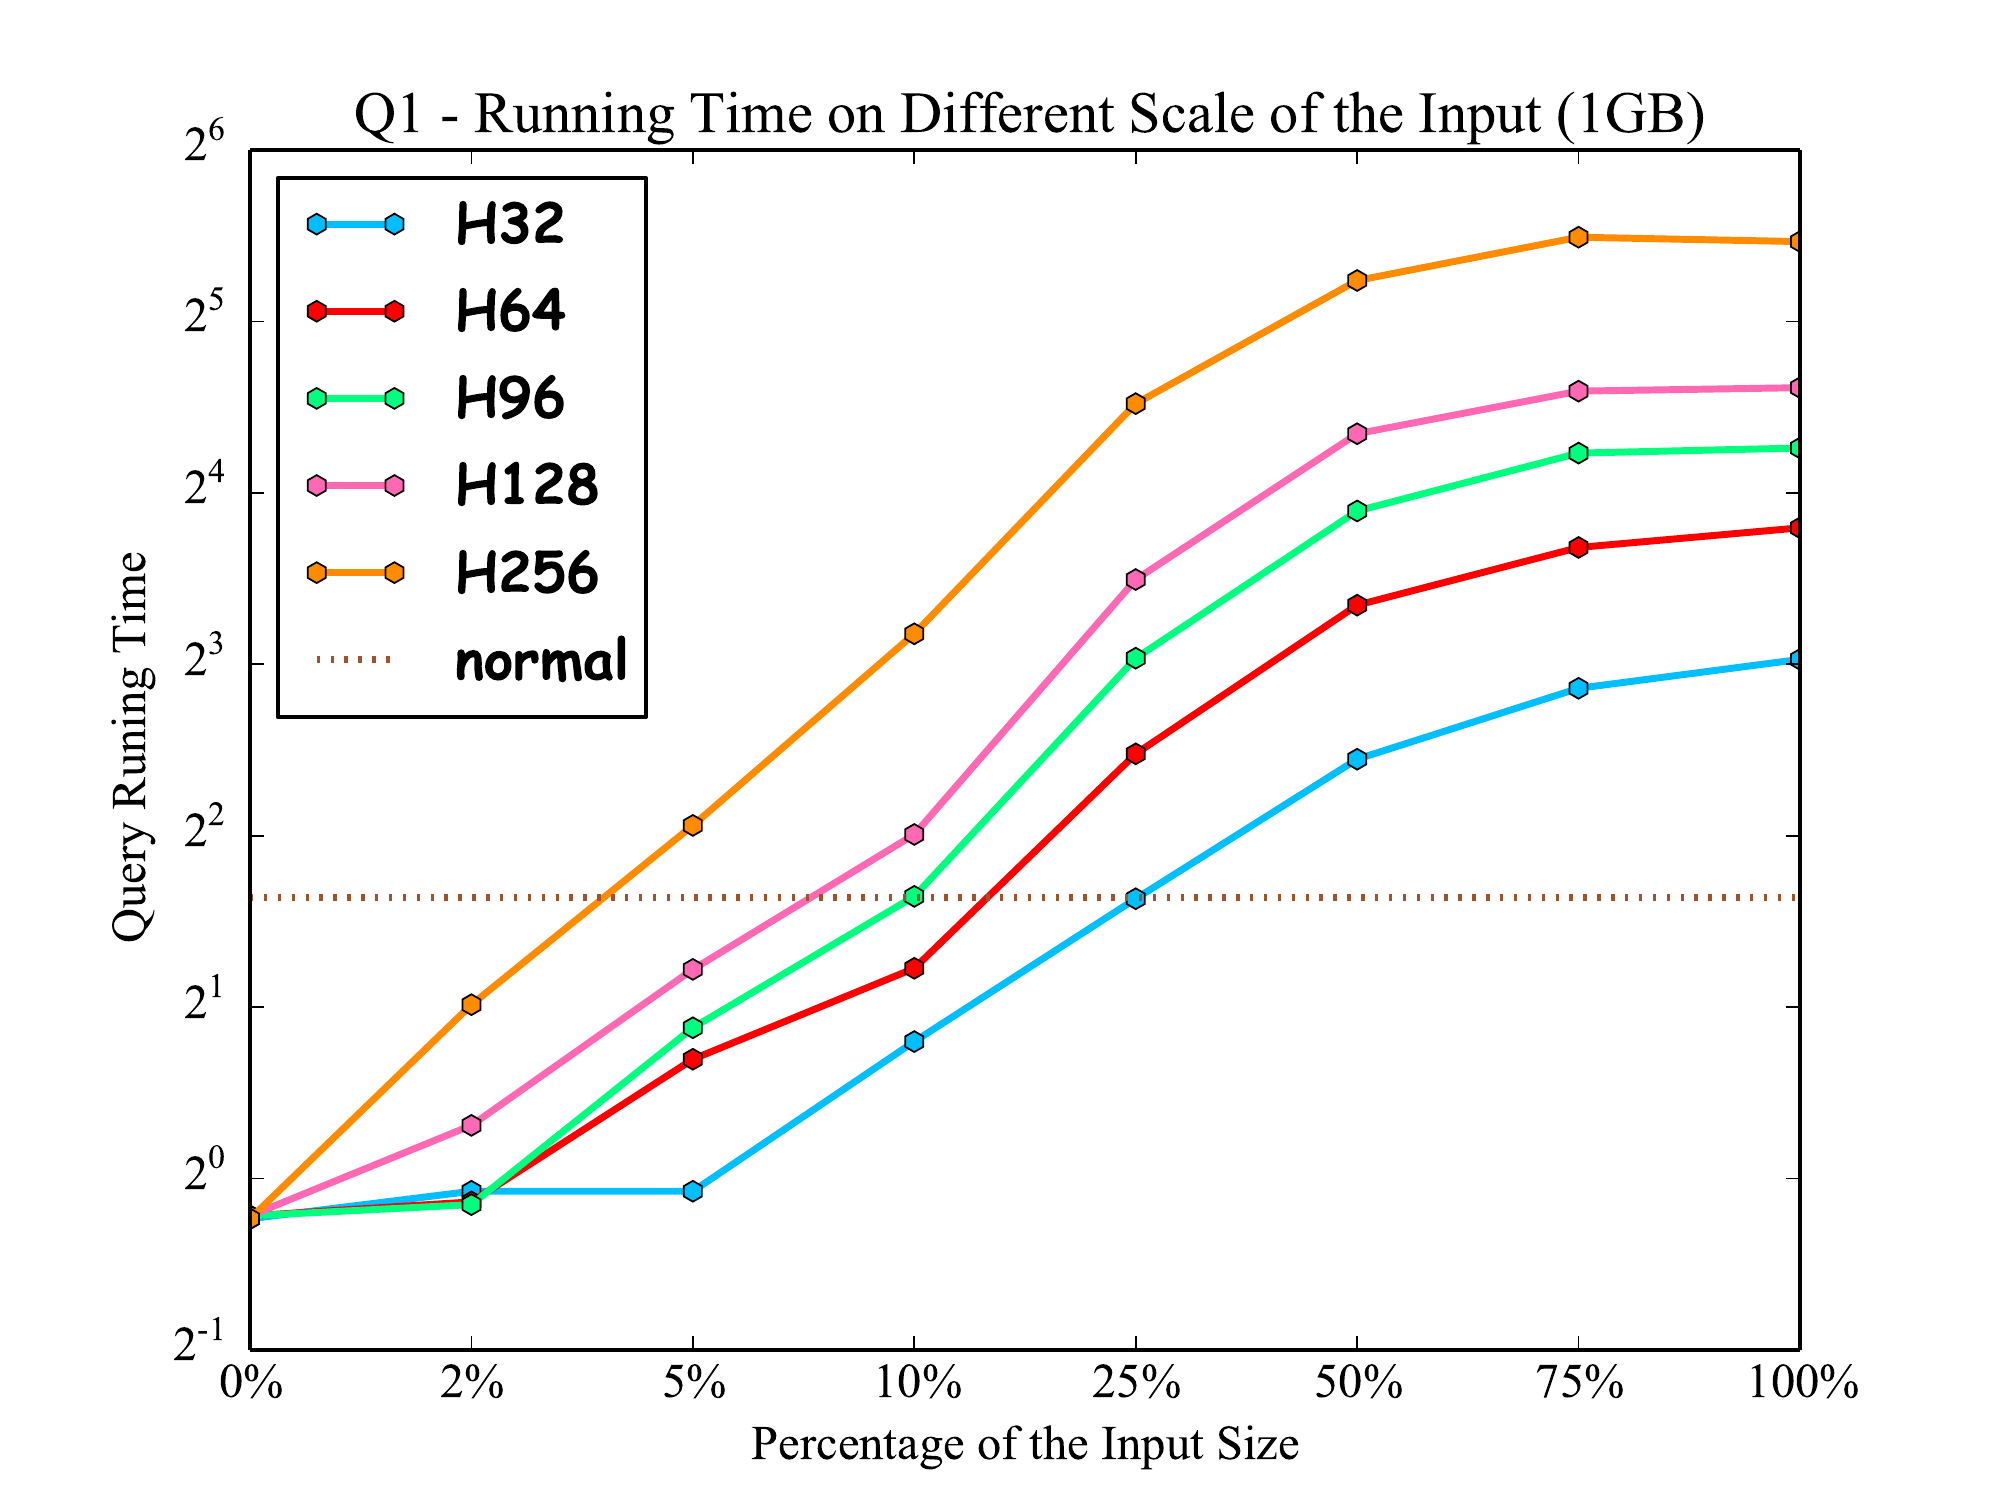}
   \caption{Fully virtual sketches + Range +  Completly synthetic for Q1 on 1GB dataset}
   \label{fig:fv-r-cs-q1-1gb}
 \end{figure}
%%%%%%%%%%%%%%%%%%%%%%%%%%%%%%%%%%%%%%%%

%%%%%%%%%%%%%%%%%%%%%%%%%%%%%%%%%%%%%%%%
 \begin{figure}[H]
   \centering
   \includegraphics[width=0.8\linewidth,trim=0pt 0pt 0 0pt, clip]{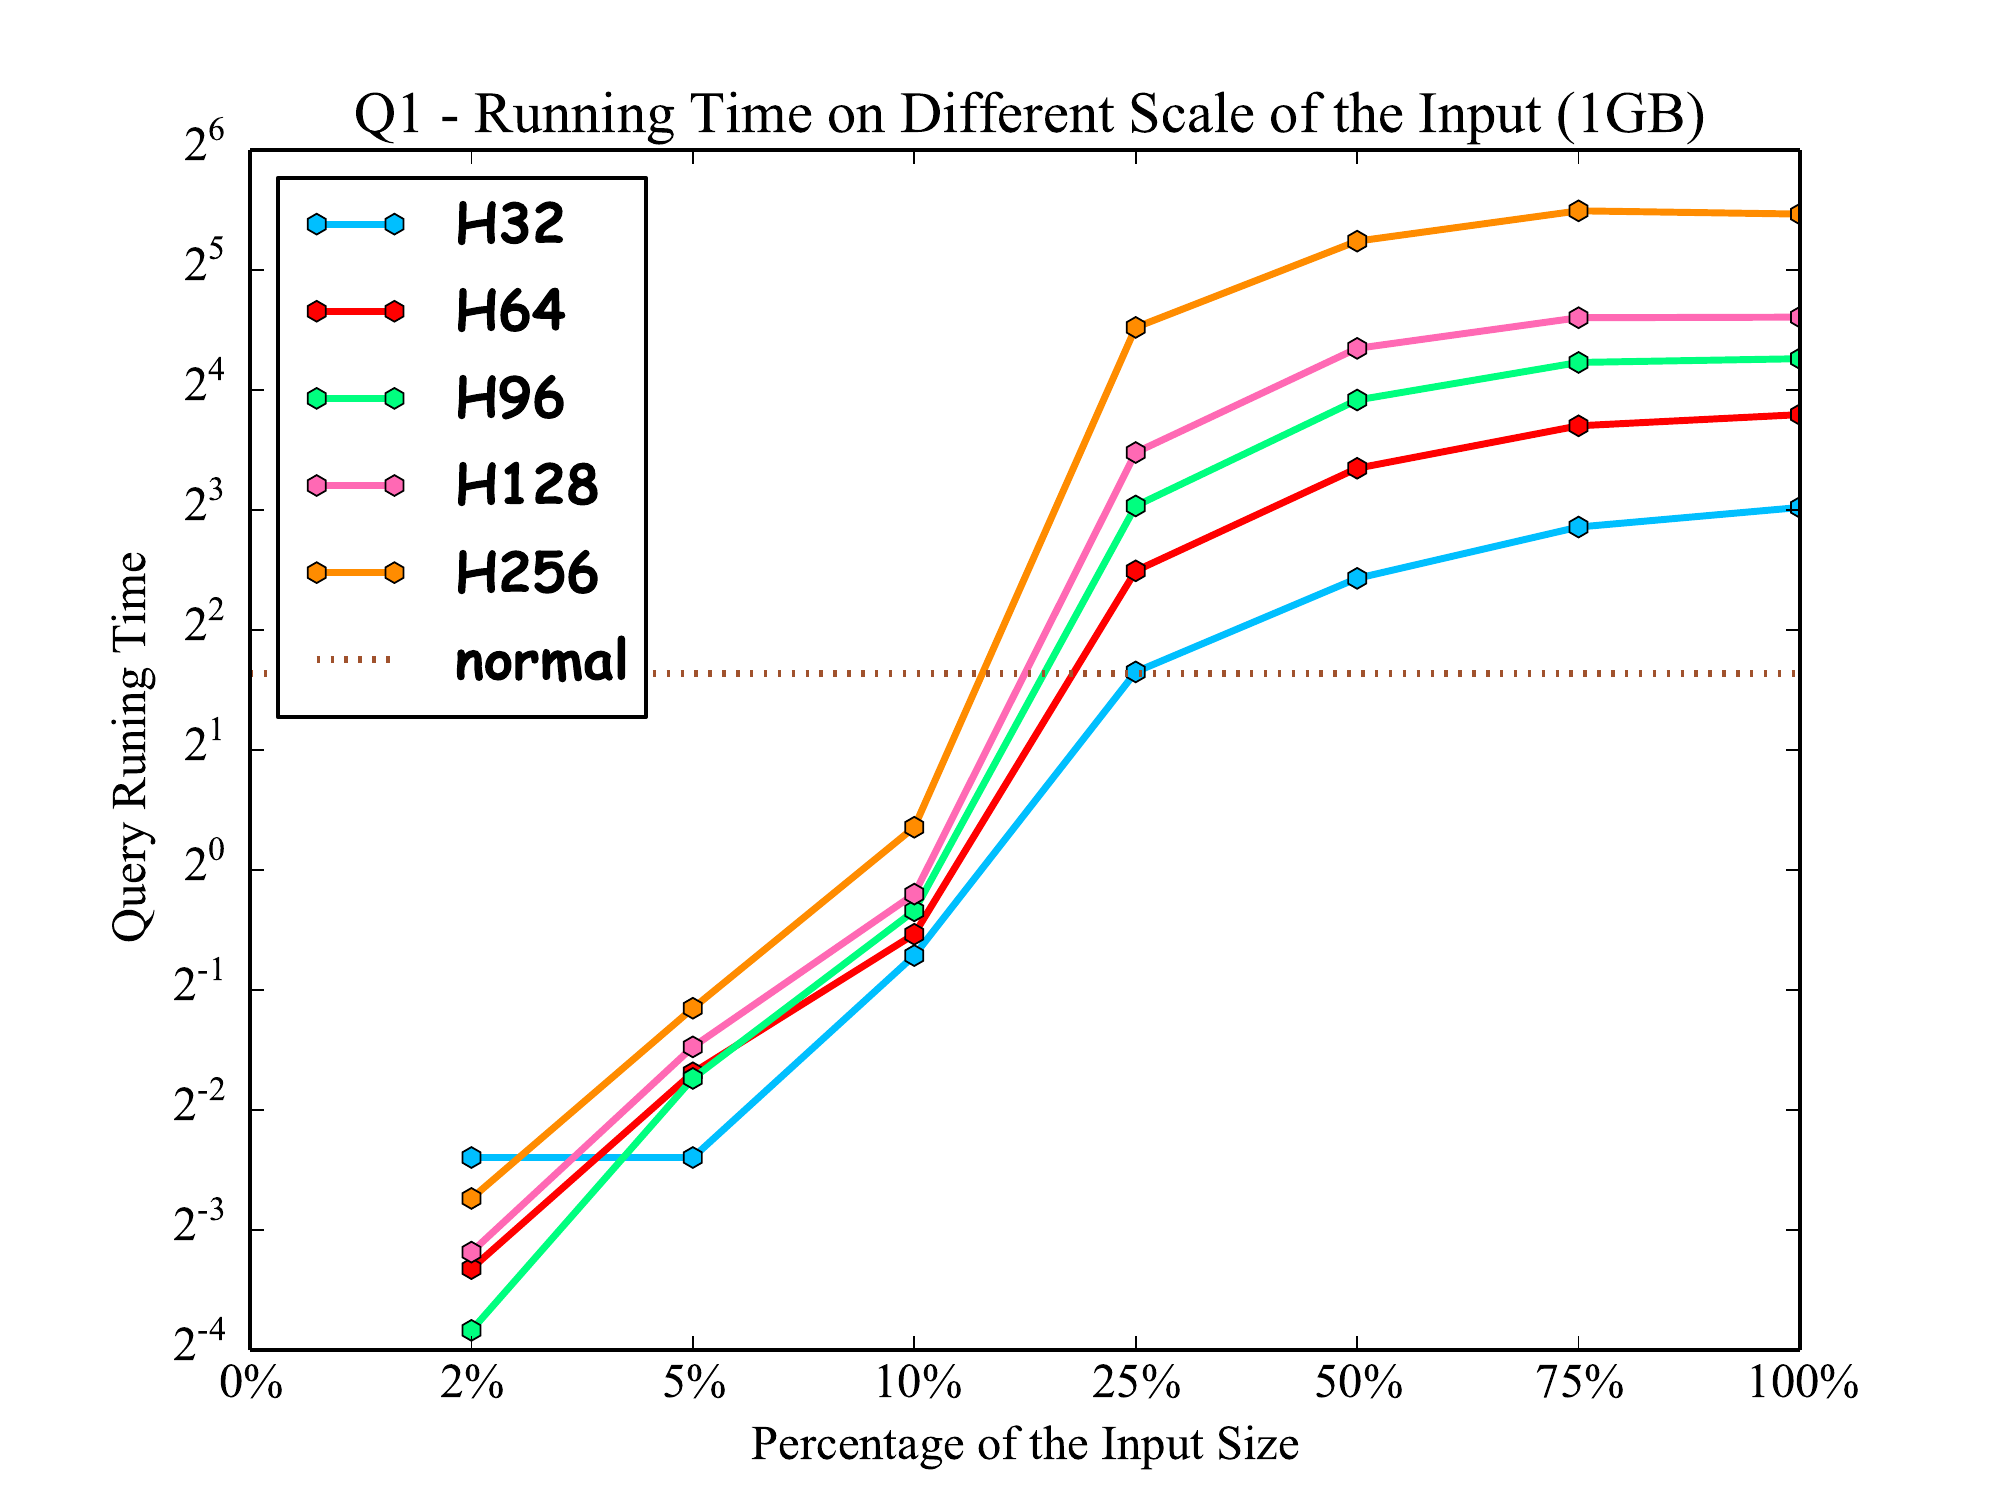}
   \caption{Fully virtual sketches + Range + index +  Completly synthetic for Q1 on 1GB dataset}
   \label{fig:fv-r-idx-cs-q1-1gb}
 \end{figure}
%%%%%%%%%%%%%%%%%%%%%%%%%%%%%%%%%%%%%%%%

%%%%%%%%%%%%%%%%%%%%%%%%%%%%%%%%%%%%%%%%
 \begin{figure}[H]
   \centering
   \includegraphics[width=0.8\linewidth,trim=0pt 0pt 0 0pt, clip]{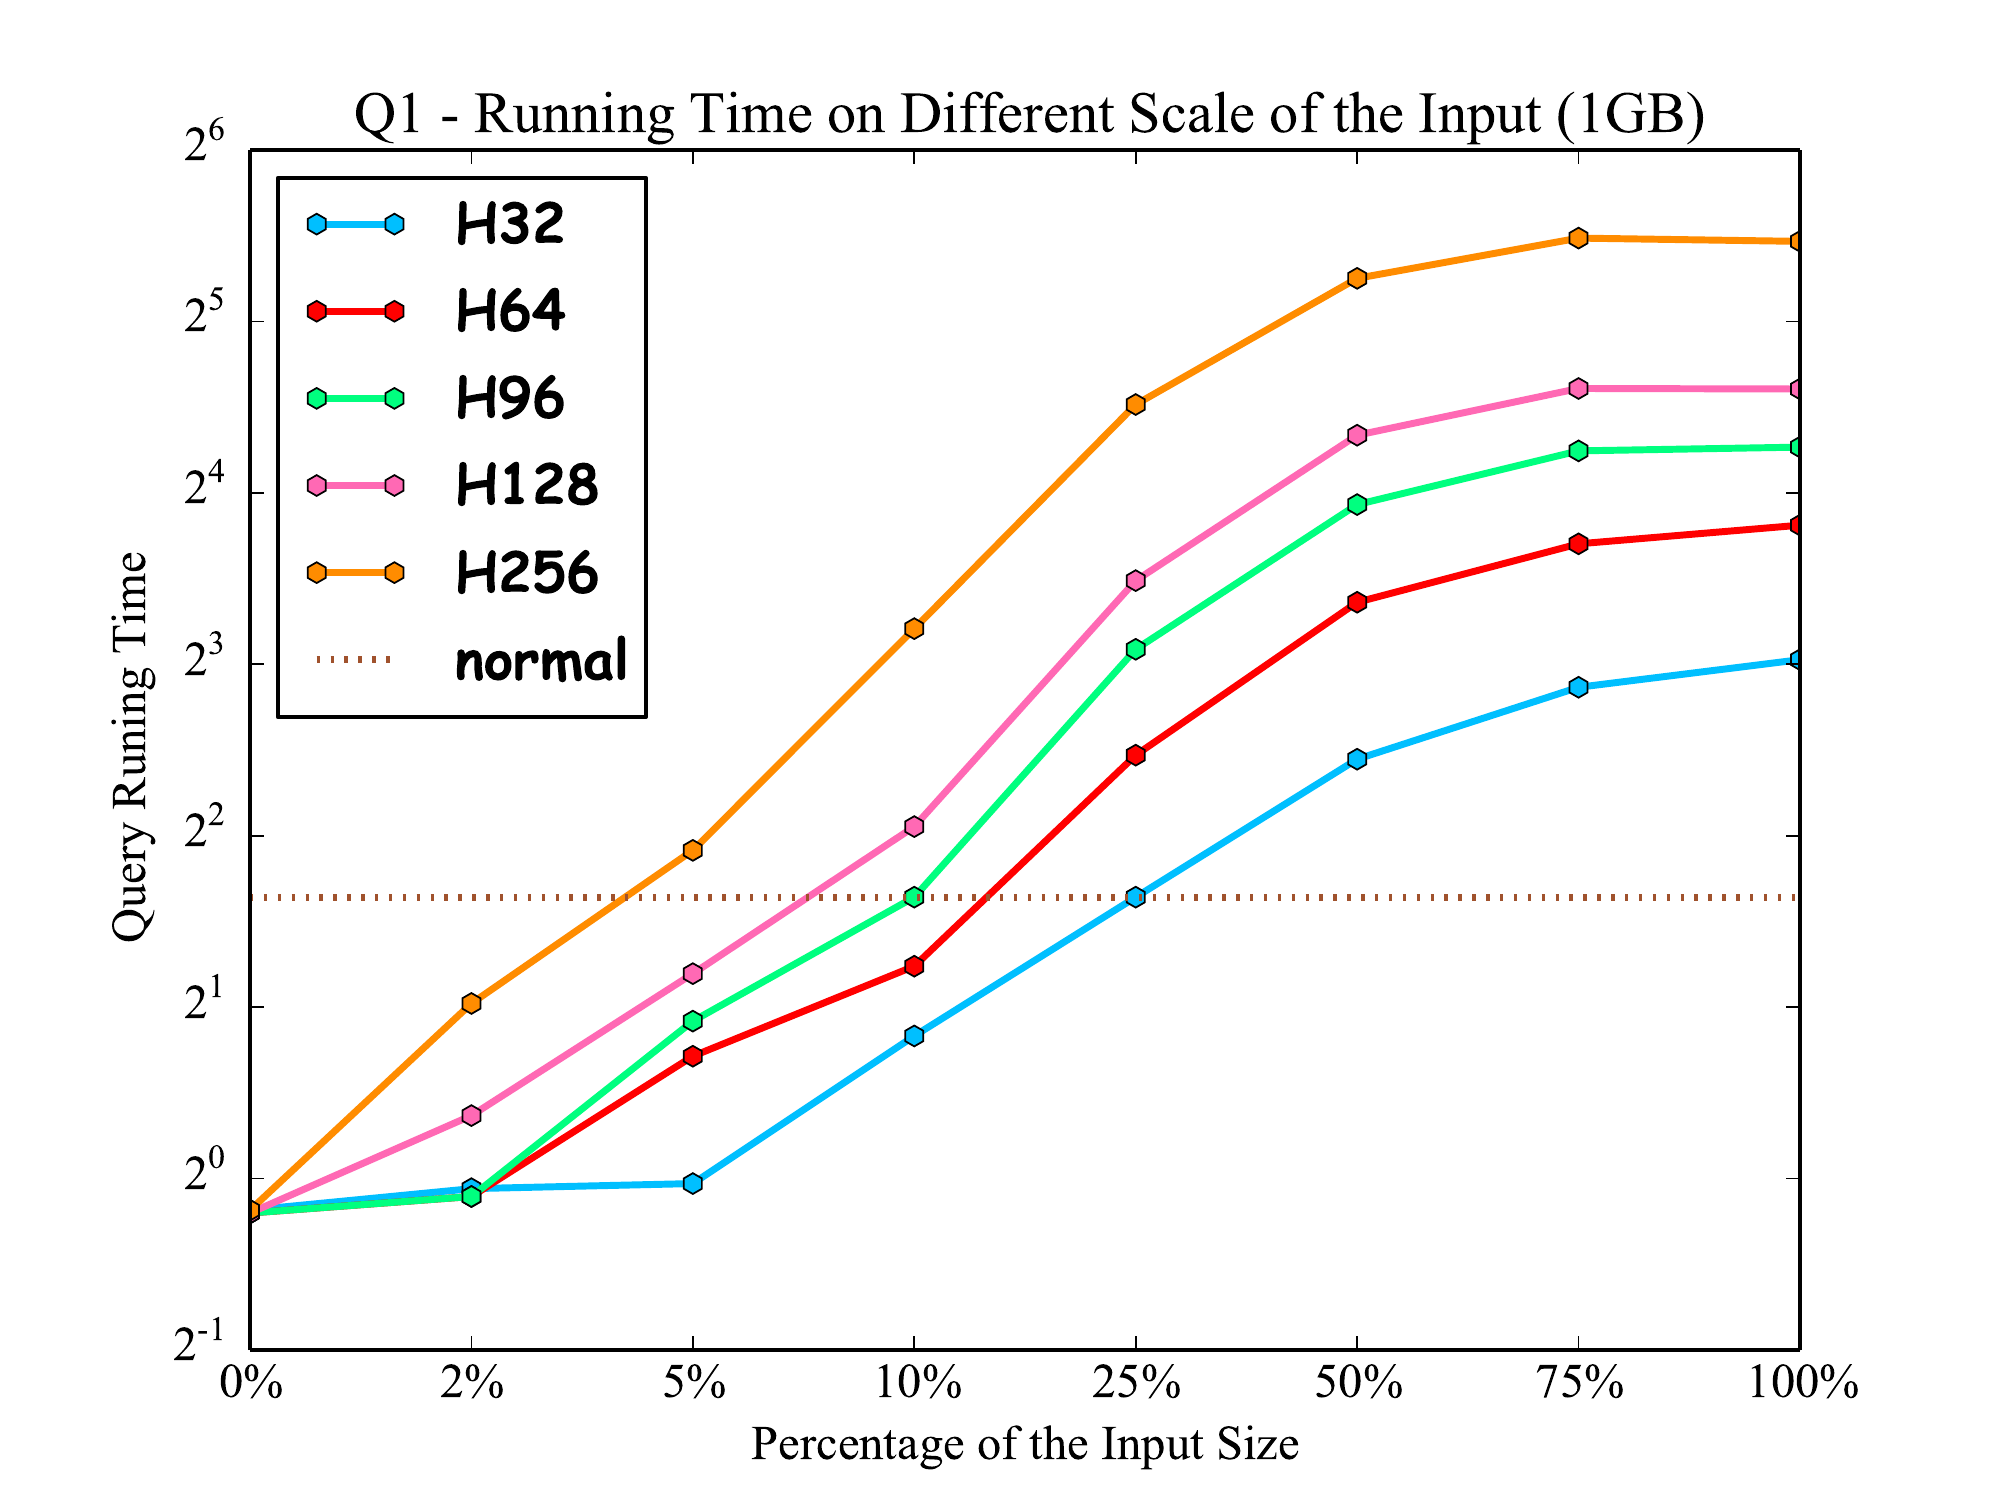}
   \caption{Physical sketches + Range +  Completly synthetic for Q1 on 1GB dataset}
   \label{fig:ph-r-cs-q1-1gb}
 \end{figure}
%%%%%%%%%%%%%%%%%%%%%%%%%%%%%%%%%%%%%%%%

%%%%%%%%%%%%%%%%%%%%%%%%%%%%%%%%%%%%%%%%
%q1 hash and range 10gb
%%%%%%%%%%%%%%%%%%%%%%%%%%%%%%%%%%%%%%%%
 \begin{figure}[H]
   \centering
   \includegraphics[width=0.8\linewidth,trim=0pt 0pt 0 0pt, clip]{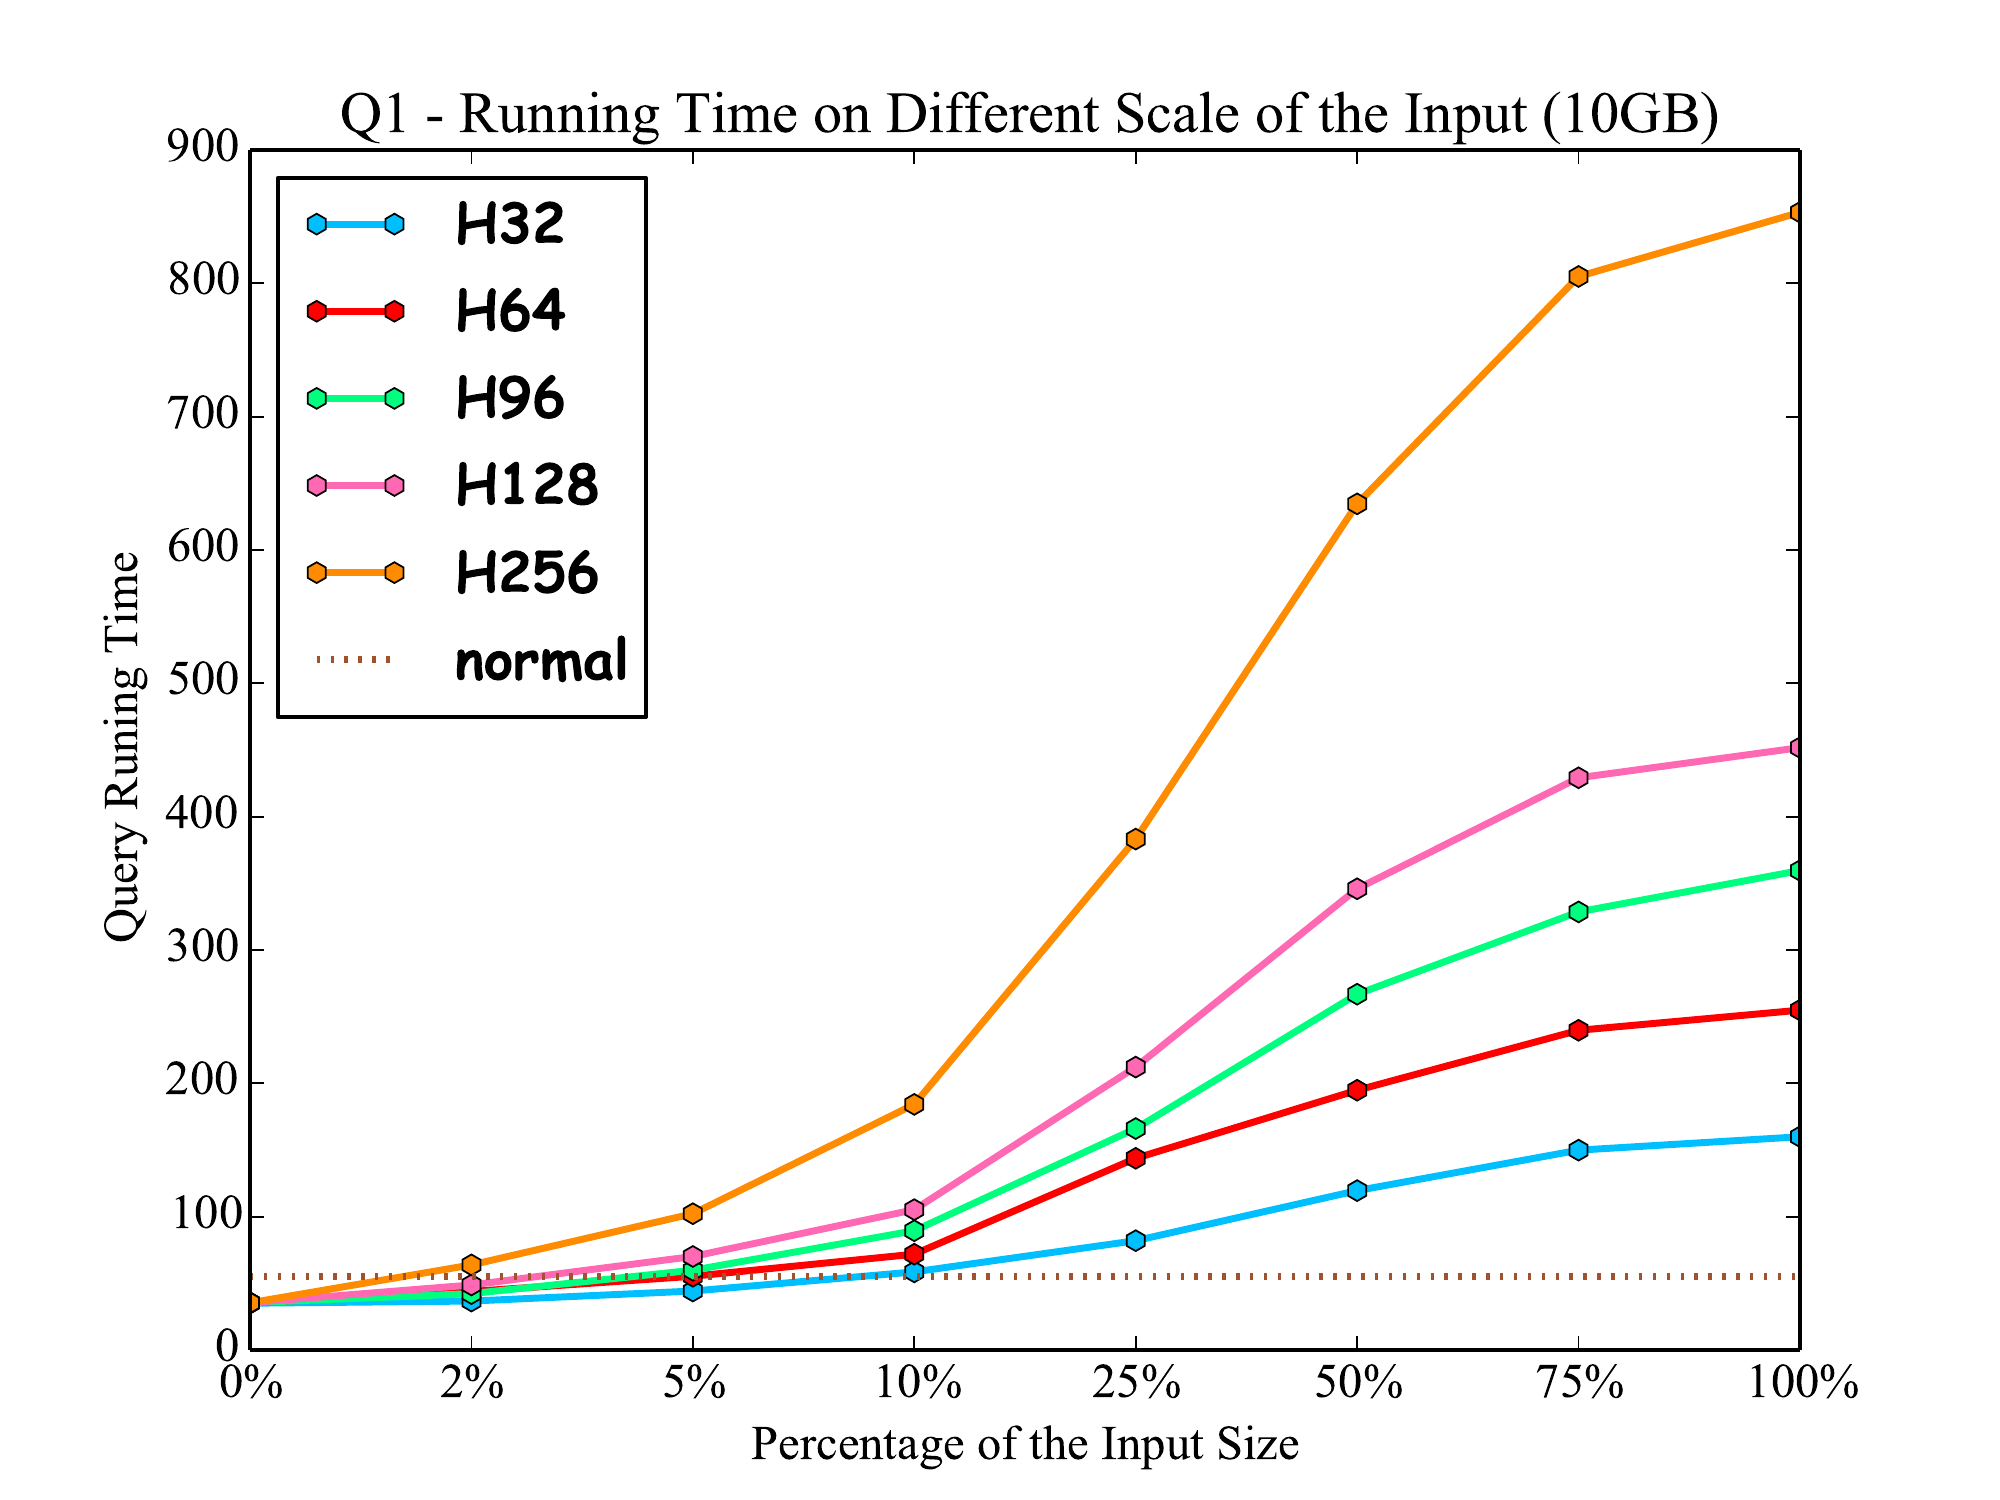}
   \caption{Fully virtual sketches + Hash +  Completly synthetic for Q1 on 10GB dataset}
   \label{fig:fv-h-cs-q1-10gb}
 \end{figure}
%%%%%%%%%%%%%%%%%%%%%%%%%%%%%%%%%%%%%%%%

%%%%%%q2
%%%%%%%%%%%%%%%%%%%%%%%%%%%%%%%%%%%%%%%%
%%%%%%q2
%%%%%%%%%%%%%%%%%%%%%%%%%%%%%%%%%%%%%%%%
 \begin{figure}[H]
   \centering
   \includegraphics[width=0.8\linewidth,trim=0pt 0pt 0 0pt, clip]{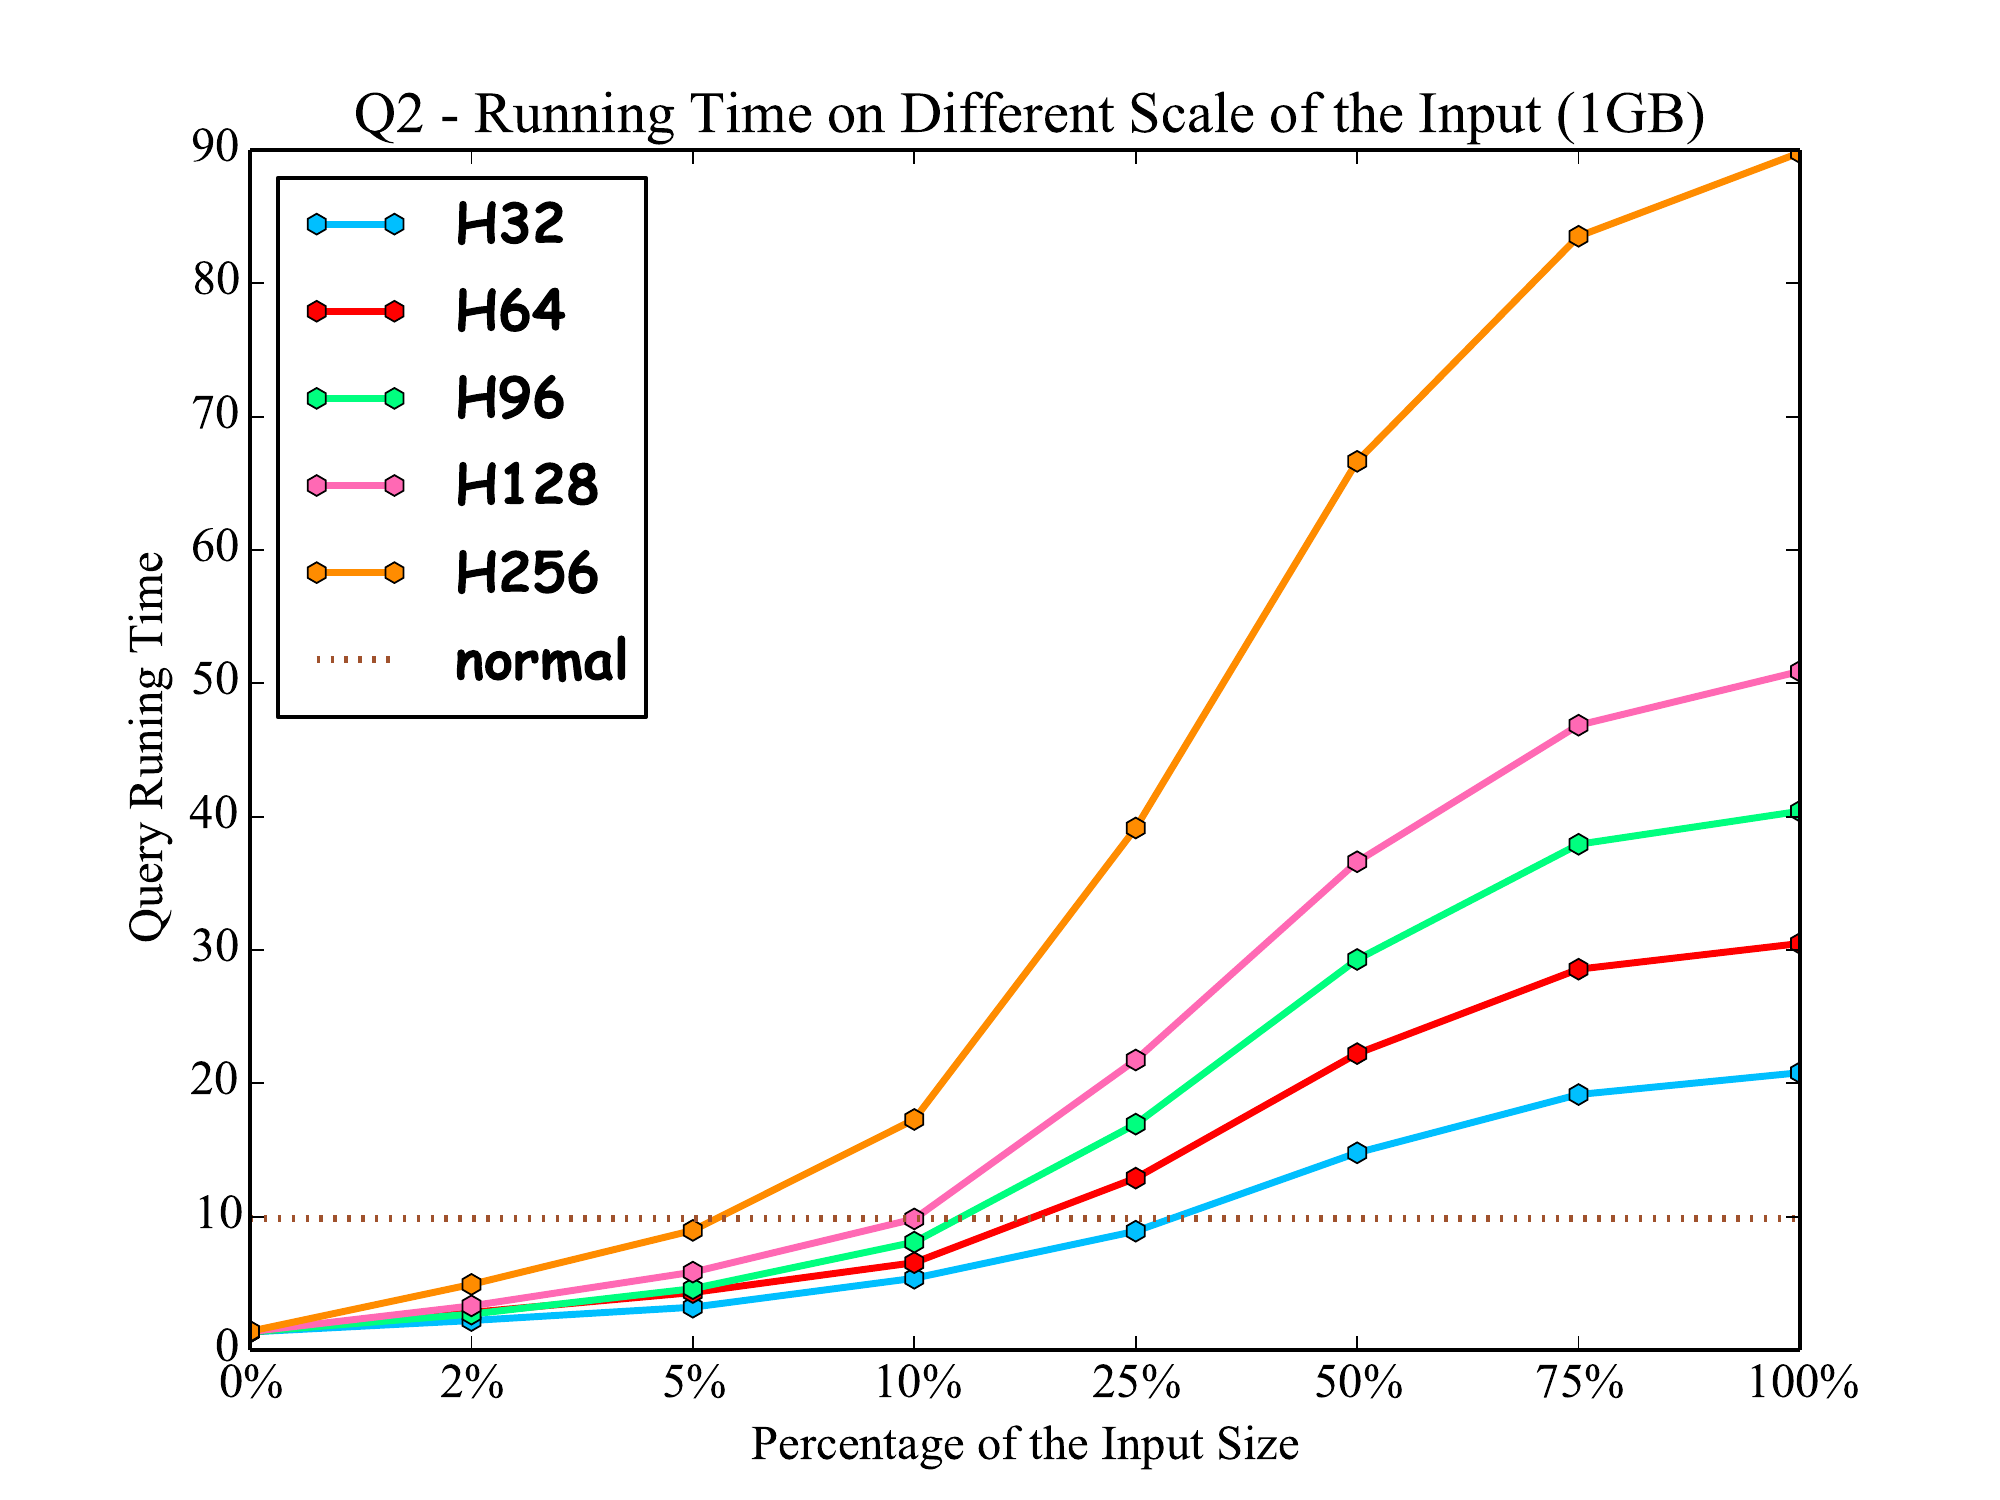}
   \caption{Fully virtual sketches + Hash +  Completly synthetic for Q2 on 1GB dataset}
   \label{fig:fv-h-cs-q2-1gb}
 \end{figure}
%%%%%%%%%%%%%%%%%%%%%%%%%%%%%%%%%%%%%%%%

%%%%%%%%%%q2 prehash @pengyuanli 4/9/2019
 \begin{figure}[H]
   \centering
   \includegraphics[width=0.8\linewidth,trim=0pt 0pt 0 0pt, clip]{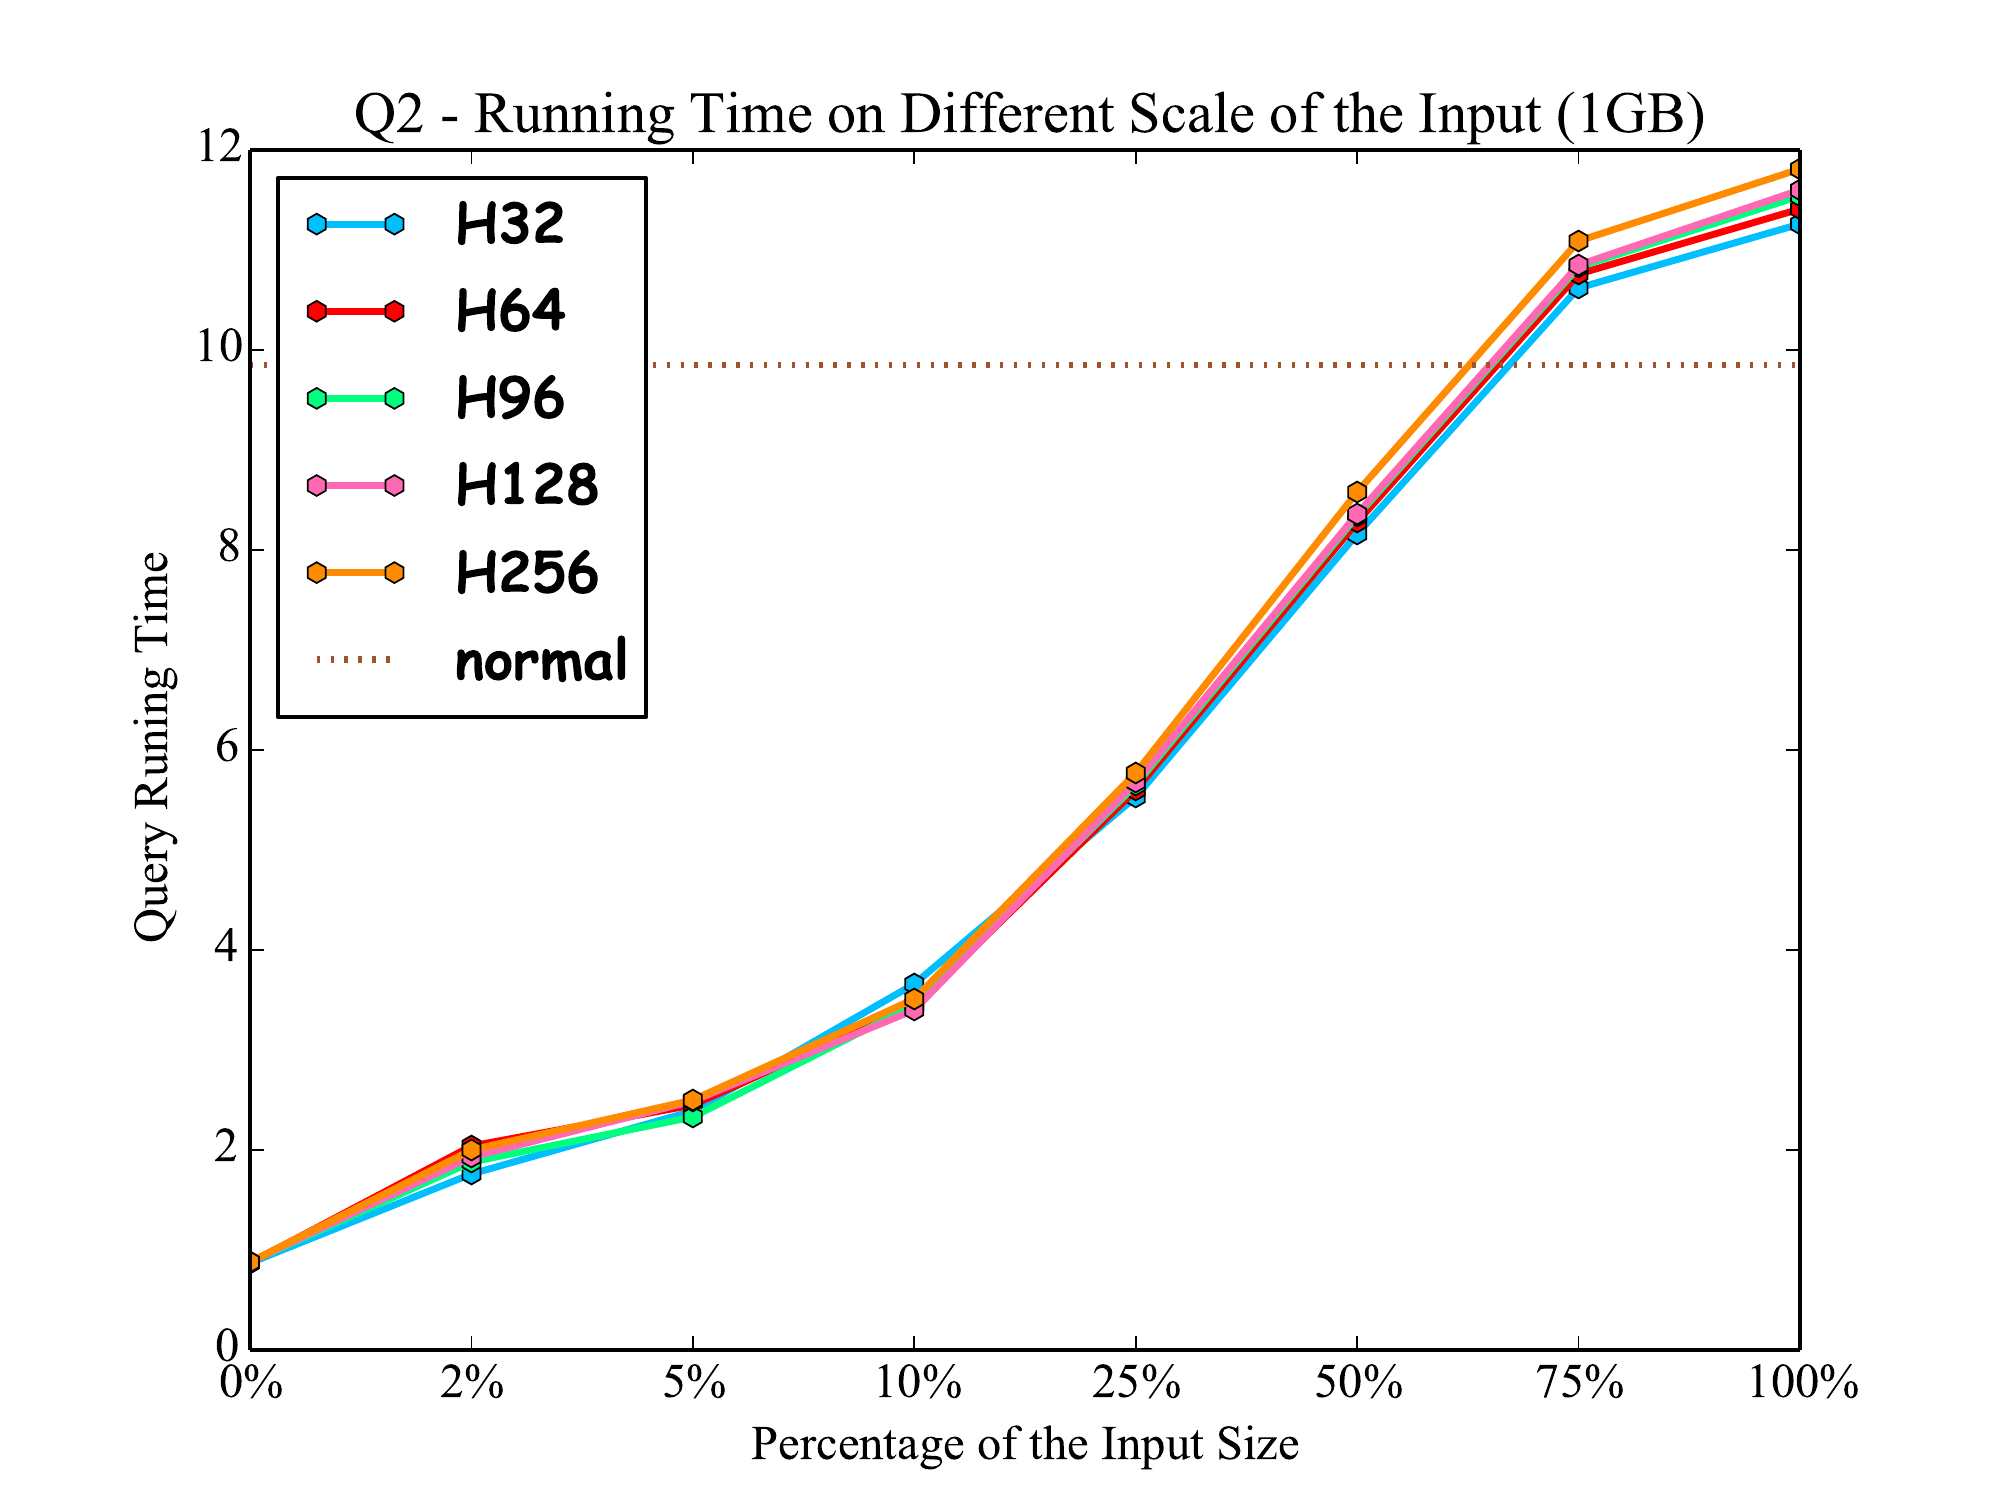}
   \caption{Fully virtual sketches + Pre-Hash +  Completly synthetic for Q2 on 1GB dataset}
   \label{fig:fv-h-cs-q2-1gb}
 \end{figure}
%%%%%%%%%%%%%%%%%%%%%%%%%%%%%%%%%%%%%%%%

%%%%%%%%%%%%%%%%%%%%%%%%%%%%%%%%%%%%%%%%
 \begin{figure}[H]
   \centering
   \includegraphics[width=0.8\linewidth,trim=0pt 0pt 0 0pt, clip]{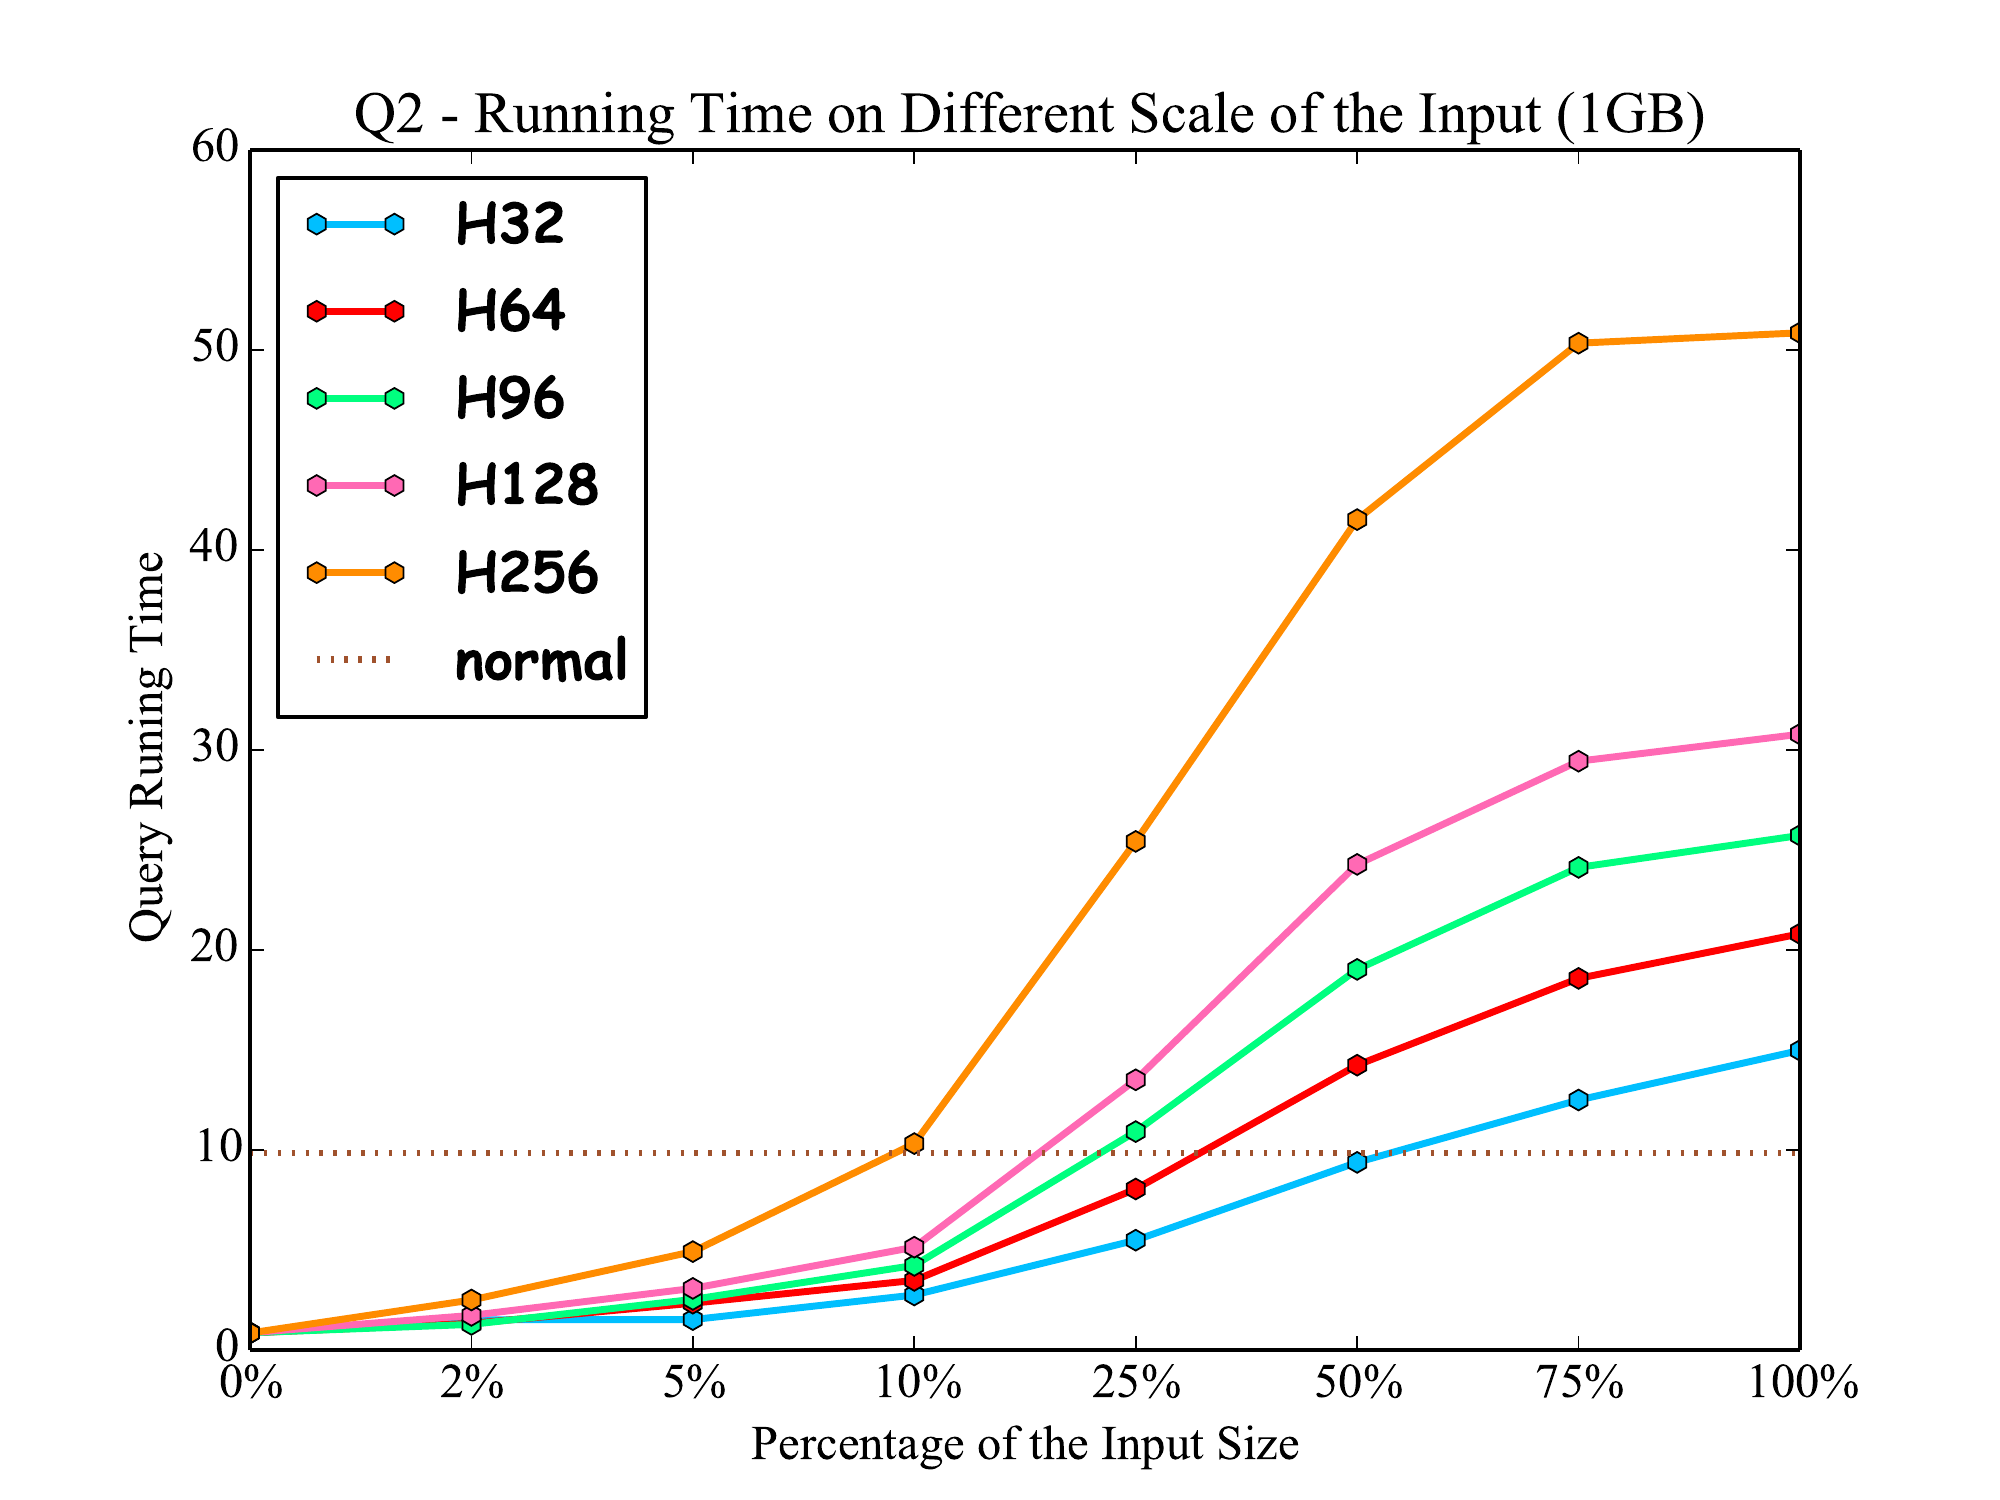}
   \caption{Fully virtual sketches + Range +  Completly synthetic for Q2 on 1GB dataset}
   \label{fig:fv-r-cs-q2-1gb}
 \end{figure}
%%%%%%%%%%%%%%%%%%%%%%%%%%%%%%%%%%%%%%%%

%%%%%%%%%%q2 index range @pengyuanli 4/9/2019
 \begin{figure}[H]
   \centering
   \includegraphics[width=0.8\linewidth,trim=0pt 0pt 0 0pt, clip]{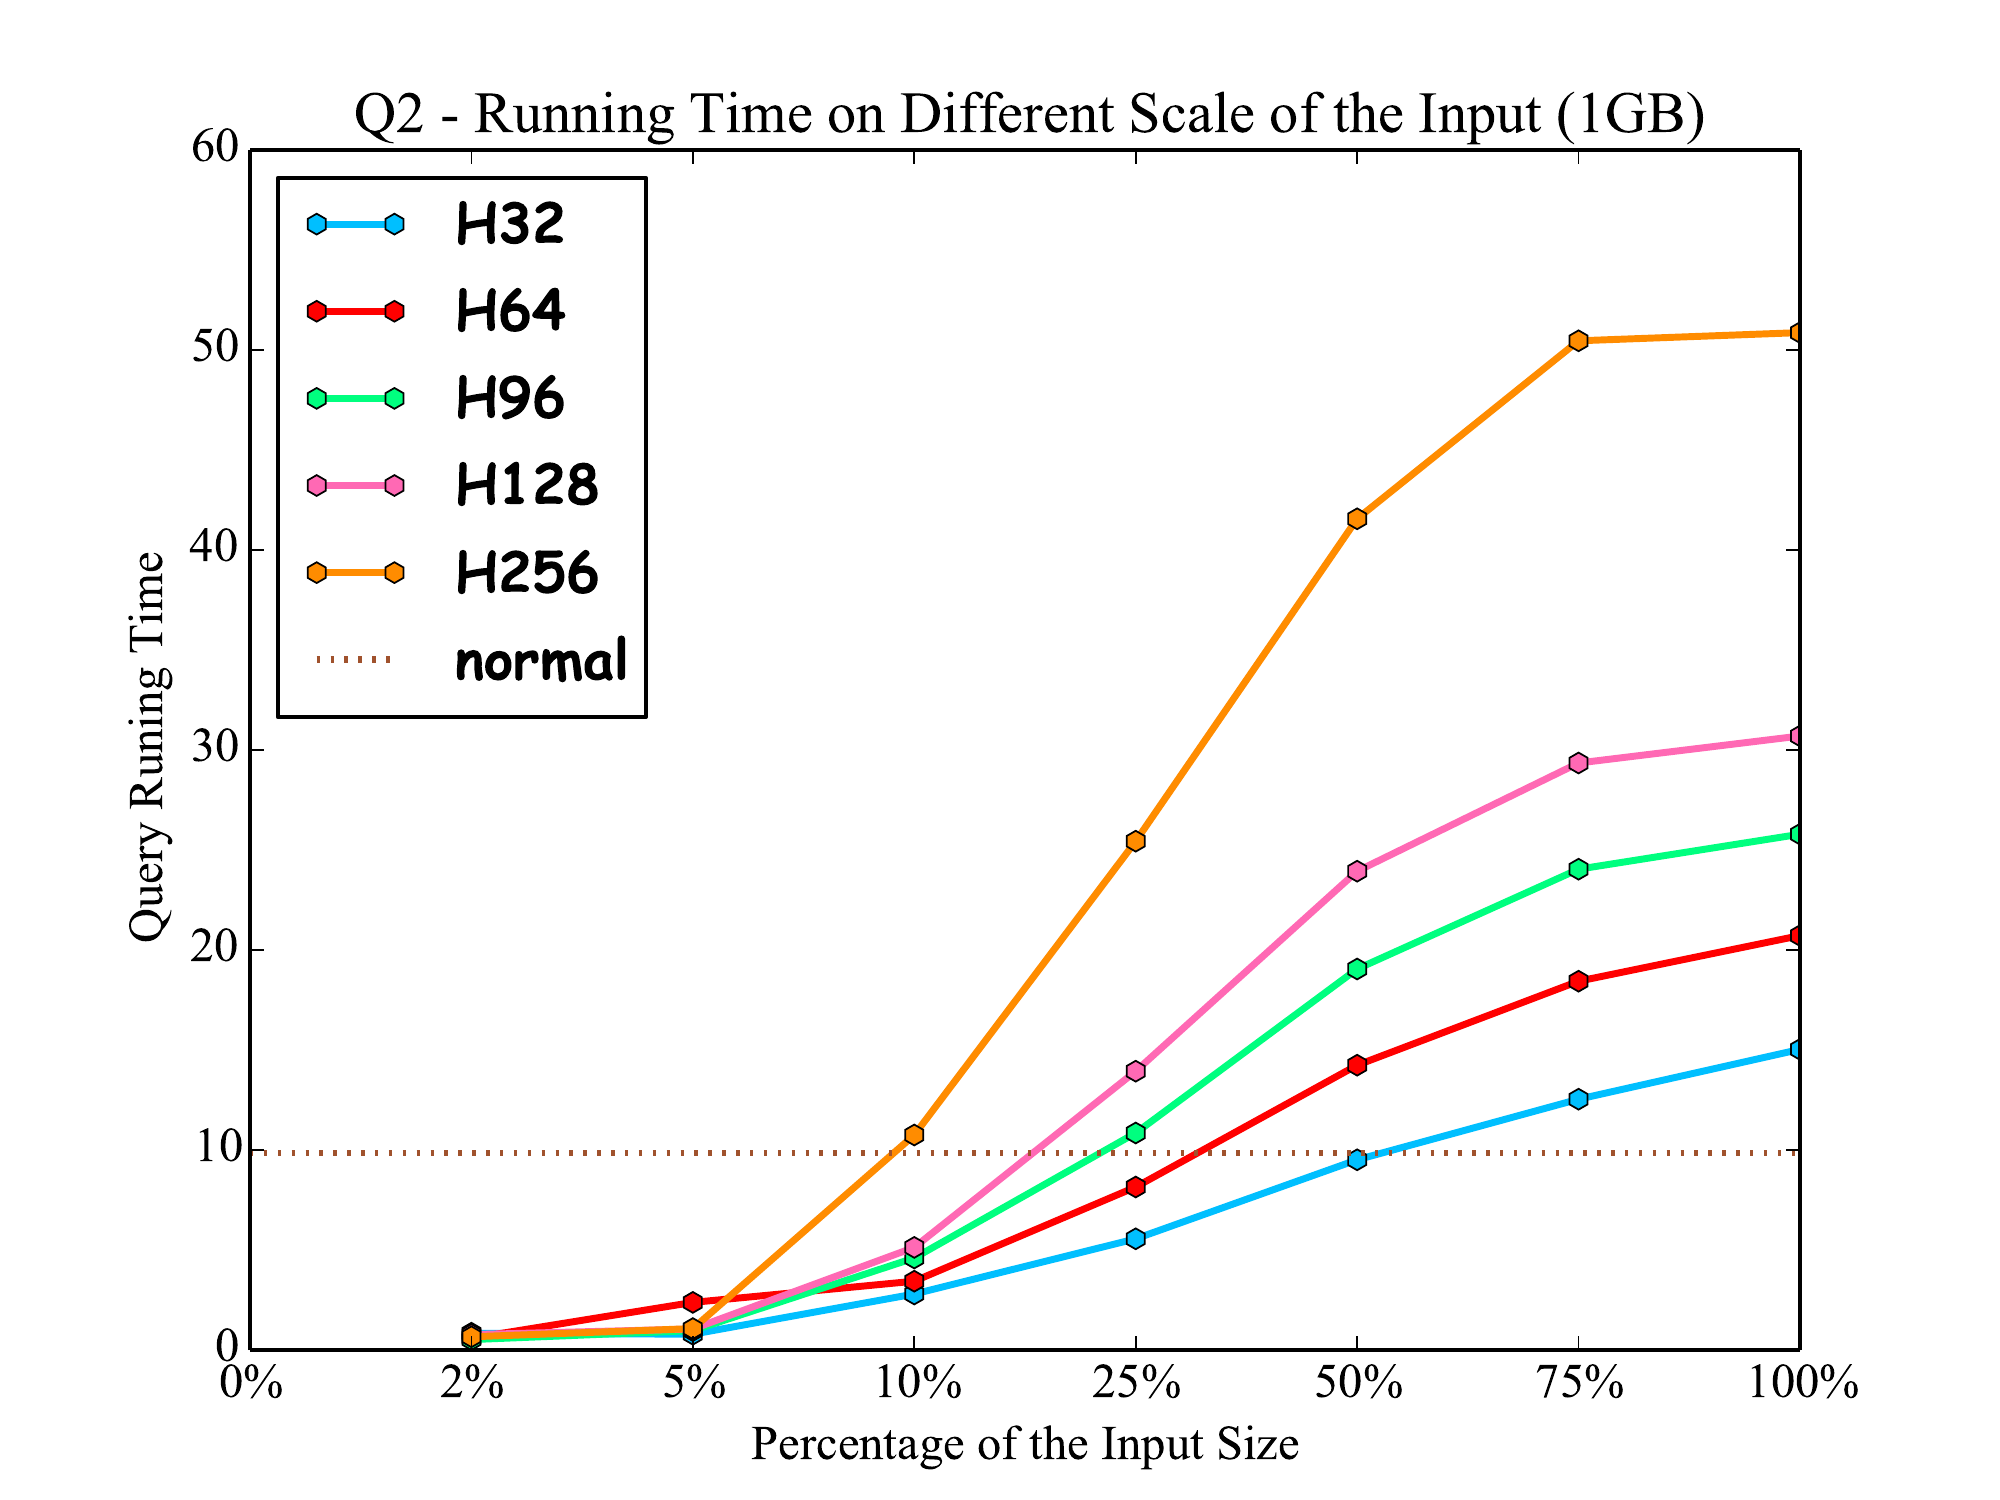}
   \caption{Fully virtual sketches + Range + index +  Completly synthetic for Q2 on 1GB dataset}
   \label{fig:fv-h-cs-q2-1gb}
 \end{figure}
%%%%%%%%%%%%%%%%%%%%%%%%%%%%%%%%%%%%%%%%

%%%%%%%%%%%%%%%%%%%%%%%%%%%%%%%%%%%%%%%%
 \begin{figure}[H]
   \centering
   \includegraphics[width=0.8\linewidth,trim=0pt 0pt 0 0pt, clip]{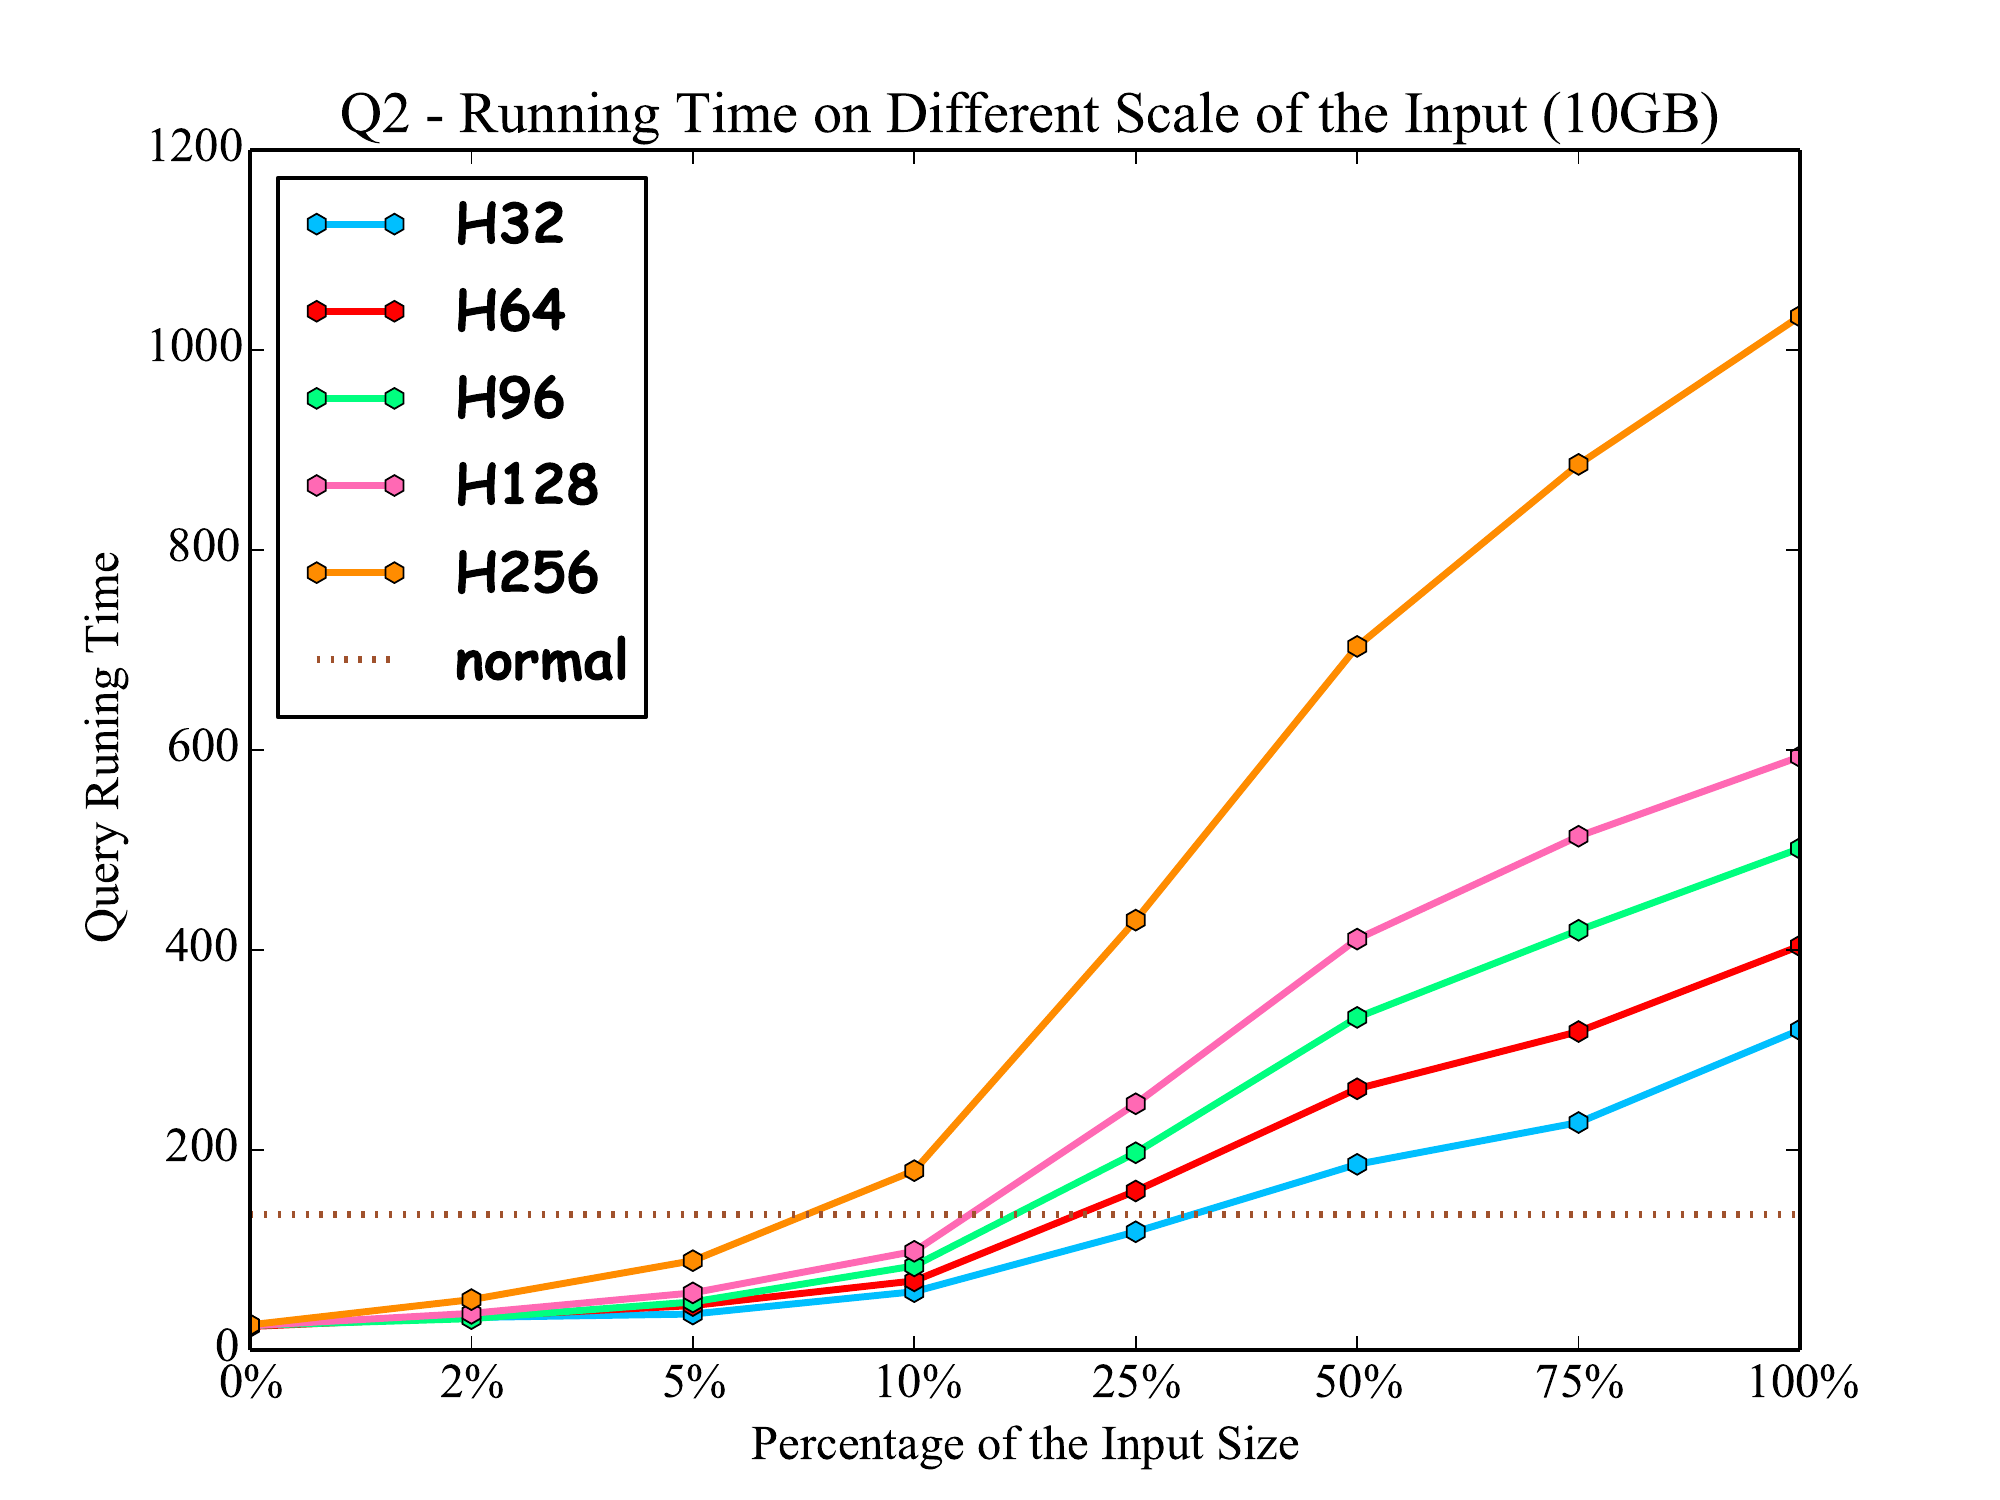}
   \caption{Fully virtual sketches + Hash +  Completly synthetic for Q2 on 10GB dataset}
   \label{fig:fv-h-cs-q2-10gb}
 \end{figure}
%%%%%%%%%%%%%%%%%%%%%%%%%%%%%%%%%%%%%%%%

%%%%%%%%%%%%%%%%%%%%%%%%%%%%%%%%%%%%%%%%%
%%%%%q3 hash
%%%%%%%%%%%%%%%%%%%%%%%%%%%%%%%%%%%%%%%%%
 \begin{figure}[H]
   \centering
   \includegraphics[width=0.8\linewidth,trim=0pt 0pt 0 0pt, clip]{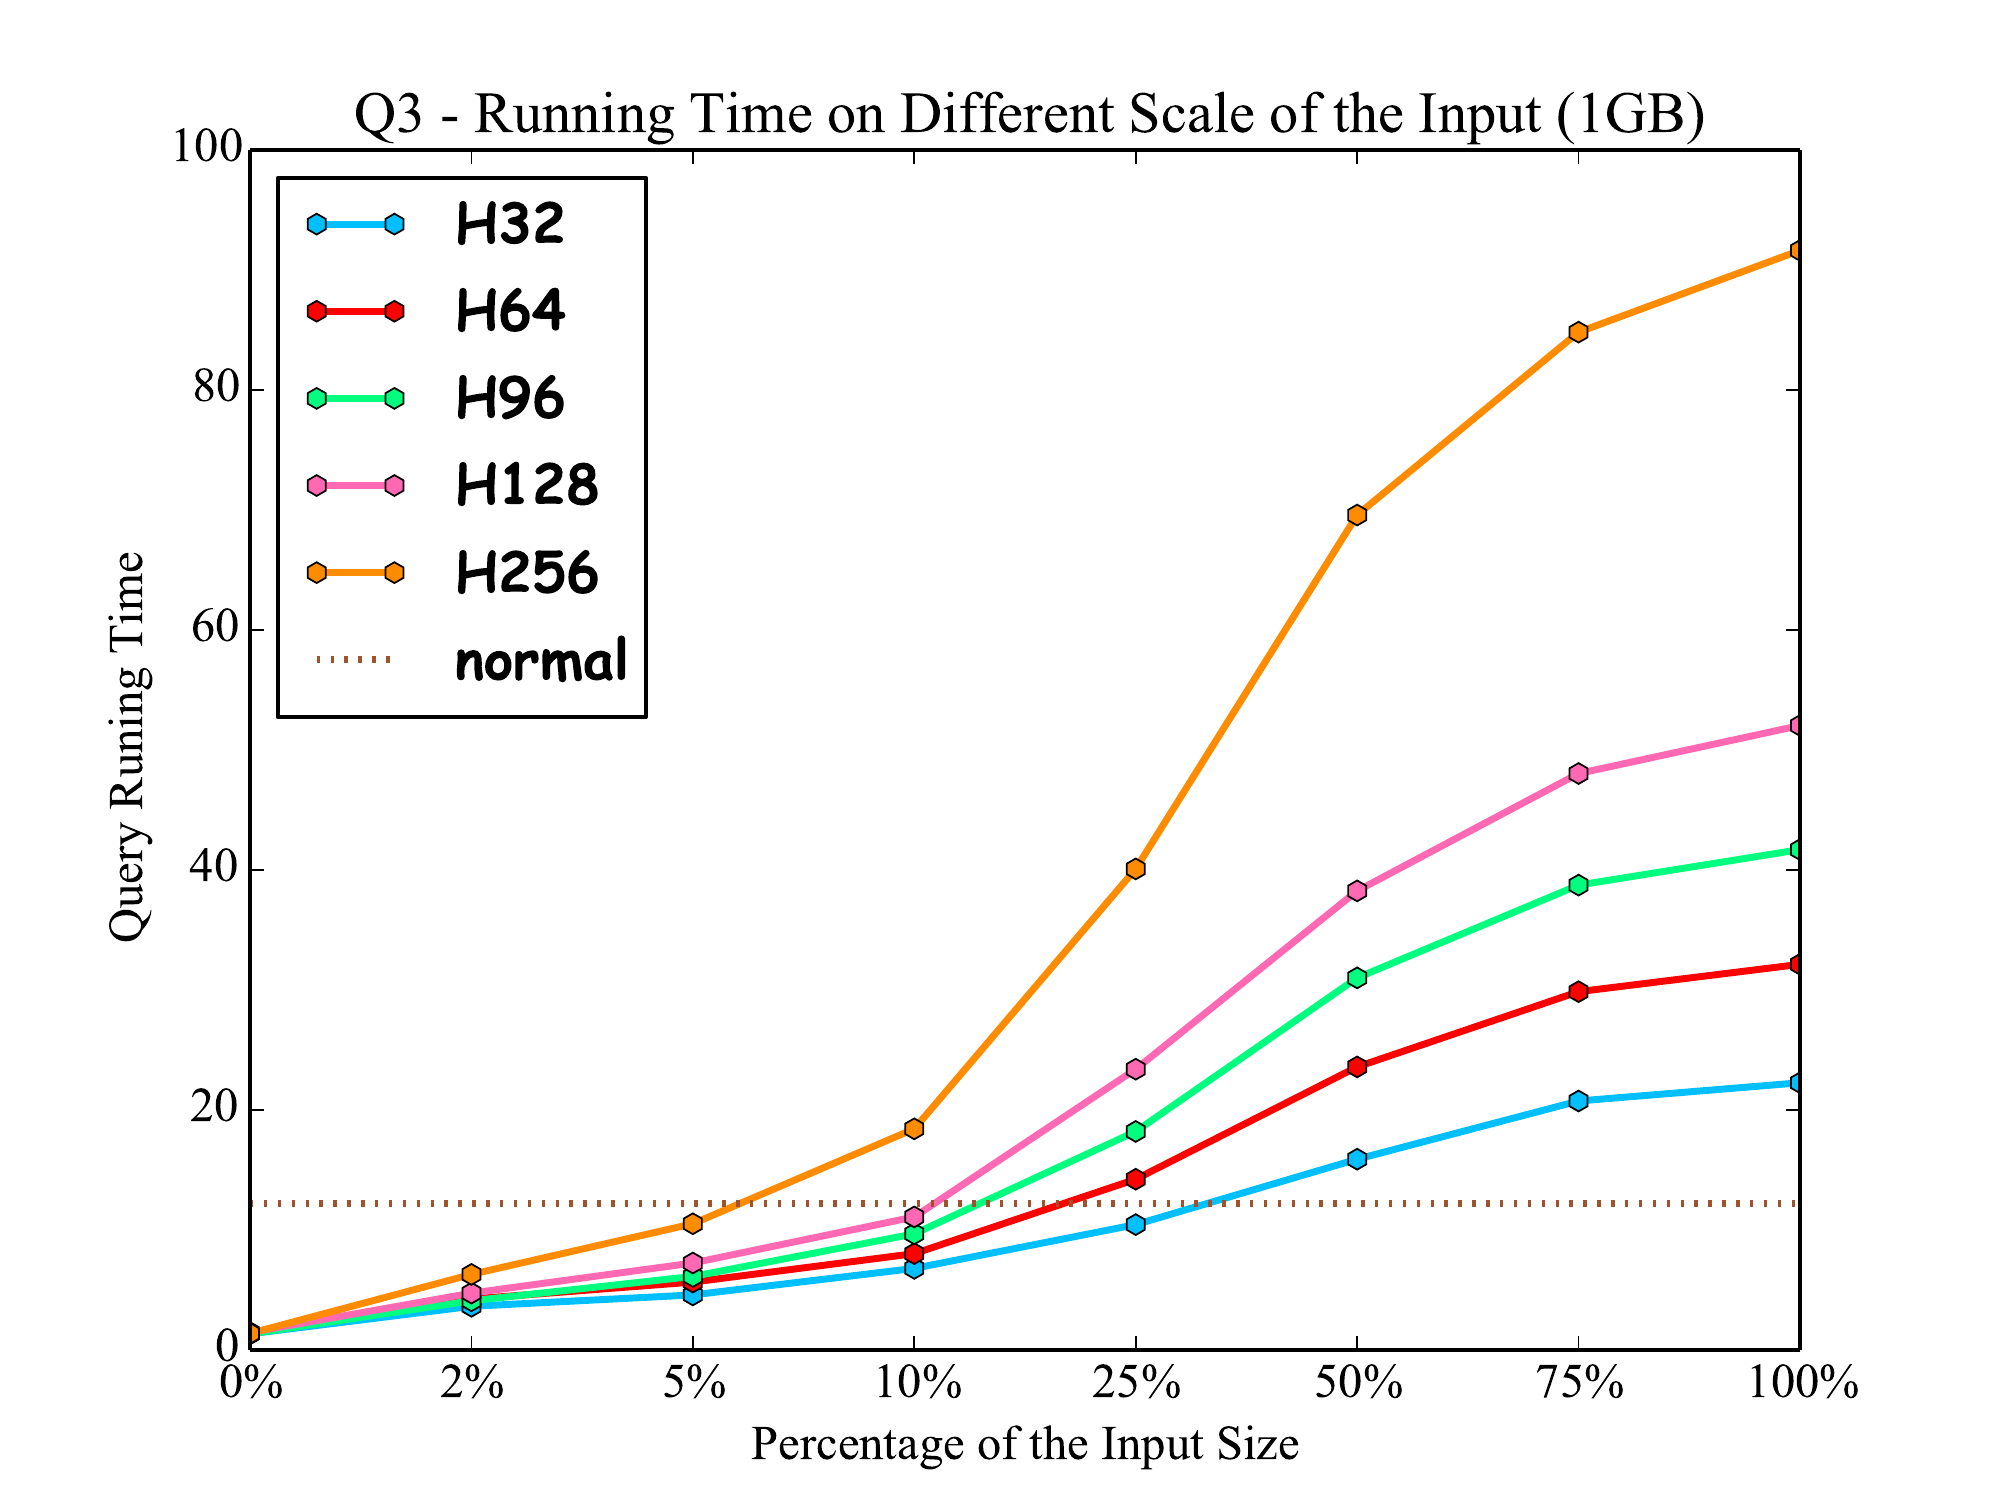}
   \caption{Fully virtual sketches + Hash +  Completly synthetic for Q3 on 1GB dataset}
   \label{fig:fv-h-cs-q3-1gb}
 \end{figure}
%%%%%%%%%%%%%%%%%%%%%%%%%%%%%%%%%%%%%%%%

%%%%%%%%%%%%%%%%%%%%%%%%%%%%%%%%%%%%%%%%%
 \begin{figure}[H]
   \centering
   \includegraphics[width=0.8\linewidth,trim=0pt 0pt 0 0pt, clip]{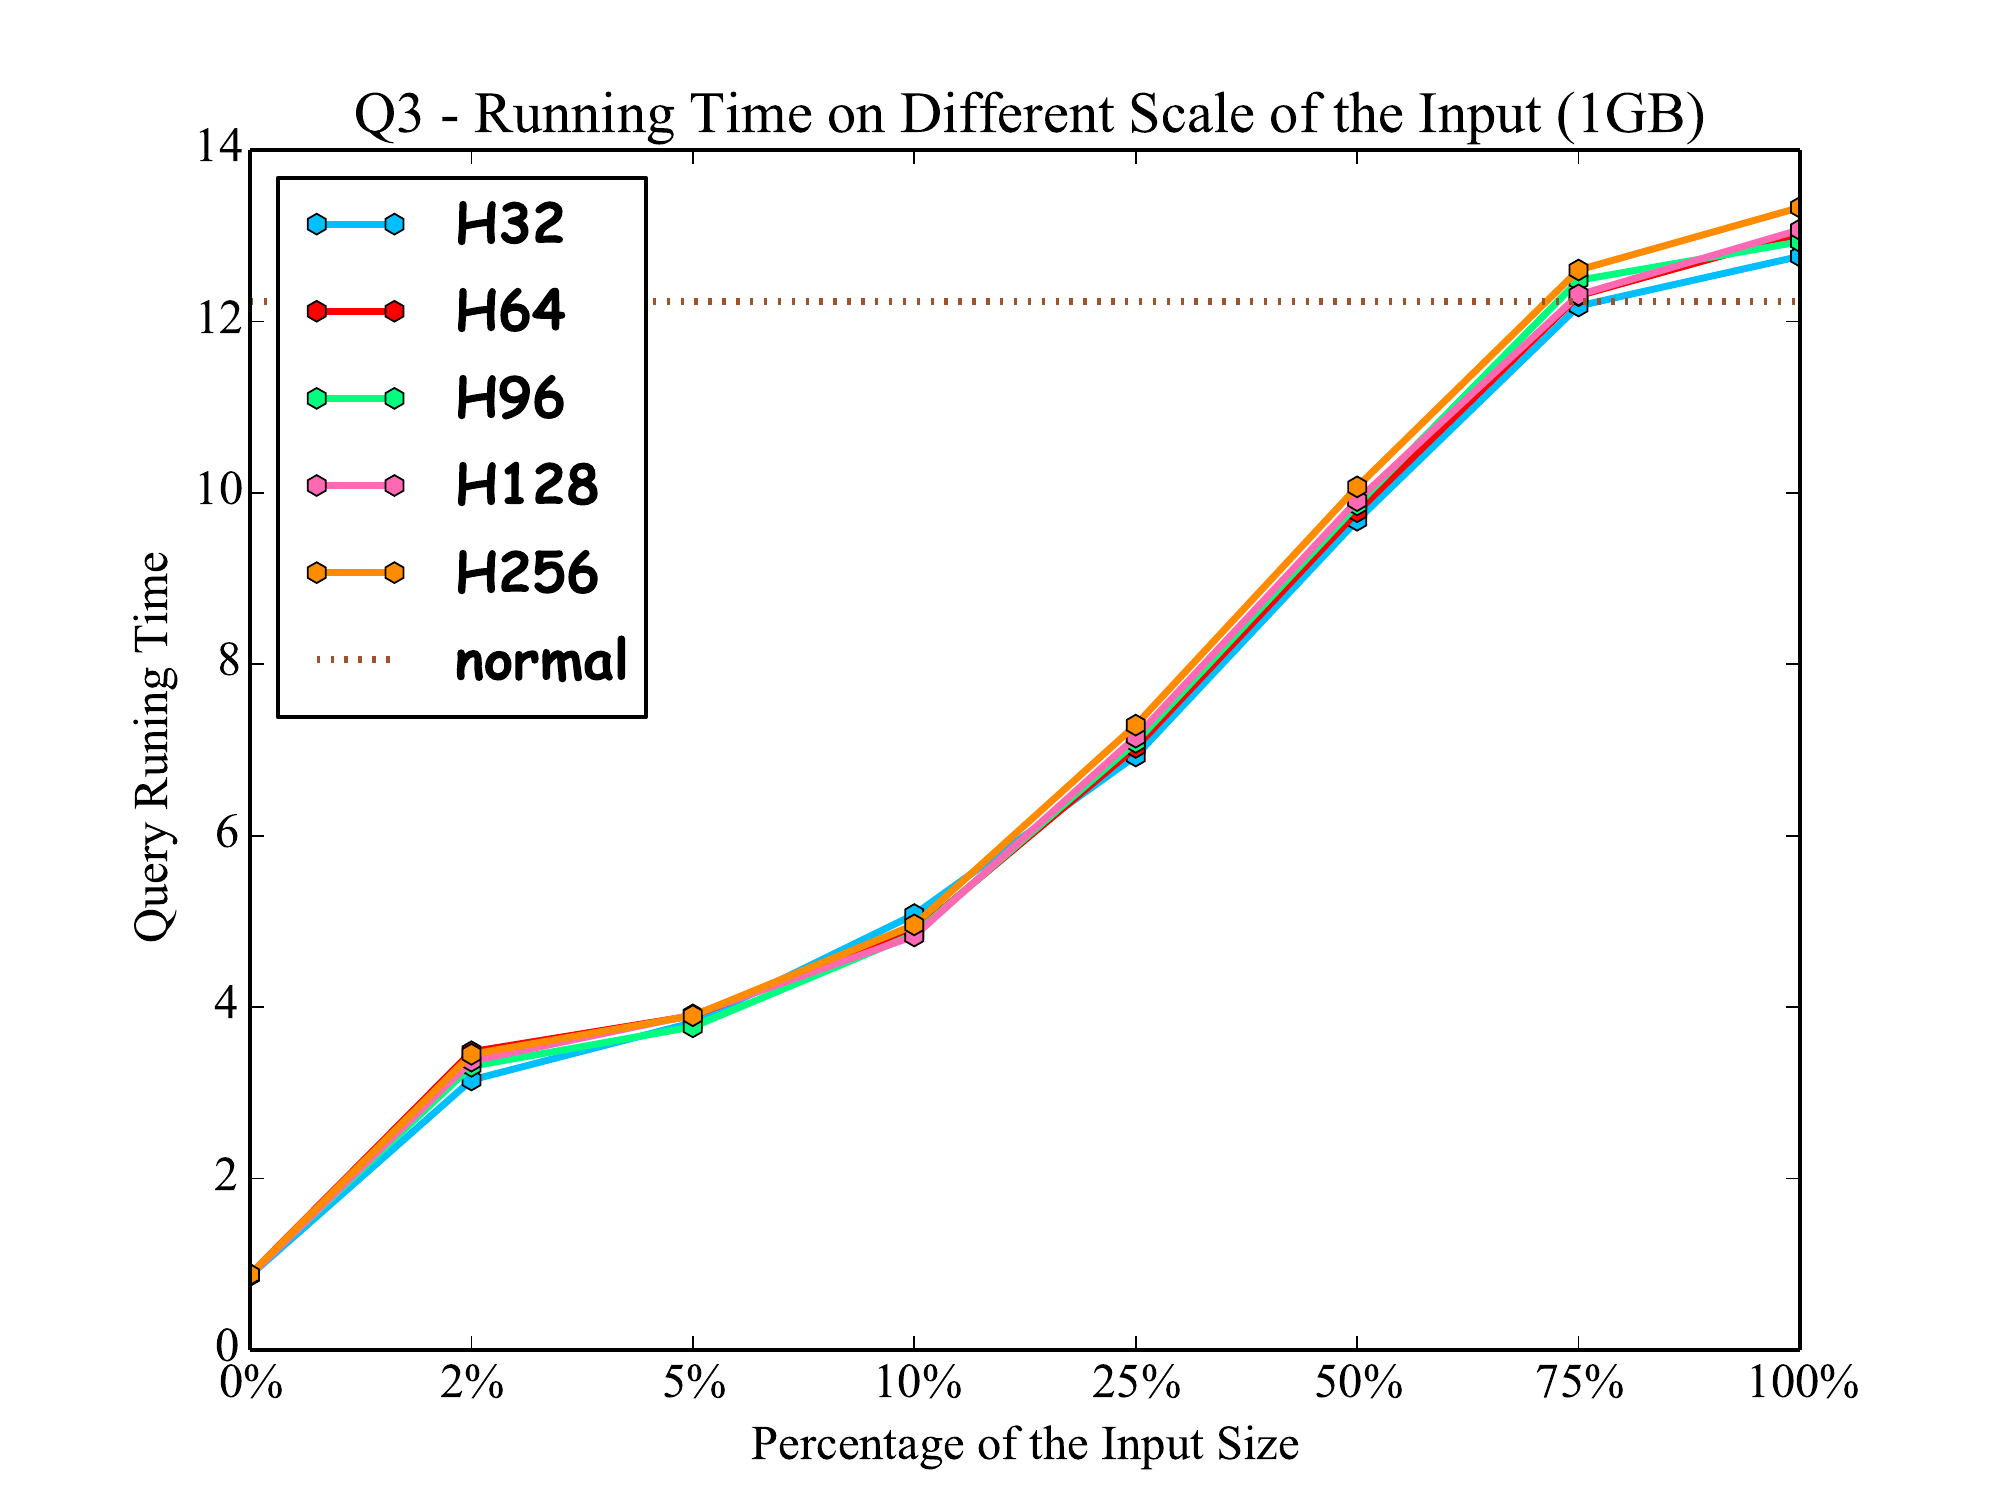}
   \caption{Fully virtual sketches + Pre-Hash +  Completly synthetic for Q3 on 1GB dataset}
   \label{fig:fv-ph-cs-q3-1gb}
 \end{figure}
%%%%%%%%%%%%%%%%%%%%%%%%%%%%%%%%%%%%%%%%
%
%
%%%%%%%%%%%%%%%%%%%%%%%%%%%%%%%%%%%%%%%%%
%%%%%q3 range
%%%%%%%%%%%%%%%%%%%%%%%%%%%%%%%%%%%%%%%%%
% \begin{figure}[H]
%   \centering
%   \includegraphics[width=0.8\linewidth,trim=0pt 0pt 0 0pt, clip]{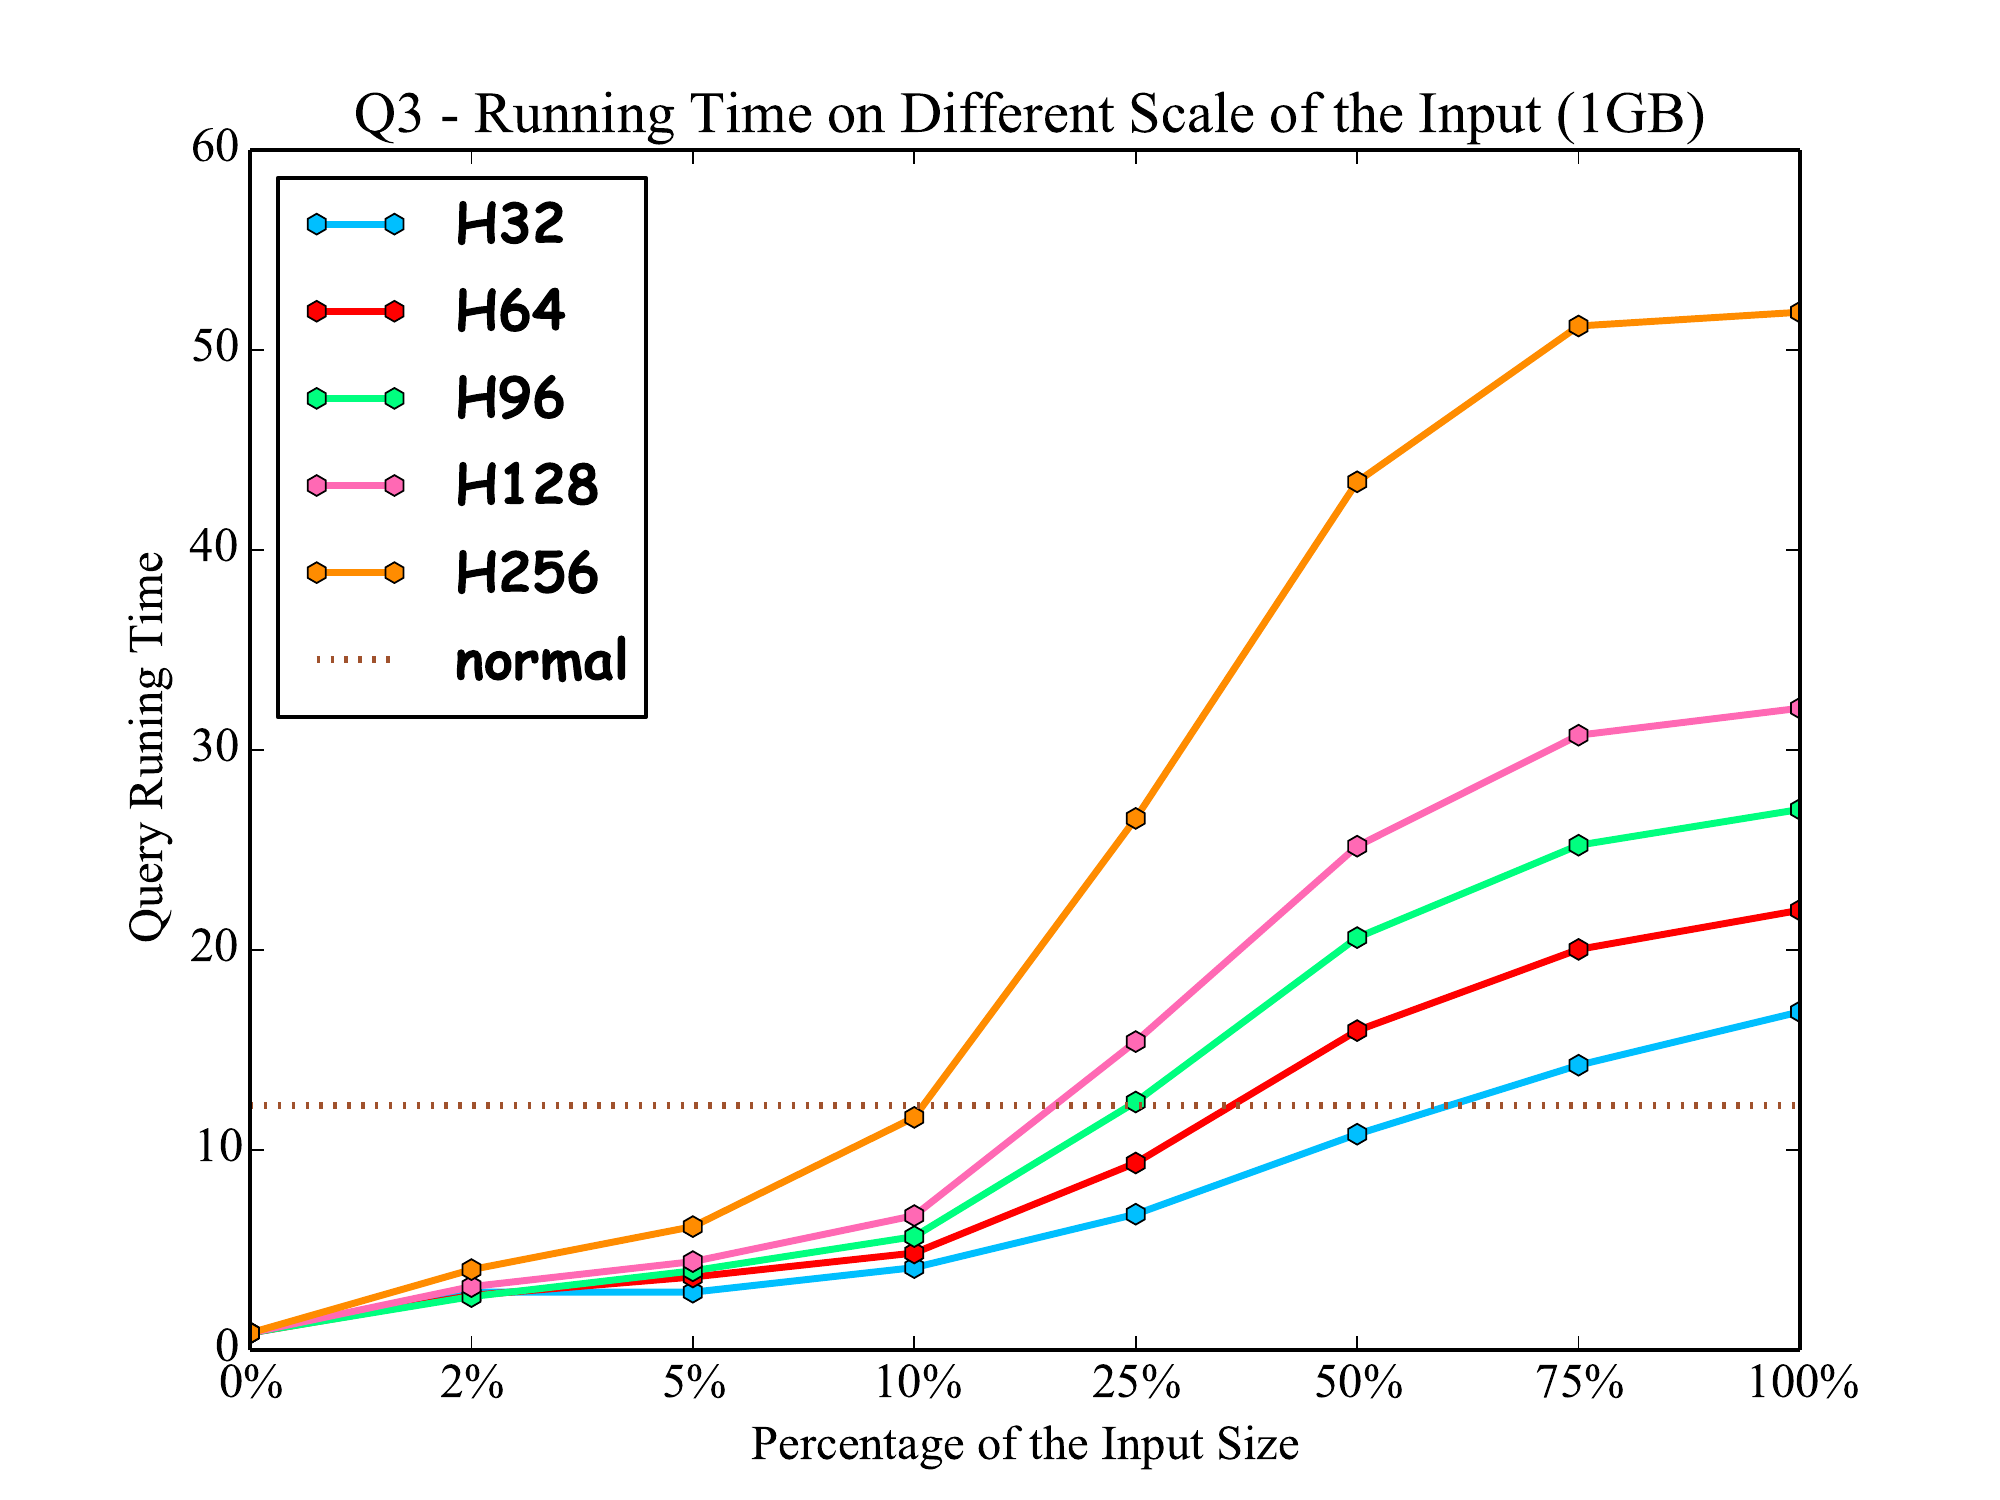}
%   \caption{Fully virtual sketches + Range +  Completly synthetic for Q3 on 1GB dataset}
%   \label{fig:fv-r-cs-q3-1gb}
% \end{figure}
%%%%%%%%%%%%%%%%%%%%%%%%%%%%%%%%%%%%%%%%%

%%%%%%%%%%q3 range @pengyuanli 4/9/2019
 \begin{figure}[H]
   \centering
   \includegraphics[width=0.8\linewidth,trim=0pt 0pt 0 0pt, clip]{figs/all/q3_range_1gb.pdf}
   \caption{Fully virtual sketches + Range +  Completly synthetic for Q3 on 1GB dataset}
   \label{fig:fv-r-cs-q3-1gb}
 \end{figure}
%%%%%%%%%%%%%%%%%%%%%%%%%%%%%%%%%%%%%%%%

%%%%%%%%%%q3 index range @pengyuanli 4/9/2019
 \begin{figure}[H]
   \centering
   \includegraphics[width=0.8\linewidth,trim=0pt 0pt 0 0pt, clip]{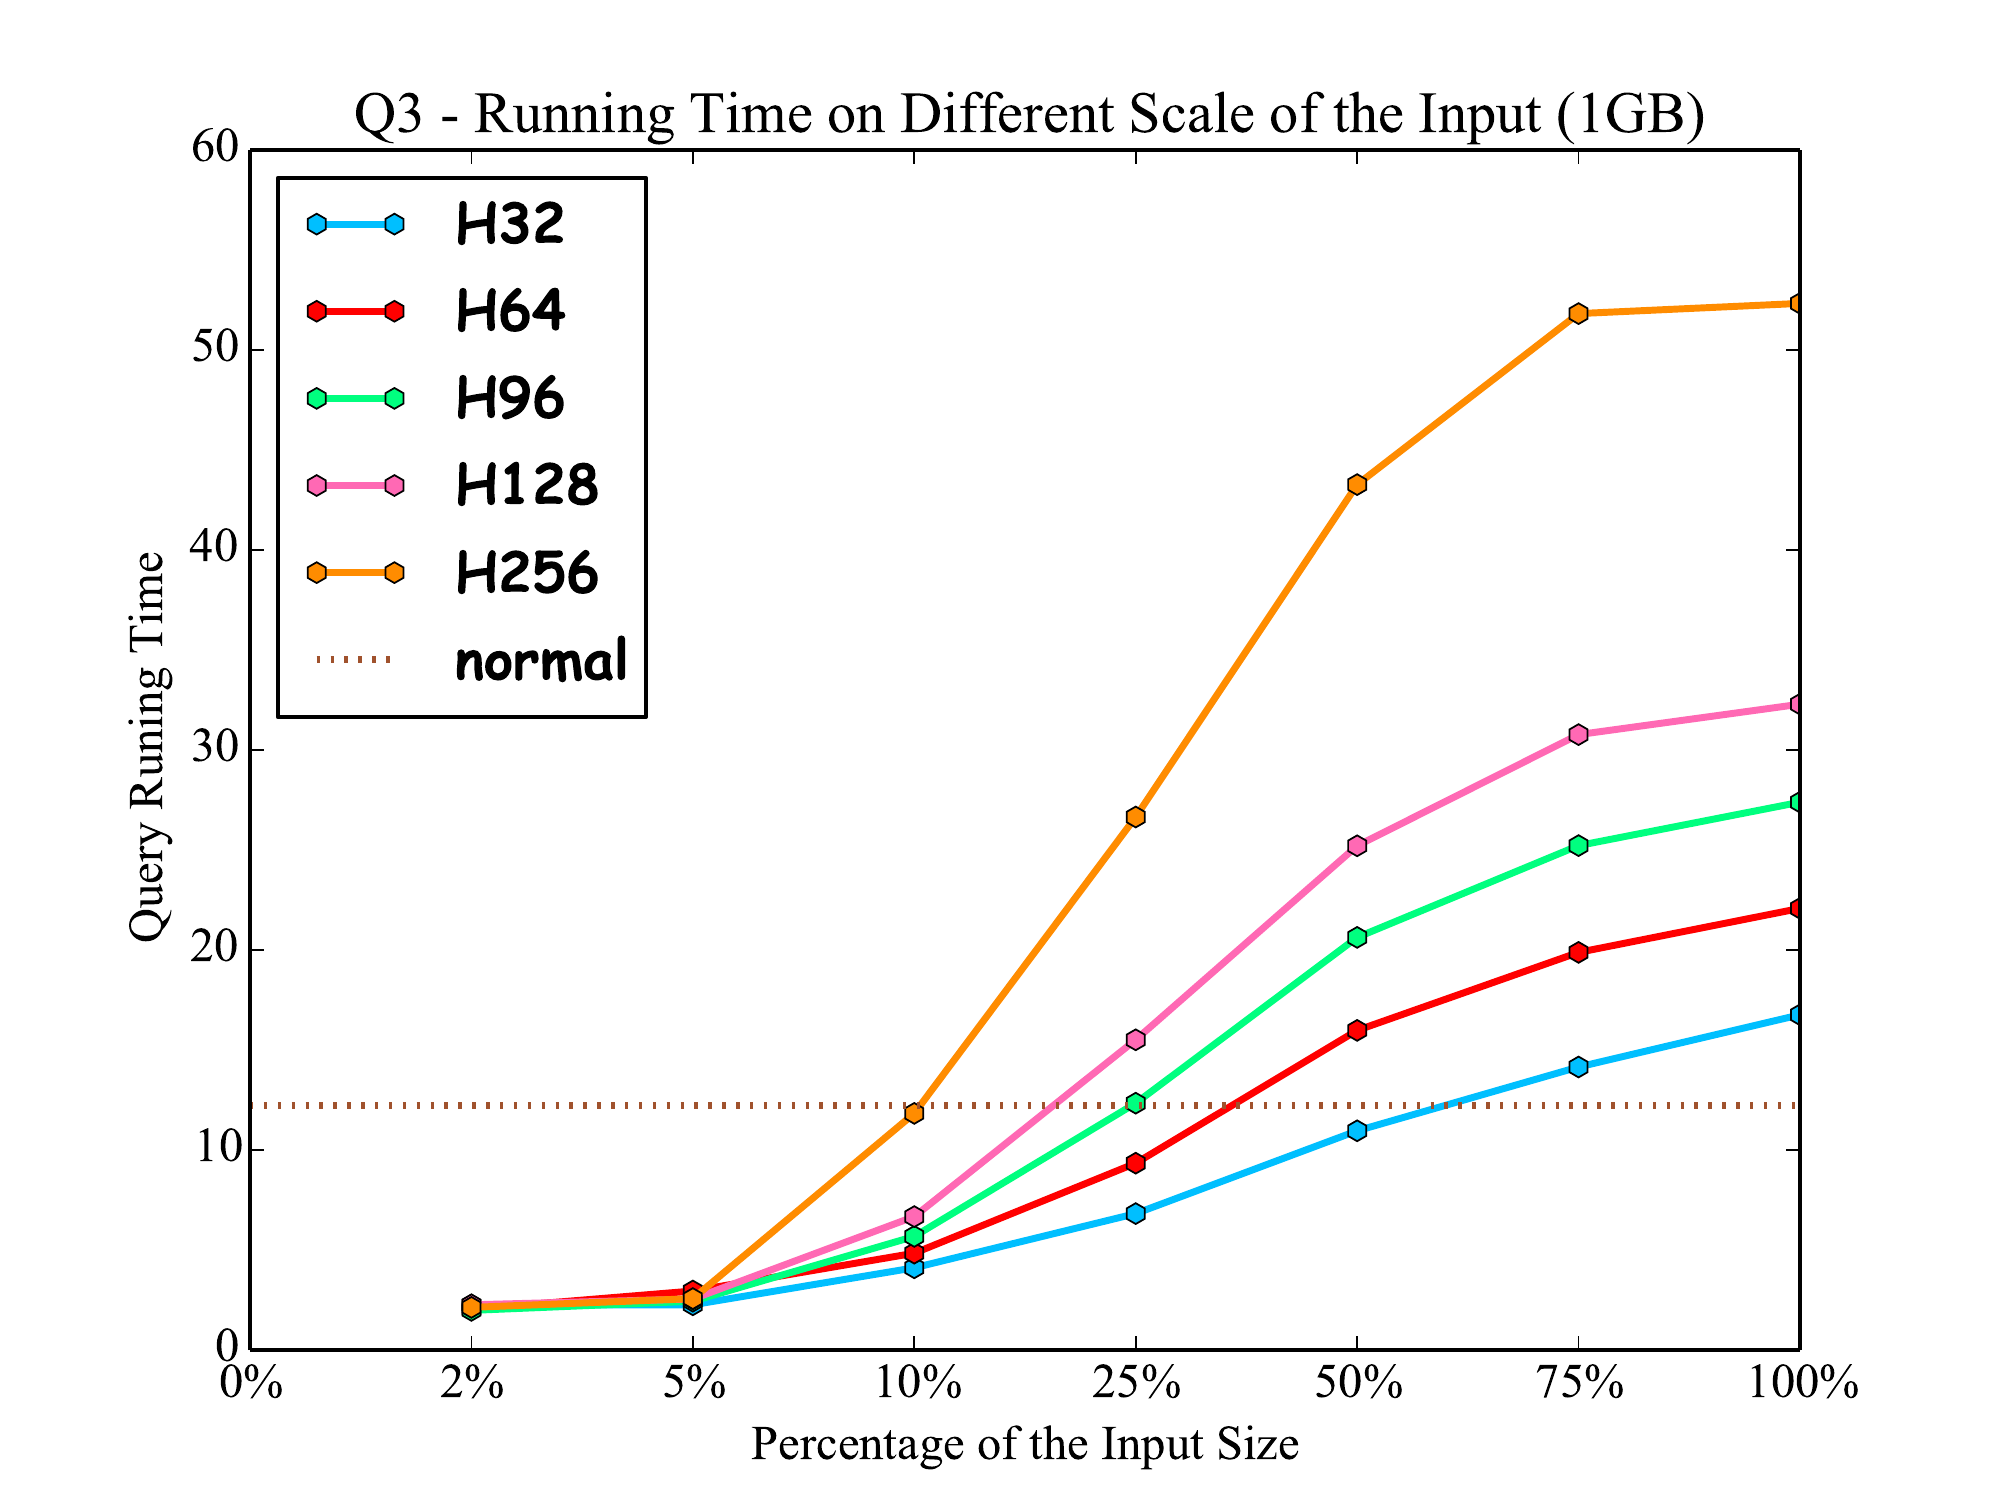}
   \caption{Fully virtual sketches + Range + index +  Completly synthetic for Q3 on 1GB dataset}
   \label{fig:fv-r-idx-cs-q3-1gb}
 \end{figure}
%%%%%%%%%%%%%%%%%%%%%%%%%%%%%%%%%%%%%%%%
%
%
%
%%%%%%%%%%%%%%%%%%%%%%%%%%%%%%%%%%%%%%%%%
%%%%%q4 hash
%%%%%%%%%%%%%%%%%%%%%%%%%%%%%%%%%%%%%%%%%
% \begin{figure}[H]
%   \centering
%   \includegraphics[width=0.8\linewidth,trim=0pt 0pt 0 0pt, clip]{figs/all/q4_hash_1gb.pdf}
%   \caption{Fully virtual sketches + Hash +  Completly synthetic for Q4 on 1GB dataset}
%   \label{fig:fv-h-cs-q4-1gb}
% \end{figure}
%%%%%%%%%%%%%%%%%%%%%%%%%%%%%%%%%%%%%%%%%
%
%
%%%%%%%%%%%%%%%%%%%%%%%%%%%%%%%%%%%%%%%%%
%%%%%q4 range
%%%%%%%%%%%%%%%%%%%%%%%%%%%%%%%%%%%%%%%%%
% \begin{figure}[H]
%   \centering
%   \includegraphics[width=0.8\linewidth,trim=0pt 0pt 0 0pt, clip]{figs/all/q4_range_1gb.pdf}
%   \caption{Fully virtual sketches + Range +  Completly synthetic for Q4 on 1GB dataset}
%   \label{fig:fv-r-cs-q4-1gb}
% \end{figure}
%%%%%%%%%%%%%%%%%%%%%%%%%%%%%%%%%%%%%%%%%

%%%%%%%%%%%%%%%%%%%%%%%%%%%%%%%%%%%%%%%%
%%%%q1 zone
%%%%%%%%%%%%%%%%%%%%%%%%%%%%%%%%%%%%%%%%
 \begin{figure}[H]
   \centering
   \includegraphics[width=0.8\linewidth,trim=0pt 0pt 0 0pt, clip]{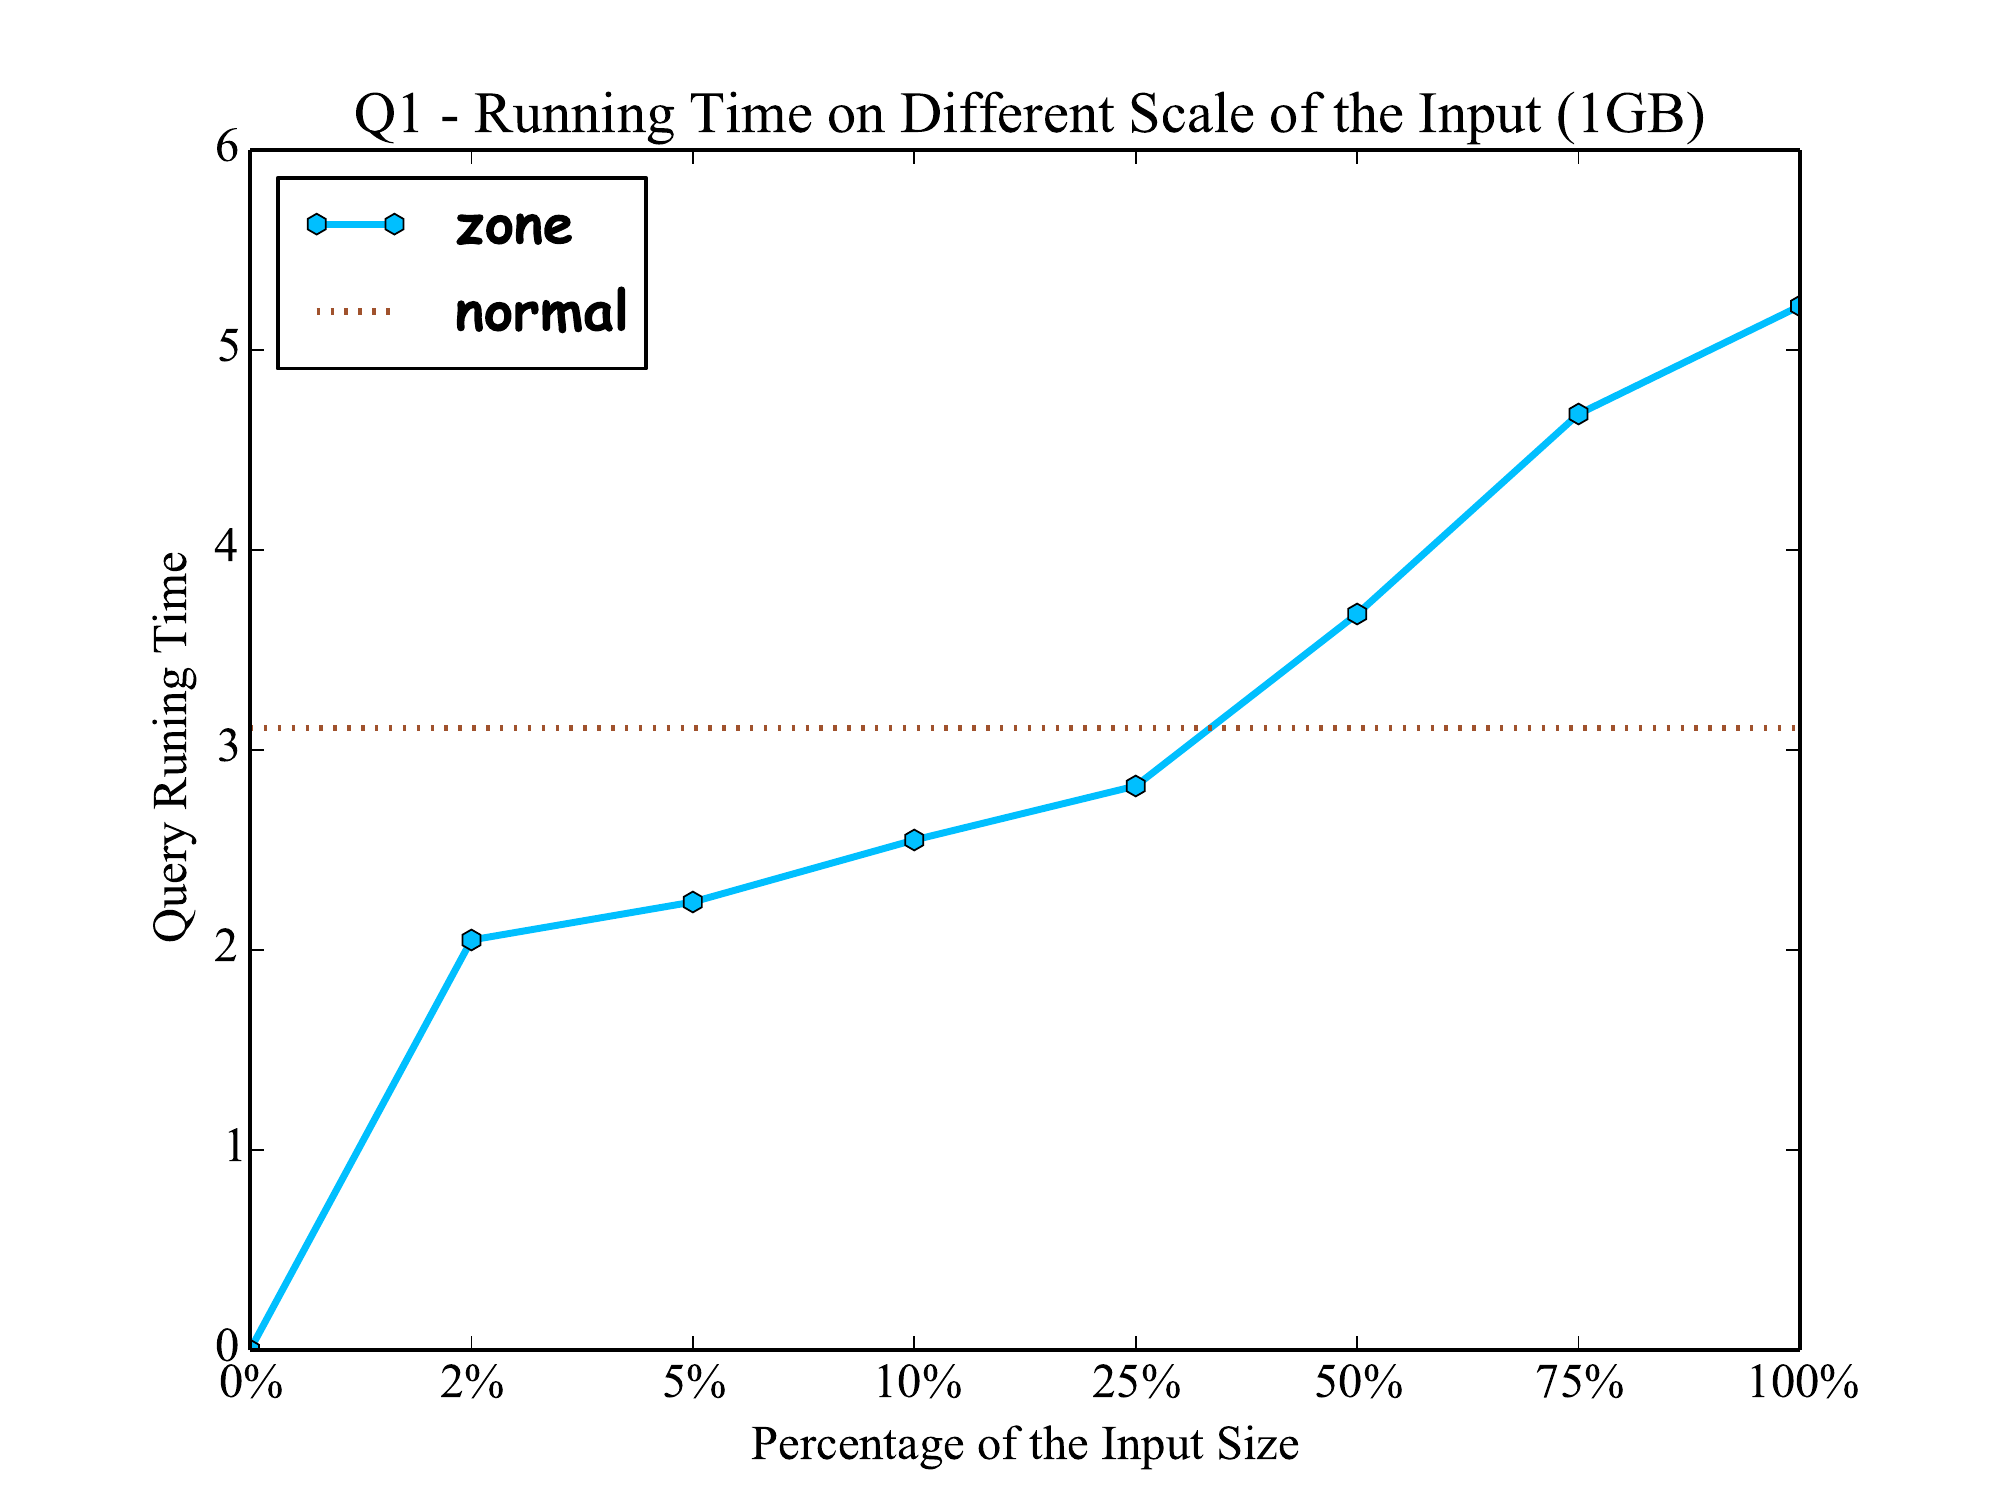}
   \caption{Fully virtual sketches + Zone +  Completly synthetic for Q1 on 1GB dataset}
   \label{fig:fv-z-cs-q1-1gb}
 \end{figure}
%%%%%%%%%%%%%%%%%%%%%%%%%%%%%%%%%%%%%%%%

%%%%%%%%%%%%%%%%%%%%%%%%%%%%%%%%%%%%%%%%
%%%%q2 zone
%%%%%%%%%%%%%%%%%%%%%%%%%%%%%%%%%%%%%%%%
 \begin{figure}[H]
   \centering
   \includegraphics[width=0.8\linewidth,trim=0pt 0pt 0 0pt, clip]{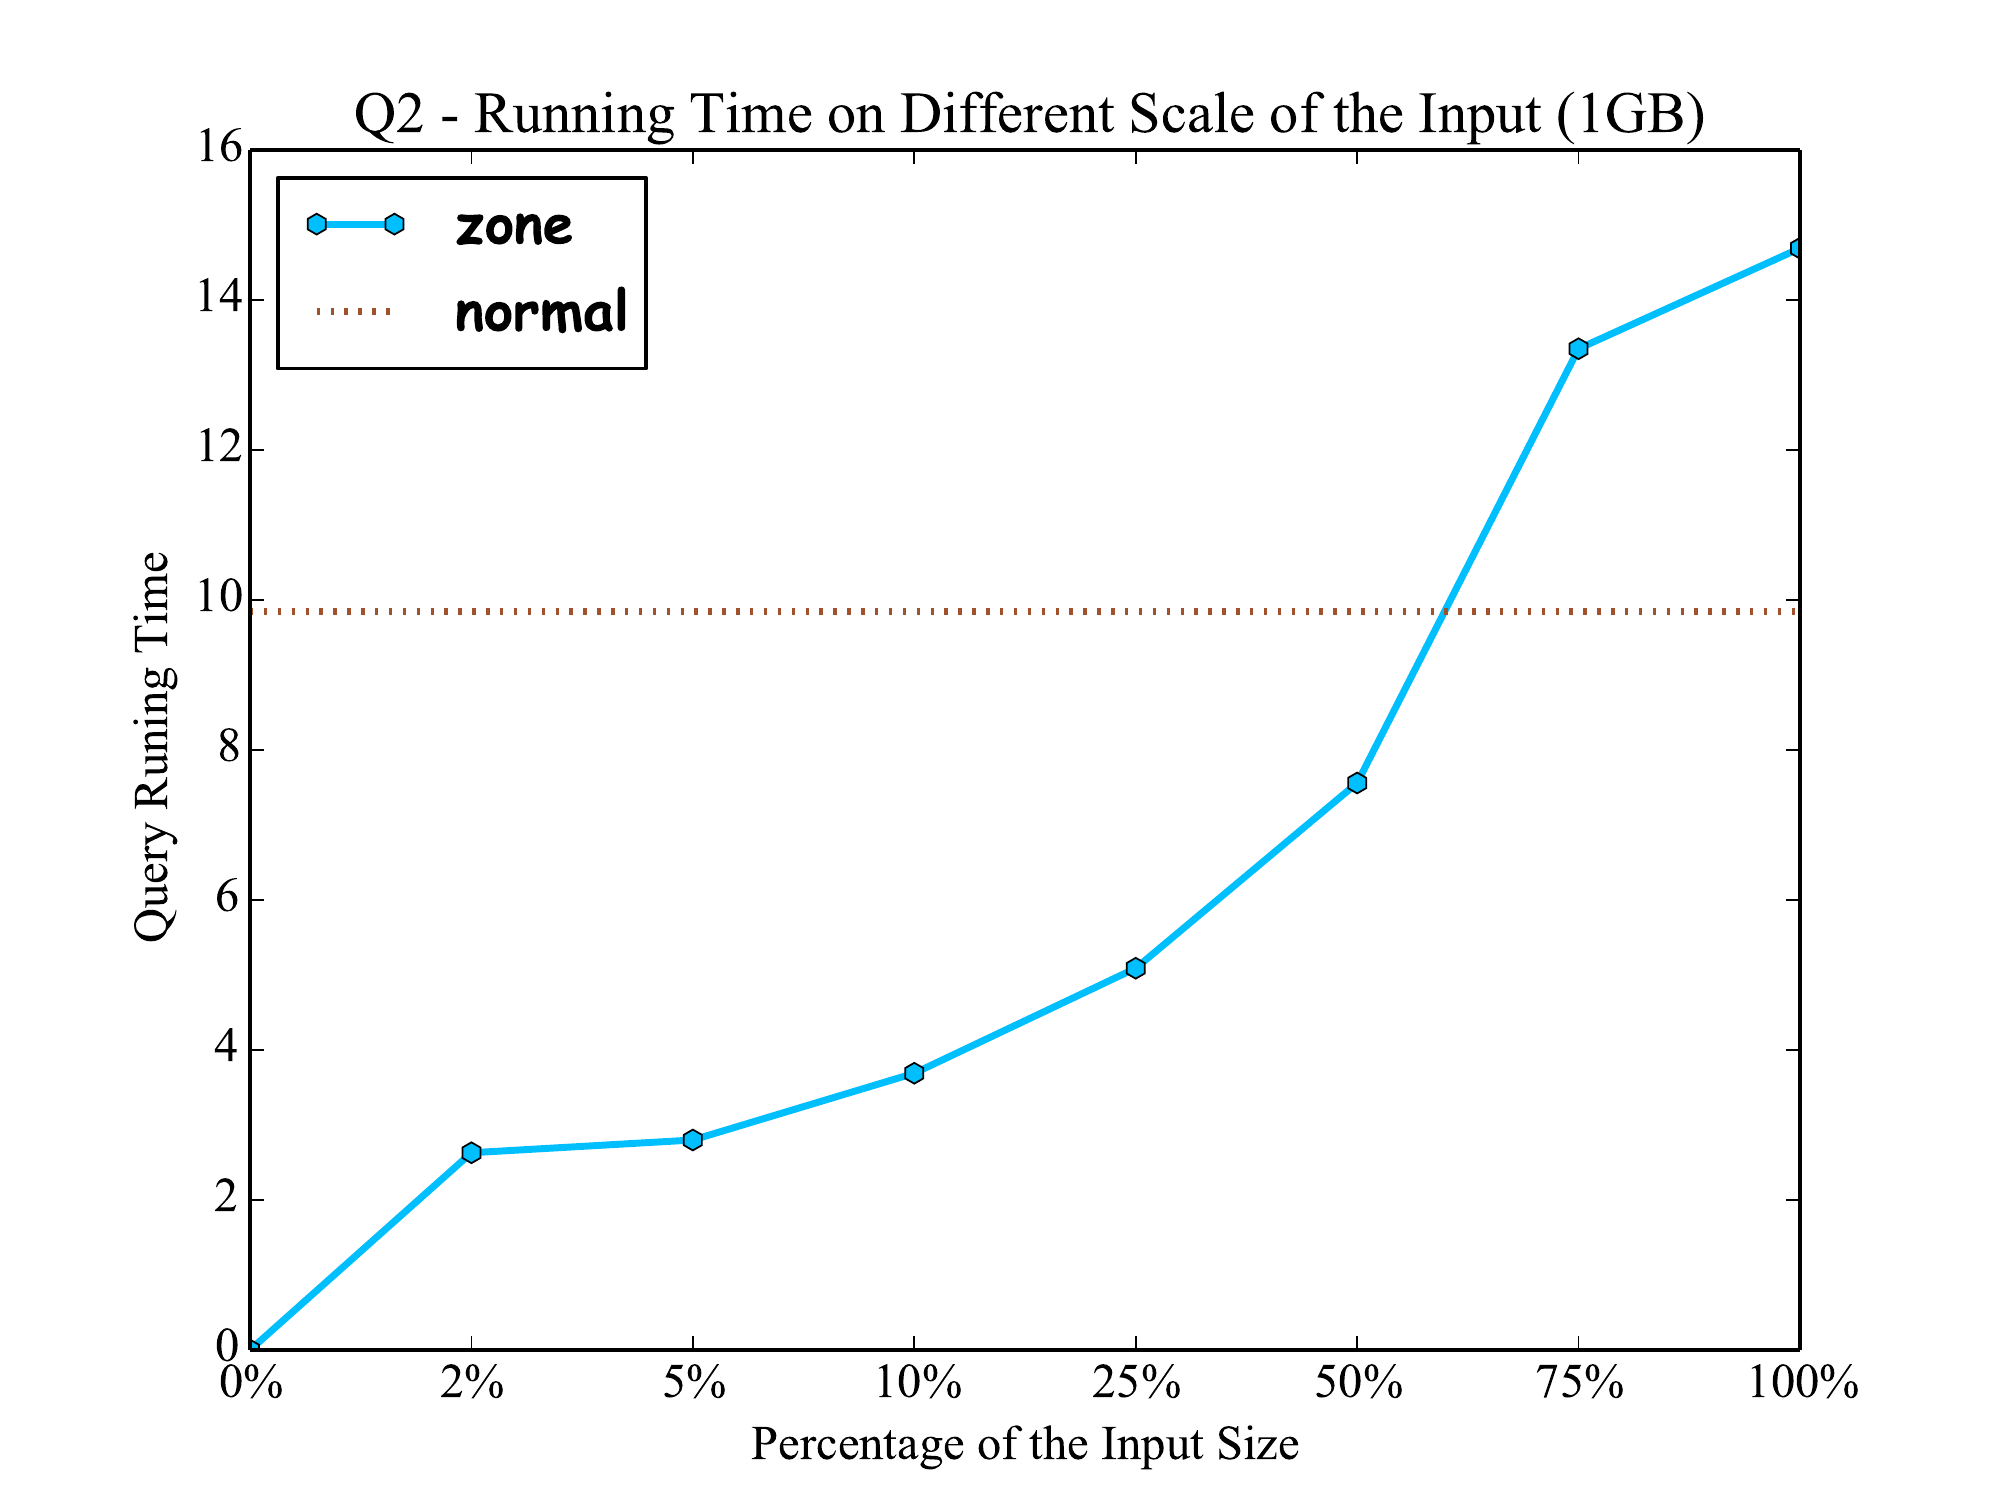}
   \caption{Fully virtual sketches + Zone +  Completly synthetic for Q2 on 1GB dataset}
   \label{fig:fv-z-cs-q2-1gb}
 \end{figure}
%%%%%%%%%%%%%%%%%%%%%%%%%%%%%%%%%%%%%%%%

%%%%%%%%%%%%%%%%%%%%%%%%%%%%%%%%%%%%%%%%
%%%%q2 zone
%%%%%%%%%%%%%%%%%%%%%%%%%%%%%%%%%%%%%%%%
 \begin{figure}[H]
   \centering
   \includegraphics[width=0.8\linewidth,trim=0pt 0pt 0 0pt, clip]{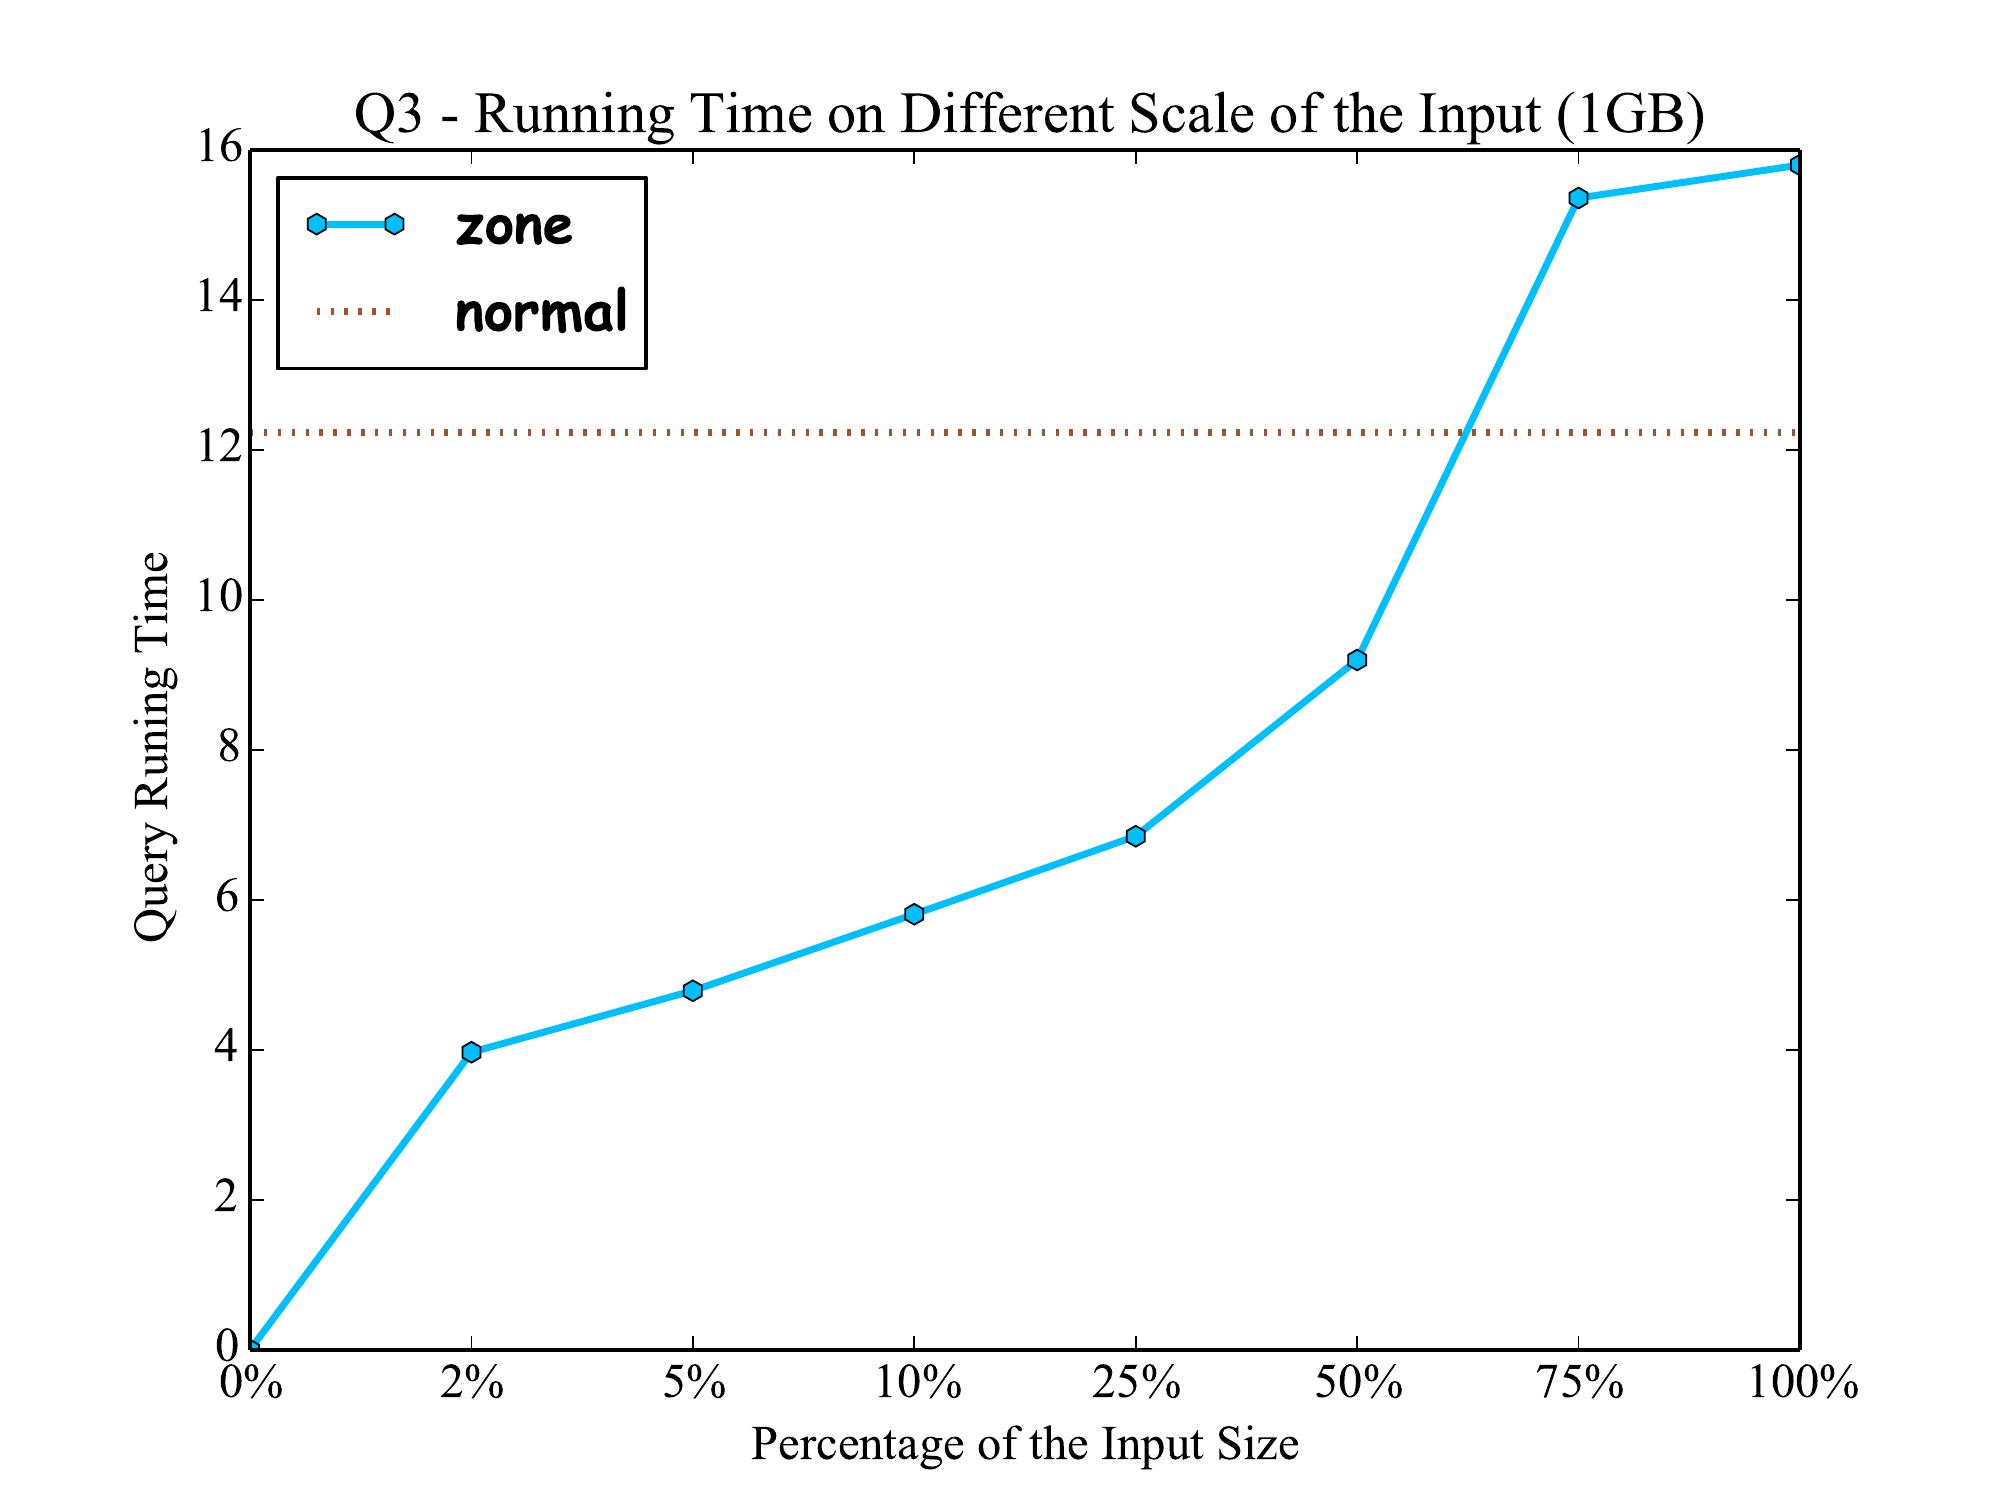}
   \caption{Fully virtual sketches + Zone +  Completly synthetic for Q3 on 1GB dataset}
   \label{fig:fv-z-cs-q3-1gb}
 \end{figure}
%%%%%%%%%%%%%%%%%%%%%%%%%%%%%%%%%%%%%%%%

\parttitle{Range + Completly synthetic} 
Test Q1, Q2 on 1GB and 10GB datasets.

%%%%%%%%%%%%%%%%
\subsection{Result - Physical sketches}
\label{sec:p-result}
