# Supplementary material for: Provenance-based Data Skipping (TechReport)
Source: arXiv:2104.12815 source file (2021-05-27)
Supplement: Supplementary file 3 [file ps_appendix.tex]

%%%%%%%%%%%%%%%%%%%%%%%%%%%%%%%%%%%%%%%%%%%%%%%%%%%%%%%%%%%%%%%%%%%%%%%%%%%%%%%%
\section{Provenance Sketches}
\label{sec:prov-sketch}

As introduced in Sec.~\ref{sec:introduction} we designed the provenance sketch to concisely represent a superset of the provenance by dividing the dataset to each distinct partition and including all the partitions which contain the provenance of the query. In this section, we focus on discussing how do we define a provenance sketch and what kinds of provenance sketches we support.

\subsection{Definitions}
\label{tab:ps_def}

\parttitle{Horizontal Partitioning} Instead of annotating each input tuple, our approach focuses on annotating each partition of inputs. Here we define horizontal partitioning that a table is horizontally divided into each distinct fragment represented as $\frag$. 
%\medskip\noindent\fbox{%\todo{relation partition, database partition}
%  \begin{minipage}{1.0\linewidth}
  \begin{defi}[Horizontal Partitioning]
    Let $R$ be a table.  $\parti = \{ \frag_1, \ldots, \frag_n \}$ is called a horizontal partitioning of $R$ if all of the following conditions are satisfied:
%     into $n$ distinct parts by tuples, we say each part is a partition of the
% table $R$ noted as $PA_{i}(R,n)$ where $i \in [1,n]$ if it satisfies following conditions:  %i.e., $$ PA_{i}(R,n) \subseteq R \wedge \displaystyle\sum_{n=1}^{n} PA_{i}(R,n) = R $$.
\begin{itemize}
%  \item $\frag_{i} \subseteq R $ for all  $i \in [1:n]$
  \item $\frag_{i} \cap \frag_{j} = \emptyset$ for all $i, j \in [1:n] \wedge i \neq j$
  \item $ \displaystyle\bigcup_{i=1}^{n} \frag_{i} = R $ for all $i \in \{1, ..., n\}$
\end{itemize}
\end{defi}
%\end{minipage}
%}\\[4mm]

%Here, we call each $\frag$ as a fragment.
\parttitle{Partitioning of Database} We do partitioning on each table of database and all of the fragments belong to the partitioning of this database. 

%\medskip\noindent\fbox{%\todo{relation partition, database partition}
%  \begin{minipage}{1.0\linewidth}
\begin{defi}[Partitioning of Database]
  Given a database $\db =  \{\rel_1, \ldots, \rel_m\}$, we call $\dbpart = \{ \parti_1, \ldots, \parti_m \}$ a partitioning of $\db$ if for all $i \in [1,m]$ $\parti_i$ is a partitioning of relation $\rel_i$.
We use $\fragsOf{\dbpart} = \bigcup_{i}^{m} \parti_i$ to denote all fragments that occur in the individual relation partitioning $\parti_i$.
\end{defi}

\parttitle{Provenance Sketch} Provenance sketch is constructed by all the fragments in the database that contain the provenance of the query. 

\begin{defi}[Provenance Sketch (PS)]
Given a query $\query$, a database $\db$, and a  partitioning $\dbpart$ for $\db$.  % where $PA(I)$ denotes each partition in $I$ and $PAD(I)$ denotes all the partitions.
We call % the unique
a subset $\provSketch \subseteq \fragsOf{\dbpart}$ that fulfills the conditions below a provenance sketch for $\query$ and $\db$ according to $\dbpart$. % if it fulfills the following conditions.
    Here we use $\instOf{\provSketch}$ to denote $\bigcup_{\frag \in \provSketch} \bigcup_{t \in \frag} t$ where t indicates the tuple in each table.
%    provenance $P(Q,I)$, tuple $t$ in $I$, we say $S$ a set of partitions ($PA$) on $I$ is a provenance sketch of the query $Q$ on database $I$ noted as $PS(Q,I)$ if following conditions hold.
\begin{itemize}
%\item $ \forall t \in P(Q,I): \exists PA \in PS: \exists S \in PA:  t \in S$
%\item $ \forall PA \in PS: \forall S \in PA: \exists t \in S: t \in P(Q,I)$
\item $ \forall t \in \prov {Q}{I} : \exists \frag \in \provSketch: t \in \frag$

\end{itemize}
\end{defi}

\begin{lem}
  If $\provSketch$ is a provenance sketch for $Q$ and $I$ wrt. $\dbpart$, then
  $ \prov{Q}{I} \subseteq I_{PS} \subseteq I $
\end{lem}

\begin{proof}
Provenance sketch is a set of fragments in I which contains the provenance of a query Q, thus $\forall t \in \prov{Q}{I} : t \in  I_{PS}$ , then  $ \prov{Q}{I} \subseteq I_{PS}$. Obviously, $I_{PS} \subseteq I $.
\end{proof}

\subsection{Types of Provenance Sketch}
\label{tab:ps_type}

To compute a provenance sketch $\provSketch$ for a query $Q$ and
database $I$ according to $\dbpart$,
we might get different $\dbpart$ which based on the different parititioning methods we used for each table in the database $I$ such that we might get different provenance sketches.
Currently, we are supporting the following partitioning methods:

\begin{itemize}
\item  \textbf{Hash-based}: we compute a hash over a set of attributes $A$, thus the tuples with the same hash value belong to the same fragment.
\begin{defi}[Hash-partition] \label{def:hash}
  Let $R$ be a table, $A \subseteq \schema{R}$, and $h: A \to \mathbb{N}$ a hash function over $A$. Then the partitioning $$\parti_{h,A}(R) = \{ S_{R,t} \mid t \in R \}$$
$$S_{R,t} = \{ t' \mid t' \in R \wedge h(t.A) = h(t'.A) \}$$
\end{defi}

\item  \textbf{Range-based}: We define a set of ranges over the value of an attribute a which covers all values of a, the tuples in the same range belong to the same fragment.

\begin{defi}[Range-partition] \label{def:range}
  Given a table $R$, a domain $\domain{a}: a \in \schema{R}$, and a set of ranges $r_1, \ldots, r_n$ covering all the values in $\domain{a}$ and $r_i \cap r_j = \emptyset: i \neq j$. Then the partitioning $$\parti_{r,a}(R) = \{ S_1, \ldots, S_n \}$$
$$S_{i} = \{ t \mid t \in R \wedge t.a \in  r_i \}$$
\end{defi}

\item \textbf{Page-based}: we extract the page numbers from the \lstinline!ROWID! values of tuples and
  then hash these page numbers into a target range of values, e.g., [0,63], such that the pages with the same hash value belong to the same fragment.
\begin{defi}[Hash-page-partition]\label{def:page}  Let $R$ be a table we use $t.\page$ to denote the number of page on which $t$ is stored on. % of the pages belong to $R$.
  Then the partitioning $$\parti_{h,page}(R) = \{  S_{R,h_{\page}} \mid \exists t \in R: h(t.\page) = h_{\page} \}$$
$$S_{R,h_{\page}} = \{ t \mid t \in R \wedge h(t.\page) = h_{page} \}$$
\end{defi}

\end{itemize}
Different partition methods might be suitable for different queries or data layout, for example, if the provenance of a query concentrates on only a few pages, page-based partitioning might be good for this case. Since range-partition could correspond directly to the physical design of the database such as index, pyhsical partitioning, small materialized aggregates and others in which case using the provenance sketch can actually skip I/O. 
