# Supplementary material for: Provenance-based Data Skipping (TechReport)
Source: arXiv:2104.12815 source file (2021-05-27)
Supplement: Supplementary file 4 [file use_appendix.tex]

%%%%%%%%%%%%%%%%%%%%%%%%%%%%%%%%%%%%%%%%%%%%%%%%%%%%%%%%%%%%%%%%%%%%%%%%%%%%%%%%
\section{Making Use of Provenance Sketch}
\label{sec:prov-reuse}
After provenance sketch is captured, we could utilize it to speed up the subsequent runs of the query. In this section we introduce how do we apply the provenance sketch to the query. The steps include decoding the provenance sketch to a format that the query could recognized, i.e., a set of filter predicts, and then we can create a where clause for the input table to add the filter predicts into the query to achieve our goal that removing the unncessary input tuples early on. And also this filter predicts could be used by some physical designs to skip the I/O. Thus the important part is how to decode the provenance sketch for different partitioning methods which would be introduced in the following. 
%to use the captured provenance sketch such that the subsequent runs of the query could be speeded up by it. The steps include decoding the provenance sketch to a where clause that indicates which partitions are used and adding the where clause to its matched table exits in the from clause to reconstruct the query. 

\subsection{Provenance Sketch Decoding}
\label{tab:ps_decode}
Since the provenance sketch represents which fragments to use, thus the idea is that we translate the provenance sketch to the fragments and construct the fragments to a condition the query could use. 

\parttitle{Range-based Provenance Sketch}
For range partition, each fragment could be represented as a range, then we only need to figure out the range of each fragment in the provenance sketch. Let us reconsider the example in Sec.~\ref{sec:ps-capture}, the captured provenance sketch is `0101' in Fig.~\ref{tab:cp-eg-result}. Recall 1' means this fragment contains the provenance and `0' without provenance. Combined with the range infromation shown in Fig.~\ref{fig:bit-vector-use}, we can figure out the ranges [2,4) and [5,6) incldues the provenance, thus we can generate the where clause with condition ($depid>= 2$ AND $depid <4$) or ($depid>=5$ AND $depid<6$). At last, we insert the where clause into the query Q (Fig.~\ref{fig:eg-q}) and the reconstructed query $Q^{use}$ is shown in Fig.~\ref{fig:eg-q-use}. 
 %%%%%%%%%%%%%%%%%%%%%%%%%%%%%%%%%%%%%%%%
 \begin{figure}[t]
   \centering
   \includegraphics[width=0.7\linewidth,trim=0 0pt 0 0pt, clip]{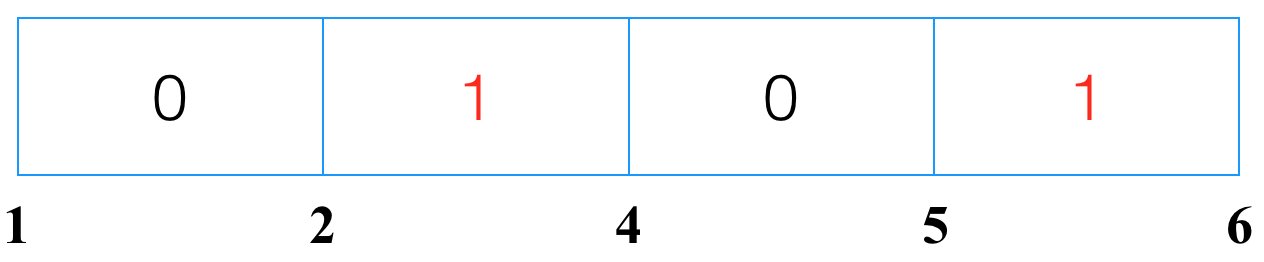}
   \caption{$ps_{salaries}$ on Column depid}
   \label{fig:bit-vector-use}
 \end{figure}
%%%%%%%%%%%%%%%%%%%%%%%%%%%%%%%%%%%%%%%% 	

\begin{figure}[t]
\begin{tabular}{c}
\lstset{tabsize=4,style=psqlcolor,basicstyle=\scriptsize\upshape\ttfamily}
\begin{lstlisting}
SELECT avg(salary) AS avg_salary, depid 
FROM (
	SELECT * FROM salaries 
	WHERE (depid>= 2 AND depid <4) or (depid>=5 AND depid<6))
GROUP BY depid
ORDER BY avg_salary
LIMIT 2;
\end{lstlisting}
\end{tabular}
\caption{Example Reconstruted Query $Q^{use}$}
\label{fig:eg-q-use}
\end{figure}

\parttitle{Hash-based Provenance Sketch}
Different with range partition, in hash partition each fragment contains the tuple with the same hash result, i.e., one distinct hash result represents one fragment. Thus the provenance sketch could be decoded to a set of hash results, then we only need to figure out which tuples' hash result is in this set. %What we do is that we first hash each tuple to get the hash result and then 
What we do is we use a \emph{in} clause which contains the set of the decoded hash results used to filter out the input tuples not in the provenance sketch. Reconsdier the captured provenance sketch is `0101' in Fig.~\ref{tab:cp-eg-result} but using the hash partition, then the generated where clause would be
\lstset{tabsize=4,style=psqlcolor,basicstyle=\scriptsize\upshape\ttfamily}
\begin{lstlisting}
	 				WHERE hash(depid,4) in (2,4)
\end{lstlisting}

\parttitle{Hash-page-based Provenance Sketch}
Similar to the hash partition, instead of hashing on column, this method do hash on the page number, thus the generated where clause would be 
\lstset{tabsize=4,style=psqlcolor,basicstyle=\scriptsize\upshape\ttfamily}
\begin{lstlisting}
	 		WHERE hash((ctid::text::point)[0],4) in (2,4)
\end{lstlisting}

\subsection{Optimization}
\label{tab:use_opt}
Since for the range partition, we might generate a large number of comparison conditions which would lead to a poor performance if the database optimizer could not figure out a suitable plan for it. Thus we apply some optimization for it, such as if the comparision condition are continous, we merge them to one comparision condition. Also, we implement the binary search method to check each condition which works for the table size is large and the database optimizer could not find a good plan for it. 

For the hash-based and hash-page-based provenance sketches, we need to compute a hash firstly which would increase the query cost. But if we do some preprocessing of the table such as pre-hashing the column and store the hash result in a column, or maybe physical partition on this column, the performance would be highly improved. However, without do any preprocessing of the table, range-based provenance sketch could already highly improve the performance for most case. At the same time, it can also use the index or other physical designs directly. Thus, in this paper, our experiment will mainly focus on the range-based provenance sketch.
